# Supplementary material for: Space-Time Modulated Metasurfaces with Spatial Discretization: Free-Space N-path Systems
Source: arXiv:2006.06394 source file (2020-11-15)
Supplement: Supplementary file 1 [file main.tex]

\documentclass{article}
\usepackage[a4paper, total={6in, 8in}]{geometry}
\usepackage[utf8]{inputenc}
\usepackage{url}
\usepackage{graphicx}% Include figure files
\usepackage{dcolumn}% Align table columns on decimal point
\usepackage{bm}% bold math
%\usepackage{hyperref}% add hypertext capabilities
%\usepackage[mathlines]{lineno}% Enable numbering of text and display math
%\linenumbers\relax % Commence numbering lines
\usepackage{slashbox}
\usepackage[caption=false]{subfig}
\usepackage{float}
\usepackage{xcolor}
\usepackage{amsmath}
\usepackage{amssymb}
\usepackage{array}
\usepackage{array,booktabs}% http://ctan.org/pkg/{array,booktabs}
\newcolumntype{P}[1]{>{\centering\arraybackslash}p{#1}}
\renewcommand{\theequation}{S.\arabic{equation}}
\renewcommand{\thefigure}{S\arabic{figure}}
\renewcommand\thesection{\Roman{section}}
\renewcommand{\thetable}{S\arabic{table}}
\usepackage{placeins}
\usepackage{adjustbox}
\usepackage{multirow}

\title{Supplemental Materials}
\author{Zhanni Wu, Cody Scarborough, Anthony Grbic}
\date{June 2020}

\begin{document}

\maketitle

%%%%%%%%%%%%%%%%%%%%%%%%%%%%%%%%%%%%%%%%%%%%%%%%%%
%%%%%%%%%%%%%%%%%%%%%%%%%%%%%%%%%%%%%%%%%%%%%%%%%%
%%%%%%%%%% Section 1
%%%%%%%%%%%%%%%%%%%%%%%%%%%%%%%%%%%%%%%%%%%%%%%%%%
%%%%%%%%%%%%%%%%%%%%%%%%%%%%%%%%%%%%%%%%%%%%%%%%%%

\section{Finding the time-modulated sheet capacitance for each stixel}

In this section, the relation between the reflection phase and the sheet capacitance over one stixel of the structure shown in Fig. 1 of the manuscript will be derived. At the operating frequency of $f_0= \omega_0/{2 \pi}= 10$ GHz, the tangential wave admittance in the substrate for $TE$ and $TM$ polarizations are, 
%If excited by a plane wave with radial frequency $\omega_0$ and tangential %wavenumber $k_x$, the scattered fields can be expanded in terms of frequencies %$\omega_q = \omega_0 +q \omega_p$, and wavenumbers $k_{xq}=k_x + 2\pi q/d$. The %wave admittances in the substrate for each polarization at frequency %$\omega_q=\omega_0+q\omega_p$ are,
%\begin{align}\label{Zmsub} 
%Y_{sq}^{TE}=\frac{k_{szq}^{TE}}{\mu_0\omega_q},\quad
%Y_{sq}^{TM}=\frac{\epsilon_0\epsilon_h\omega_q}{k_{szq}^{TM}}.
%\end{align}
%where
%\begin{align}\label{Kmsub}
%k_{sqz}^{TE}=\sqrt{\frac{\omega_q^2}{c^2}\epsilon_h-k_x^2},\quad
%k_{sqz}^{TM}=\sqrt{\frac{\omega_q^2}{c^2}\epsilon_h-k_x^2\frac{\epsilon_h}{\eps%ilon_{zz}}}, 
%\end{align}
%are the normal wavenumbers in the substrate. 
\begin{align}
Y_{s0}^{TE}&=\frac{E_y}{-H_x} =\frac{k_{s0z}^{TE}}{\mu_0\omega_0}, \label{ZsubTE} \\
Y_{s0}^{TM}&=\frac{E_x}{H_y}=\frac{\epsilon_0\epsilon_h\omega_0}{k_{s0z}^{TM}},
\label{ZsubTM} 
\end{align}
where subscripts $s$, $0$ and $z$ denote the substrate, the operating frequency $\omega_0$, and the z-component of the wavenumber, respectively. The relative permittivity of the substrate is $\epsilon_h$. Note that the substrate admittance looking down from $z=0^-$ is simply a ground plane translated by a distance $l$, which provides an inductive input reactance (see Fig. 2b)
\begin{equation}\label{Yshort}
Y_{sub}^{TX}=-jY_{s0}^{TX}\cot(k_{s0z}^{TX}l),
\end{equation}
where ``X" is either ``E" for TE polarized waves or ``M" for TM polarized waves. The capacitance modulation $C^{TX}(t)$ over one stixel is assumed to be a periodic function of time, 
\begin{equation}\label{CapFun}
C^{TX}(t)=C_0^{TX}+\Delta C^{TX}(t).
\end{equation}
where $C_0^{TX}$ is static capacitance designed to resonate with the inductive reactance given by (\ref{Yshort}) at frequency $f_0$ for each polarization. It is given by
\begin{equation}\label{Cap_0}
C_0^{TX}=\frac{Y_{s0}^{TX}\cot(k_{s0z}^{TX}l)}{\omega_0}.  
\end{equation}
Since $Y_{sub}^{TX}$ resonates with $C_0^{TX}$ at frequency $f_0$, the reflection phase $\phi(t)$ at the incident frequency is fully controlled by $\Delta C^{TX}(t)$,
% \begin{equation}\label{RefPhase}
% \phi(t)=\arctan \frac{-2\omega_0 Y_{00}^{TX}\Delta C^{TX}(t)}{Y_{00}^{TX}-\omega_0^2\Delta C^{TX}(t)^2}
% \end{equation}
\begin{equation} \label{RefPhase}
\phi \left( t \right) =  - 2\arctan \frac{{{\omega _0}\Delta {C^{TX}}\left( t \right)}}{{Y_{00}^{TX}}},
\end{equation}
where $Y_{00}^{TX}$ is the tangential wave admittance in free space at radial frequency $\omega_0$ for each polarization:
\begin{align}
Y_{00}^{TE}&=\frac{\sqrt{k_0^2-k_x^2}}{\mu_0\omega_0}, \label{Z0TE} \\
Y_{00}^{TM}&=\frac{\epsilon_0\omega_0}{\sqrt{k_0^2-k_x^2}}.
\label{Z0TM} 
\end{align} 
where $k_0$ is the free space wavenumber at radial frequency $\omega_0$, and $k_x$ is the tangential wavenumber of the incident wave.
In this paper, the reflection phase of each column of the stixels is either a sawtooth ($\phi(t)=\omega_p t$), or a sinusoidal function ($\phi(t)=A_0\sin(\omega_p t)$) in time; where $\omega_p$ is the radial frequency of the modulation. From Eq. \ref{RefPhase}, the capacitance $\Delta C^{TX}(t)$ can be found for a desired time-varying phase $\phi(t)$
% \begin{equation}\label{Cap_D}
%   \Delta C^{TX}(t) =
%     \begin{cases}
%       \frac{Y_{00}^{TX}(1-\sqrt{1+\tan^2(\phi(t)})}{\omega_0\tan (\phi(t))}, \quad -\frac{\pi}{2}<\phi(t)<\frac{\pi}{2}\\
%       \frac{Y_{00}^{TX}(1+\sqrt{1+\tan^2(\phi(t))})}{\omega_0\tan (\phi(t))}, \quad \text{otherwise}
%     \end{cases}
% \end{equation} 
\begin{equation}\label{Cap_D}
    \Delta {C^{TX}}\left( t \right) =  - \frac{{Y_{00}^{TX}}}{{{\omega _0}}}\tan \left( {\frac{\phi \left( t \right) }{2}} \right) .
\end{equation}
% where $\omega_p$ is the radial frequency of the modulation.
% $Y_{00}^{TX}$ is the tangential wave admittance in free space at radial frequency $\omega_0$ for each polarization:
% \begin{align}
% Y_{00}^{TE}&=\frac{\sqrt{k_0^2-k_x^2}}{\mu_0\omega_0}, \label{Z0TE} \\
% Y_{00}^{TM}&=\frac{\epsilon_0\omega_0}{\sqrt{k_0^2-k_x^2}}.
% \label{Z0TM} 
% \end{align} 
% where $k_0$ is the free space wavenumber at radial frequency $\omega_0$, and $k_x$ is the tangential wavenumber of the incident wave.
The capacitance $C^{TX}(t)$ is a periodic function in time. Therefore, it can be expressed as a Fourier series:
\begin{equation}\label{CapTemporal}
C^{TX}(t)=\sum_{q=-\infty}^{\infty} C_{q}^{TX}e^{jq\omega_p t},  
\end{equation}
where the coefficient $C_q^{TX}$ is equal to
\begin{equation}\label{CapTCoef}
C_q^{TX}=\frac{1}{T_p}\int_{0}^{T_p} C^{TX}(t)e^{-jq\omega_pt} dt.
\end{equation}
This Fourier representation of the capacitance is used to find the fields scattered from each stixel: a time modulated capacitive sheet over a grounded uniaxial dielectric substrate.
%%%%%%%%%%%%%%%%%%%%%%%%%%%%%%%%%%%%%%%%%%%%%%%%%%%%%%%%%%%%%%%%%%%%%%%%%%%%%%%%%%%%%%%%%%%%%%%%%%%%%%%%%

\section{\label{app:Npath} Finding the spatially-discrete, traveling-wave modulated (SD-TWM) sheet capacitance}

A homogenized model of the spatially-discrete, traveling-wave modulated (SD-TWM) metasurface is shown in Fig. 4b. It consists of a SD-TWM capacitive sheet over a grounded dielectric substrate. The spatial modulation period of the capacitive sheet is $d$, and its temporal modulation period is $T_p=2\pi/\omega_p$. Each spatial modulation period is discretized into $N$ paths (stixels of width $d_0$) over which the sheet capacitance is uniform. The space-time capacitance, $C(t,x)$, of the capacitive sheet can be expanded as a 2-D Fourier series:
\begin{equation}\label{CapacitanceMod}
C(t,x)=\sum_{m=-\infty}^{\infty}\sum_{q=-\infty}^{\infty} C_{mq}e^{-jm\beta_p x}e^{jq\omega_p t},
\end{equation}
where $\beta_p=2\pi/d$ is the spatial modulation wavenumber and $\omega_p=2\pi/T_p$ is the radial frequency (temporal modulation wavenumber) of the modulation. The coefficients $C_{mq}$ of the 2-D Fourier series can be calculated as:
\begin{equation}\label{CapSTCoef}
C_{mq}=\frac{1}{dT_p}\int_{0}^{d}\int_{0}^{T_p} C(t,x)e^{jm\beta_px}e^{-jq\omega_pt} dtdx.
\end{equation}

As noted in the main text, the capacitive sheet is assumed to be spatially invariant across a given path. According to Eq. (5), the capacitance modulation of a path is staggered in time by $T_p/N$ with respect to its adjacent path. Therefore, if there are $N$ unit cells in one spatial modulation period $d$ (N-path configuration), the sheet capacitance, of path $\nu$ can be expressed as
\begin{equation}\label{Capv}
   C^v(t,x) =
    \begin{cases}
      C^{TX}(t-(v-1)\frac{T_p}{N}), & \frac{v-1}{N}d<x<\frac{v}{N}d\\ 
      0, & \text{otherwise}
    \end{cases},
\end{equation} 
which is a pulse function in space, and periodic function in time (see Eq. (\ref{CapTemporal})). The spatio-temporally varying sheet capacitance can then be expressed as
\begin{equation}
    C\left( {t,x} \right) = \sum\limits_{v = 1}^{N} {{C^v}\left( {t,x} \right)} .
\end{equation}
The capacitance of path $v$, $C^v(t,x)$, can also be expanded as a 2-D Fourier series,
\begin{equation}\label{CapacitanceModv}
C^v(t,x)=\sum_{m=-\infty}^{\infty}\sum_{q=-\infty}^{\infty} C_{mq}^ve^{-jm\beta_p x}e^{jq\omega_p t},
\end{equation}
where 
\begin{align}\label{CapSTCoefv}
C_{mq}^v&=\frac{1}{dT_p}\int_{0}^{d}\int_{0}^{T_p} C^v(t,x)e^{jm\beta_px}e^{-jq\omega_pt} dtdx \nonumber\\
&=\frac{1}{dT_p}\int_{\frac{v-1}{N}d}^{\frac{v}{N}d}\int_{0}^{T_p}  C^{TX}(t-(v-1)\frac{T_p}{N})e^{jm\beta_px}e^{-jq\omega_pt} dtdx .
\end{align}
The equation above can be used to derive the following relationship between the Fourier coefficients of the sheet capacitance on adjacent paths,
\begin{equation}\label{NpathRelationship}
C_{mq}^v=C_{mq}^{v-1}e^{jm\frac{2\pi}{N}}e^{-jq\frac{2\pi}{N}}.
\end{equation}
The Fourier coefficents of the overall capacitive sheet, $C_{mq}$, given by Eq. (\ref{CapSTCoef}), can be found by summing the capacitance over all the paths and employing Eq. (\ref{NpathRelationship}),
\begin{align}\label{PathSum}
C_{mq}&=\frac{1}{dT_p}\left(\int_{0}^{\frac{d}{N}}\int_{0}^{T_p} C(t,x)e^{jm\beta_px}e^{-jq\omega_pt} dtdx + \ldots \right. \nonumber\\
& \qquad \qquad \left.+\int_{\frac{N-1}{N}d}^{d}\int_{0}^{T_p} C(t,x)e^{jm\beta_px}e^{-jq\omega_pt} dtdx \right) \nonumber\\
&=\frac{1}{dT_p}\left(\int_{0}^{d}\int_{0}^{T_p} C^1(t,x)e^{jm\beta_px}e^{-jq\omega_pt} dtdx + \ldots \right. \nonumber\\
& \qquad \qquad \left.+\int_{0}^{d}\int_{0}^{T_p} C^N(t,x)e^{jm\beta_px}e^{-jq\omega_pt} dtdx \right) \nonumber\\
&=\sum_{v=1}^{N}C_{mq}^v=\sum_{v=1}^{N}C_{mq}^1e^{j\frac{2\pi}{N}(m-q)(v-1)}.
\end{align}
It is clear from Eq. (\ref{PathSum}) that the coefficient $C_{mq}$ is zero except when 
\begin{equation}\label{ModeRelation0}
m-q=rN,\quad \text{where}\quad r\in \mathbb{Z}.
\end{equation}
% $m-q$ is an integer multiple of $N$ ($m-q=0,\pm N, \pm 2N, \pm 3N, \ldots$). 
Therefore,
\begin{equation}\label{NoneZero}
   C_{mq} =
    \begin{cases}
      NC_{mq}^1, & m-q=rN, \text{where}\quad r\in \mathbb{Z}\\ 
      0, & \text{otherwise}
    \end{cases}.
\end{equation} 
Given the staggered modulation of the paths (stixels), the metasurface functions as an N-path system \cite{cody_meta}, and the indices $m$ and $q$ are related by Eq. (\ref{ModeRelation0}).  
%as follows,
%\begin{equation}\label{ModeRelation}
%m-q=rN,\quad \text{where}\quad r\in \mathbb{Z}
%\end{equation}
Inserting Eq. (\ref{ModeRelation0}) into Eq. (\ref{CapacitanceMod}), the sheet capacitance can be rewritten as,
\begin{align}\label{CapMod}
C(t,x)&=\sum_{r=-\infty}^{\infty}\sum_{q=-\infty}^{\infty} C_{q+rN,q}e^{-j(q+rN)\beta_p x}e^{jq\omega_p t}\nonumber\\
&   {\buildrel \Delta \over =}  \sum_{r=-\infty}^{\infty}\sum_{q=-\infty}^{\infty} C_{rq}e^{jq(\omega_p t-\beta_px)}e^{-jr\beta_d x},
\end{align}
where the wavenumber $\beta_d=N\beta_p=2\pi/d_0$ is an additional wavenumber resulting from the discretization of the spatial modulation. The summation over $r$ accounts for the discontinuity in capacitance at the the boundary of each path as well as the microscopic spatial variation of capacitance within the paths (which in this case is uniform). The summation over $q$ accounts for the macroscopic capacitance variation over one spatial modulation period $d$.
% Observing the capacitance over a single path, it can be concluded that the staggered modulation between paths impresses a tangential wavenumber of $q \beta_p$ onto the $q^{th}$ harmonic.

Given Eq. (\ref{NoneZero}), the spatio-temporal coefficients of the capacitance variation are given by
\begin{align}\label{CapCoNpath}
C_{rq} &=\frac{1}{dT_p}\int_{0}^{d}\int_{0}^{T_p} C(t,x)e^{j(q+rN)\beta_px}e^{-jq\omega_pt} dtdx \nonumber\\
&=NC_{rq}^1\nonumber\\
&=\frac{N}{dT_p}\int_{0}^{d/N}\int_{0}^{T_p} C^{TX}(t)e^{j(q+rN)\beta_px}e^{-jq\omega_pt} dtdx \nonumber\\
&=\frac{N}{dT_p}\int_{0}^{d/N}\int_{0}^{T_p} C^{TX}(t)e^{-jq(\omega_p t-\beta_px)}e^{jr\beta_d x} dtdx.
\end{align} 
Inserting Eq. (\ref{CapTCoef}) into Eq. (\ref{CapCoNpath}), we obtain
\begin{align}\label{CapCoNpathF}
C_{rq}
&=\frac{N}{dT_p}\int_{0}^{\frac{d}{N}}e^{j(q+rN)\beta_px} dx \int_{0}^{T_p} C^{TX}(t)e^{-jq\omega_pt} dt \nonumber \\
&=e^{j \frac{\pi(q+rN)}{N}}\text{sinc}\frac{\pi(q+rN)}{N}C_q^{TX},
\end{align} 
where $C_q^{TX}$ are the temporal coefficients of the capacitance modulation for a single path, given by Eq. (\ref{CapTCoef}).

\section{\label{app:SpaceTimeModeCal} Calculation of the reflected spectrum from a SD-TWM metasurface}

As a result of the symmetry introduced by the staggered modulation scheme, the tangential field above the metasurface satisfies the interpath relation \cite{cody_meta}.
\begin{equation}\label{NpathRelationshipE}
E_t(t,x)=e^{j(\frac{\omega_0T_p}{N}-\frac{k_xd}{N})}E_t(t-\frac{T_p}{N},x-\frac{d}{N})
\end{equation}
This space-time field distribution on the surface can also be expressed in terms of a 2-D Floquet expansion:
\begin{equation}\label{FieldMod}
E_t(t,x) =E_t|_{z=0^+}=E_t|_{z=0^-}=\sum_{m=-\infty}^{\infty}\sum_{q=-\infty}^{\infty} V_{mq}e^{-jm\beta_p x}e^{jq\omega_p t}e^{j(\omega_0t-k_xx)}.
\end{equation}
Substituting  (\ref{FieldMod}) into (\ref{NpathRelationshipE}), one again finds that (\ref{ModeRelation0}) must hold. As a result,
\begin{align}
E_t(t,x) &=\sum_{r=-\infty}^{\infty}\sum_{q=-\infty}^{\infty} V_{(q+rN) q}e^{-j(q+rN)\beta_p x}e^{jq\omega_p t}e^{j(\omega_0t-k_xx)}\nonumber\\
\label{FieldMod3}
 &{\buildrel \Delta \over =}\sum_{r=-\infty}^{\infty}\sum_{q=-\infty}^{\infty} V_{r q}e^{-jr\beta_d x}e^{jq(\omega_p t-\beta_p x)}e^{j(\omega_0t-k_xx)},
\end{align}
where the wavenumber $\beta_d=N\beta_p=2\pi/d_0$ results from the spatial discretization of the modulation. The summation over $r$ accounts for the microscopic field variation along each path (unit cell size of length $d_0=d/N$). The summation over $q$ accounts for the macroscopic field variation over one spatial modulation period $d$. Observing the field expression in Eq. (\ref{FieldMod3}), it can be concluded that the macroscopic variation (travelling-wave modulation) impresses a tangential wavenumber of $q \beta_p$ onto the $q^{th}$ harmonic. 
The total tangential magnetic field on the spatio-temporally modulated metasurface (see Fig. 3) can be expressed as,
\begin{align}
H_t|_{z=0^+}&=\sum_{r,q=-\infty}^{\infty} I_{rq}e^{-jr\beta_dx}e^{jq(\omega_p t-\beta_p x)}e^{j(\omega_0 t-k_{x} x)} \label{HSTTotal1} \\
H_t|_{z=0^-}&=\sum_{r,q=-\infty}^{\infty} -jV_{rq} Y_{srq}^{TX}\cot(k_{srqz}^{TX}l)e^{-jr\beta_dx}e^{jq(\omega_p t-\beta_p x)}e^{j(\omega_0 t-k_{x} x)}.
\label{HSTTotal2} 
\end{align}
$Y_{srq}^{TX}$ and $k_{srqz}^{TX}$ are the tangential wave admittance and normal wavenumber in the substrate for each spatio-temporal harmonic pair $(r,q)$,
\begin{align}\label{Zrqsub} 
Y_{srq}^{TE}=\frac{k_{srqz}^{TE}}{\mu_0\omega_{rq}},\quad
Y_{srq}^{TM}=\frac{\epsilon_0\epsilon_h\omega_{rq}}{k_{srqz}^{TM}},
\end{align}
\begin{align}\label{Krqsub}
k_{srqz}^{TE}=\sqrt{\frac{\omega_{rq}^2}{c^2}\epsilon_h-k_{xrq}^2},\quad
k_{srqz}^{TM}=\sqrt{\frac{\omega_{rq}^2}{c^2}\epsilon_h-k_{xrq}^2\frac{\epsilon_h}{\epsilon_{zz}}},
\end{align}
where $s$, $r$, $q$, and $z$ denote the substrate, harmonic pair $(r,q)$, and z-component of the wavenumber. $k_{xrq}=k_x+q\beta_p+r\beta_d$ is the tangential wavenumber of the the harmonic pair $(r,q)$. 

If the magnitude of the voltage signal that modulates the varactors comprising the stixel is much larger than the incident signal at $f_0$, the sheet impedance over one stixel can be treated as a linear, time-varying capacitance. Therefore, the boundary condition \cite{Collin} at $z=0$ is given by
\begin{equation}\label{BoundaryT}
H_t|_{z=0^+}-H_t|_{z=0^-}=\frac{d}{dt}(C^{TX}(t,x)E_t).
\end{equation}
Inserting Eqs. (\ref{CapMod}), (\ref{FieldMod3}), (\ref{HSTTotal1}) and (\ref{HSTTotal2}) into the boundary condition given by Eq. (\ref{BoundaryT}) yields
\begin{align}\label{BoundaryST}
I_{rq}=j(q\omega_p+\omega_0)\sum_{r',q'=-M}^M C^{TX}_{r-r',q-q'}V_{r'q'} -jV_{rq} Y_{srq}^{TX}\cot(k_{srqz}^{TX}l), 
\end{align}

 \begin{table}[t]
 \caption{\label{tab:ModeRelation}%
Harmonic mapping relationship used in the analysis} 
 \begin{tabular}{>{\centering\arraybackslash}p{0.3\columnwidth} >{\centering\arraybackslash}p{0.3\columnwidth}>{\centering\arraybackslash}p{0.33\columnwidth}}
 \toprule
  $r$ &$q$&$\alpha$\\
\hline
 $-M$&$-M$&1\\
 $-M$&$-M+1$&2\\
 $\vdots$ & $\vdots$&$\vdots$\\
 $-M$&$M$&$2M+1$\\
 $-M+1$&$-M$&$2M+2$\\
 $-M+1$&$-M+1$&$2M+3$\\
 $\vdots$ & $\vdots$&$\vdots$\\
 $M$&$M$&$(2M+1)^2$\\
  \bottomrule
 \end{tabular}
 \end{table}

In order to simplify the calculation, each harmonic pair $(r,q)$ is mapped to one harmonic index $\alpha=(r+M)(2M+1)+q+1$ \cite{Tsang}, as shown in Table \ref{tab:ModeRelation}. The harmonic mapping allows the tangential fields, given by Eqs. (\ref{FieldMod3}) and (\ref{HSTTotal1}), to be represented as vectors $\bm{V^{TX}}$ and $\bm{I^{TX}}$, where each contains $(2M+1)^2$ entries: $V_\alpha$ and $I_\alpha$ respectively. The boundary condition given by Eqs. (\ref{BoundaryST}) can then be written in matrix form. 
\begin{equation}\label{BoundaryMT}
\bm{I^{TX}}=\bm{Y^{TX}V^{TX}},
\end{equation} 
The size of metasurface input admittance matrix $\bm{Y^{TX}}$ is $(2M+1)^2\times(2M+1)^2$, which contains entries:
\begin{align}\label{Yspatetime}
Y_{\alpha \alpha'}^{TX}=j\omega_\alpha C_{\alpha-\alpha'}^{TX}-j\delta(\alpha-\alpha')Y_{s\alpha}^{TX}\cot(k_{sz\alpha}^{TX}l).
\end{align}
We can separate the total tangential field into incident and reflected tangential fields, 
\begin{equation} \label{ESPInc}
E_t^{\rm{inc}}=V_{00}^{\rm{inc}}e^{j(\omega_0 t-k_{x} x)},
\end{equation}
\begin{equation} \label{ESPRef}
E_t^{\rm{ref}}=\sum_{r,q=-M}^{M} V_{rq}^{\rm{ref}}e^{-jr\beta_dx}e^{jq(\omega_p t-\beta_p x)}e^{j(\omega_0 t-k_{x} x)},
\end{equation}
\begin{equation} \label{HSPInc}
H_t^{\rm{inc}}=I_{00}^{\rm{inc}}e^{j(\omega_0 t-k_{x} x)},
\end{equation}
\begin{equation} \label{HSPRef}
H_t^{\rm{ref}}=\sum_{r,q=-M}^{M} I_{rq}^{\rm{ref}}e^{-jr\beta_dx}e^{jq(\omega_p t-\beta_p x)}e^{j(\omega_0 t-k_{x} x)}. 
\end{equation}
The coefficients of the incident and reflected fields, are related by the free-space tangential admittance:
\begin{equation}\label{FTM}
\bm{I^{\rm{inc}}}=\bm{Y_0^{TX}V^{\rm{inc}}},\quad \bm{I^{\rm{ref}}}=-\bm{Y_0^{TX}V^{\rm{ref}}}.
\end{equation}
For each polarization, the diagonal admittance matrix $\bm{Y_0^{TX}}$ contains entries
\begin{align}
Y_{0\alpha \alpha'}^{TE}&=\frac{\delta(\alpha-\alpha')\sqrt{\omega_\alpha^2/c^2-k_{x\alpha}^2}}{\mu_0\omega_\alpha}, \label{Y0TE} \\
Y_{0\alpha \alpha'}^{TM}&=\frac{\delta(\alpha-\alpha')\epsilon_0\omega_\alpha}{\sqrt{\omega_\alpha^2/c^2-k_{x\alpha}^2}}.
\label{Y0TM} 
\end{align}
From Eq. (\ref{BoundaryMT}) and (\ref{FTM}), the reflected electric field can be calculated for each polarization,
\begin{align}\label{TemporalRefCalTE}
\bm{V^{\rm{ref}}}=&\bm{(Y^{TX}+Y_0^{TX} )^{-1}}\bm{(Y_0^{TX}-Y^{TX} ) V^{\rm{inc}}},
\end{align} 

%%%%%%%%%%%%%%%%%%%%%%%%%%%%%%%%%%%%%%%%%%%%%%%%%%
%%%%%%%%%%%%%%%%%%%%%%%%%%%%%%%%%%%%%%%%%%%%%%%%%%
%%%%%%%%%% Section 4
%%%%%%%%%%%%%%%%%%%%%%%%%%%%%%%%%%%%%%%%%%%%%%%%%%
%%%%%%%%%%%%%%%%%%%%%%%%%%%%%%%%%%%%%%%%%%%%%%%%%%


\section{Theoretical study of the spatio-temporally modulated metasurface for a high modulation frequency}

\begin{figure}[t!]
\subfloat[\label{sfig:TE25High}]{%
  \includegraphics[clip,width=0.25\columnwidth]{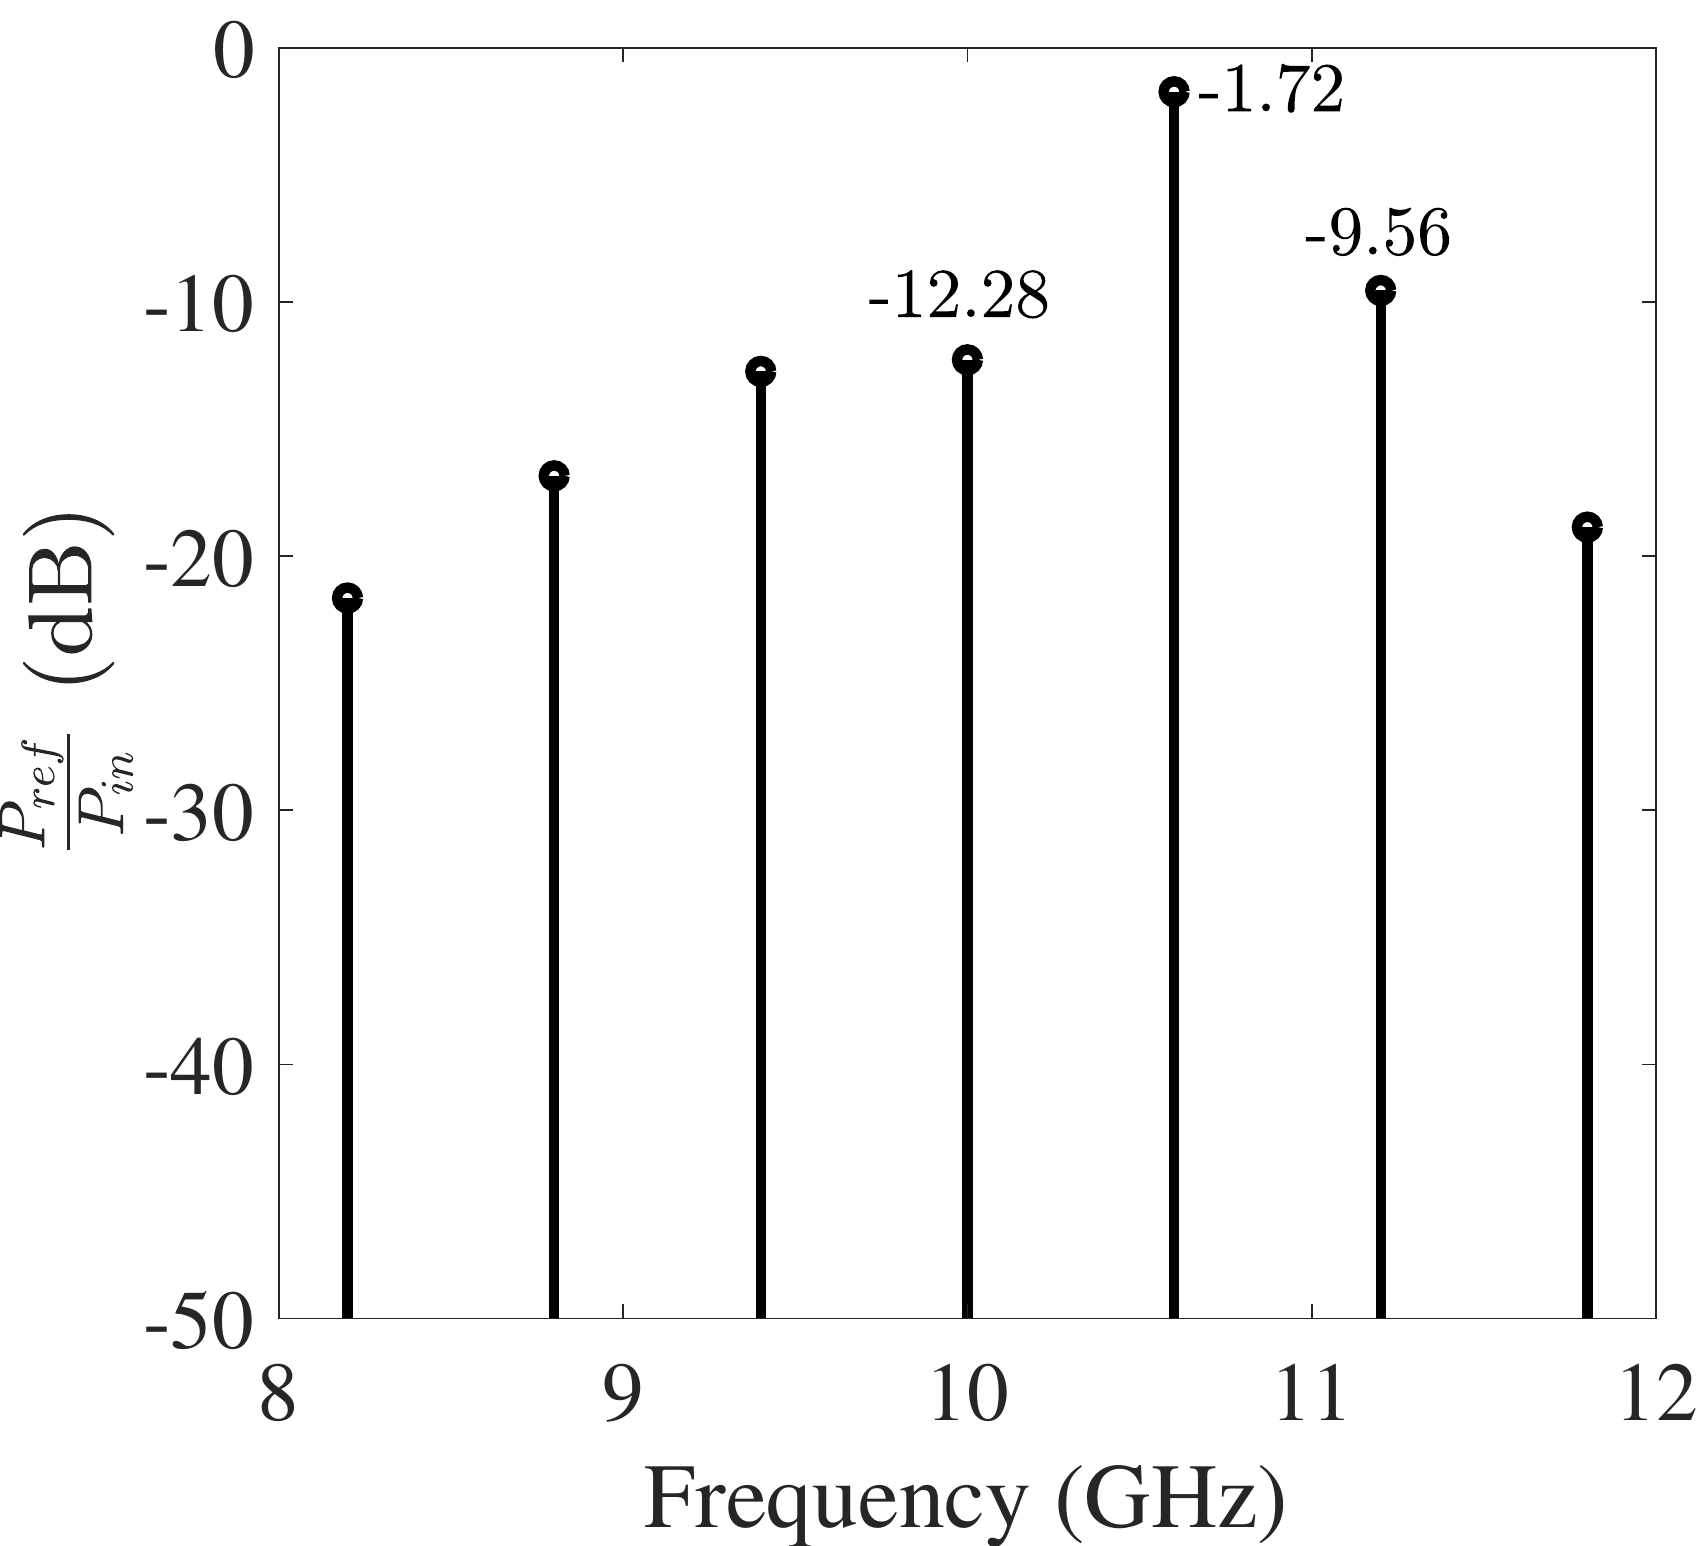}%
}\hfill
\subfloat[\label{sfig:TM25High}]{%
  \includegraphics[clip,width=0.25\columnwidth]{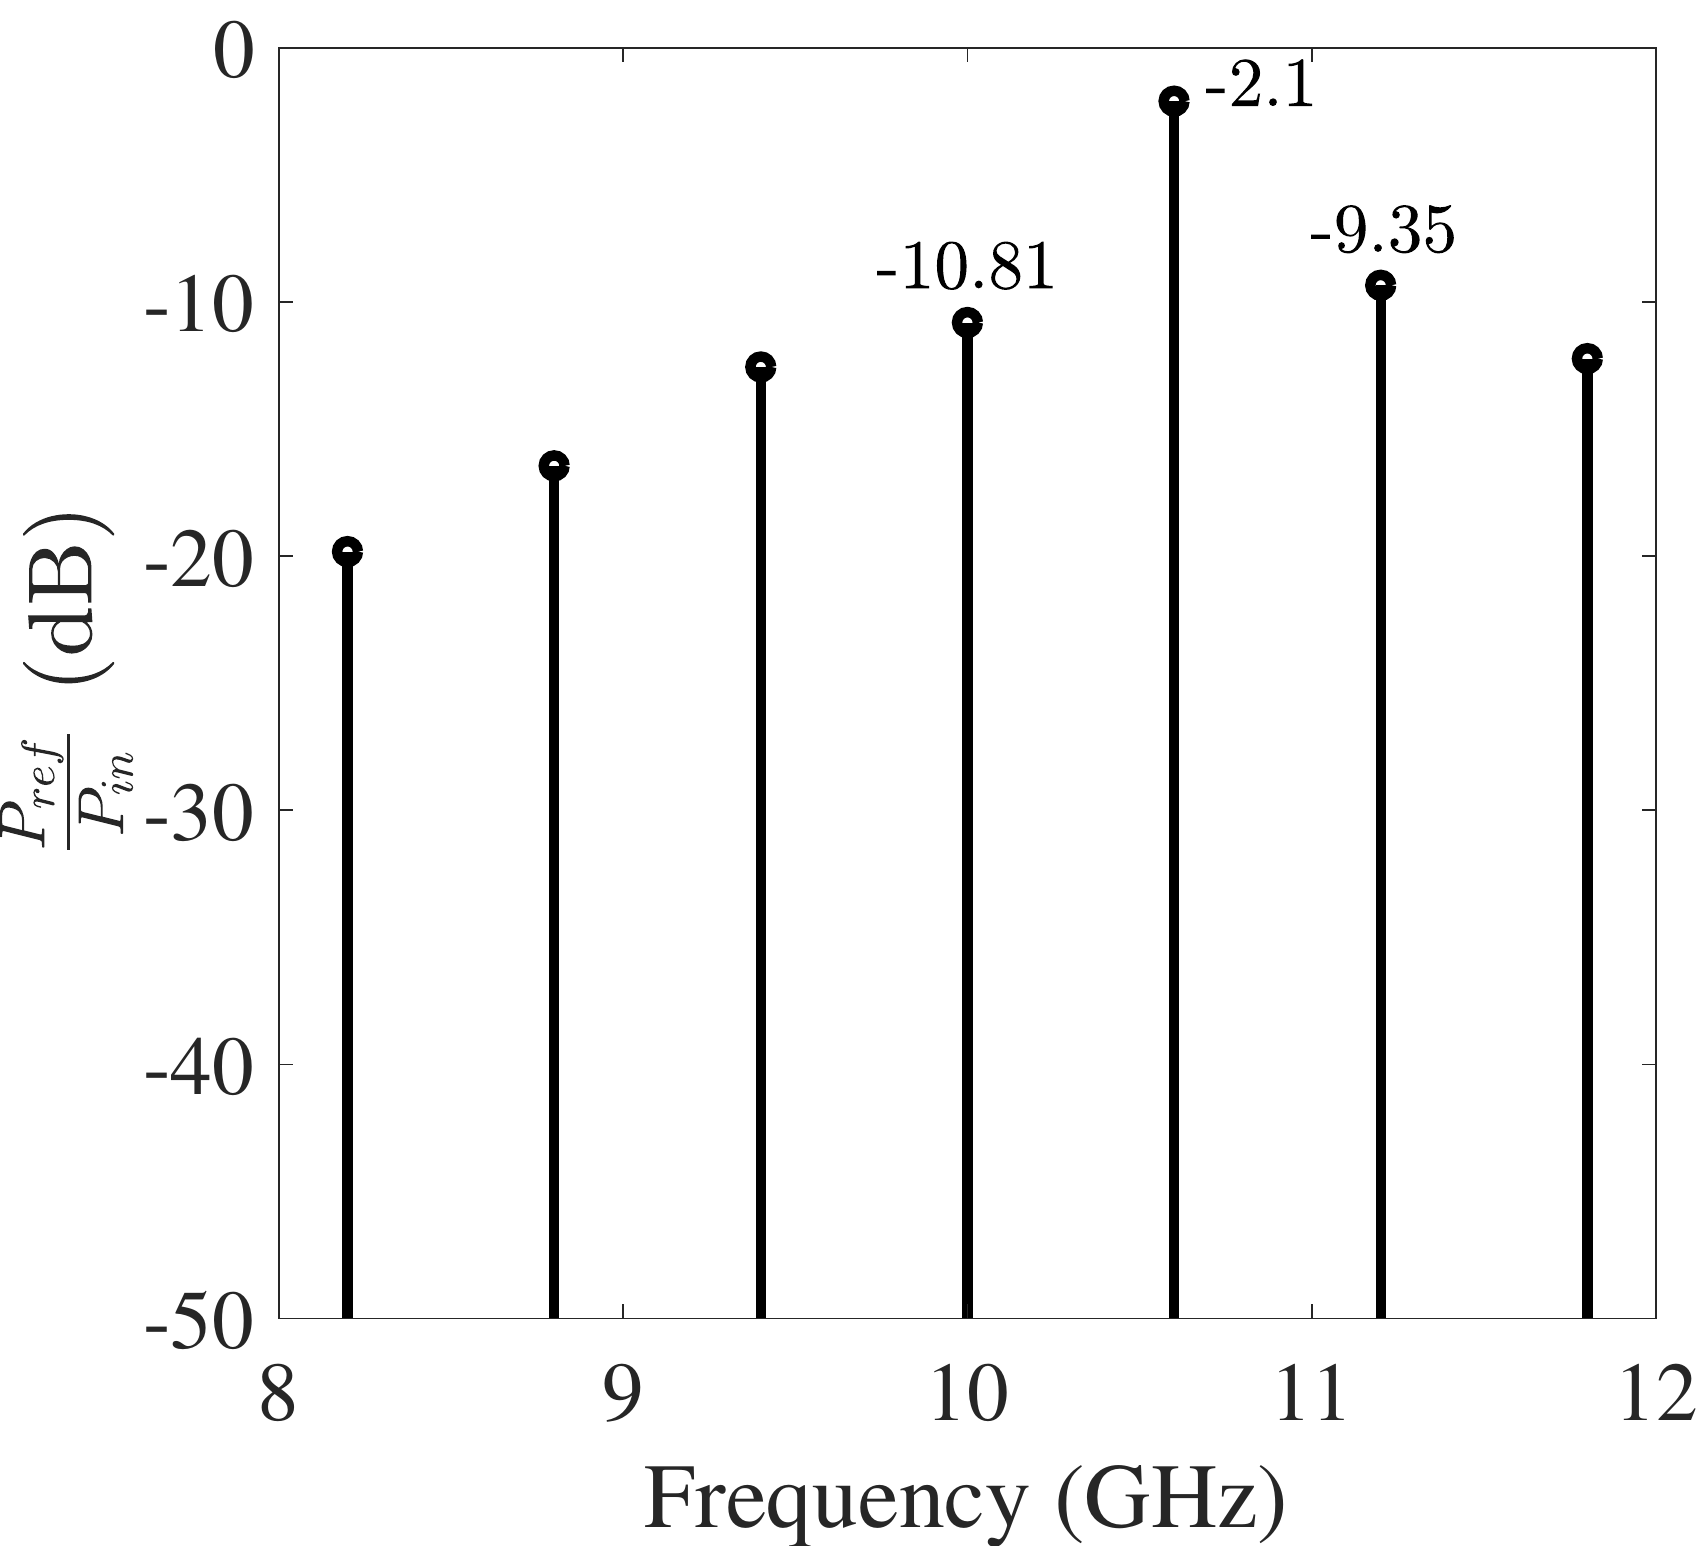}%
}\hfill
\subfloat[\label{sfig:TEN39High}]{%
  \includegraphics[clip,width=0.25\columnwidth]{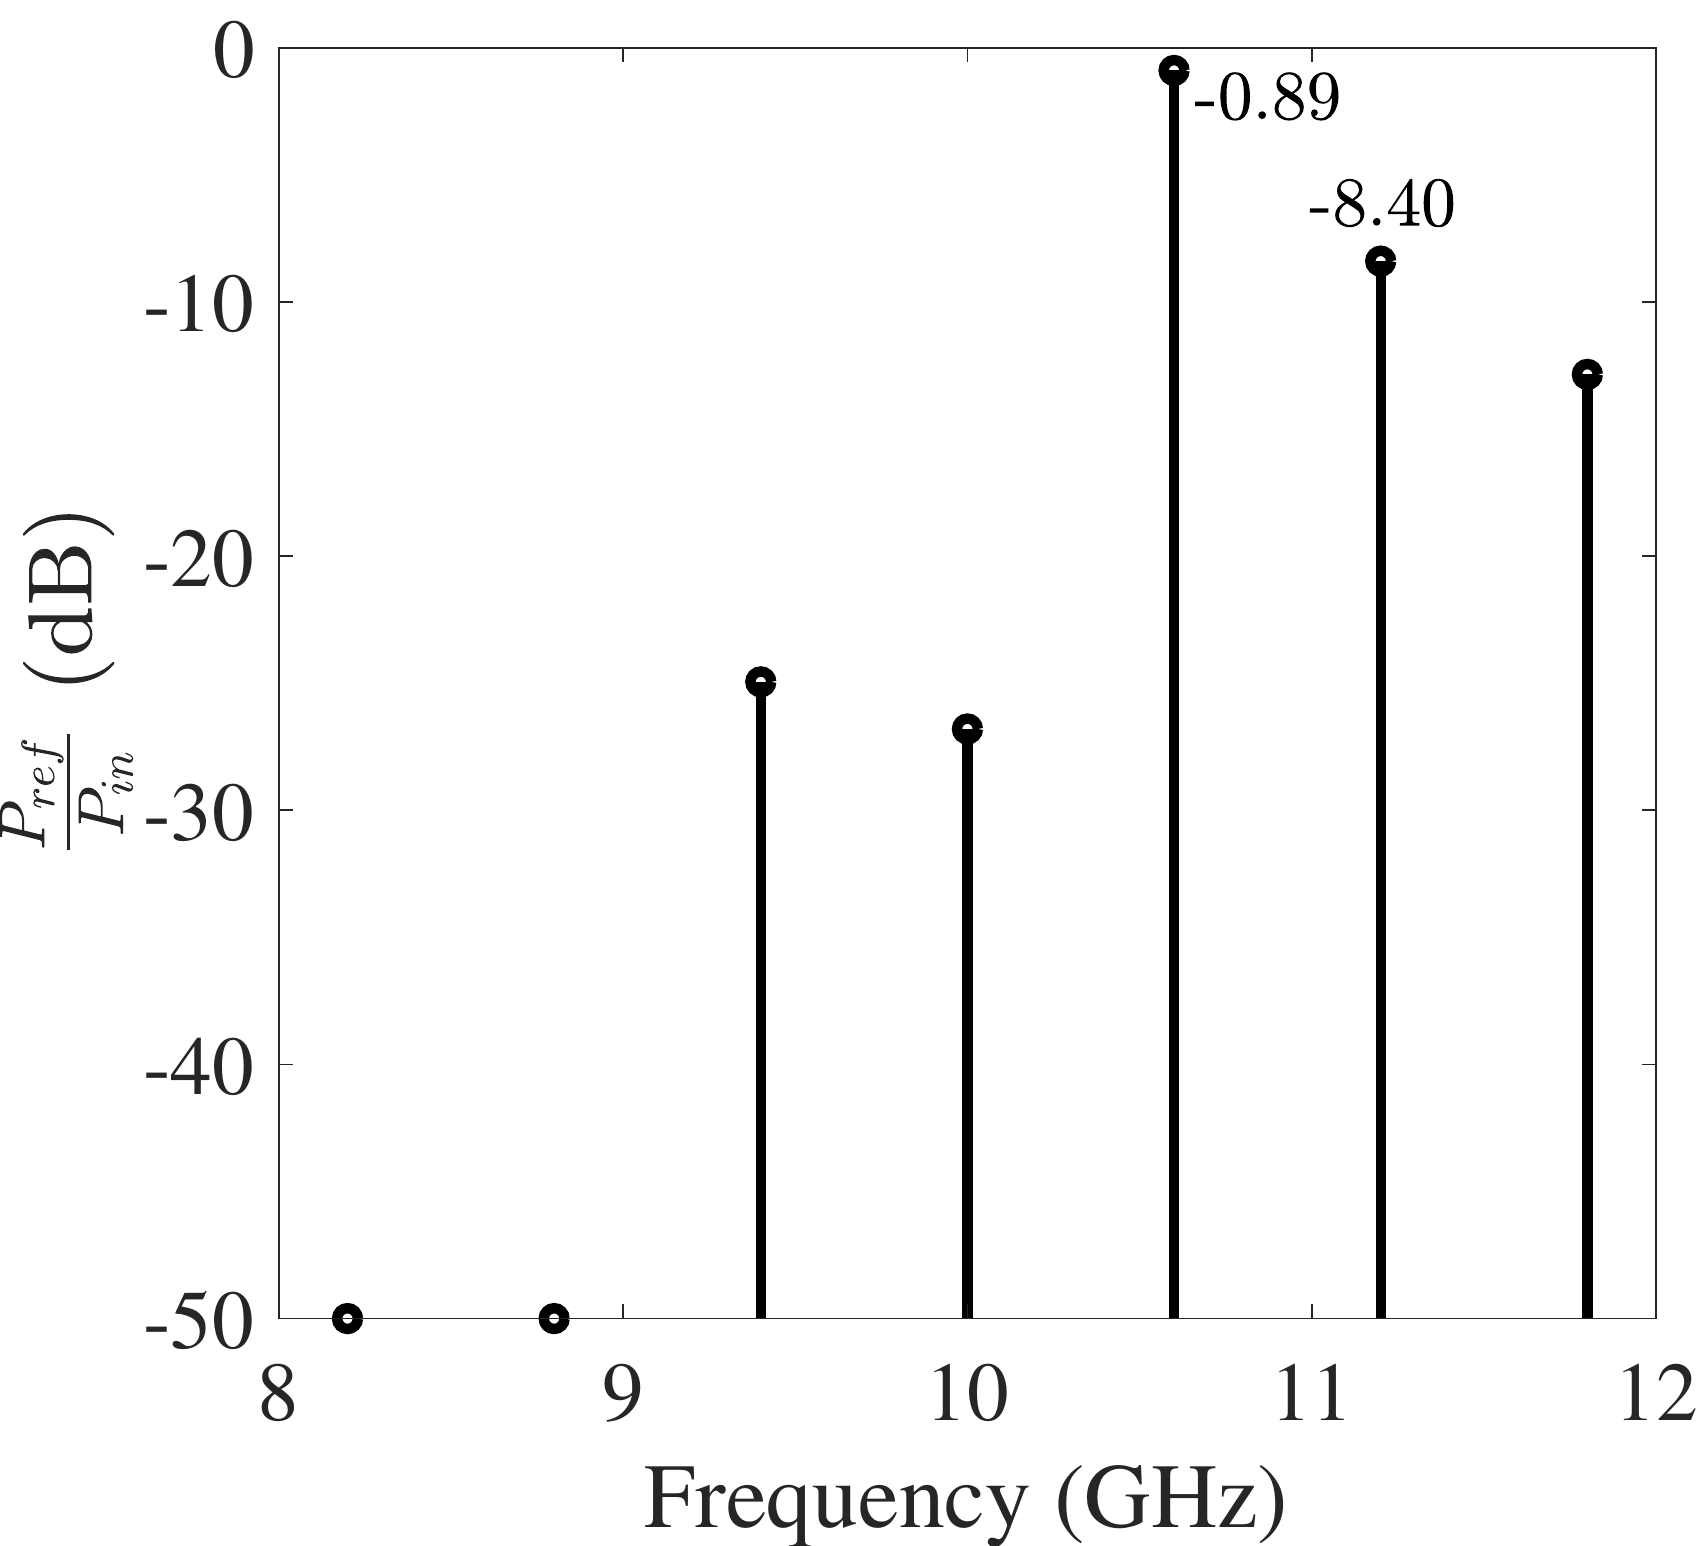}%
}\hfill
\subfloat[\label{sfig:TMN39High}]{%
  \includegraphics[clip,width=0.25\columnwidth]{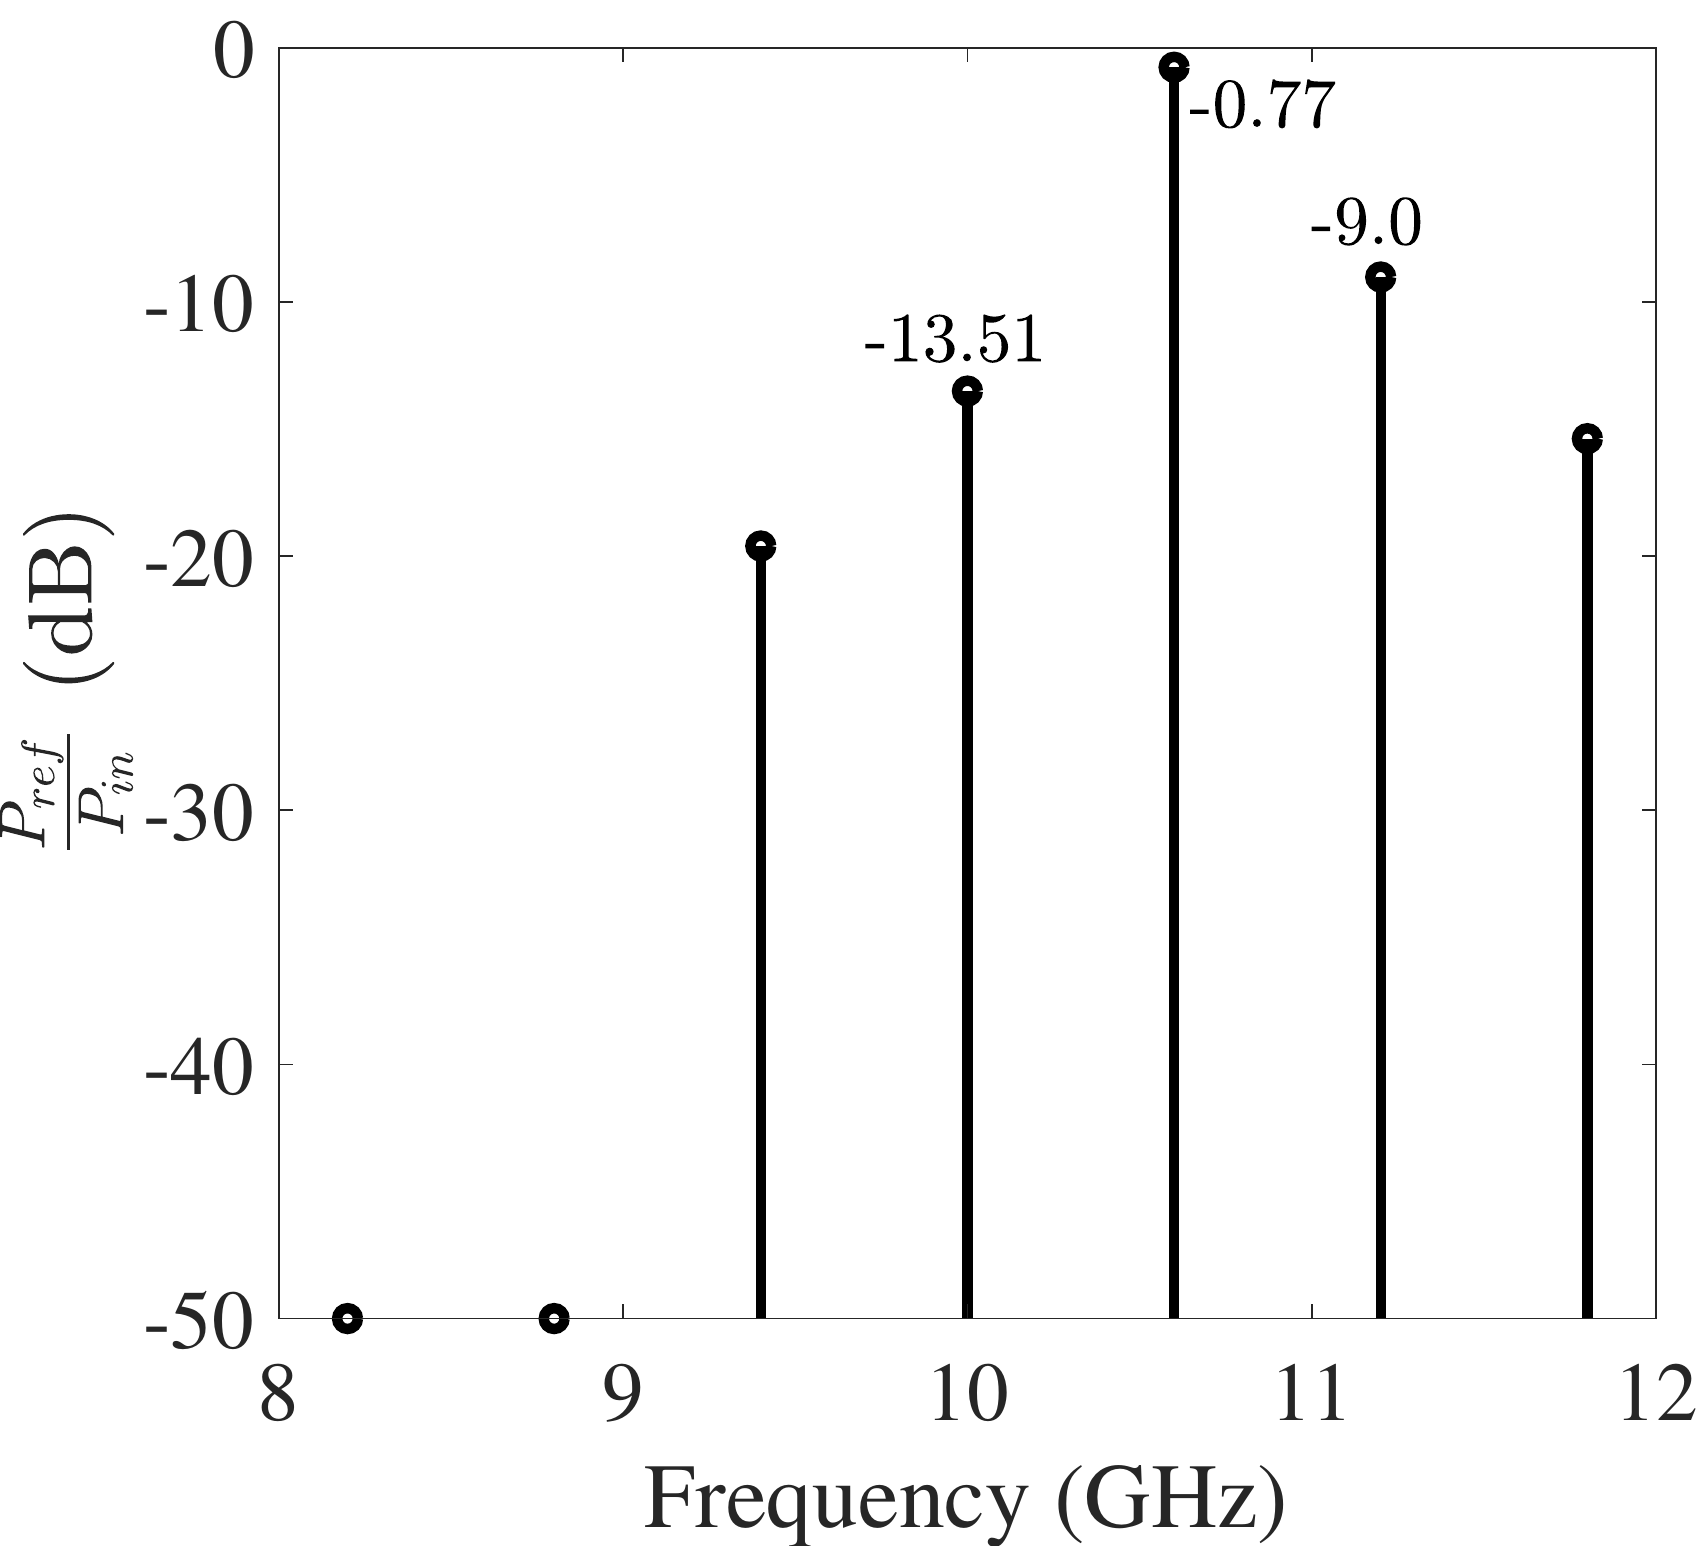}%
}\quad
\caption{Analytical  reflection  spectrum  of  the  homogenized, lossless SD-TWM metasurface modulated at $f_p=0.6$ GHz. (a) 20-path ($N=20$) modulation for TE polarization, for an incident angle of $25^\circ$. (b) 20-path ($N=20$) modulation for TM polarization, for an incident angle of $25^\circ$. (c) 20-path ($N=20$) modulation for TE polarization, for an incident angle of $-39^\circ$. (d) 20-path ($N=20$) modulation for TM polarization, for an incident angle of $-39^\circ$.}
\label{fig:HighFreq}
\end{figure} 

In this section, we study the SD-TWM metasurface under a modulation frequency $f_p$ that is comparable to the incident frequency $f_0$.
The metasurface is modulated at a frequency $f_p=0.6$ GHz with $N=20$ paths included per spatial period. The incident plane wave is assumed to at a frequency $f_0=10$ GHz and is obliquely incident at an angle of $\theta_1 = 25^\circ$.
%The modulation frequency is chosen to be $f_p=0.6$ GHz and the incident frequency is $f_0=10$ GHz. The incident plane wave is obliquely incident at $\theta_1 = 25^\circ$, and $20$ paths per modulation period are chosen.
The reflection phase of each column is a sawtooth function in time. For both polarizations, the field is expanded into 141 frequency harmonics as well as spatial harmonics.  The temporal capacitance modulation on each path is truncated to 101 frequency harmonics.

Based on Eq. (20), the harmonics inside the light cone are those with $q=0,\pm 1, \pm 2, \pm 3, -4$. Based on Eq. (12), the harmonic of interest ($f_0+f_p$) reflects at an angle of $\theta_2=39^\circ$. The reflected TE and TM spectra are given in Fig. \ref{sfig:TE25High} and Fig. \ref{sfig:TM25High}, respectively. For TE polarization, a $1.72$ dB conversion loss and $7.84$ dB sideband suppression are observed. For TM polarization, a $2.1$ dB conversion loss and $7.25$ dB sideband suppression are observed.

When the incident signal impinges on the metasurface at $\theta_2=-39^\circ$, the propagating reflected harmonics are those with $q=0,\pm 1, 2,3,4, 5, 6, 7, 8$. The harmonic of interest ($f_0+f_p$) travels with a reflection angle of $\theta_3=-21^\circ$. Note that the reflected angle $\theta_3\neq\theta_1$, indicating non-reciprocal response of the spatio-temporally modulated metasurface \cite{Shaltout}. Therefore, for a fixed transmitter and receiver position, the metasurface supports uni-directional transmission. The reflected spectrum for TE and TM polarization is given in Fig. \ref{sfig:TEN39High} and Fig. \ref{sfig:TMN39High}, respectively. For TE polarization, a $0.89$ dB conversion loss and $7.51$ dB sideband suppression are observed. For TM polarization, a $0.77$ dB conversion loss and $8.23$ dB sideband suppression are observed.

%%%%%%%%%%%%%%%%%%%%%%%%%%%%%%%%%%%%%%%%%%%%%%%%%%
%%%%%%%%%%%%%%%%%%%%%%%%%%%%%%%%%%%%%%%%%%%%%%%%%%
%%%%%%%%%% Section 6
%%%%%%%%%%%%%%%%%%%%%%%%%%%%%%%%%%%%%%%%%%%%%%%%%%
%%%%%%%%%%%%%%%%%%%%%%%%%%%%%%%%%%%%%%%%%%%%%%%%%%

\section{Reflection from a DC biased unit cell for an incident angle of $25^\circ$}

As described in the paper, the tunability of the metasurface is provided by surface-mounted varactor diodes MAVR-000120-1411. In the full-wave simulations, the varactor diode is modeled as a lumped capacitance in series with a resistance. The capacitance and resistance values are extracted as a function of bias voltage from the varactor's SPICE model \cite{MACOM}. The simulated reflection coefficient of the unit cell for various capacitance values  is shown in Fig. 24 for an incident angle of $25^\circ$. In addition, the reflection coefficient of the fabricated metasurface is measured for various bias voltages for the same angle of incidence, and is shown in Fig. 25. Comparing the simulated and measured reflection coefficients, we noticed that the varactor capacitance versus bias voltage characteristic given by the SPICE model did not accurately match the experimental results. Therefore,
the varactor capacitance versus experimental bias voltage characteristic was obtained by aligning the measured reflection phase to simulation. In addition, the measured reflection amplitude indicated that there was higher loss in measurement than in simulation. The additional loss can be introduced by a higher measured  varactor resistance or by the tinning and soldering processes used to mount the varactor diodes.

\begin{figure}[b!]
\subfloat[\label{sfig:ExtractCircuitTE}]{%
  \includegraphics[clip,width=0.46\columnwidth]{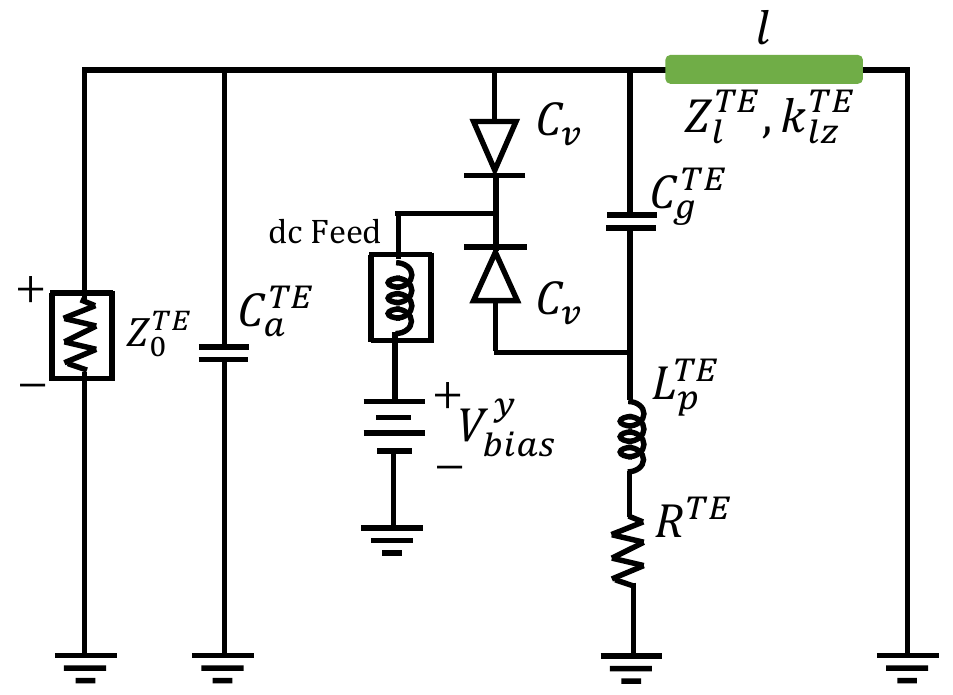}%
}\hfill
\subfloat[\label{sfig:ExtractCircuitTM}]{%
  \includegraphics[clip,width=0.54\columnwidth]{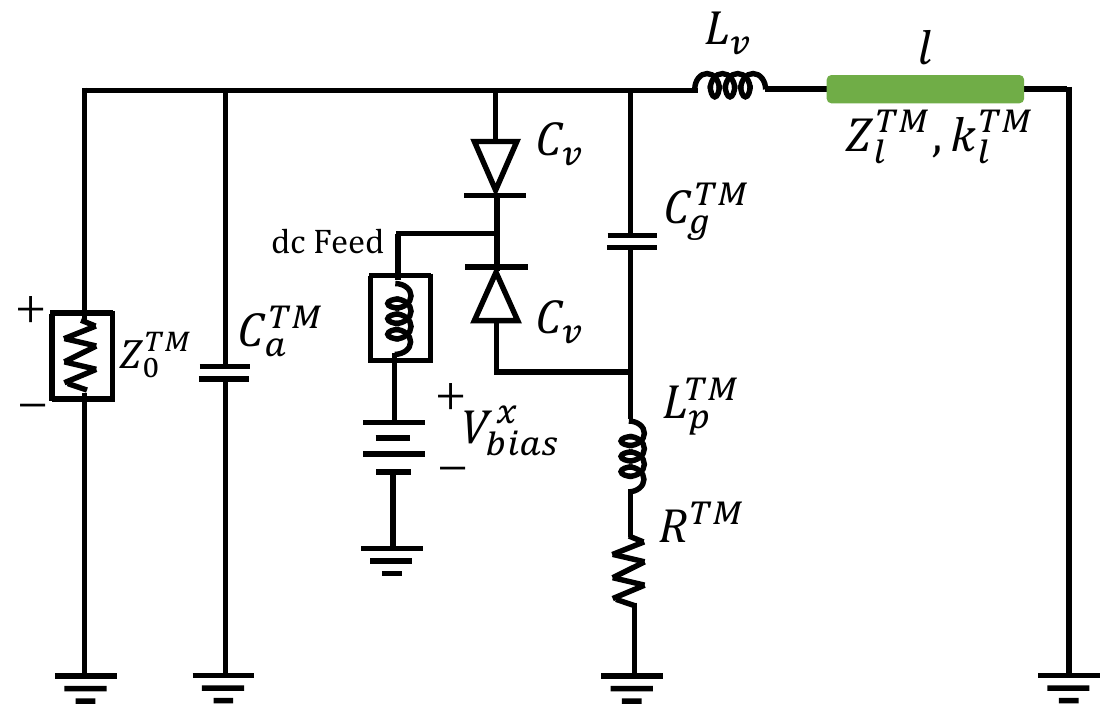}%
}\quad
\caption{Extracted circuit models for for a unit cell (see Fig. 2a)  of the metasurface under an oblique incident angle of $25^\circ$. (a) TE polarization. (b) TM polarization.}
\label{fig:ExtractCircuit}
\end{figure} 

\begin{table}[t!]
  \centering
  \caption{Detailed information an values of the extracted circuit shown in Fig. \ref{fig:ExtractCircuit}}
  \label{tab:CircuitParam}
  \renewcommand{\arraystretch}{1.5}% Spread rows out...
  \begin{tabular}{>{\centering\bfseries}p{0.02\columnwidth} >{\centering}p{0.42\columnwidth} >{\centering}p{0.02\columnwidth} >{\centering\arraybackslash}p{0.42\columnwidth}}
    \toprule
    $Z_0^{TE}$ &Free space tangential wave impedance (TE) under the oblique angle of $25^\circ$, $415.97\ \Omega$ &$Z_0^{TM}$&Free space tangential wave impedance (TM) under the oblique angle of $25^\circ$, $341.68\ \Omega$ \\
    $Z_h^{TE}$&Substrate tangential wave impedance (TE) under the oblique angle of $25^\circ$, $220.77\ \Omega$&$Z_h^{TM}$&Substrate tangential wave impedance (TM) under the oblique angle of $25^\circ$, $181.34\ \Omega$ \\
     $C_g^{TE}$& Extracted pattern capacitance, $0.0325$ pF & $C_g^{TM}$& Extracted pattern capacitance, $0.046$ pF \\
    $C_a^{TE}$& Extracted pattern capacitance, $0.02$ pF & $C_a^{TM}$& Extracted pattern capacitance, $0.03$ pF \\
    $L_p^{TE}$& Extracted pattern inductance, $0.67$ nH & $L_p^{TM}$& Extracted pattern inductance, $0.61$ nH \\
    $R^{TE}$& Extracted voltage-dependent resistance  & $R^{TM}$& Extracted voltage-dependent resistance \\
    $k_{hz}^{TX}$& Substrate normal wavenumber for TE or TM, electric thickness $k_{hz}^{TX}l=10.411^\circ$ & $L_v$& Extracted series inductance of the vias, $0.11$ nH \\
    $l$& Substrate thckness, $0.508$ mm & $C_d$& Varactor diode SPICE model \\
    \bottomrule
  \end{tabular}
\end{table}

\begin{table}[t!]
\caption{\label{tab:DiodeTE}%
Varactor (MAVR-000120-1411) capacitance and resistance verses bias voltage characteristic for TE polarization.} 
\begin{tabular}{>{\centering\arraybackslash}p{0.25\columnwidth}>{\centering\arraybackslash}p{0.2\columnwidth} >{\centering\arraybackslash}p{0.2\columnwidth}>{\centering\arraybackslash}p{0.25\columnwidth}}
 \toprule
 Varactor capacitance (pF) &Additional loss $R^{TE}$ in circuit simulation ($\Omega$)&Bias voltage used in circuit simulation (V)& Bias voltage used in measurement (V)\\
  \hline
0.4&2.08&4.03&4\\
0.329&1.82&5.2&5\\
0.284&1.758&6.5&6\\
0.25&1.74&7.98&7\\
0.22&1.60&9.58&8\\
0.202&1.20&11.28&9\\
  \bottomrule
\end{tabular}
\end{table}

\begin{table}[t!]
\caption{\label{tab:DiodeTM}%
Varactor (MAVR-000120-1411) capacitance and resistance verses bias voltage characteristic for TM polarization.} 
\begin{tabular}{>{\centering\arraybackslash}p{0.25\columnwidth}>{\centering\arraybackslash}p{0.2\columnwidth} >{\centering\arraybackslash}p{0.2\columnwidth}>{\centering\arraybackslash}p{0.25\columnwidth}}
 \toprule
 Varactor capacitance (pF) & Additional loss $R^{TM}$ used in simulation ($\Omega$)&Bias voltage used in circuit simulation (V)&Bias voltage used in measurement (V)\\
  \hline
0.385&2.066&4.16&4\\
0.319&1.95&5.44&5\\
0.271&2.00&6.92&6\\
0.239&2.17&8.4&7\\
0.213&2.39&10.2&8\\
0.19&2.12&12.49&9\\
  \bottomrule
\end{tabular}
\end{table}

\begin{figure}[t!]
\subfloat[\label{sfig:DC4_M_TE}]{%
  \includegraphics[clip,width=0.165\columnwidth]{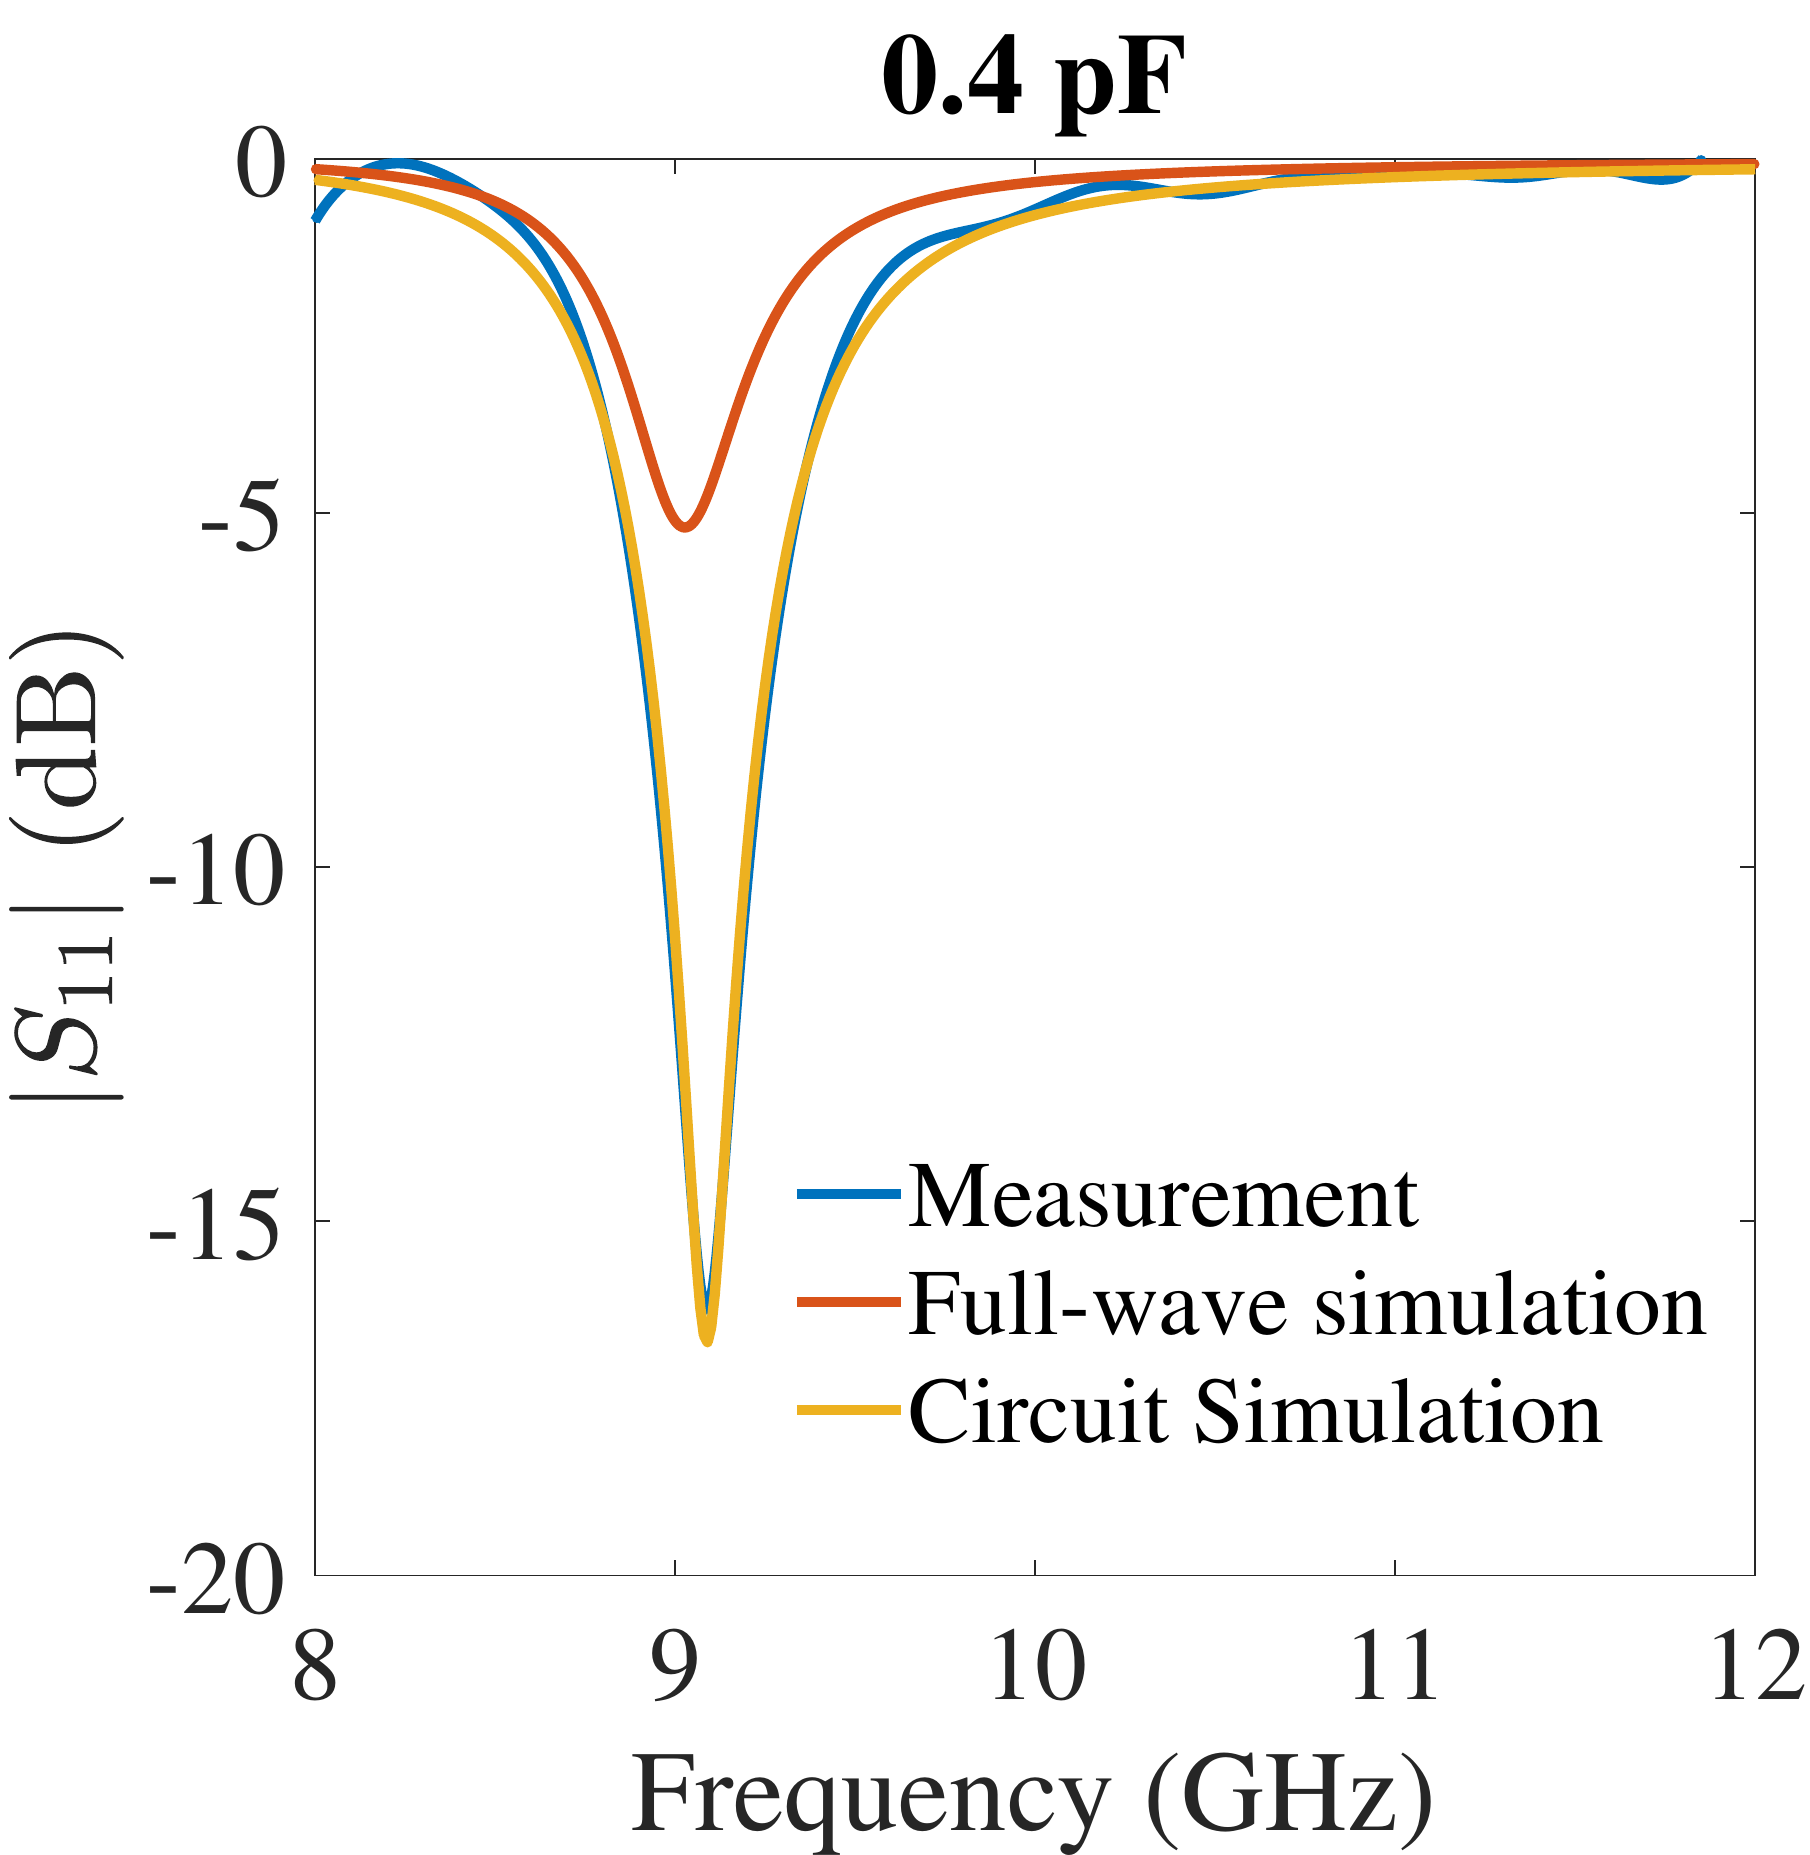}%
}\hfill
\subfloat[\label{sfig:DC5_M_TE}]{%
  \includegraphics[clip,width=0.165\columnwidth]{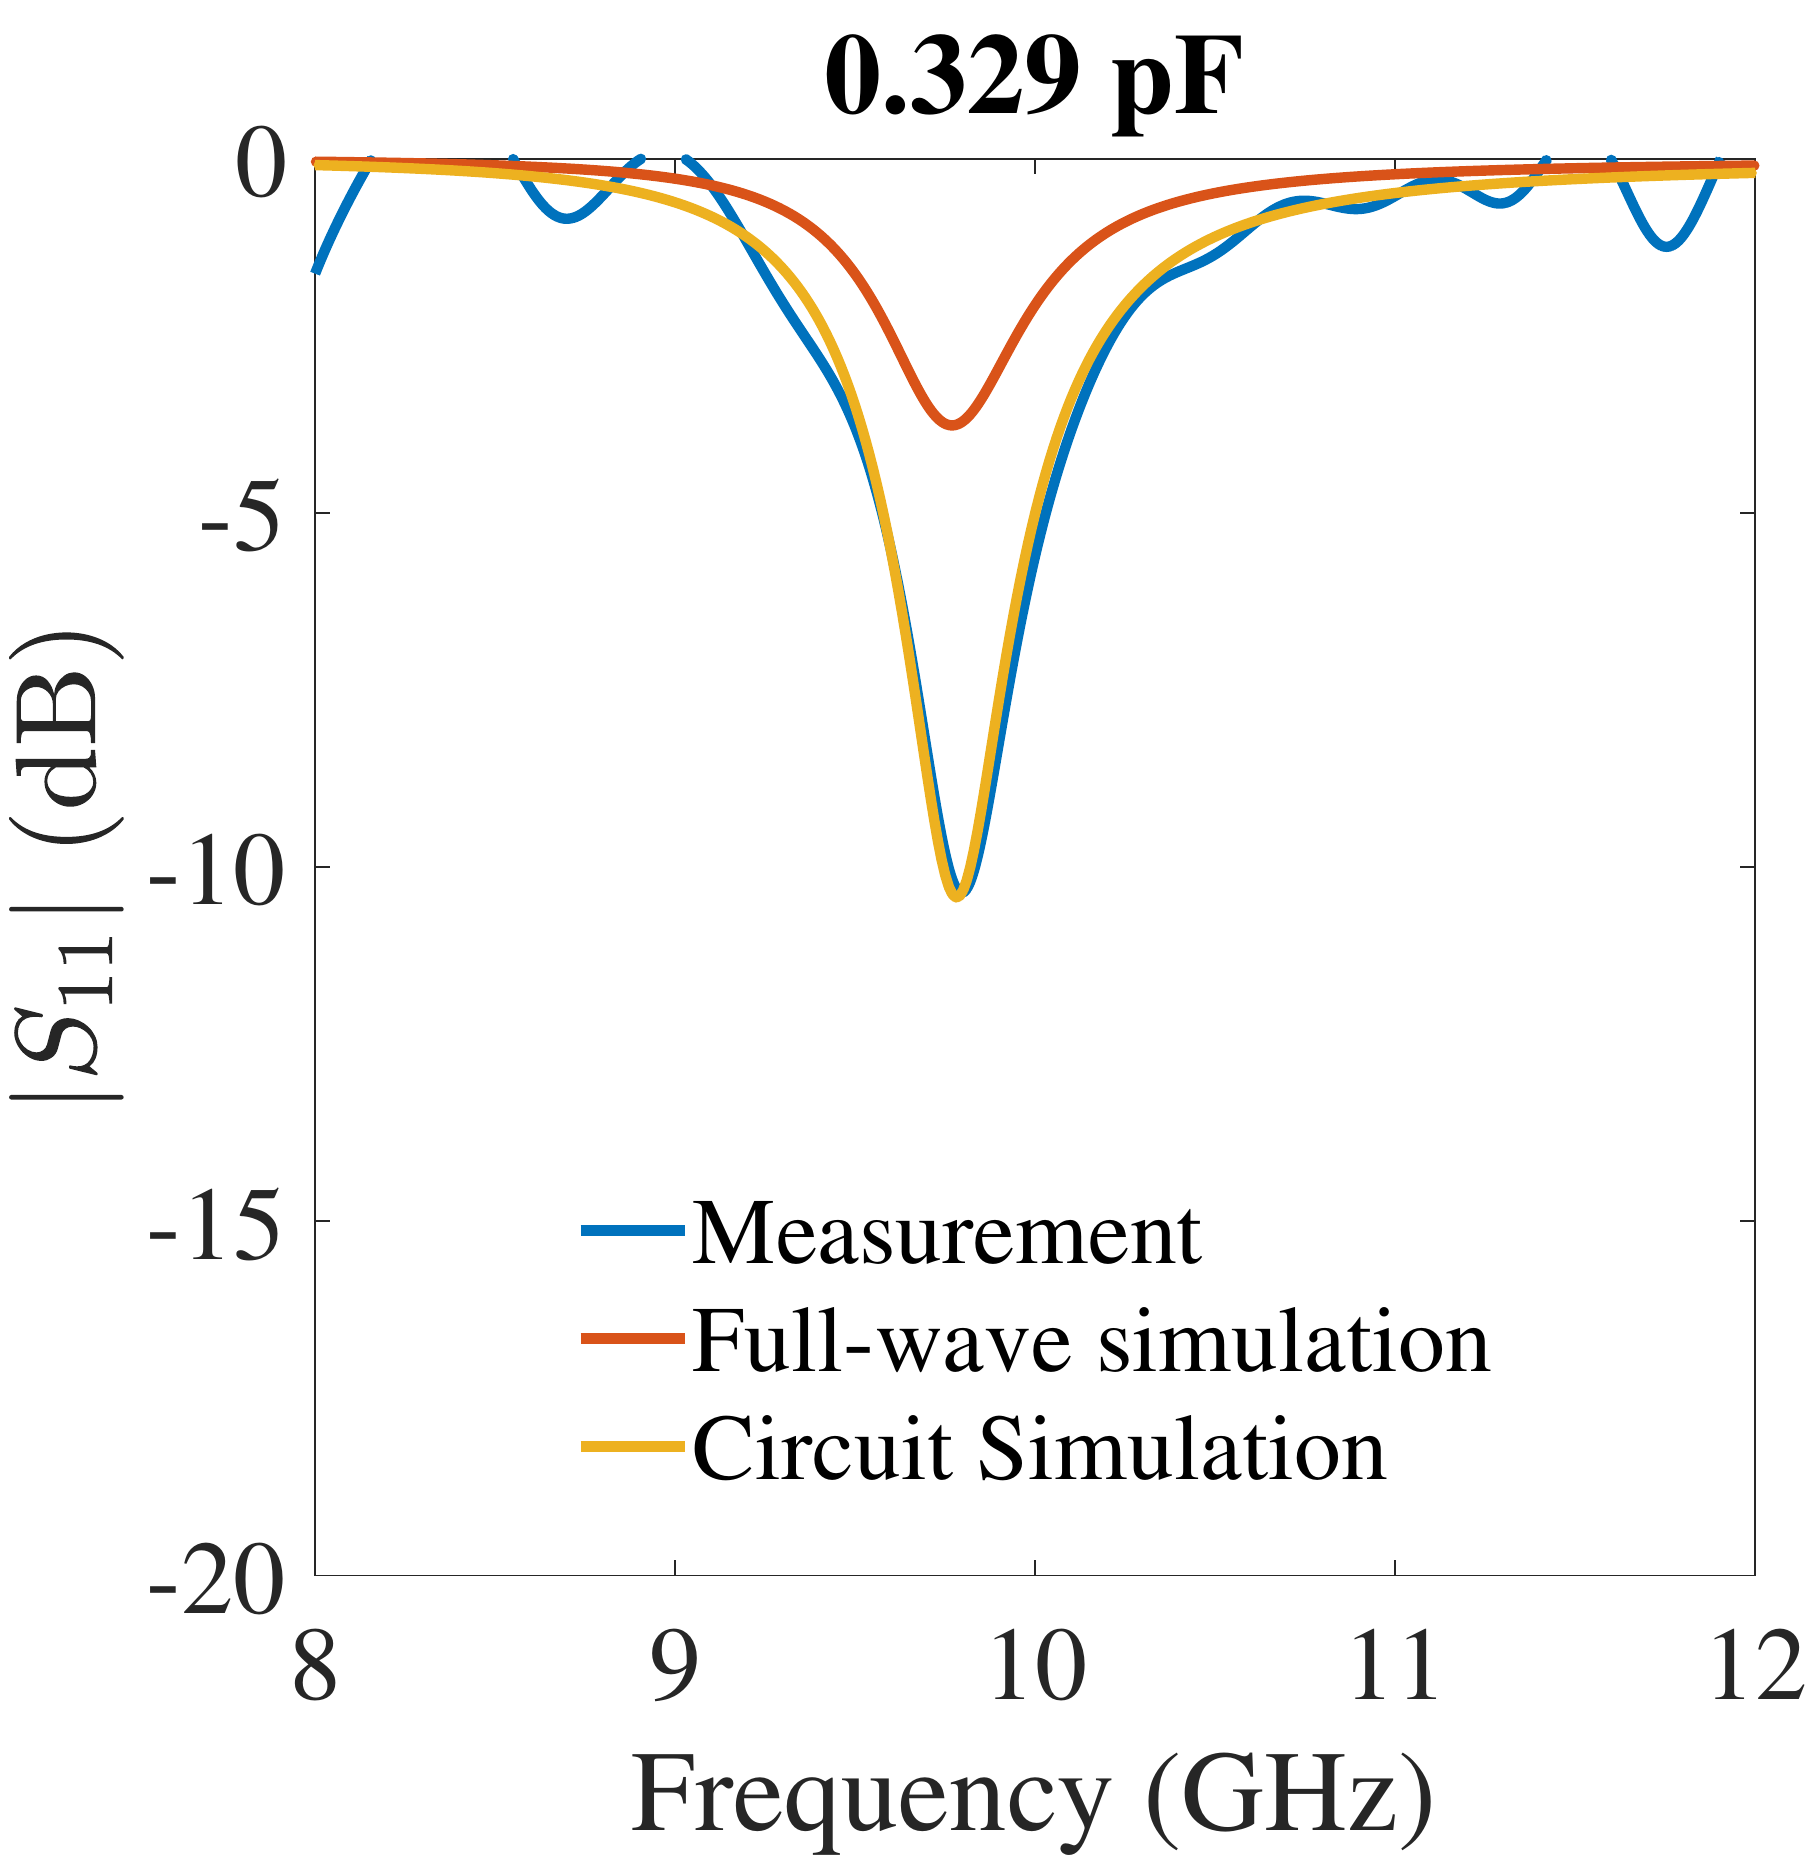}%
}\hfill
\subfloat[\label{sfig:DC6_M_TE}]{%
  \includegraphics[clip,width=0.165\columnwidth]{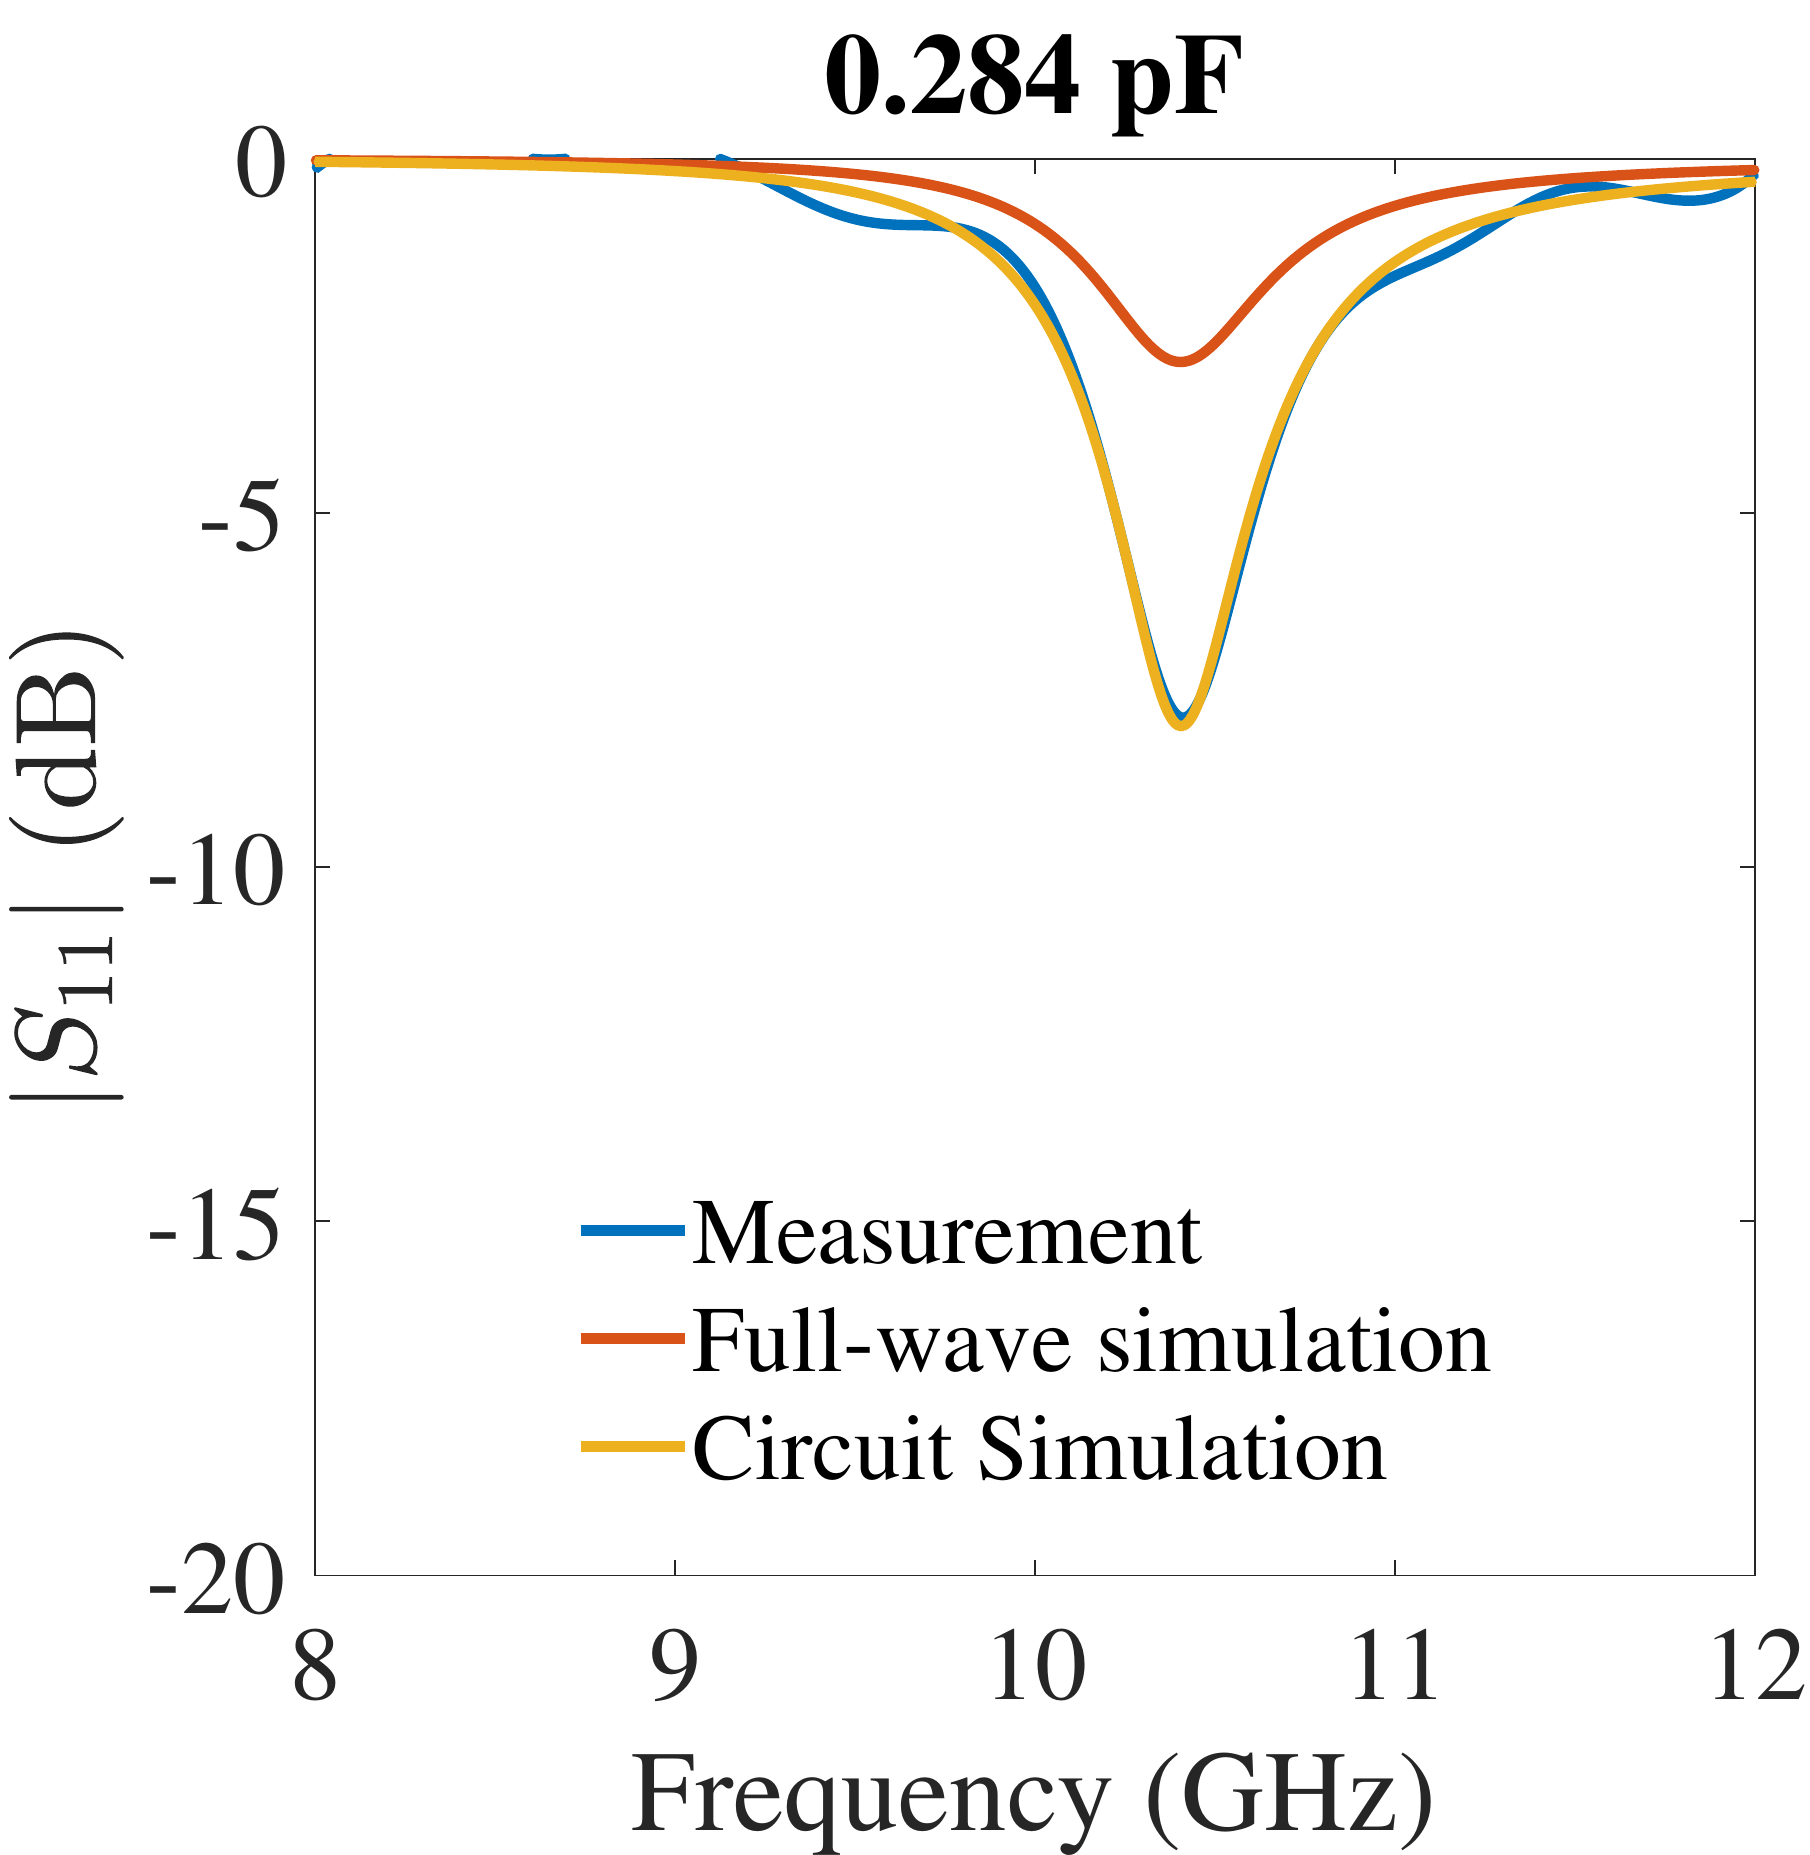}%
}\hfill
\subfloat[\label{sfig:DC7_M_TE}]{%
  \includegraphics[clip,width=0.165\columnwidth]{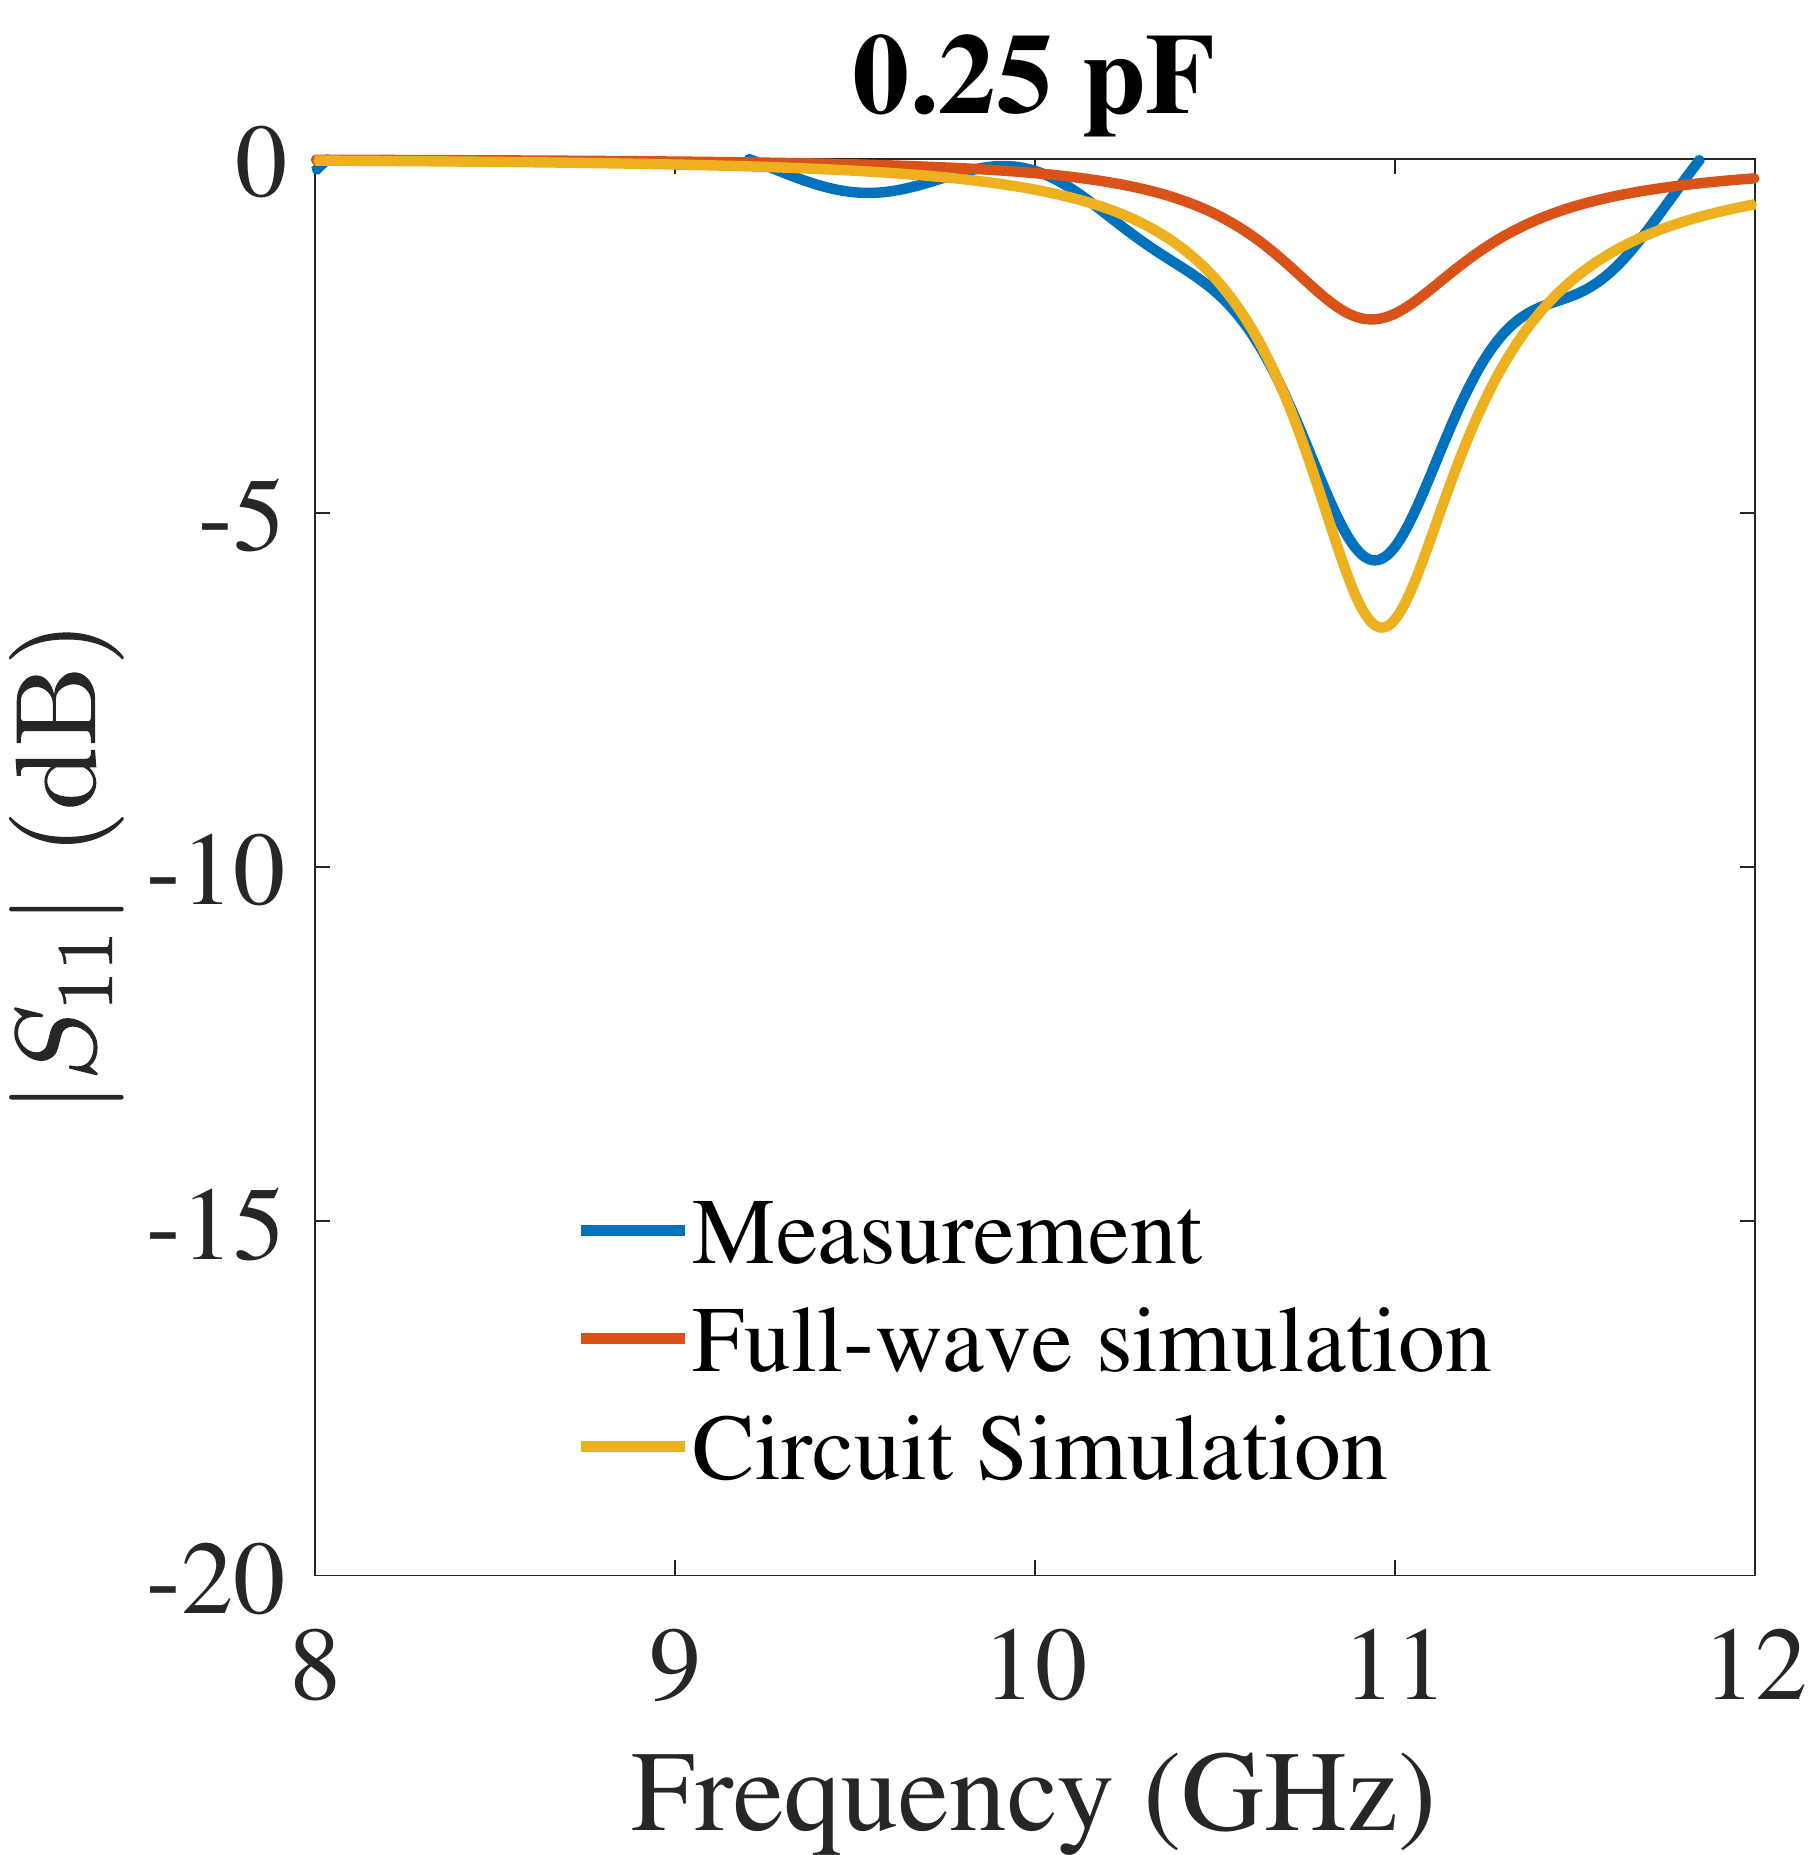}%
}\hfill
\subfloat[\label{sfig:DC8_M_TE}]{%
  \includegraphics[clip,width=0.165\columnwidth]{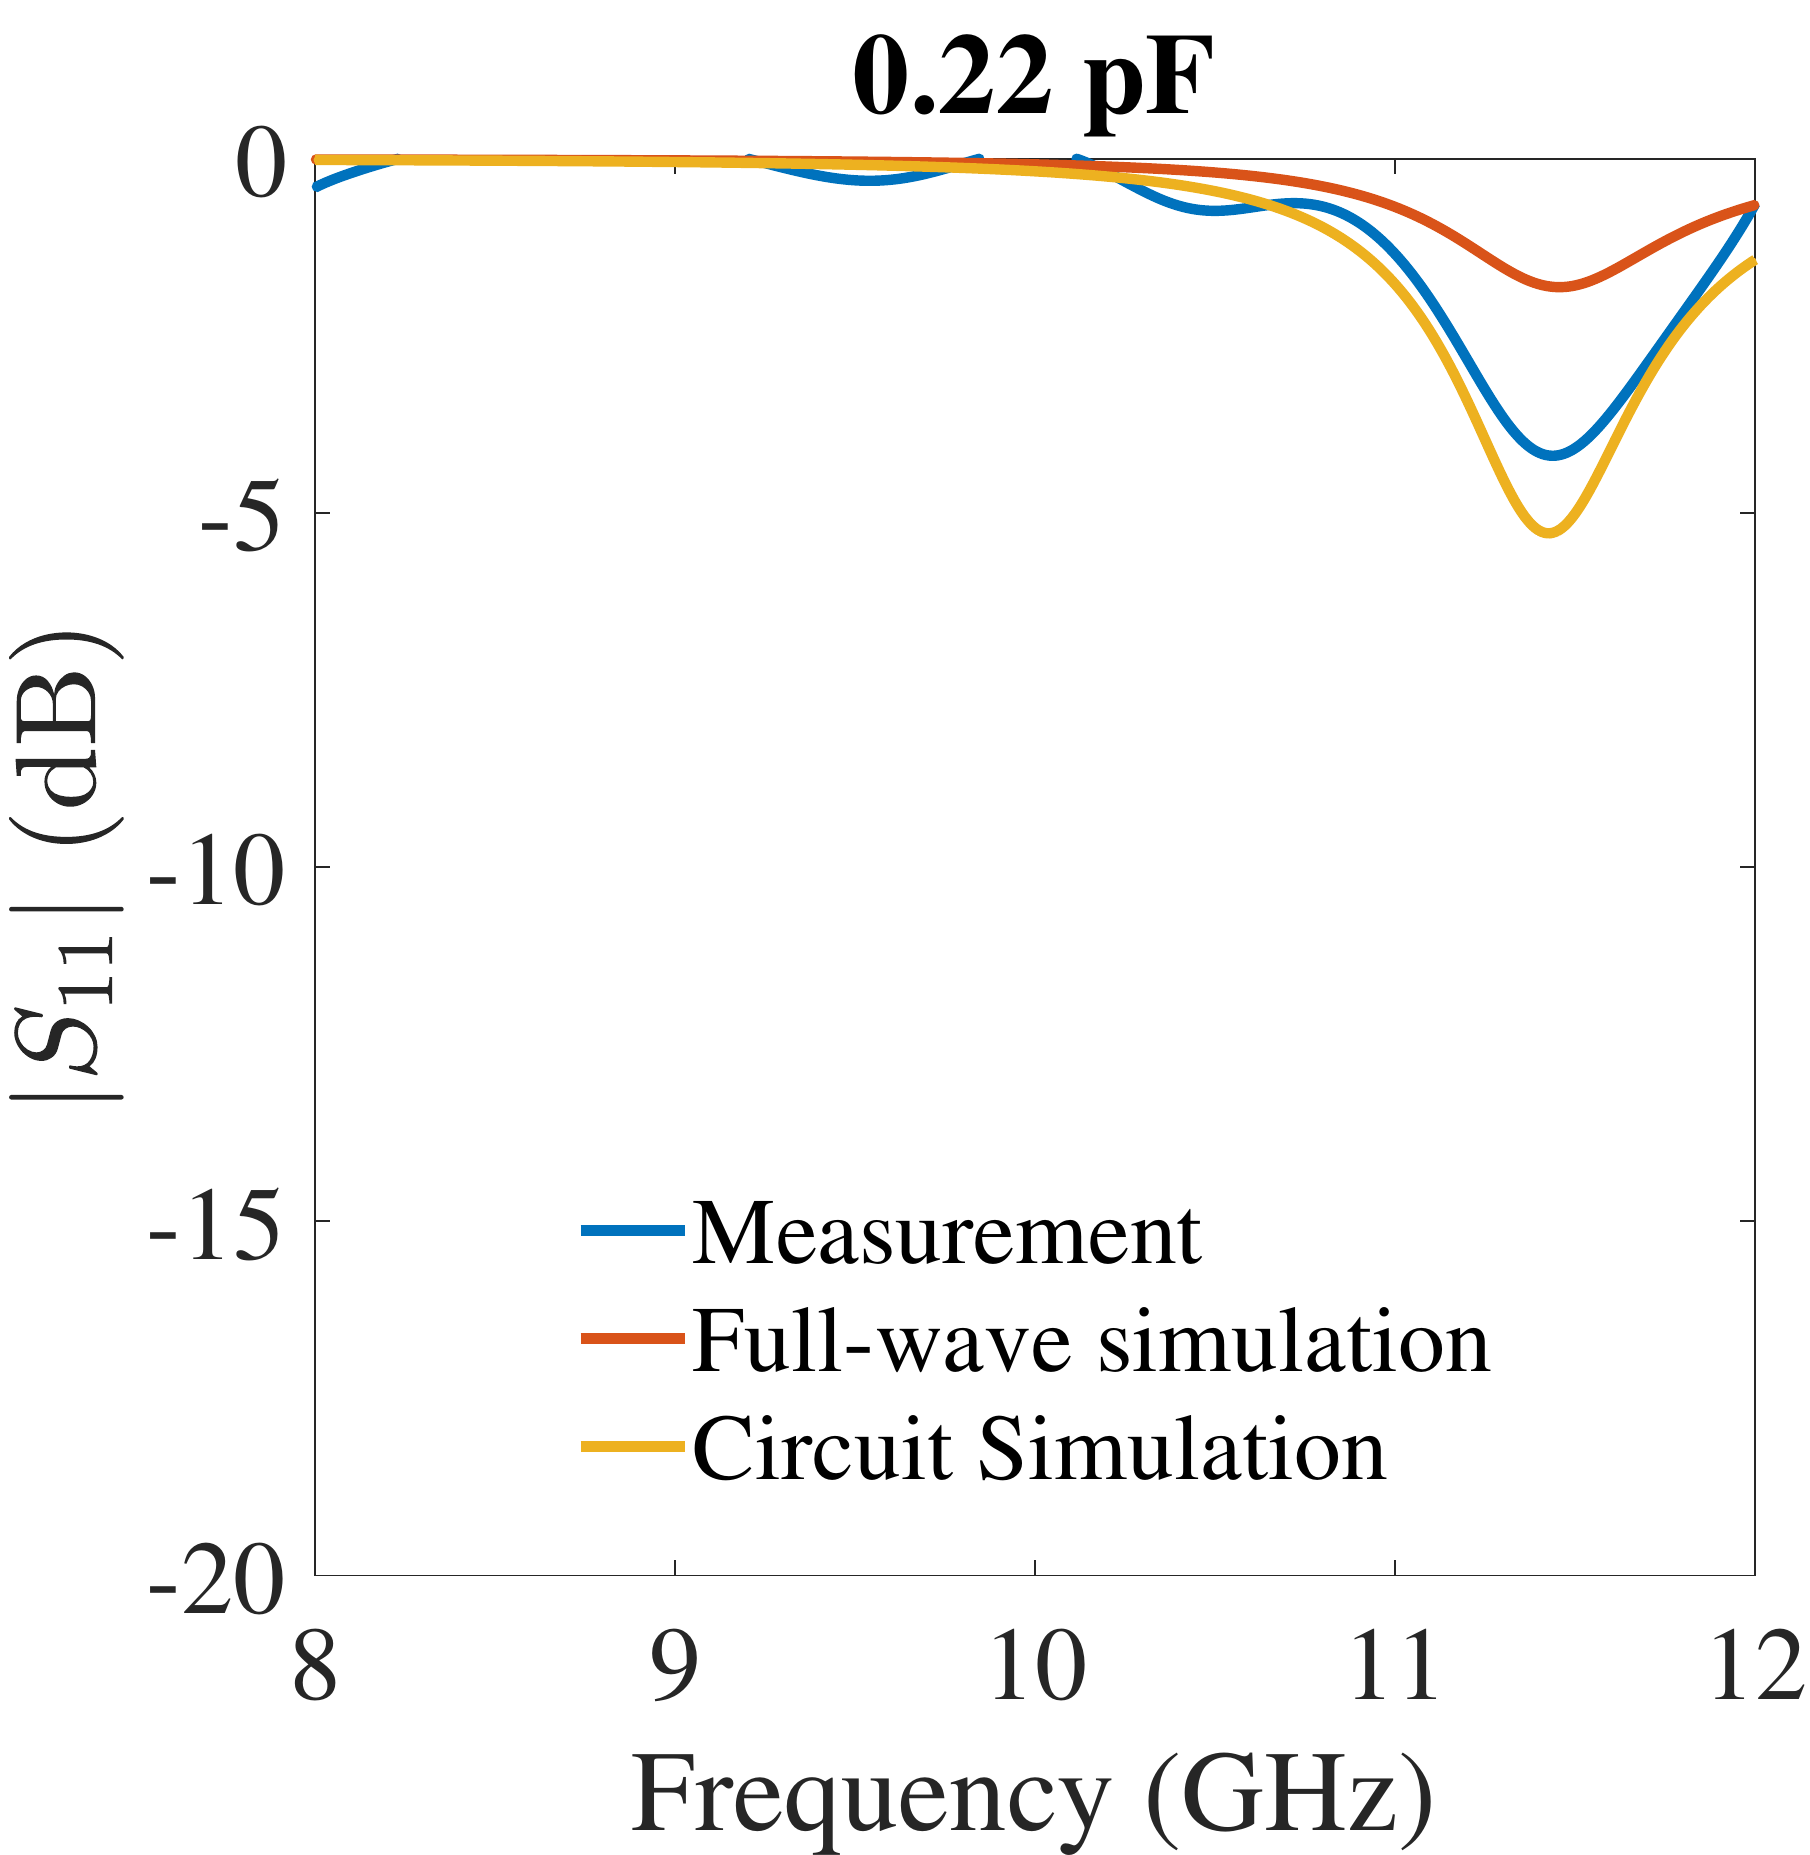}%
}\hfill
\subfloat[\label{sfig:DC9_M_TE}]{%
  \includegraphics[clip,width=0.165\columnwidth]{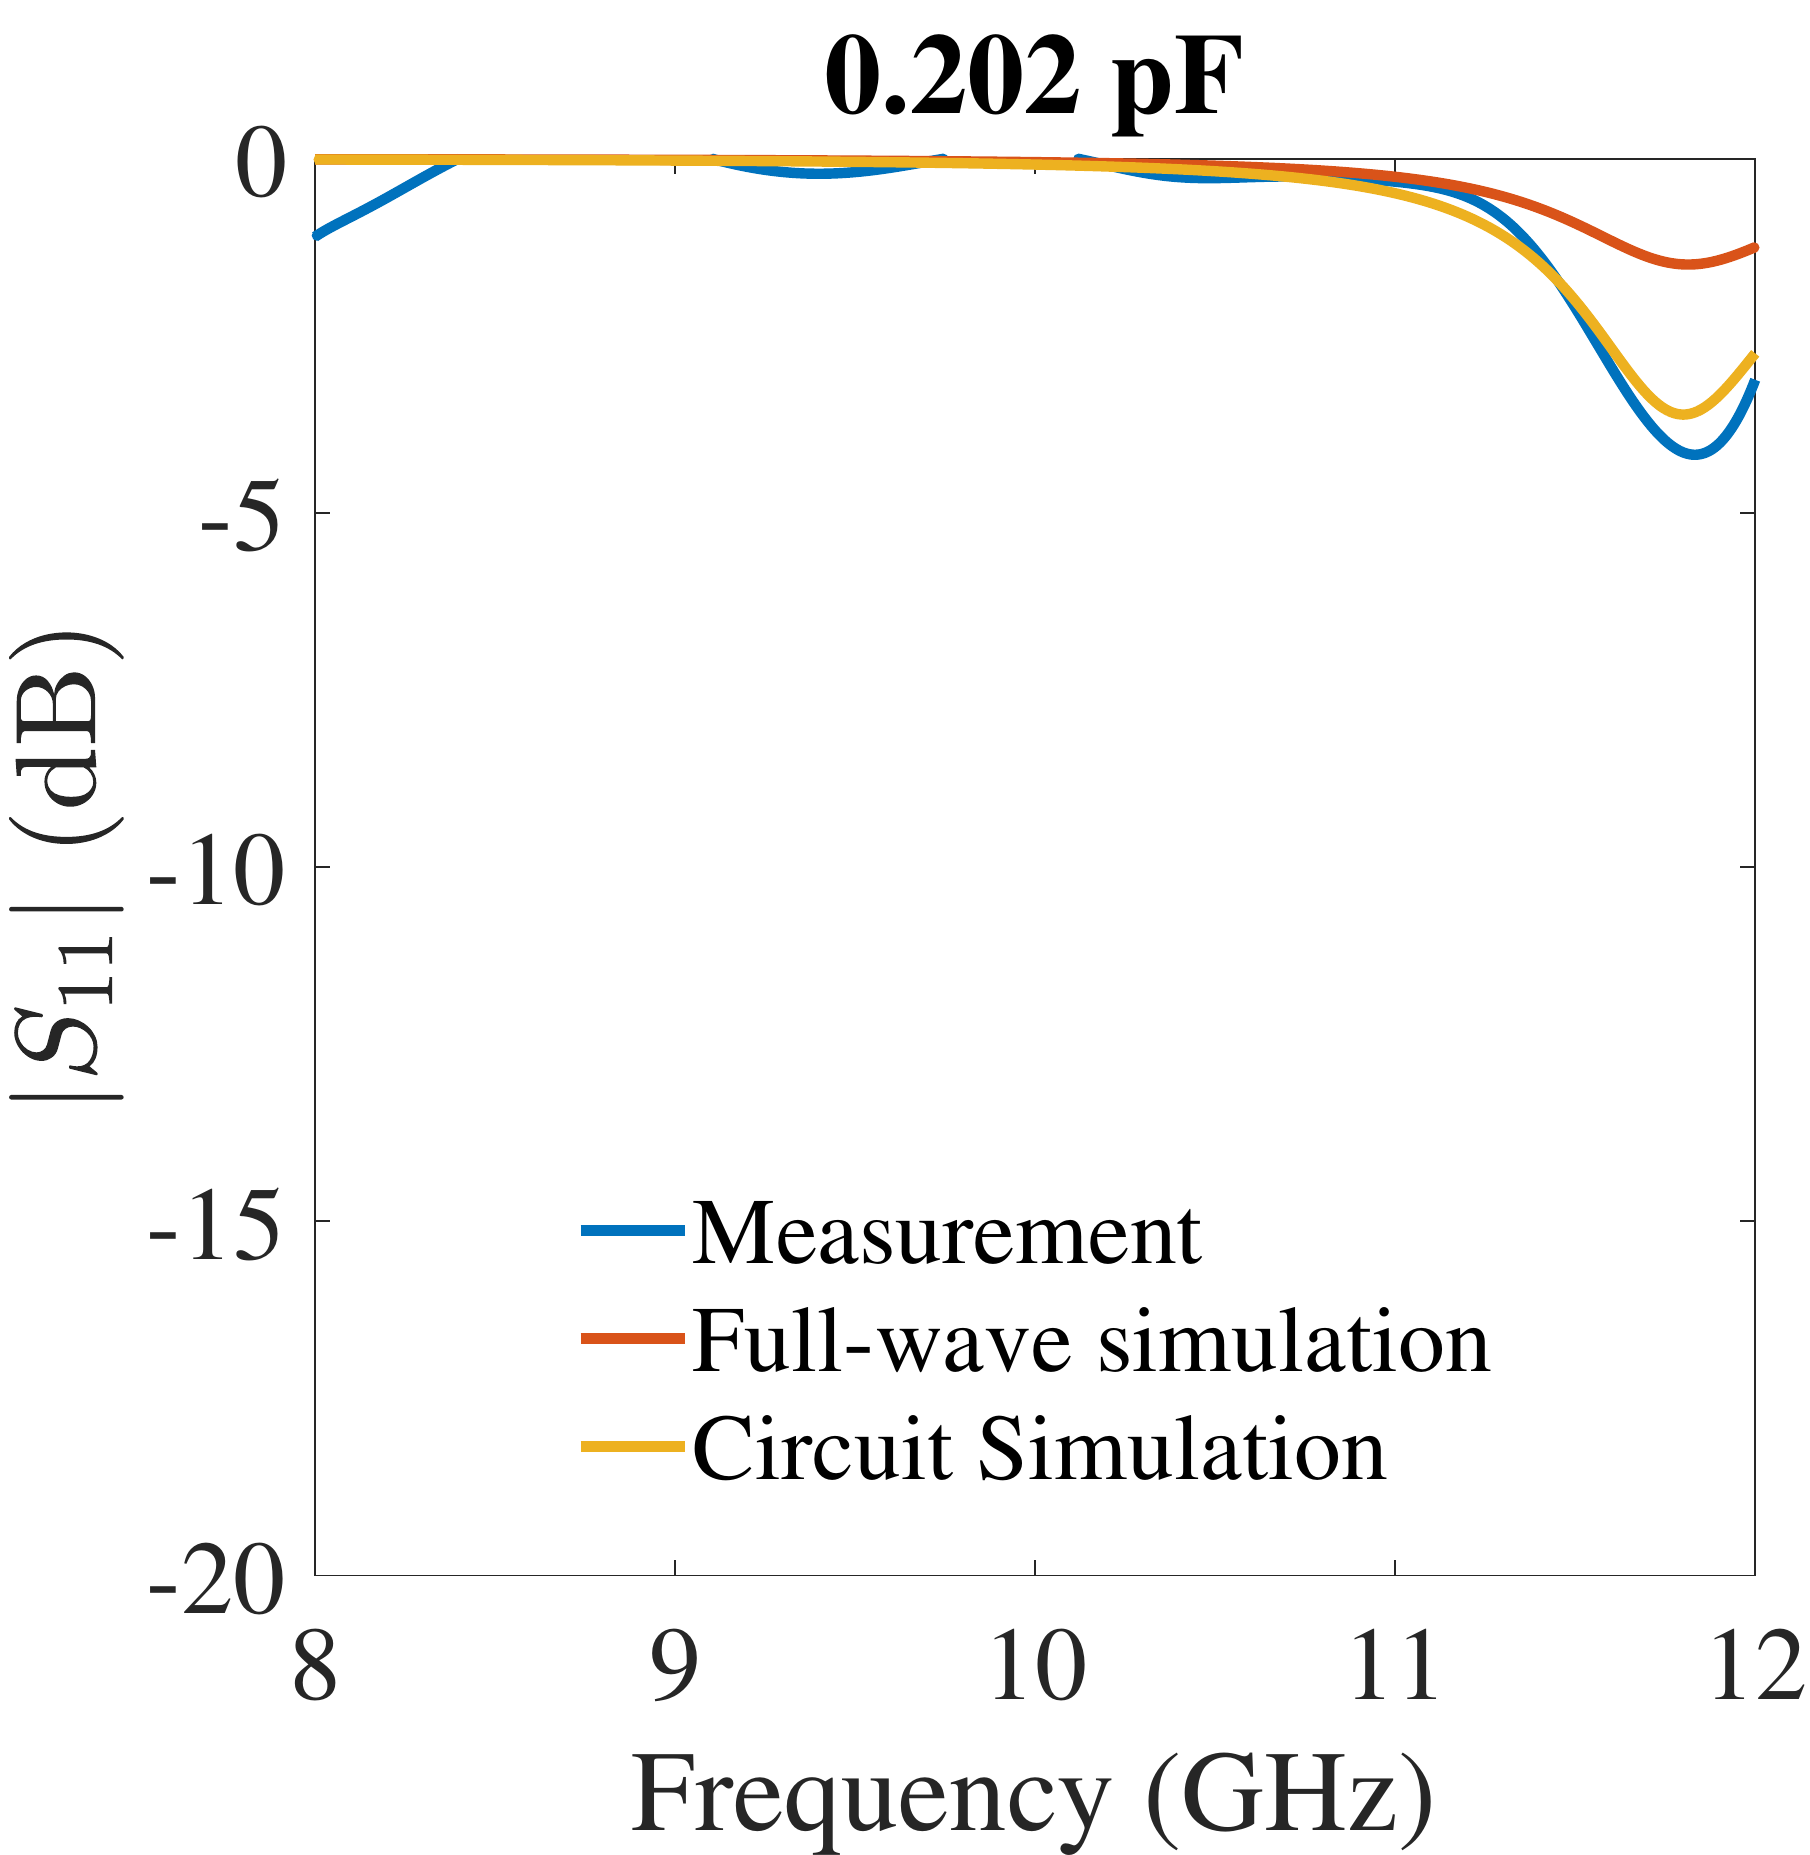}%
}\quad
\subfloat[\label{sfig:DC4_P_TE}]{%
  \includegraphics[clip,width=0.165\columnwidth]{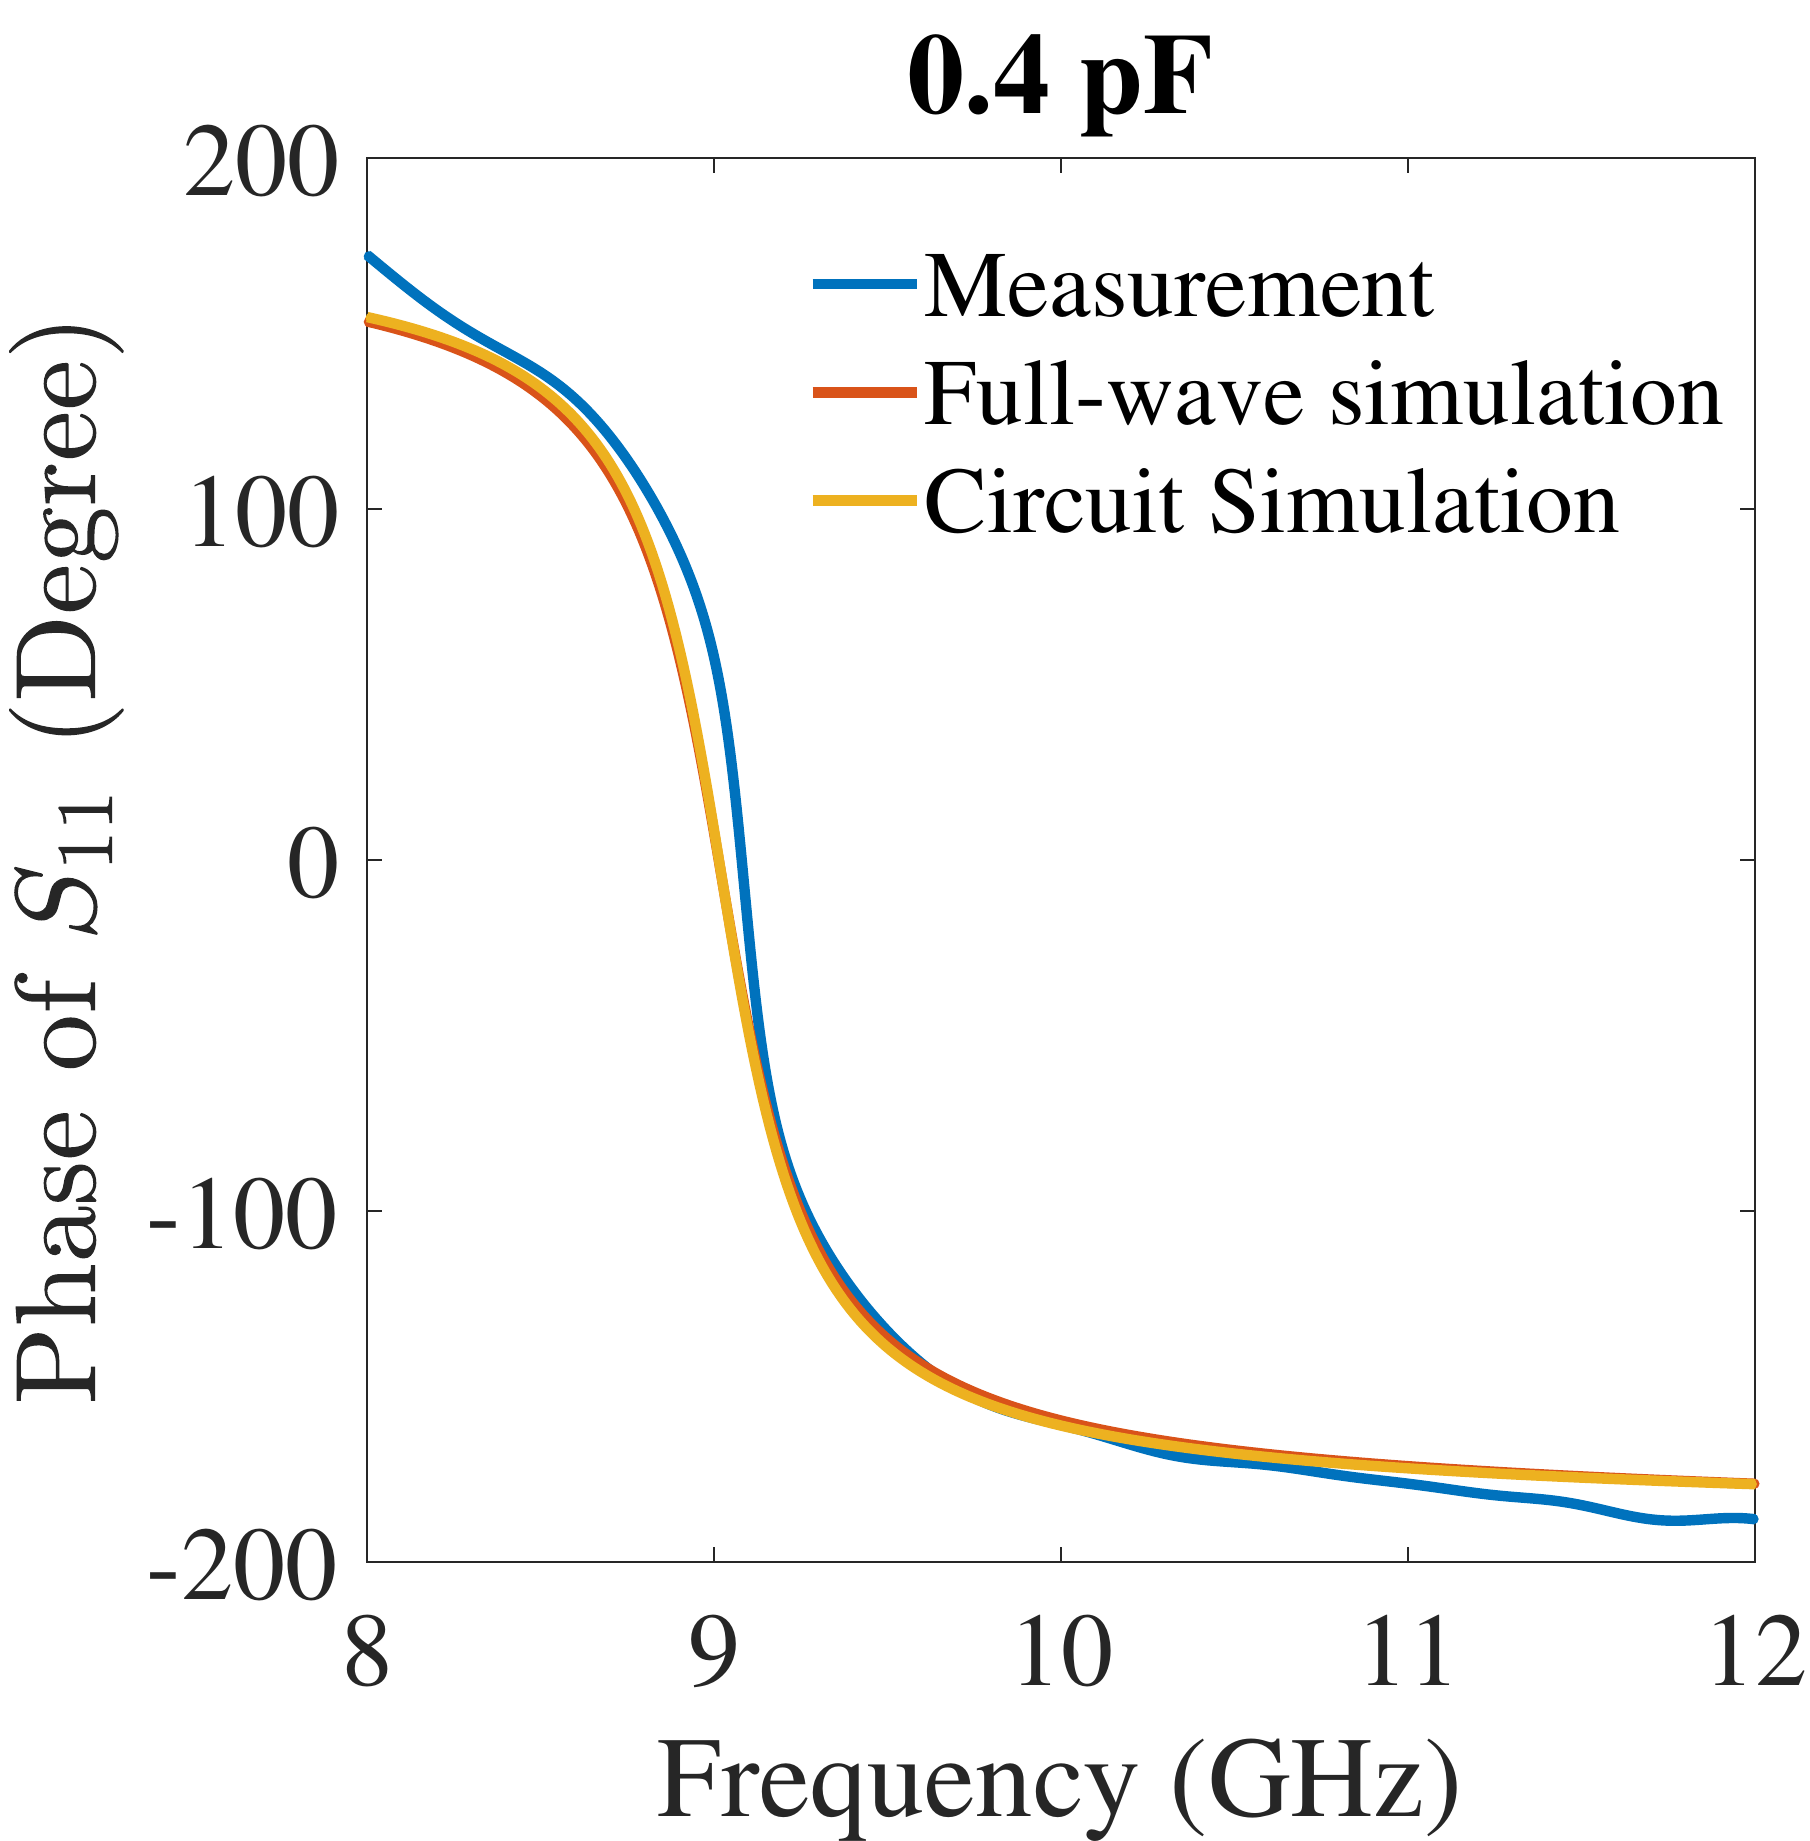}%
}\hfill
\subfloat[\label{sfig:DC5_P_TE}]{%
  \includegraphics[clip,width=0.165\columnwidth]{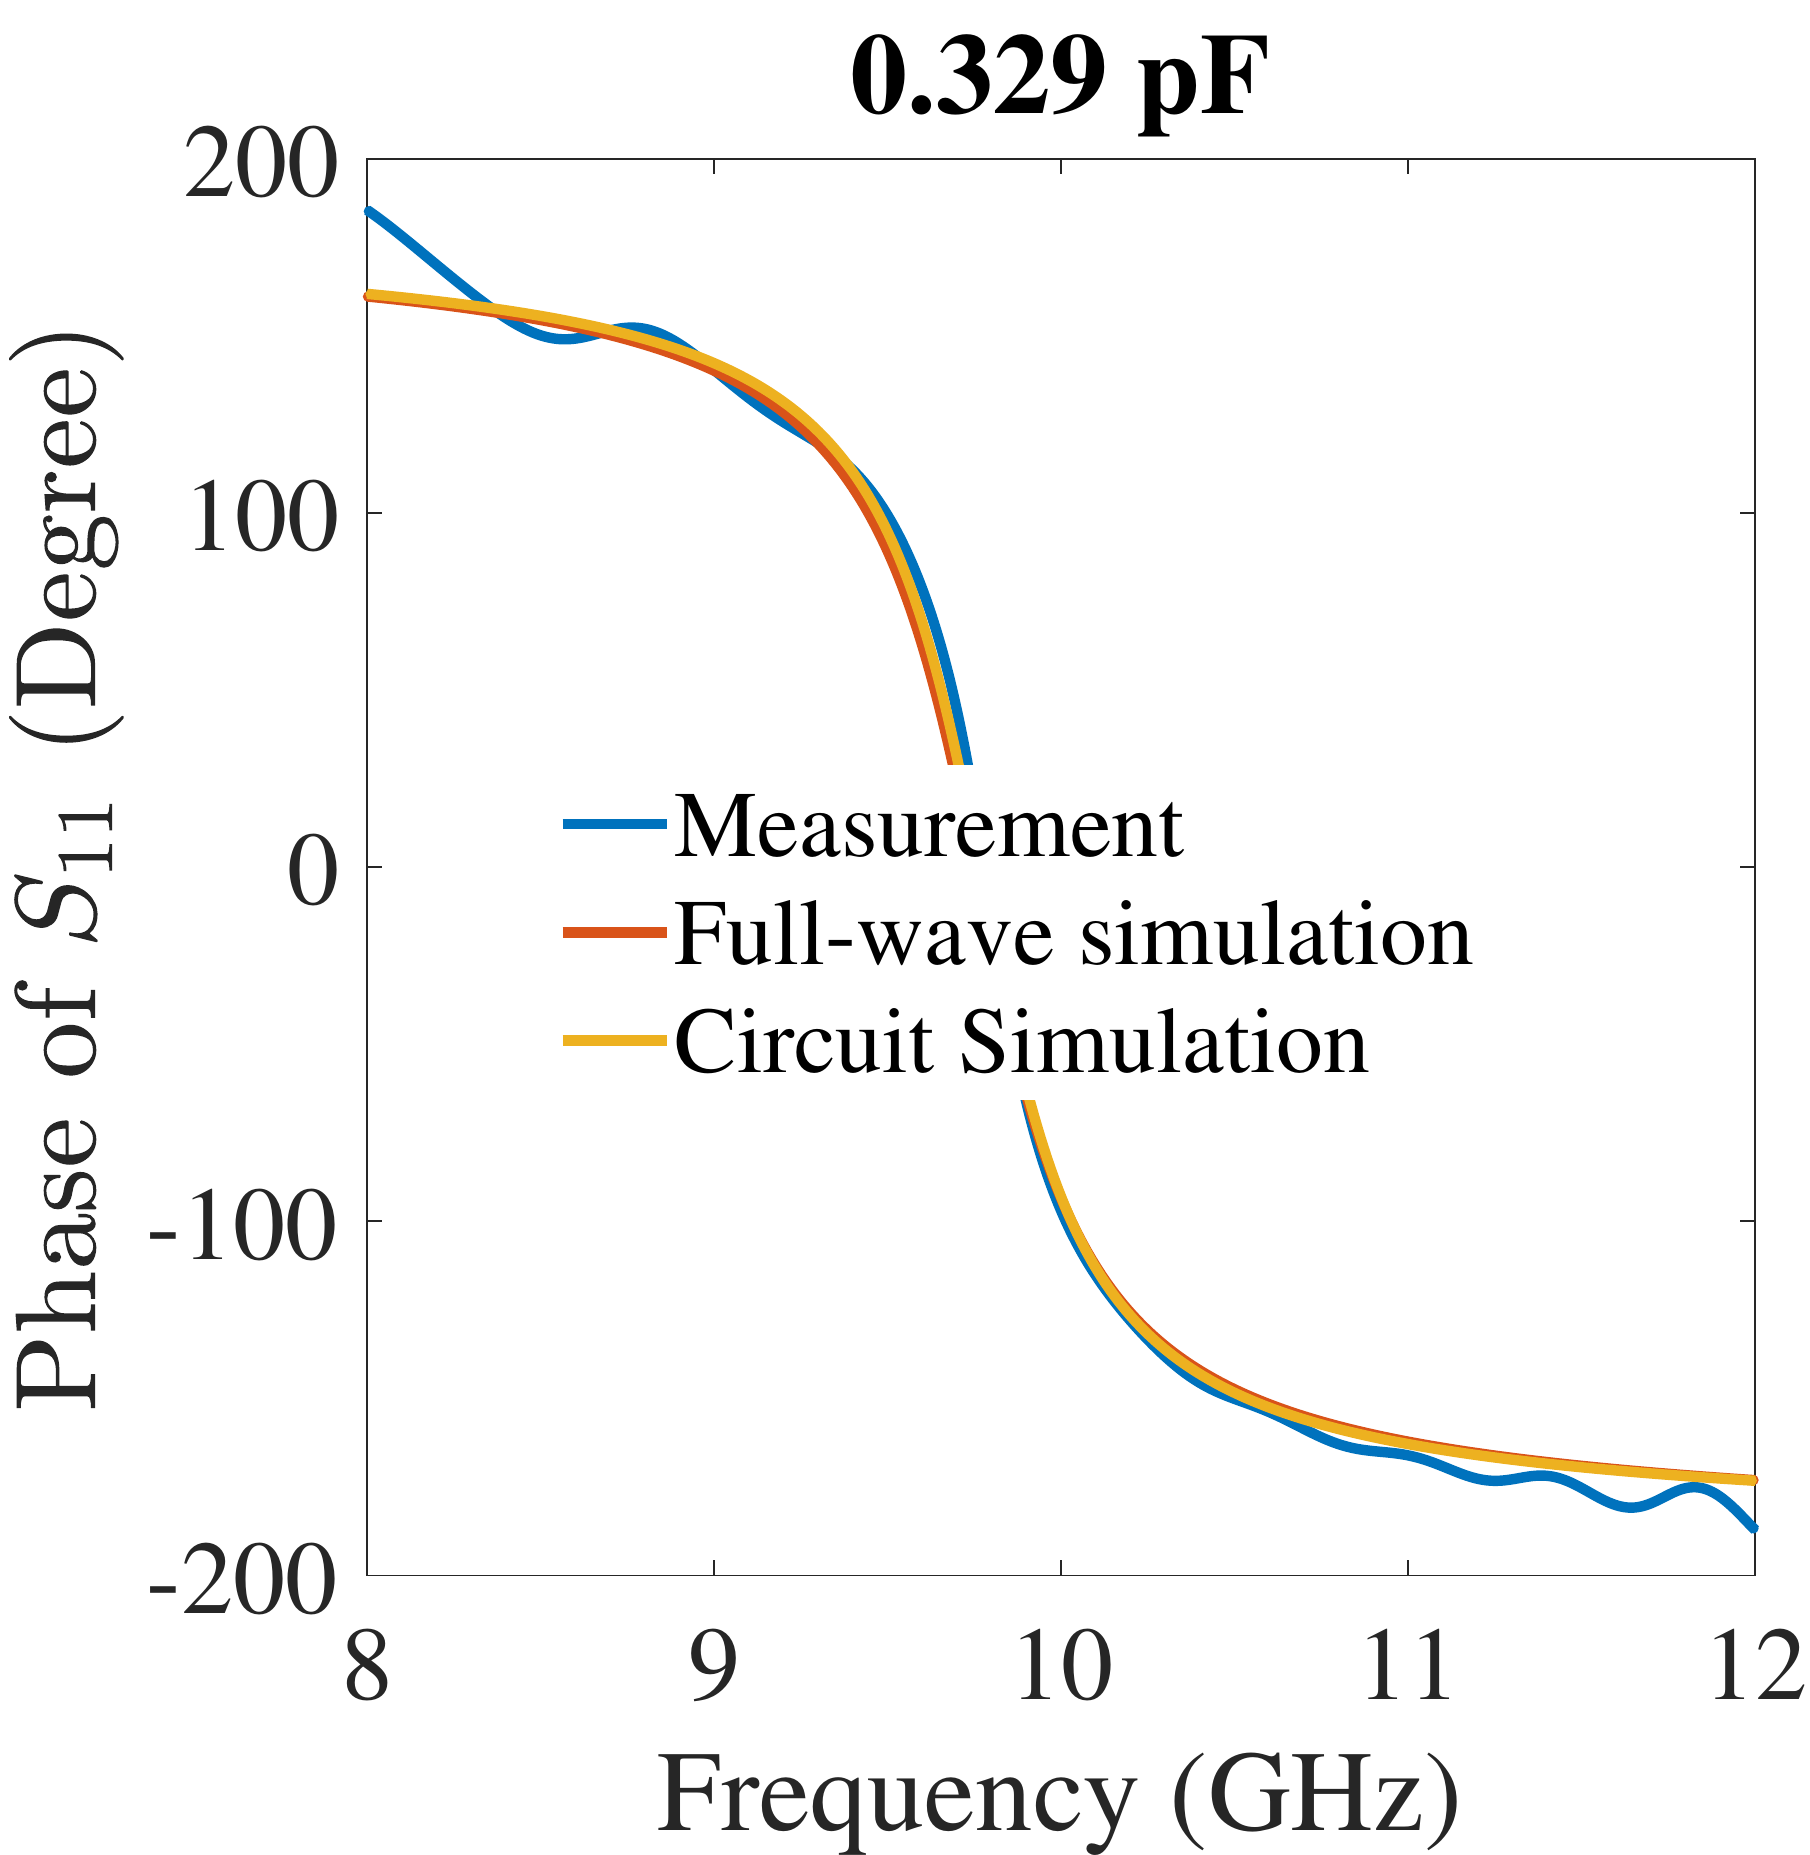}%
}\hfill
\subfloat[\label{sfig:DC6_P_TE}]{%
  \includegraphics[clip,width=0.165\columnwidth]{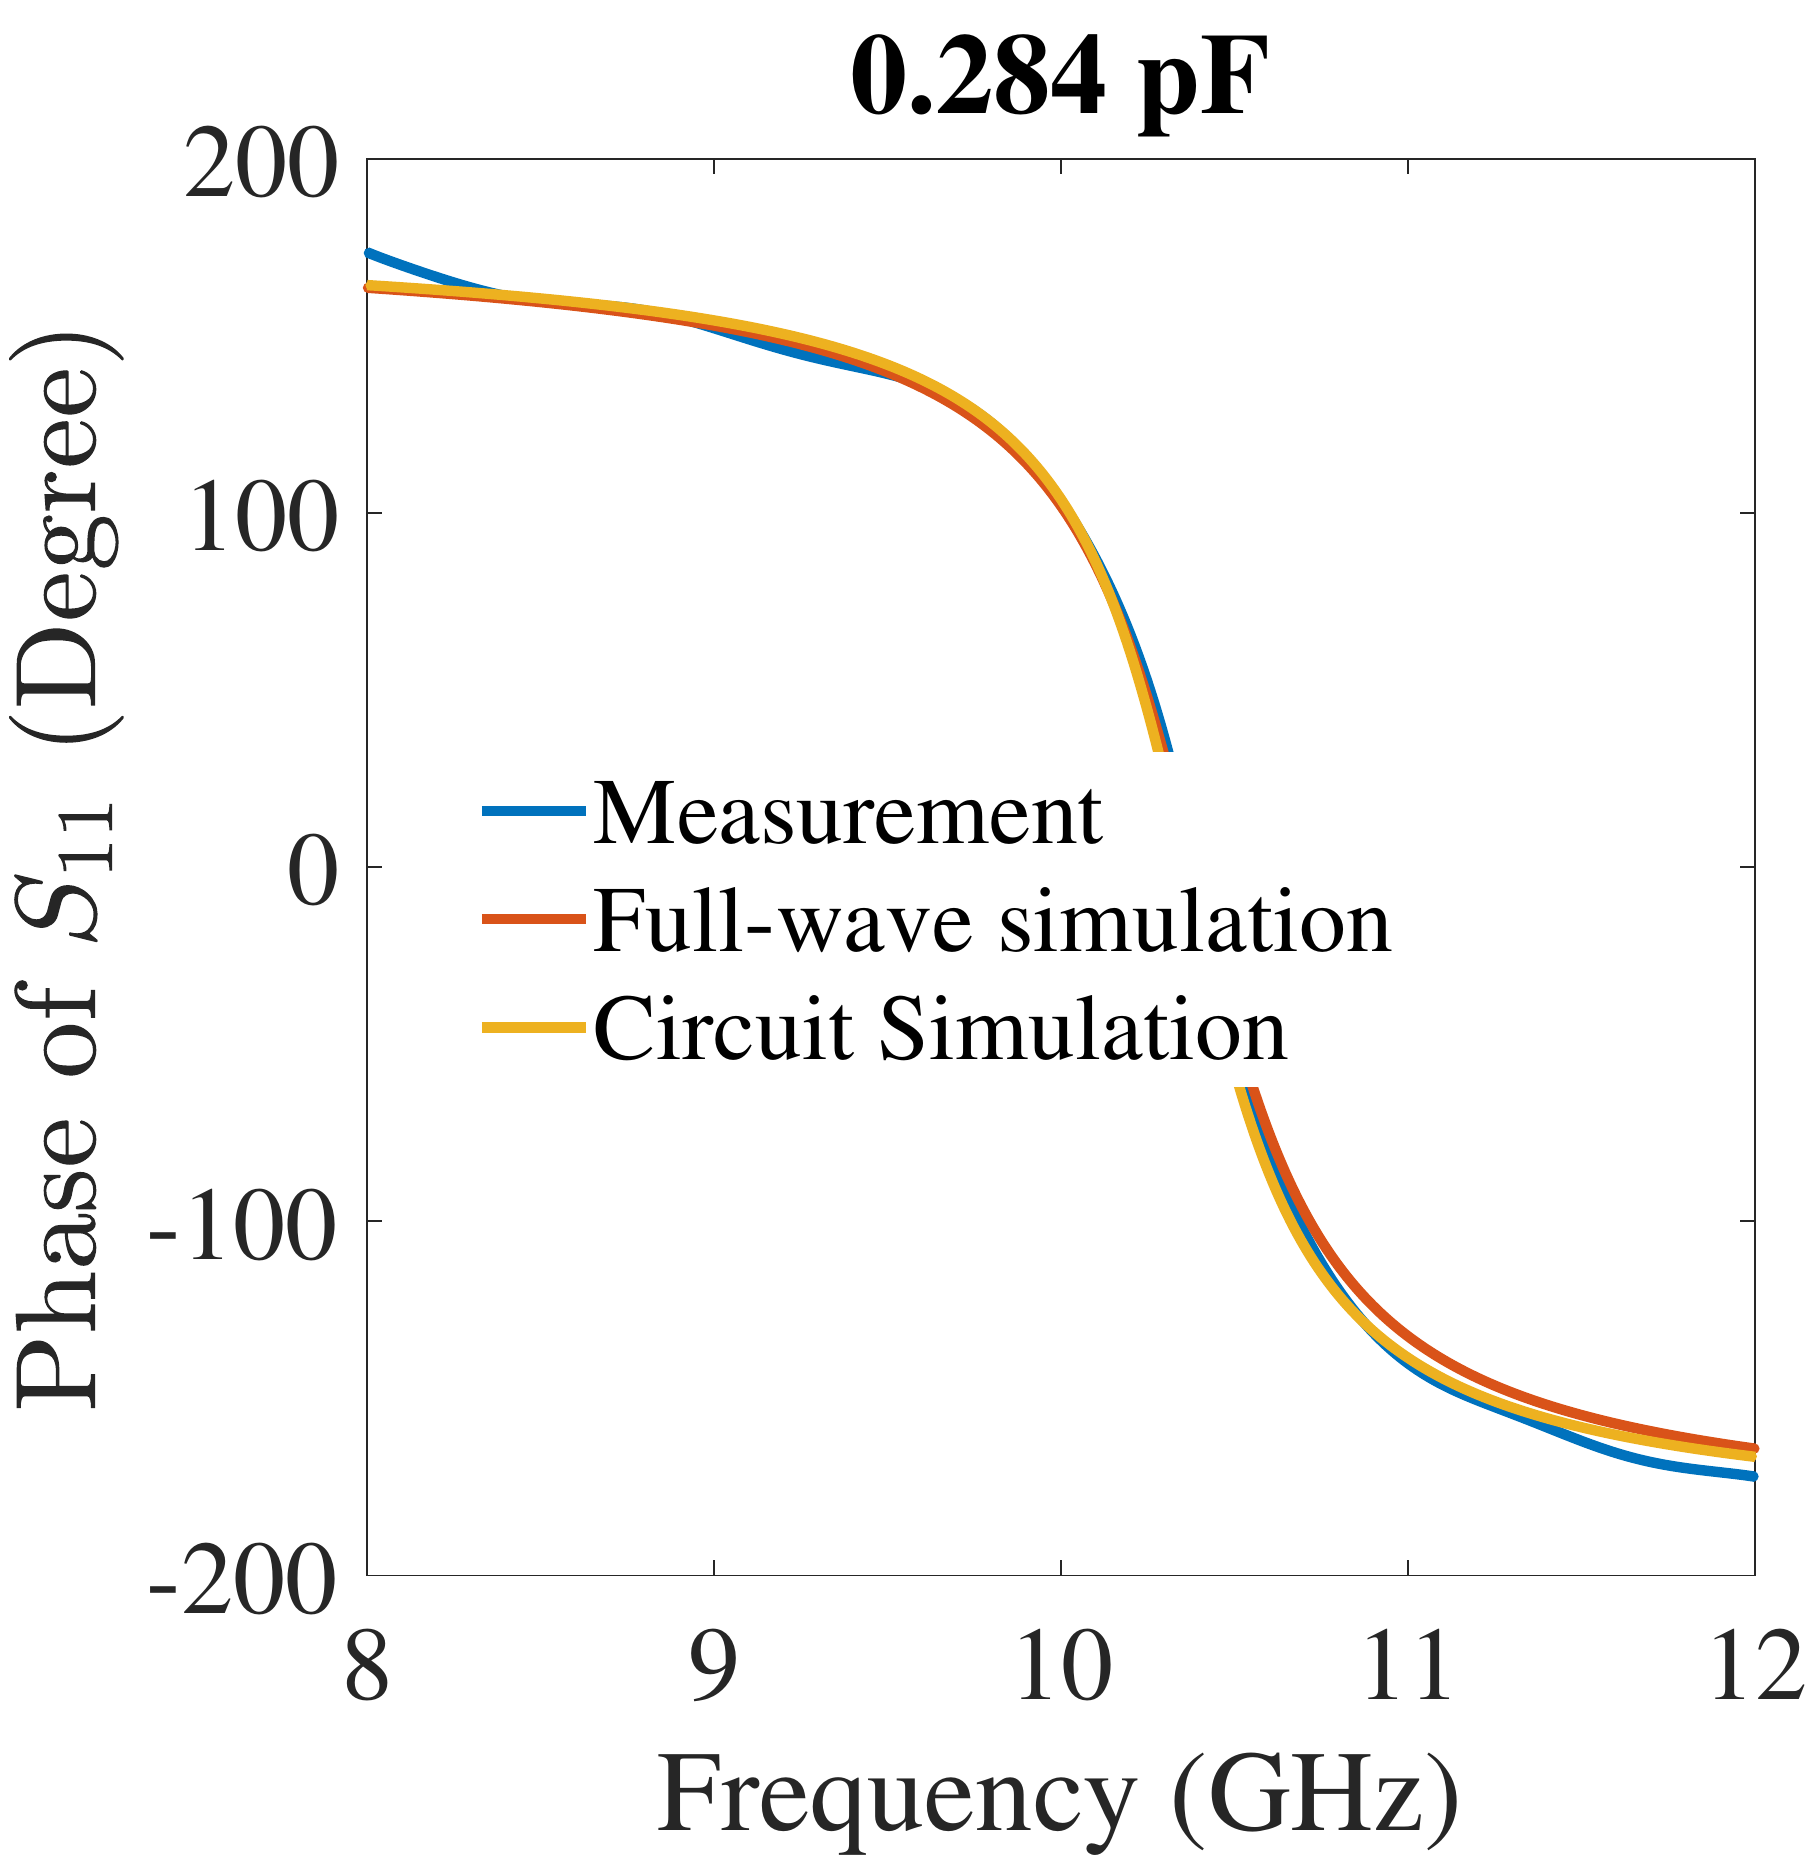}%
}\hfill
\subfloat[\label{sfig:DC7_P_TE}]{%
  \includegraphics[clip,width=0.165\columnwidth]{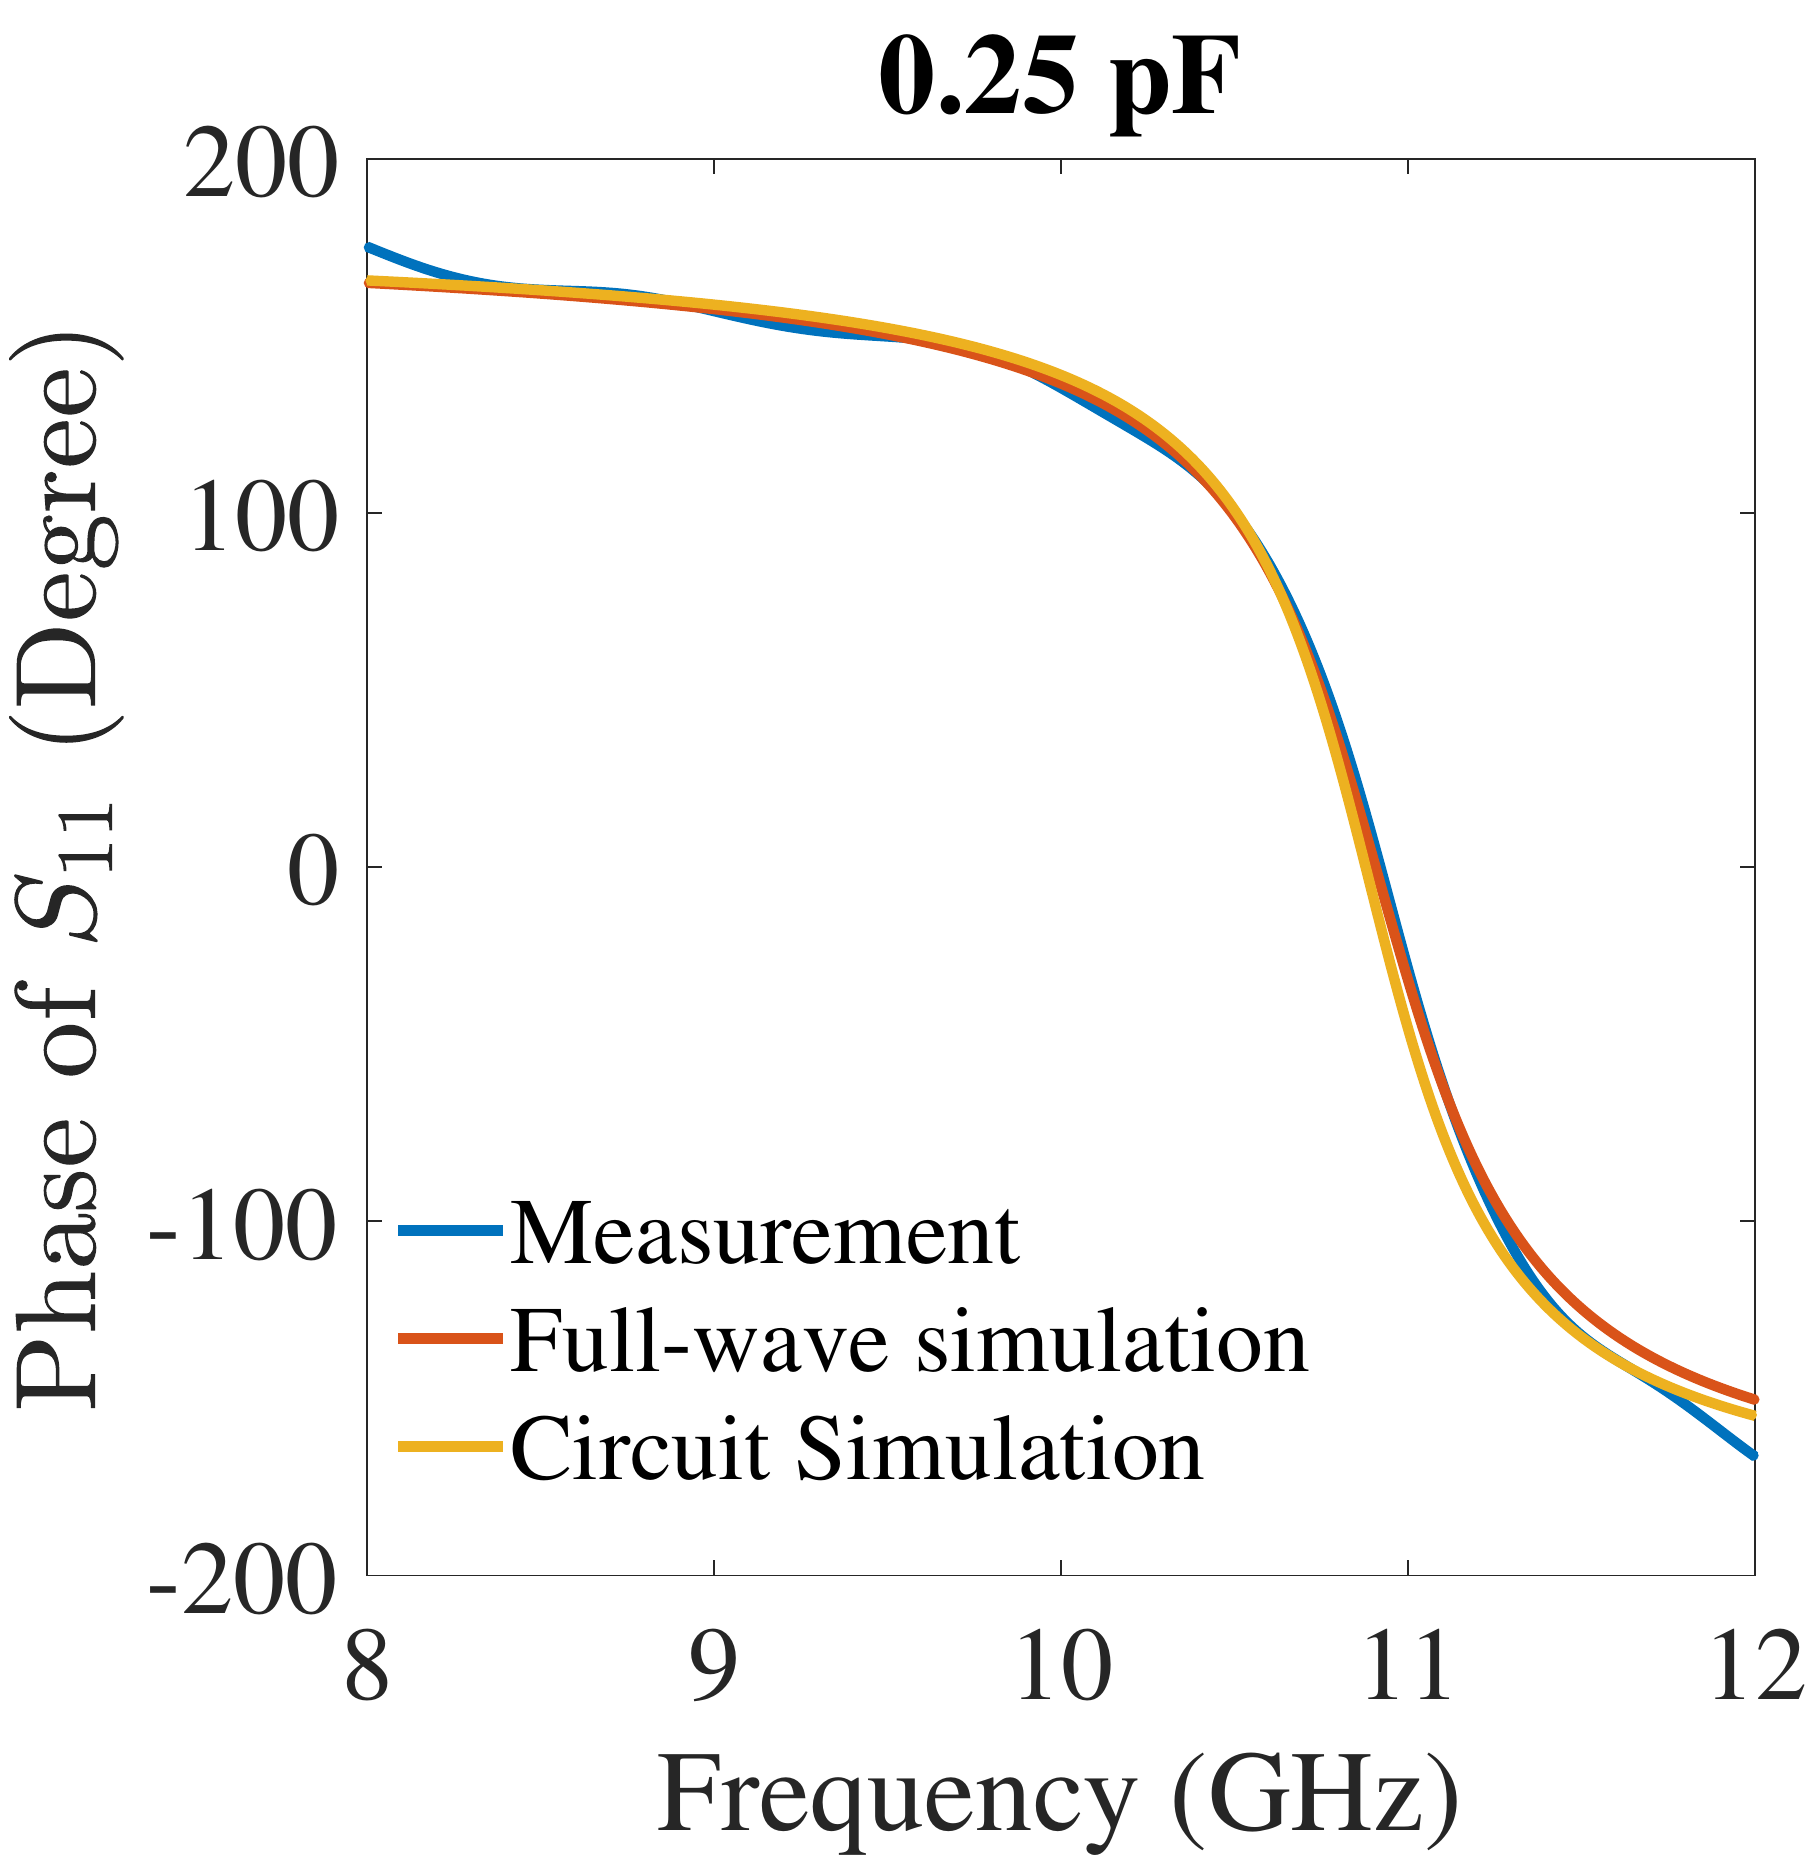}%
}\hfill
\subfloat[\label{sfig:DC8_P_TE}]{%
  \includegraphics[clip,width=0.165\columnwidth]{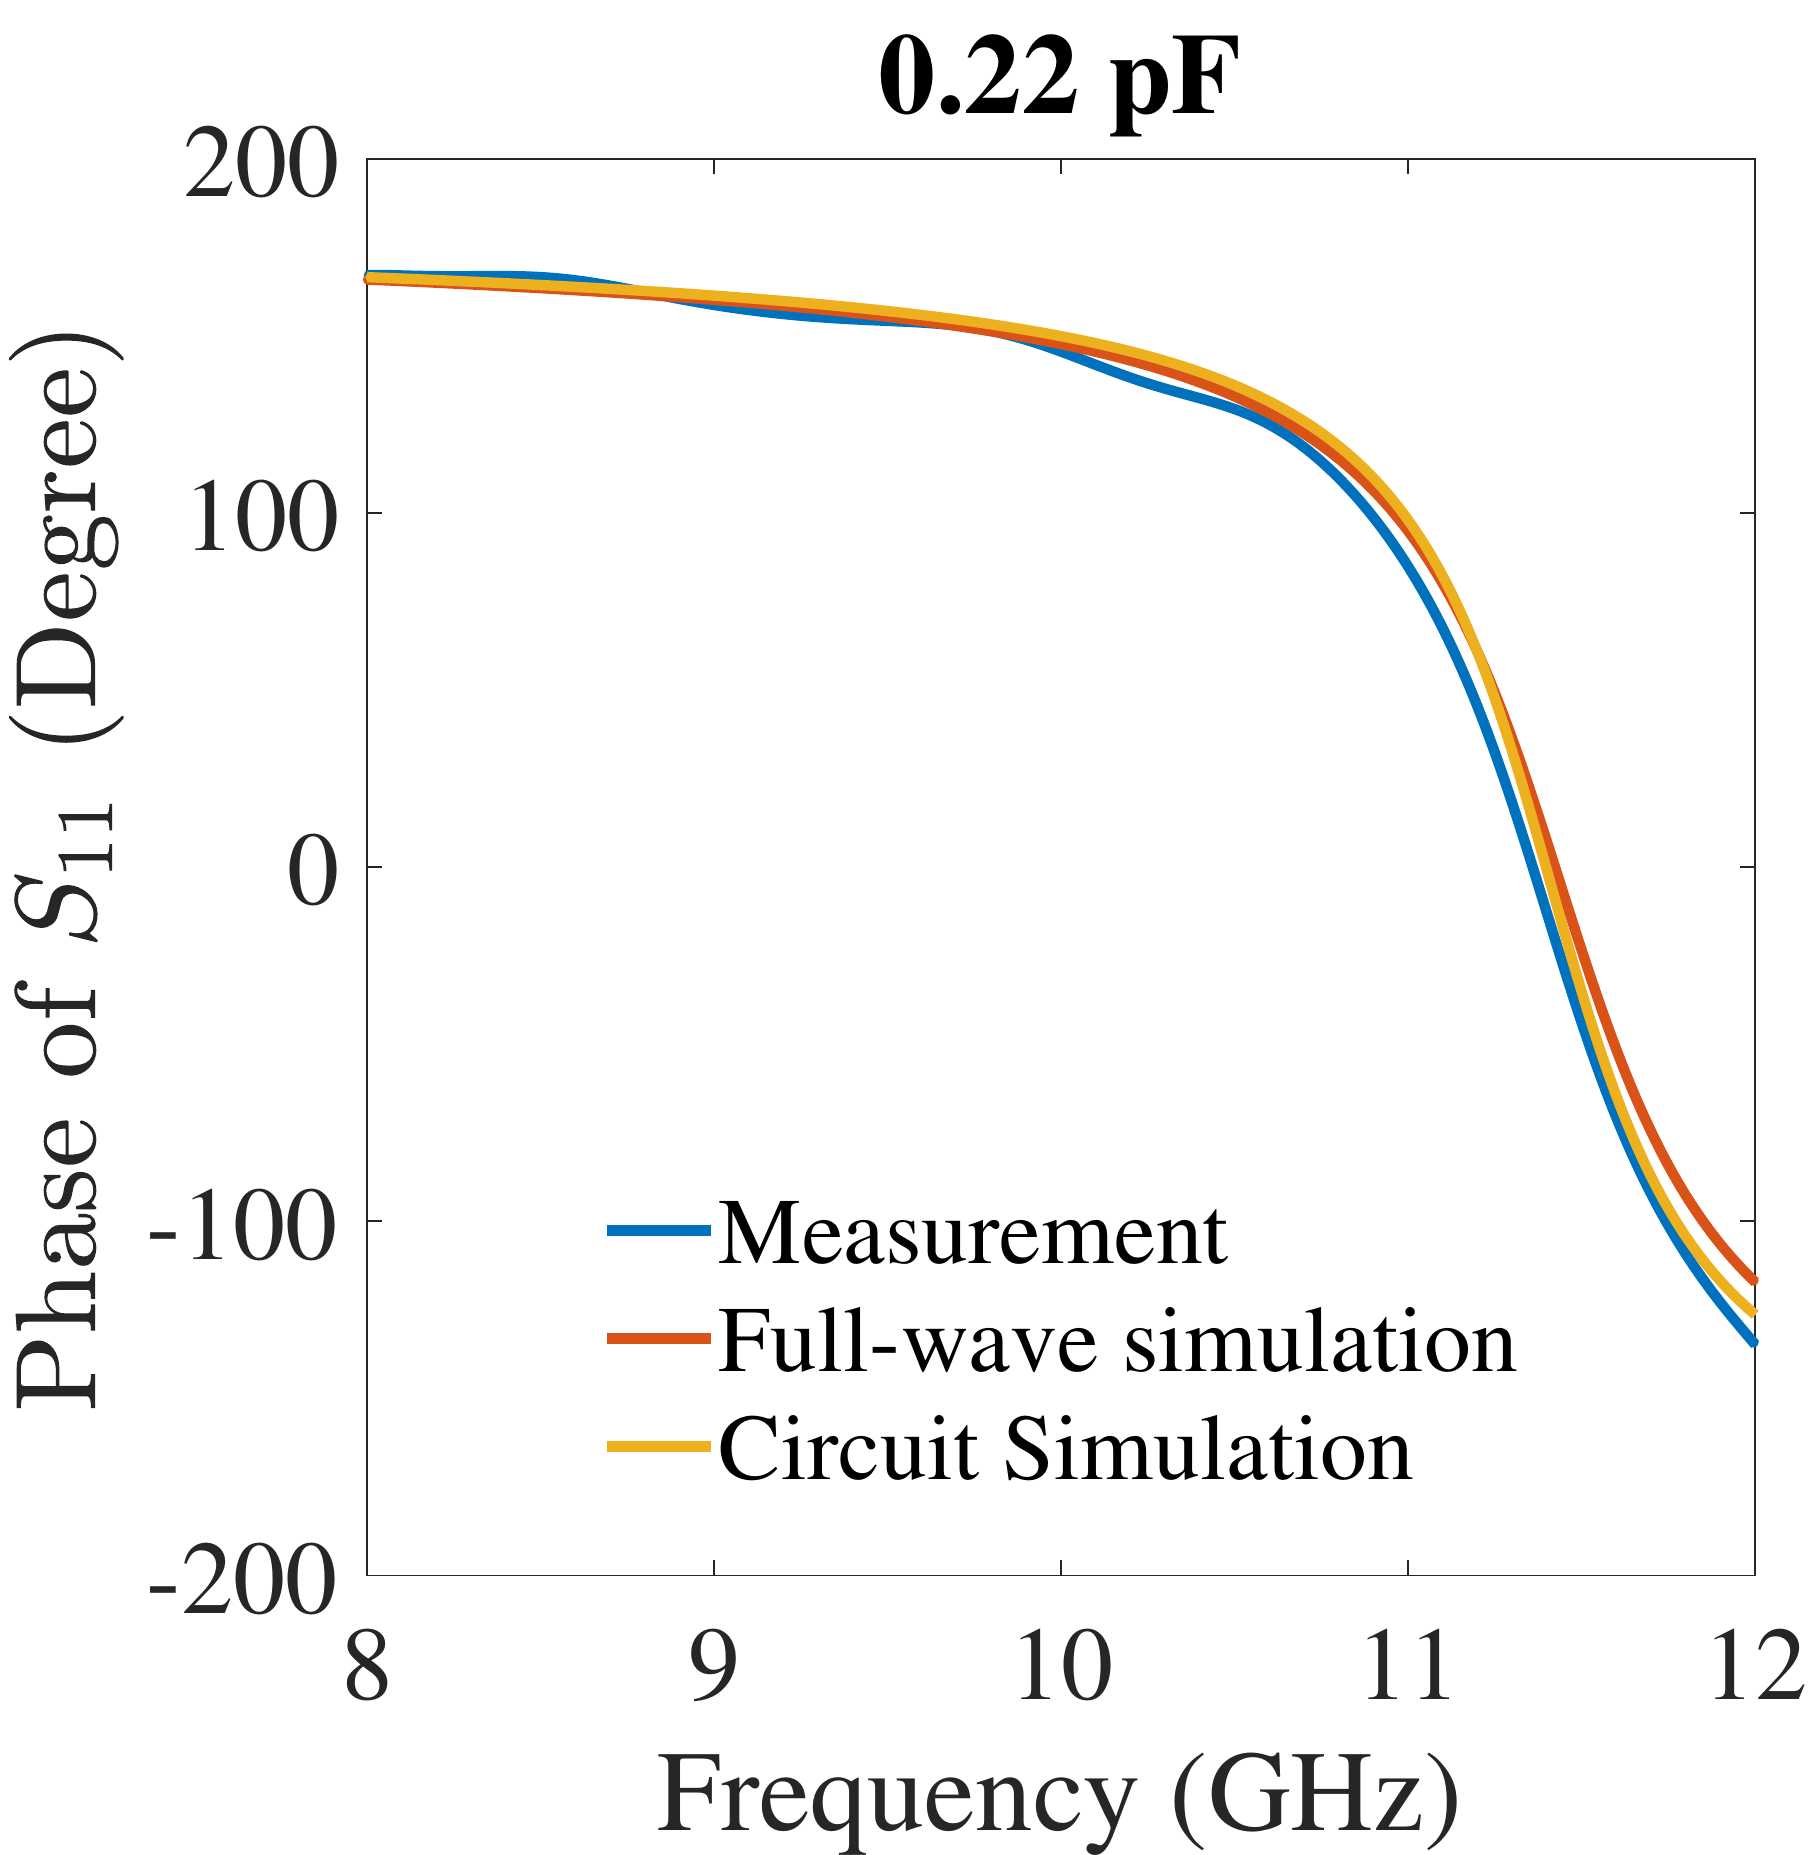}%
}\hfill
\subfloat[\label{sfig:DC9_P_TE}]{%
  \includegraphics[clip,width=0.165\columnwidth]{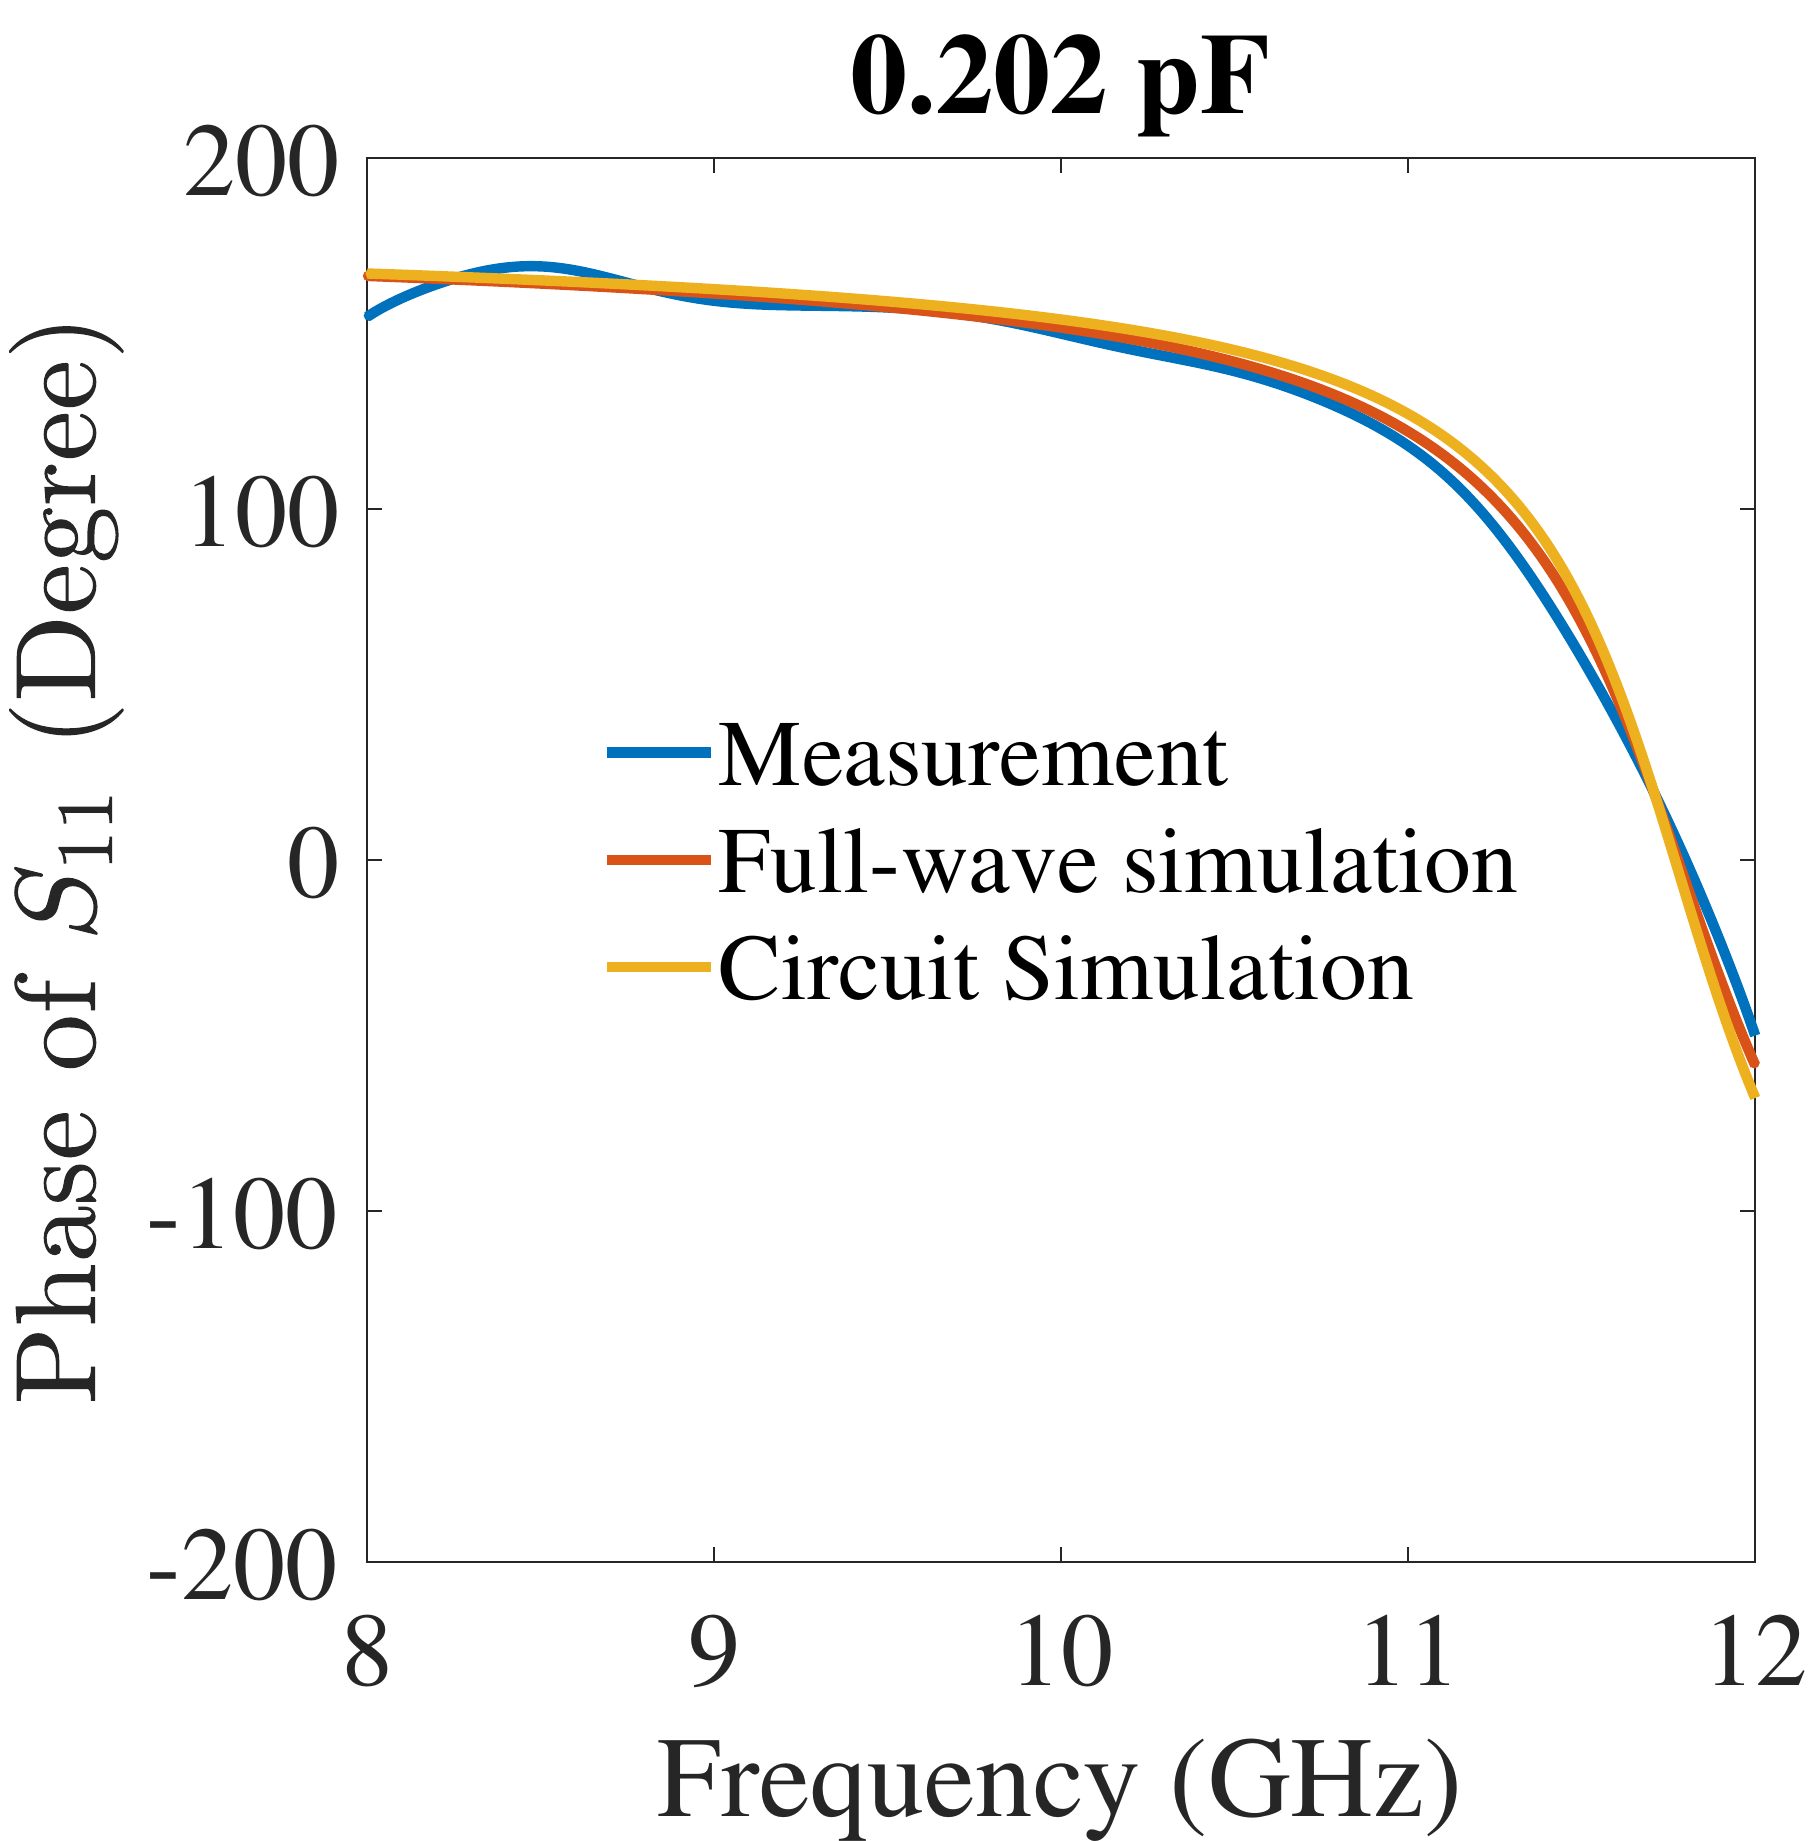}%
}\quad
\caption{Reflection phase and magnitude versus varactor capacitance for the realized metasurface from full-wave simulation, circuit model simulation and measurement under an oblique incident angle of $25^\circ$. Results are shown for a TE polarization.}
\label{fig:DCPerformance_TE}
\end{figure} 

\begin{figure}[t!]
\subfloat[\label{sfig:DC4_M_TM}]{%
  \includegraphics[clip,width=0.165\columnwidth]{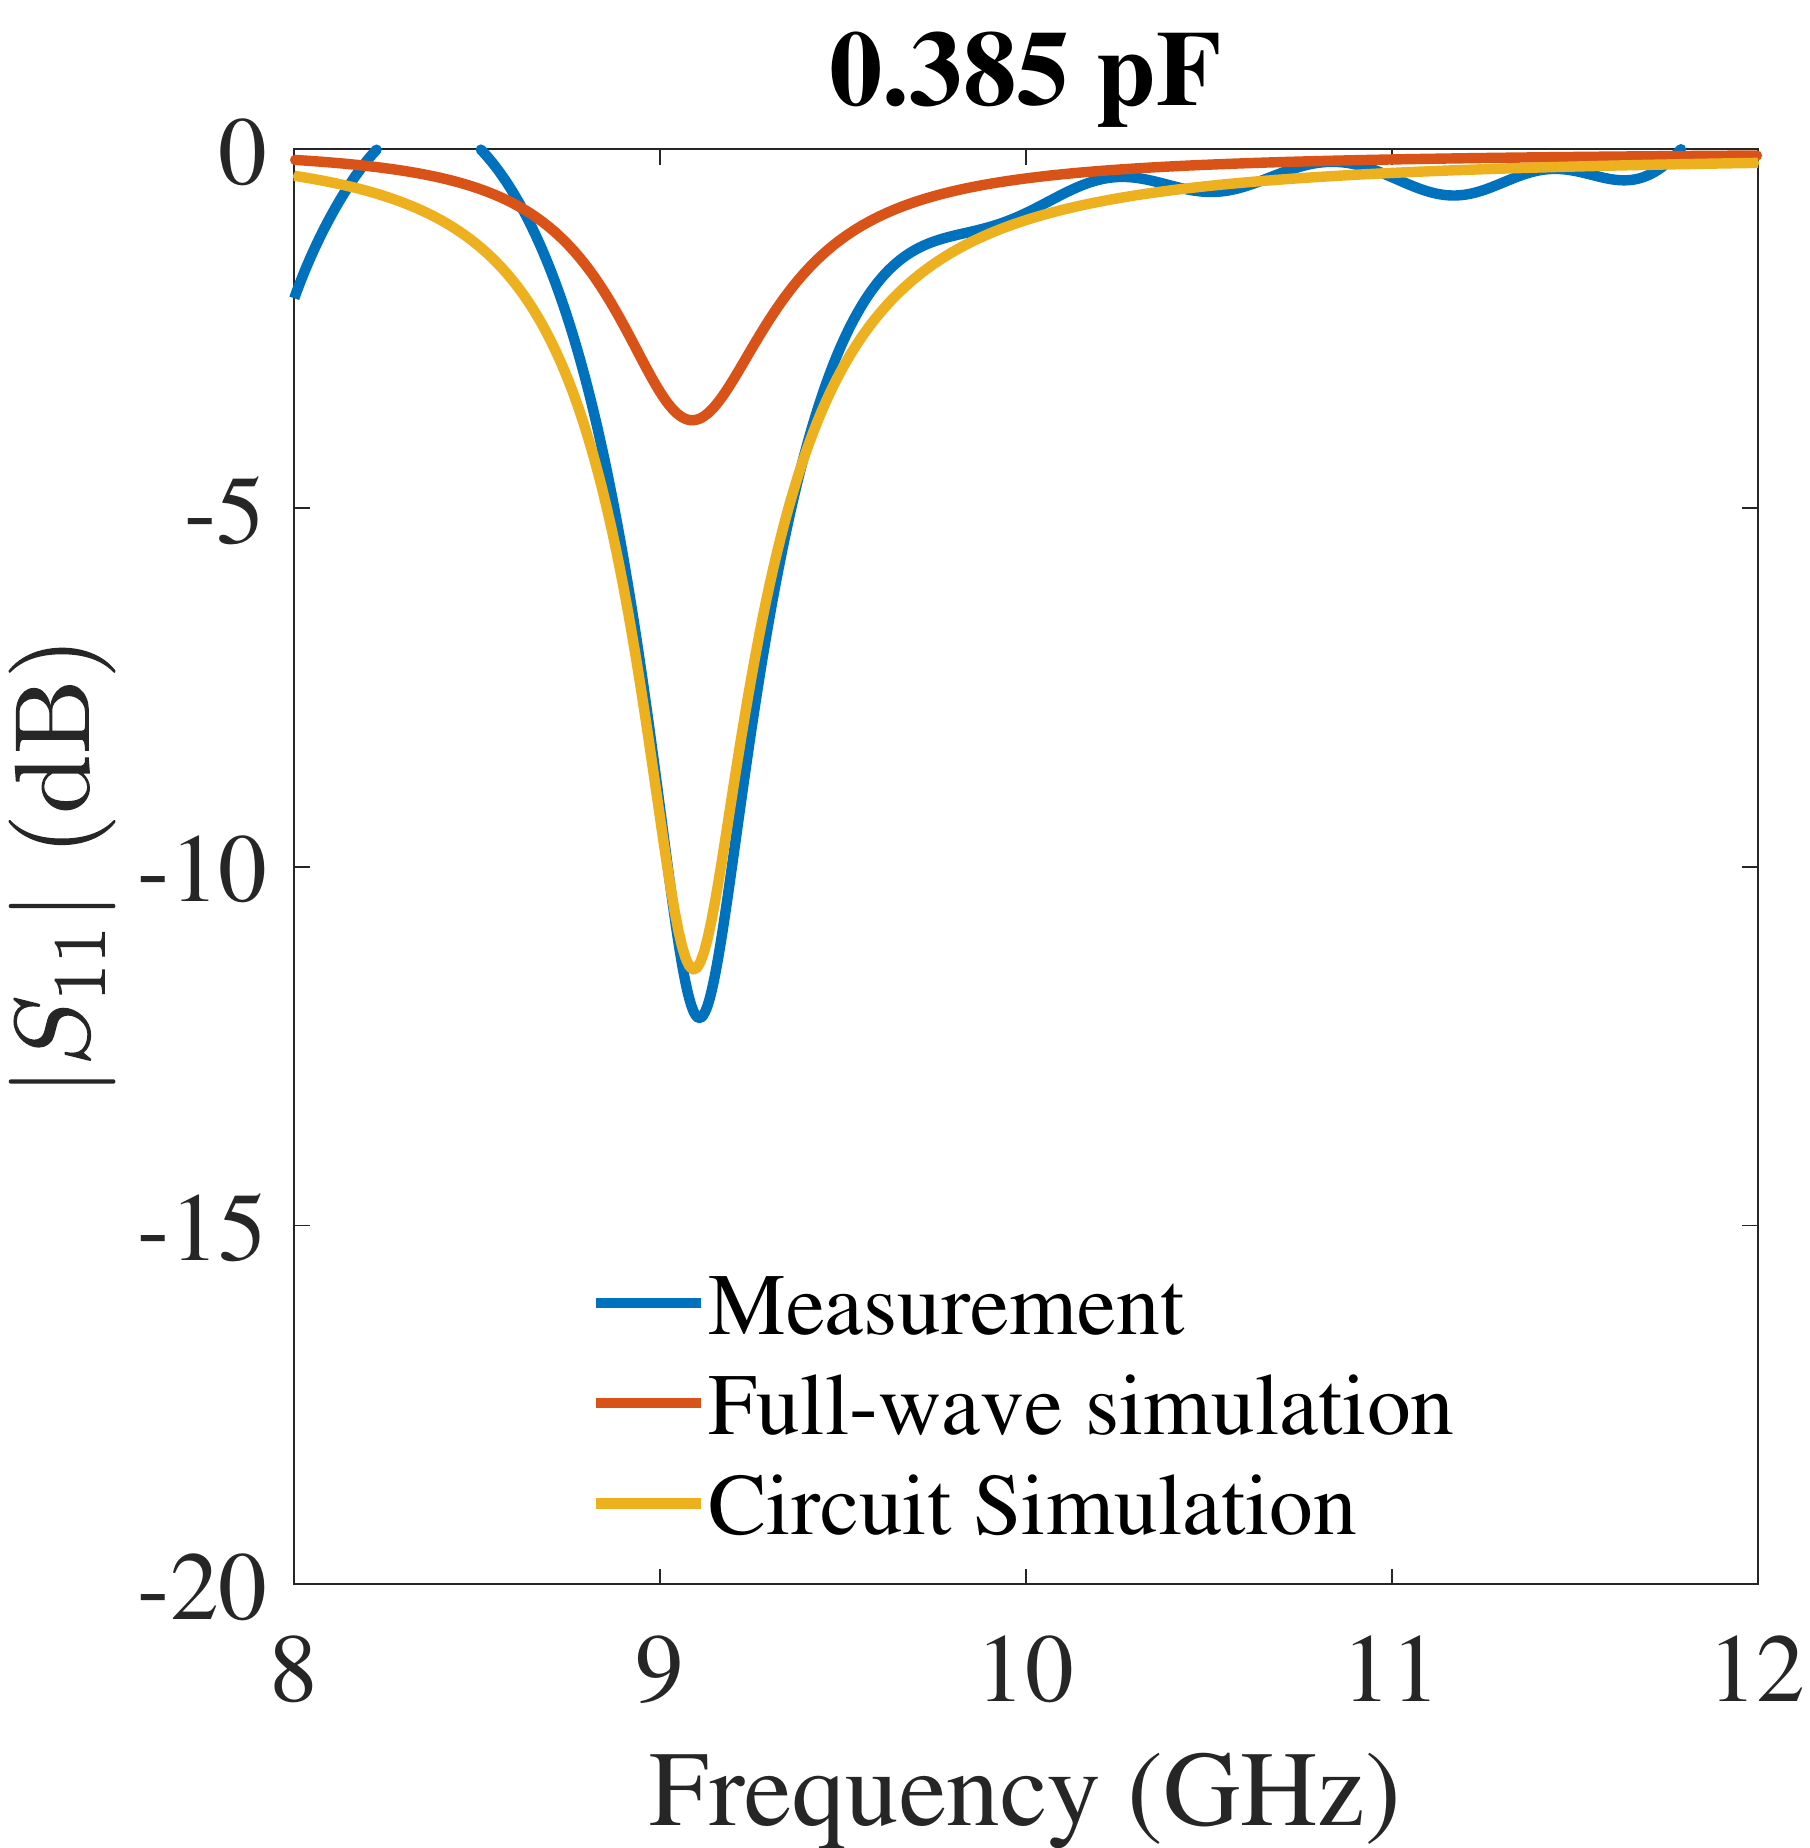}%
}\hfill
\subfloat[\label{sfig:DC5_M_TM}]{%
  \includegraphics[clip,width=0.165\columnwidth]{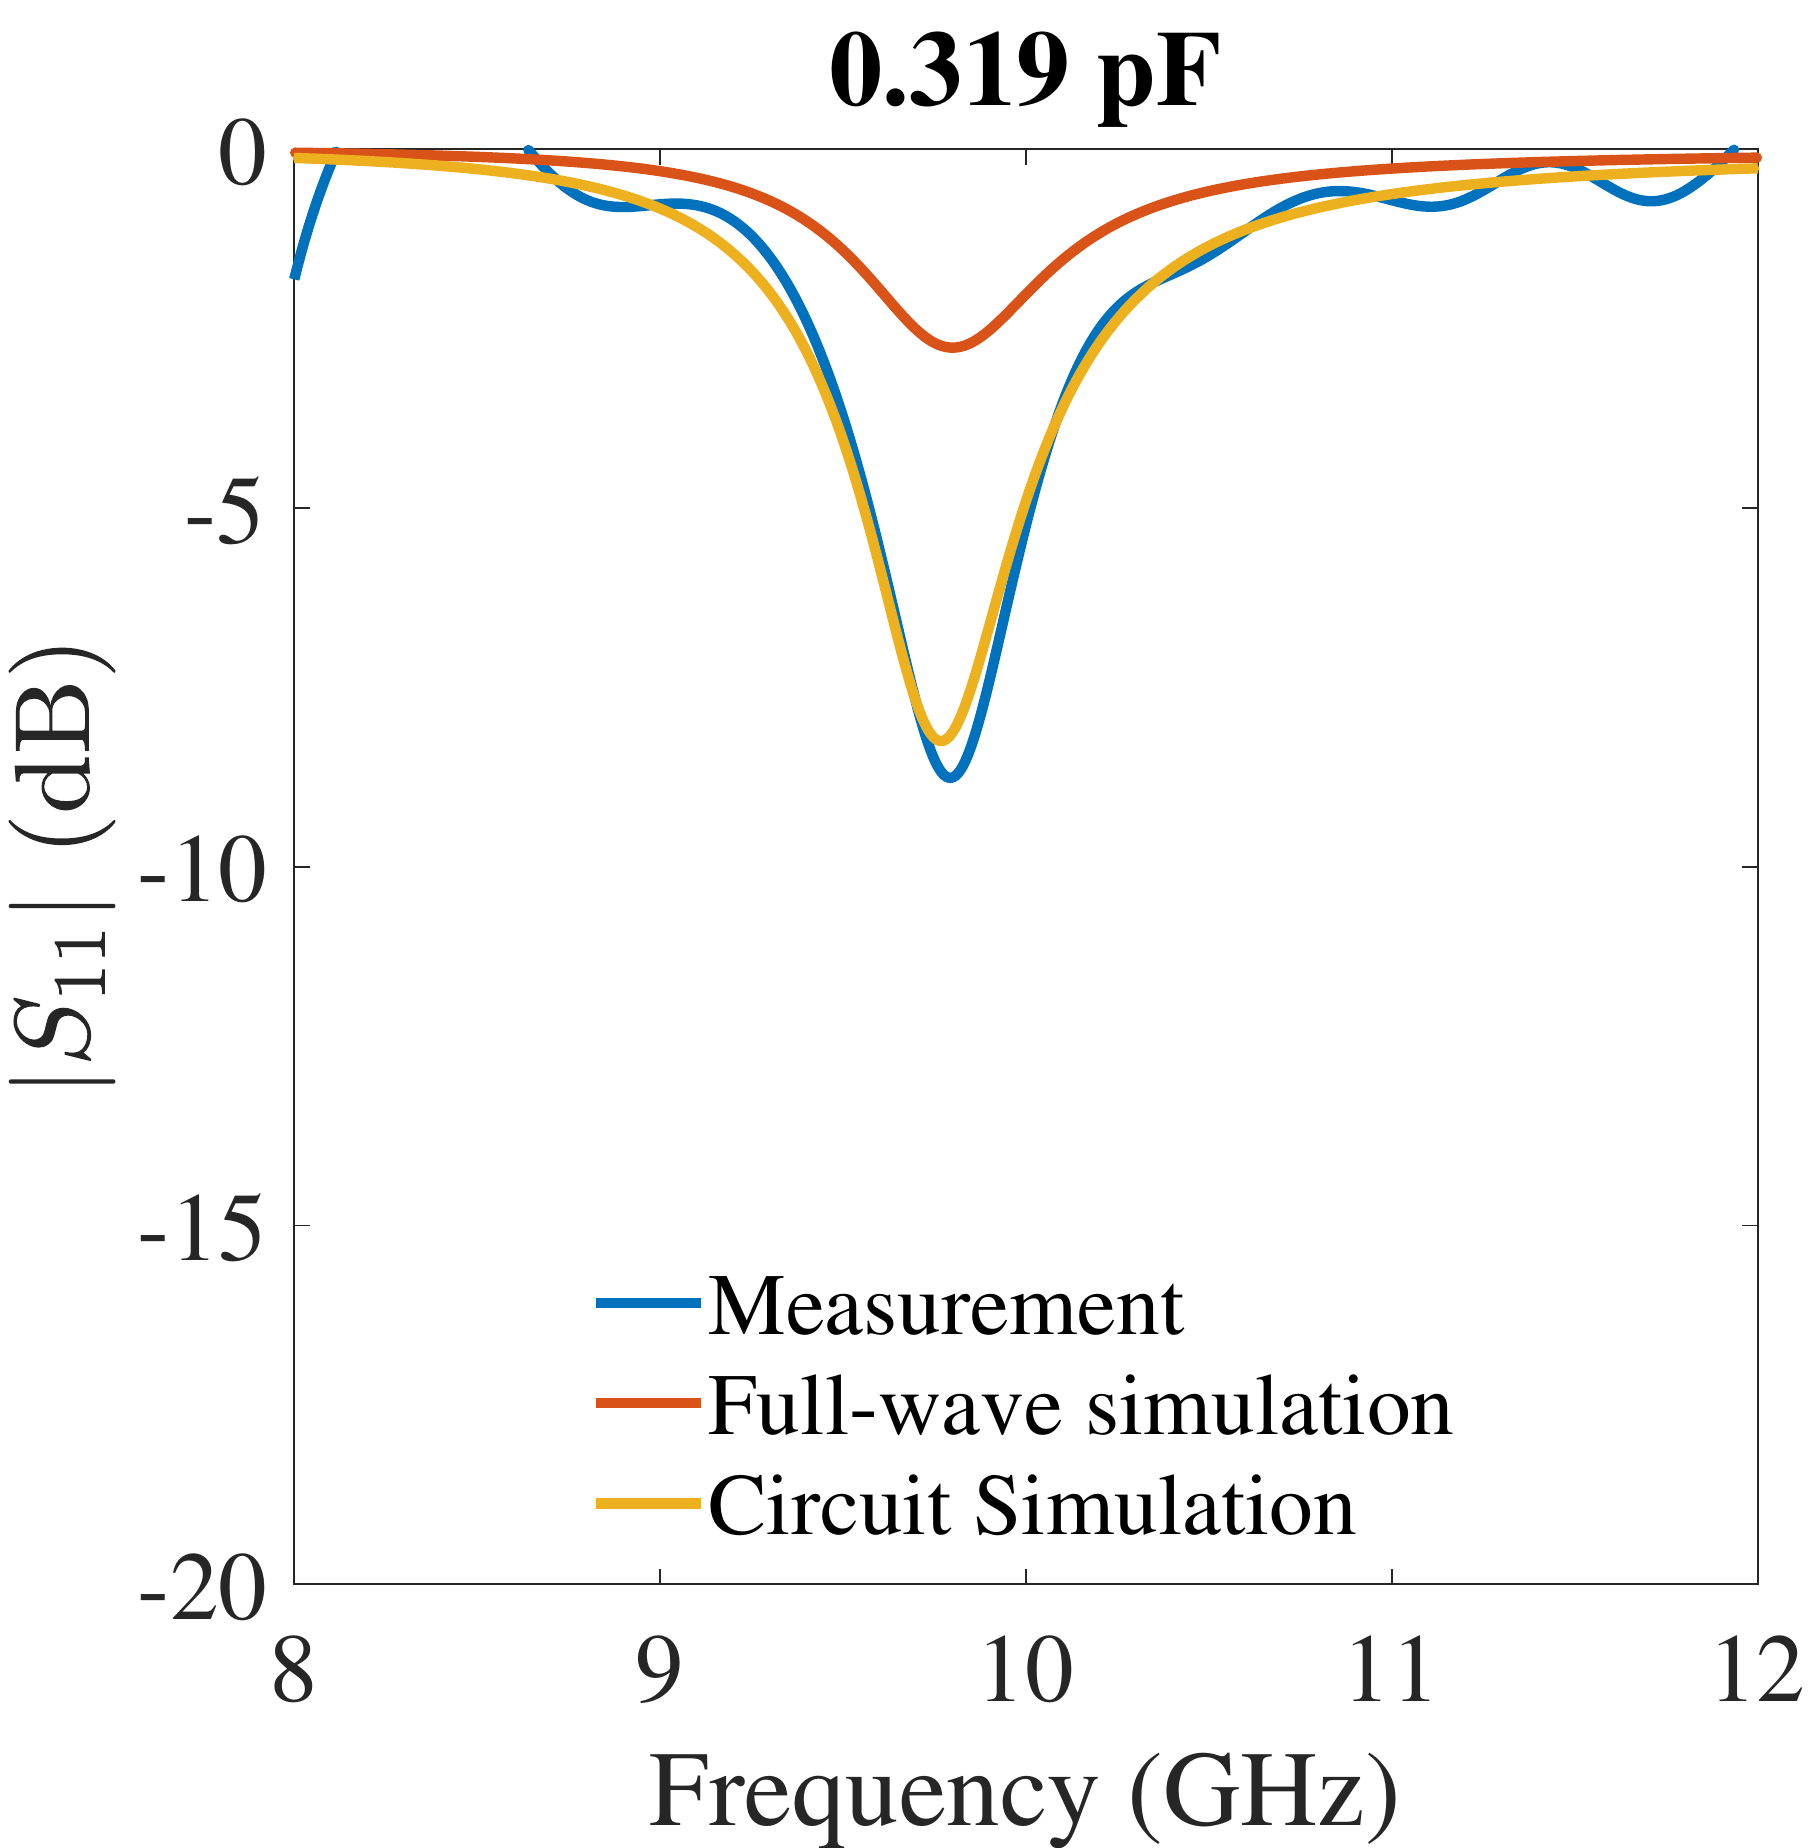}%
}\hfill
\subfloat[\label{sfig:DC6_M_TM}]{%
  \includegraphics[clip,width=0.165\columnwidth]{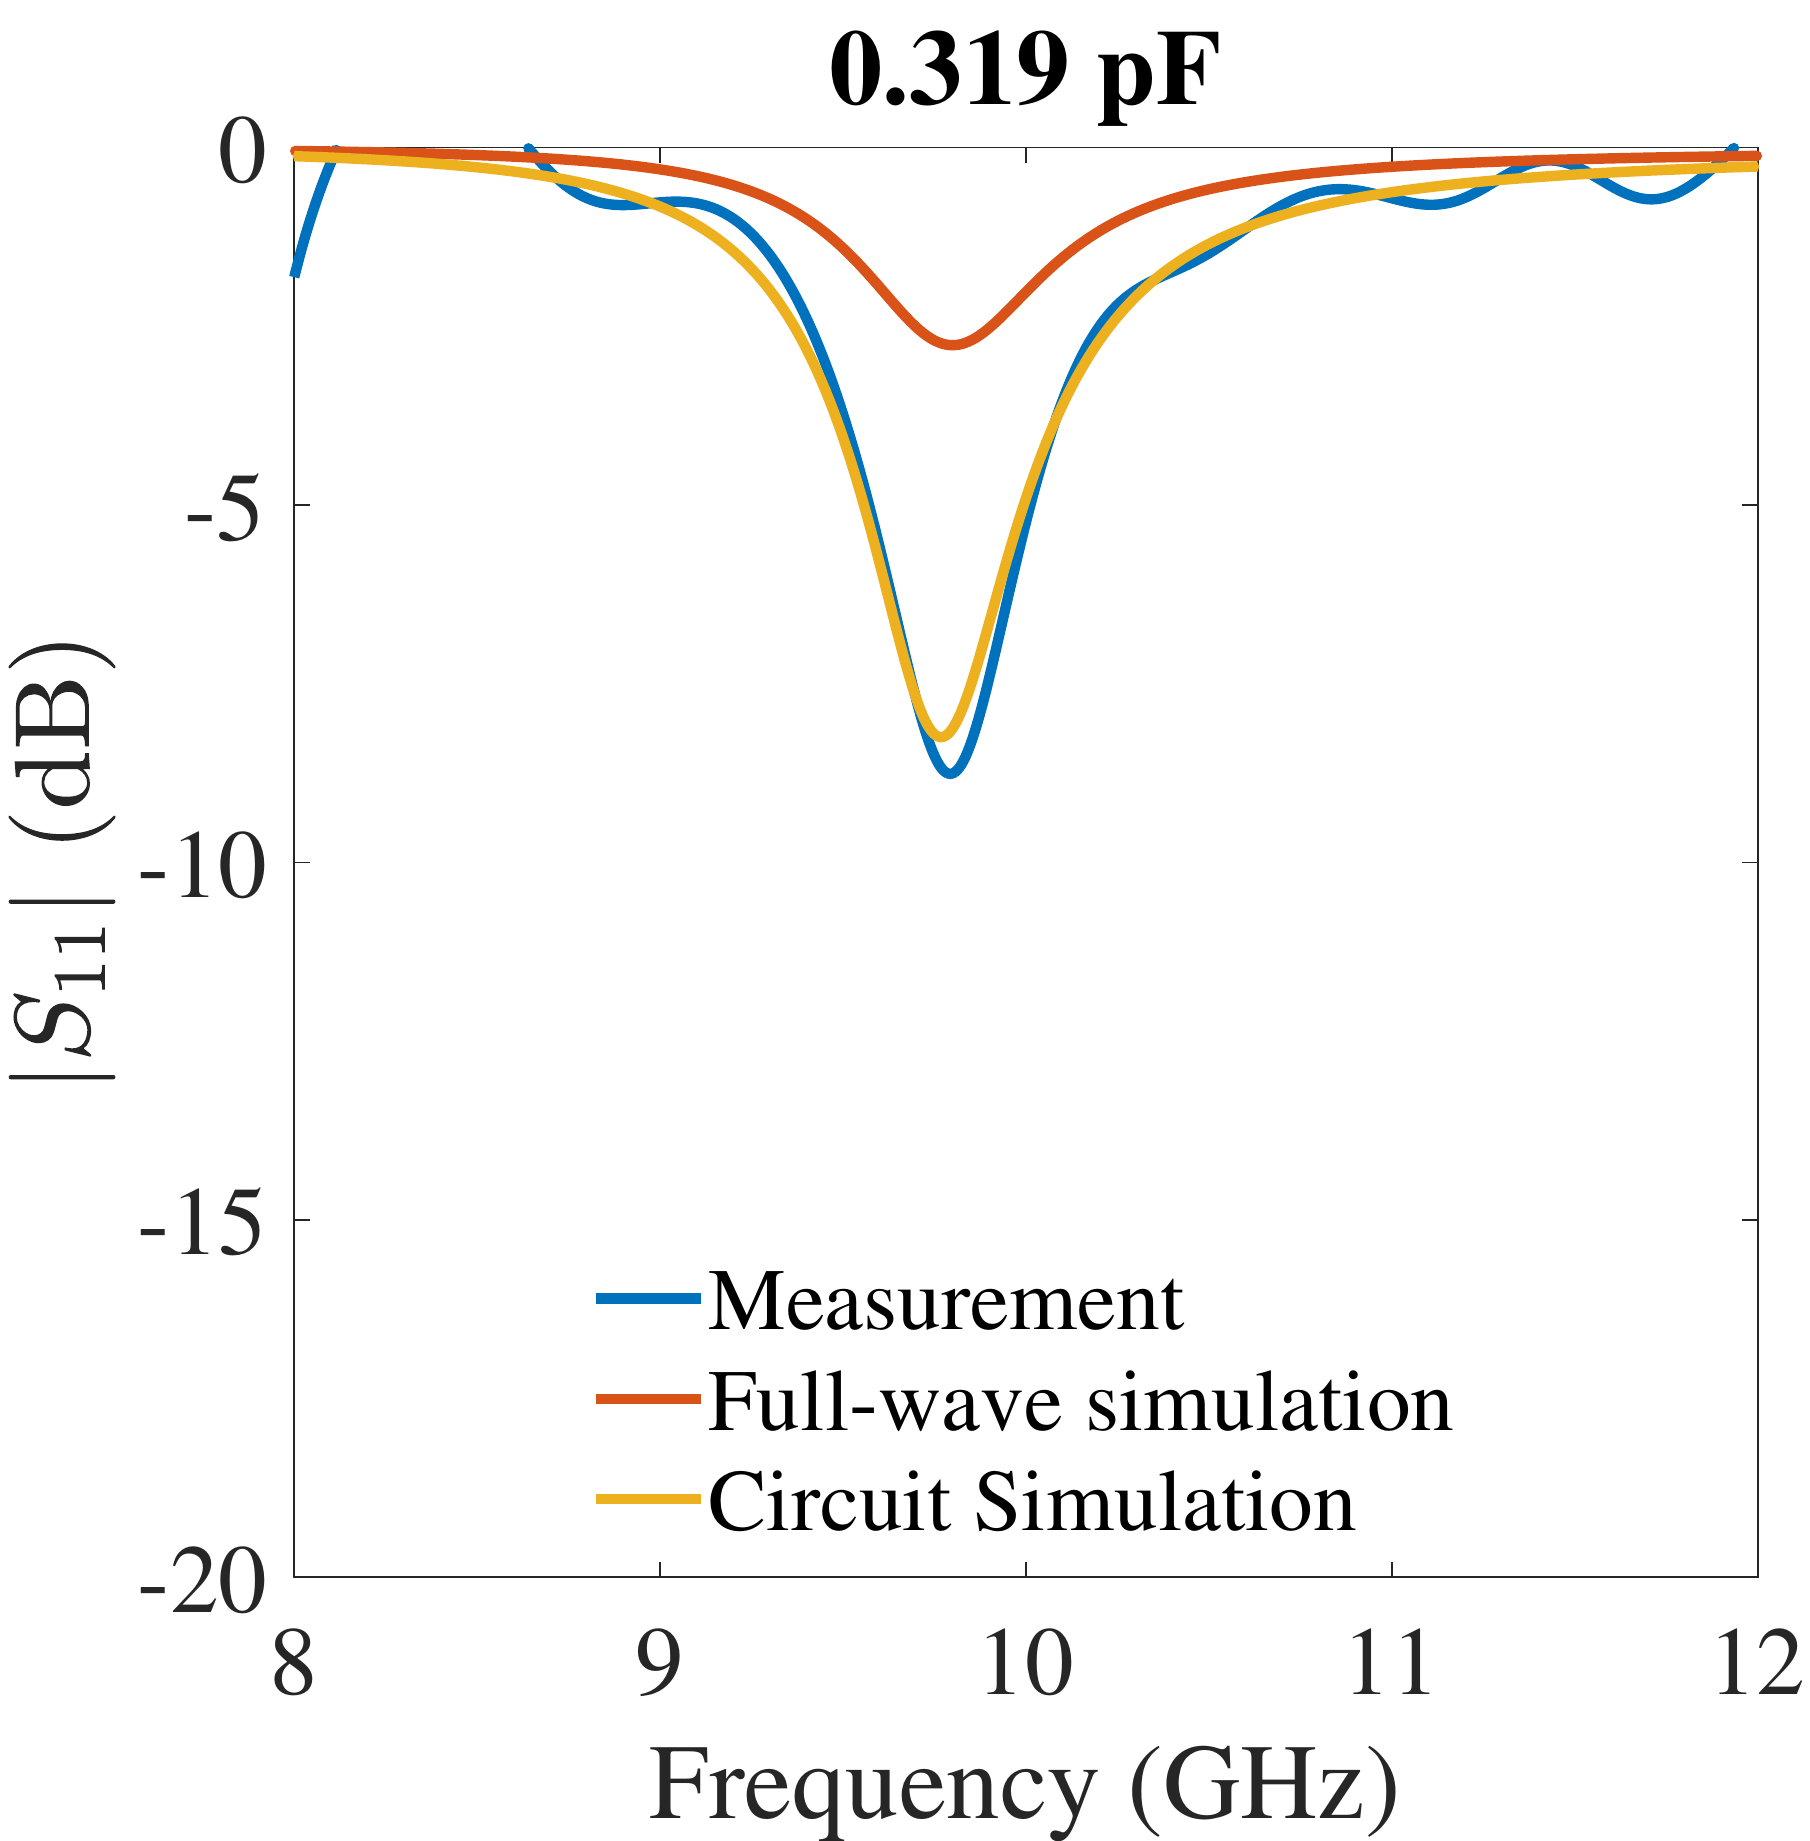}%
}\hfill
\subfloat[\label{sfig:DC7_M_TM}]{%
  \includegraphics[clip,width=0.165\columnwidth]{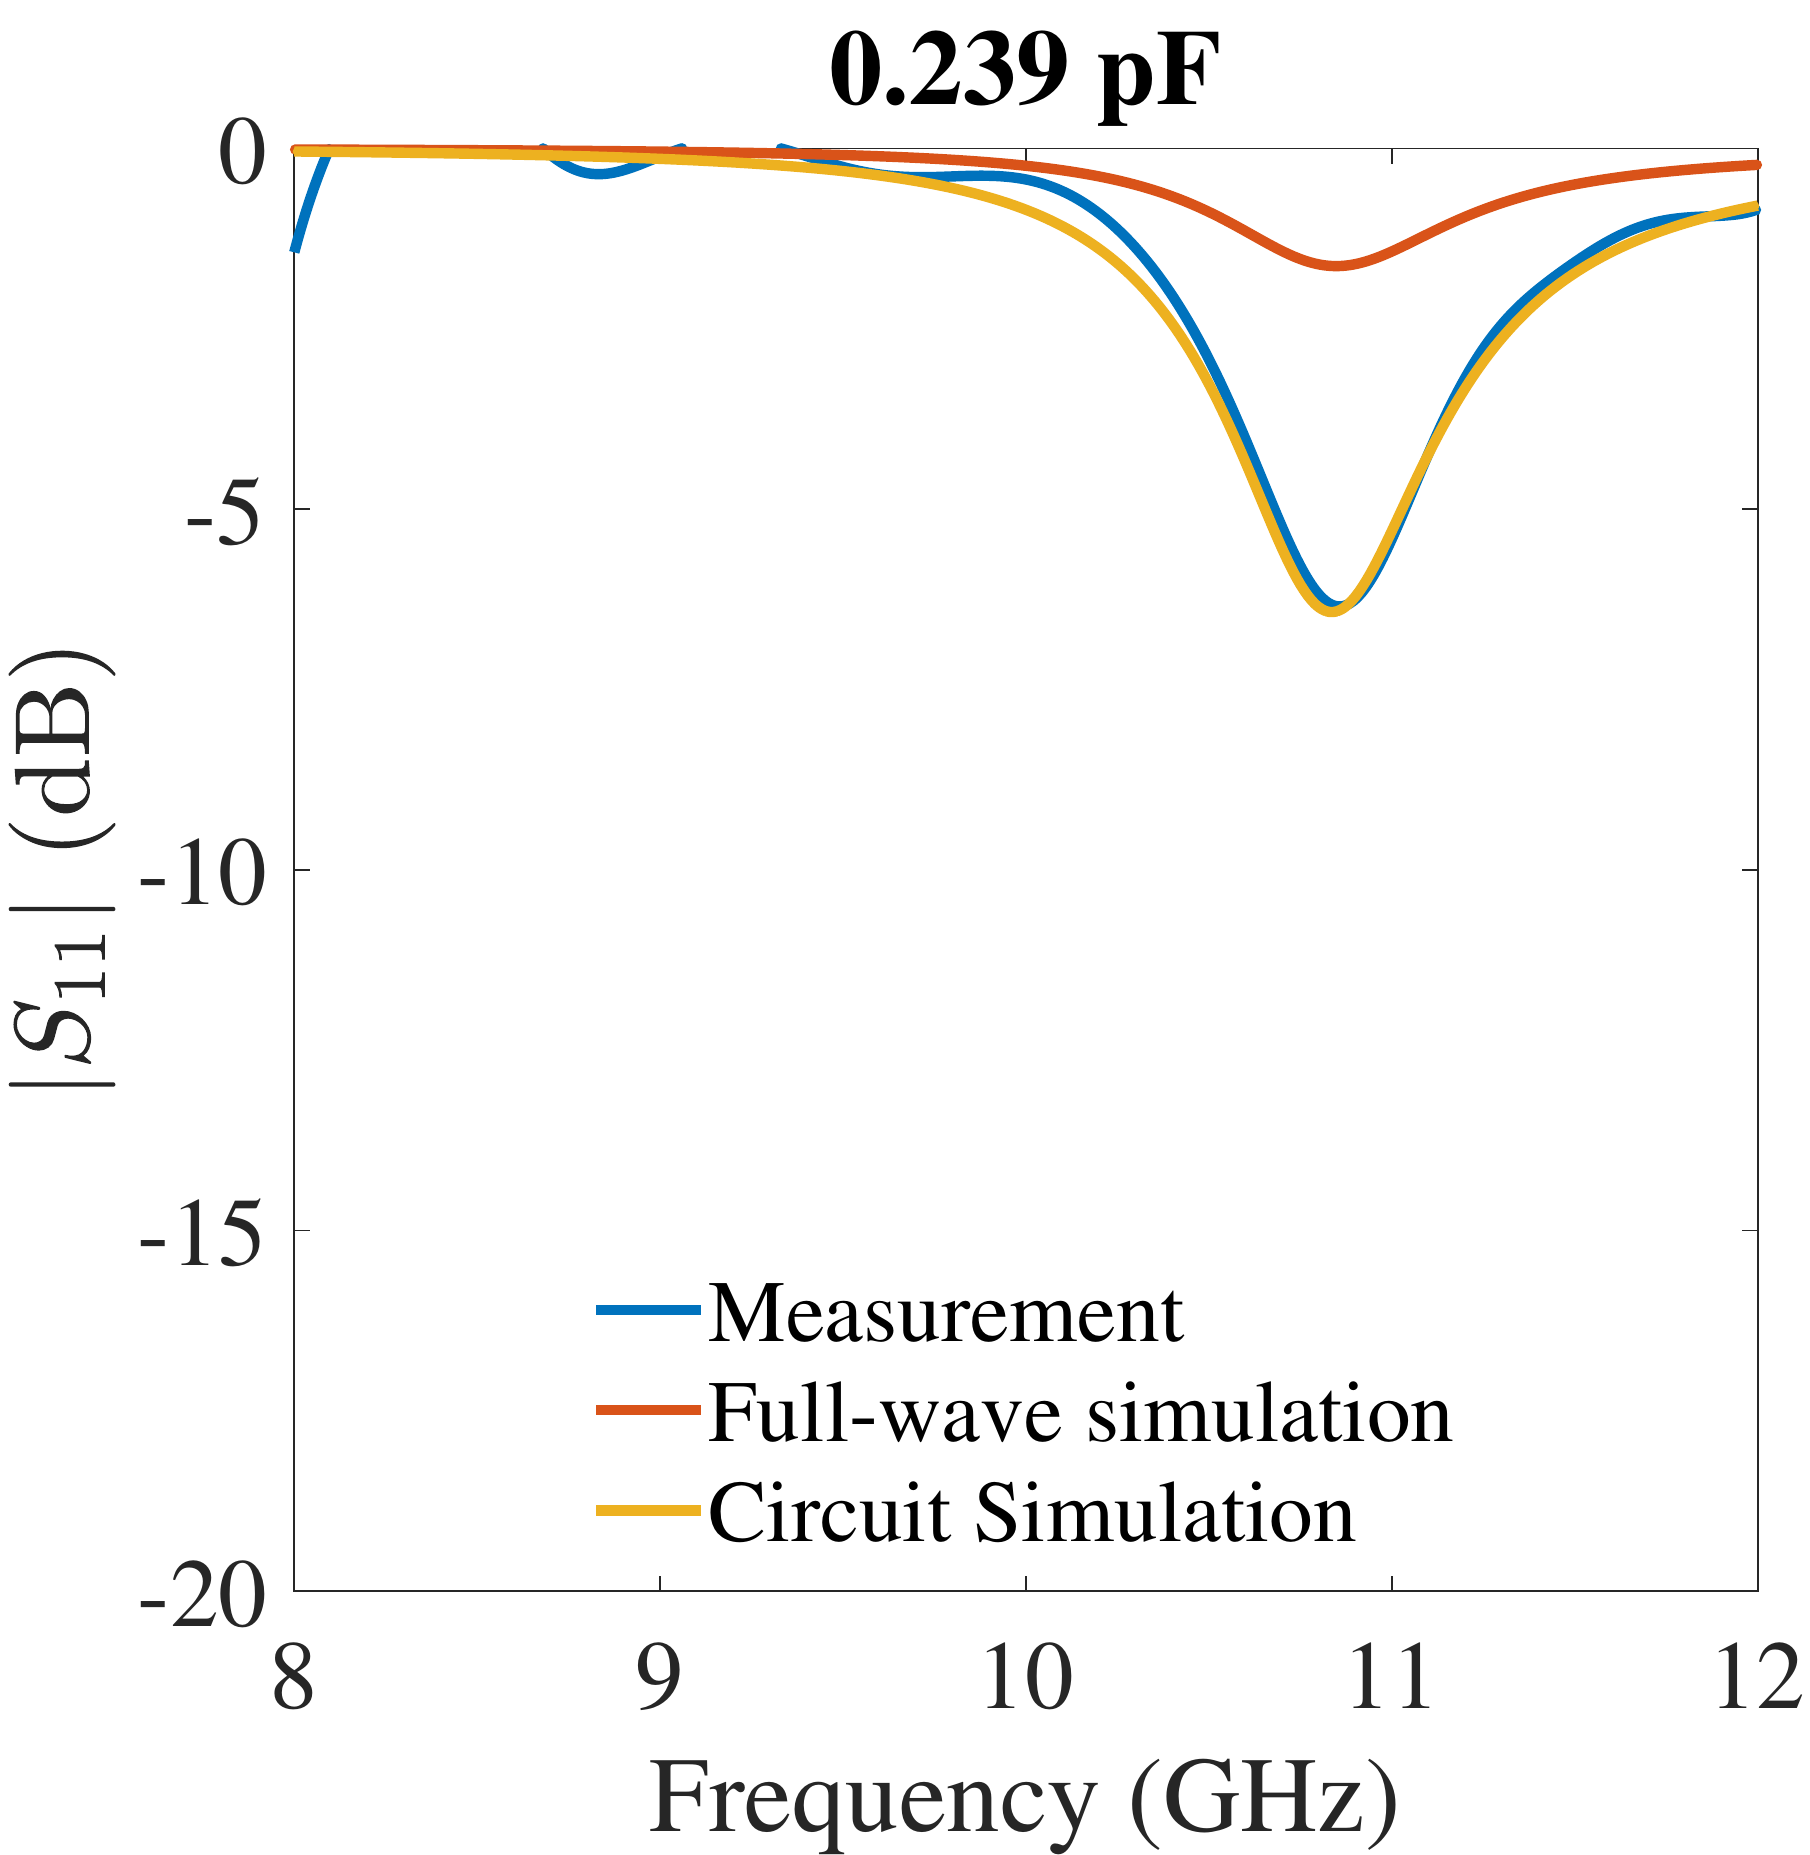}%
}\hfill
\subfloat[\label{sfig:DC8_M_TM}]{%
  \includegraphics[clip,width=0.165\columnwidth]{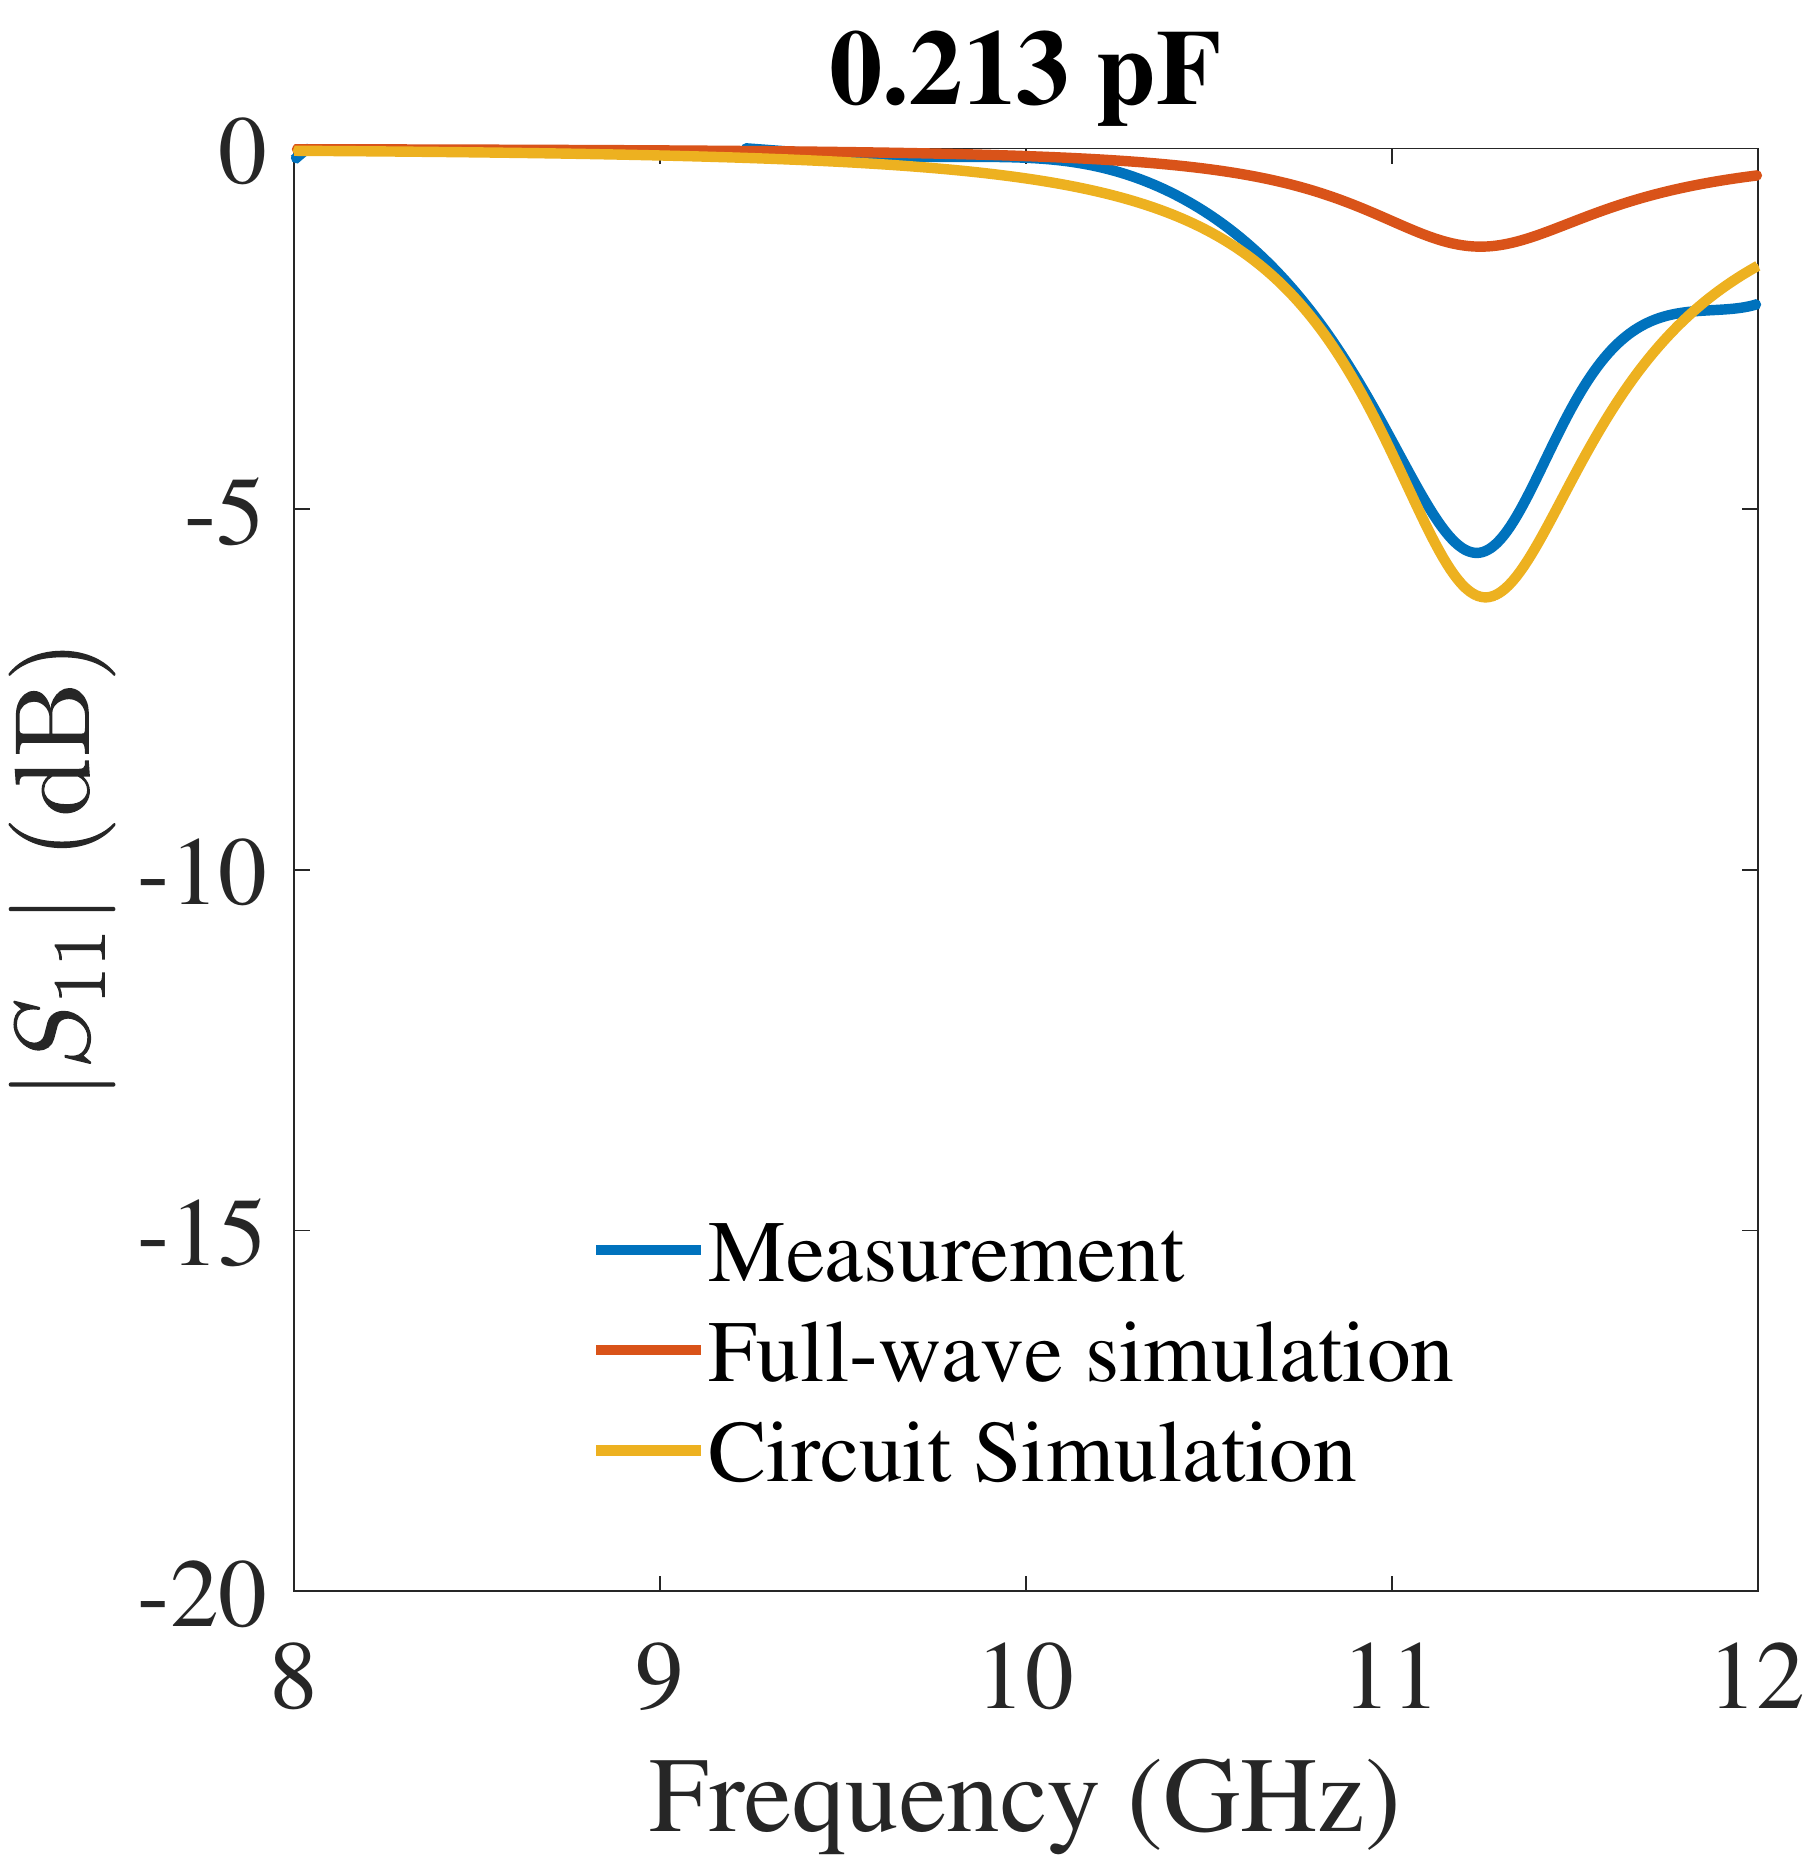}%
}\hfill
\subfloat[\label{sfig:DC9_M_TM}]{%
  \includegraphics[clip,width=0.165\columnwidth]{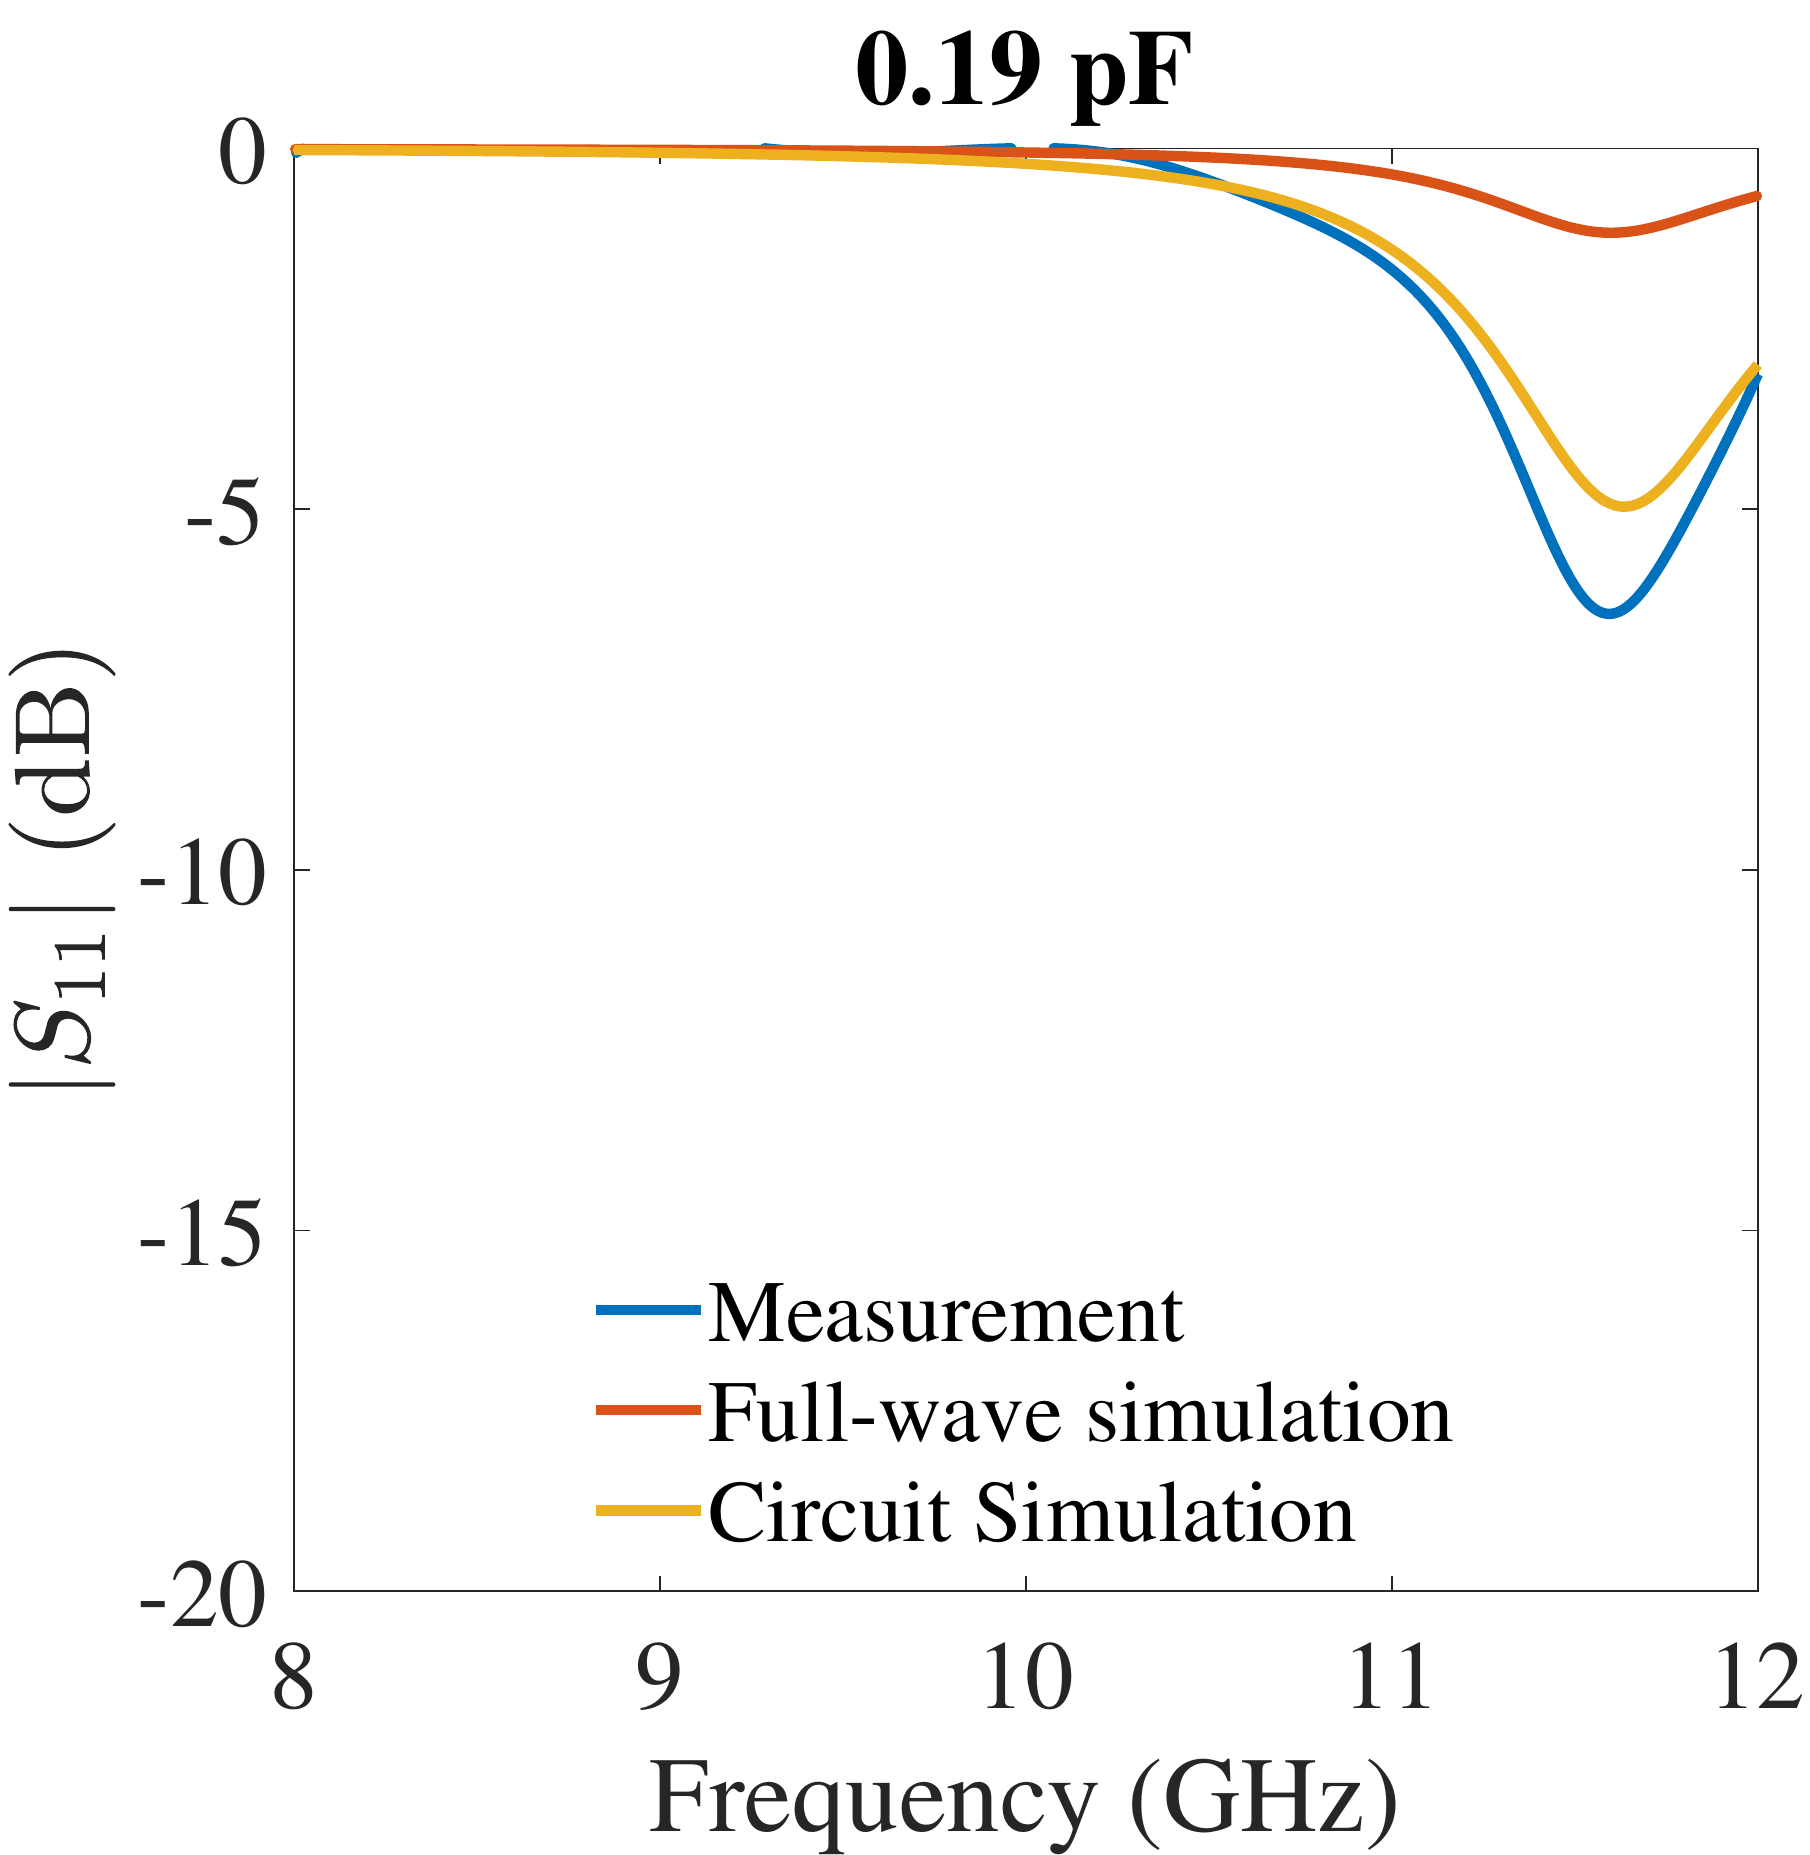}%
}\quad
\subfloat[\label{sfig:DC4_P_TM}]{%
  \includegraphics[clip,width=0.165\columnwidth]{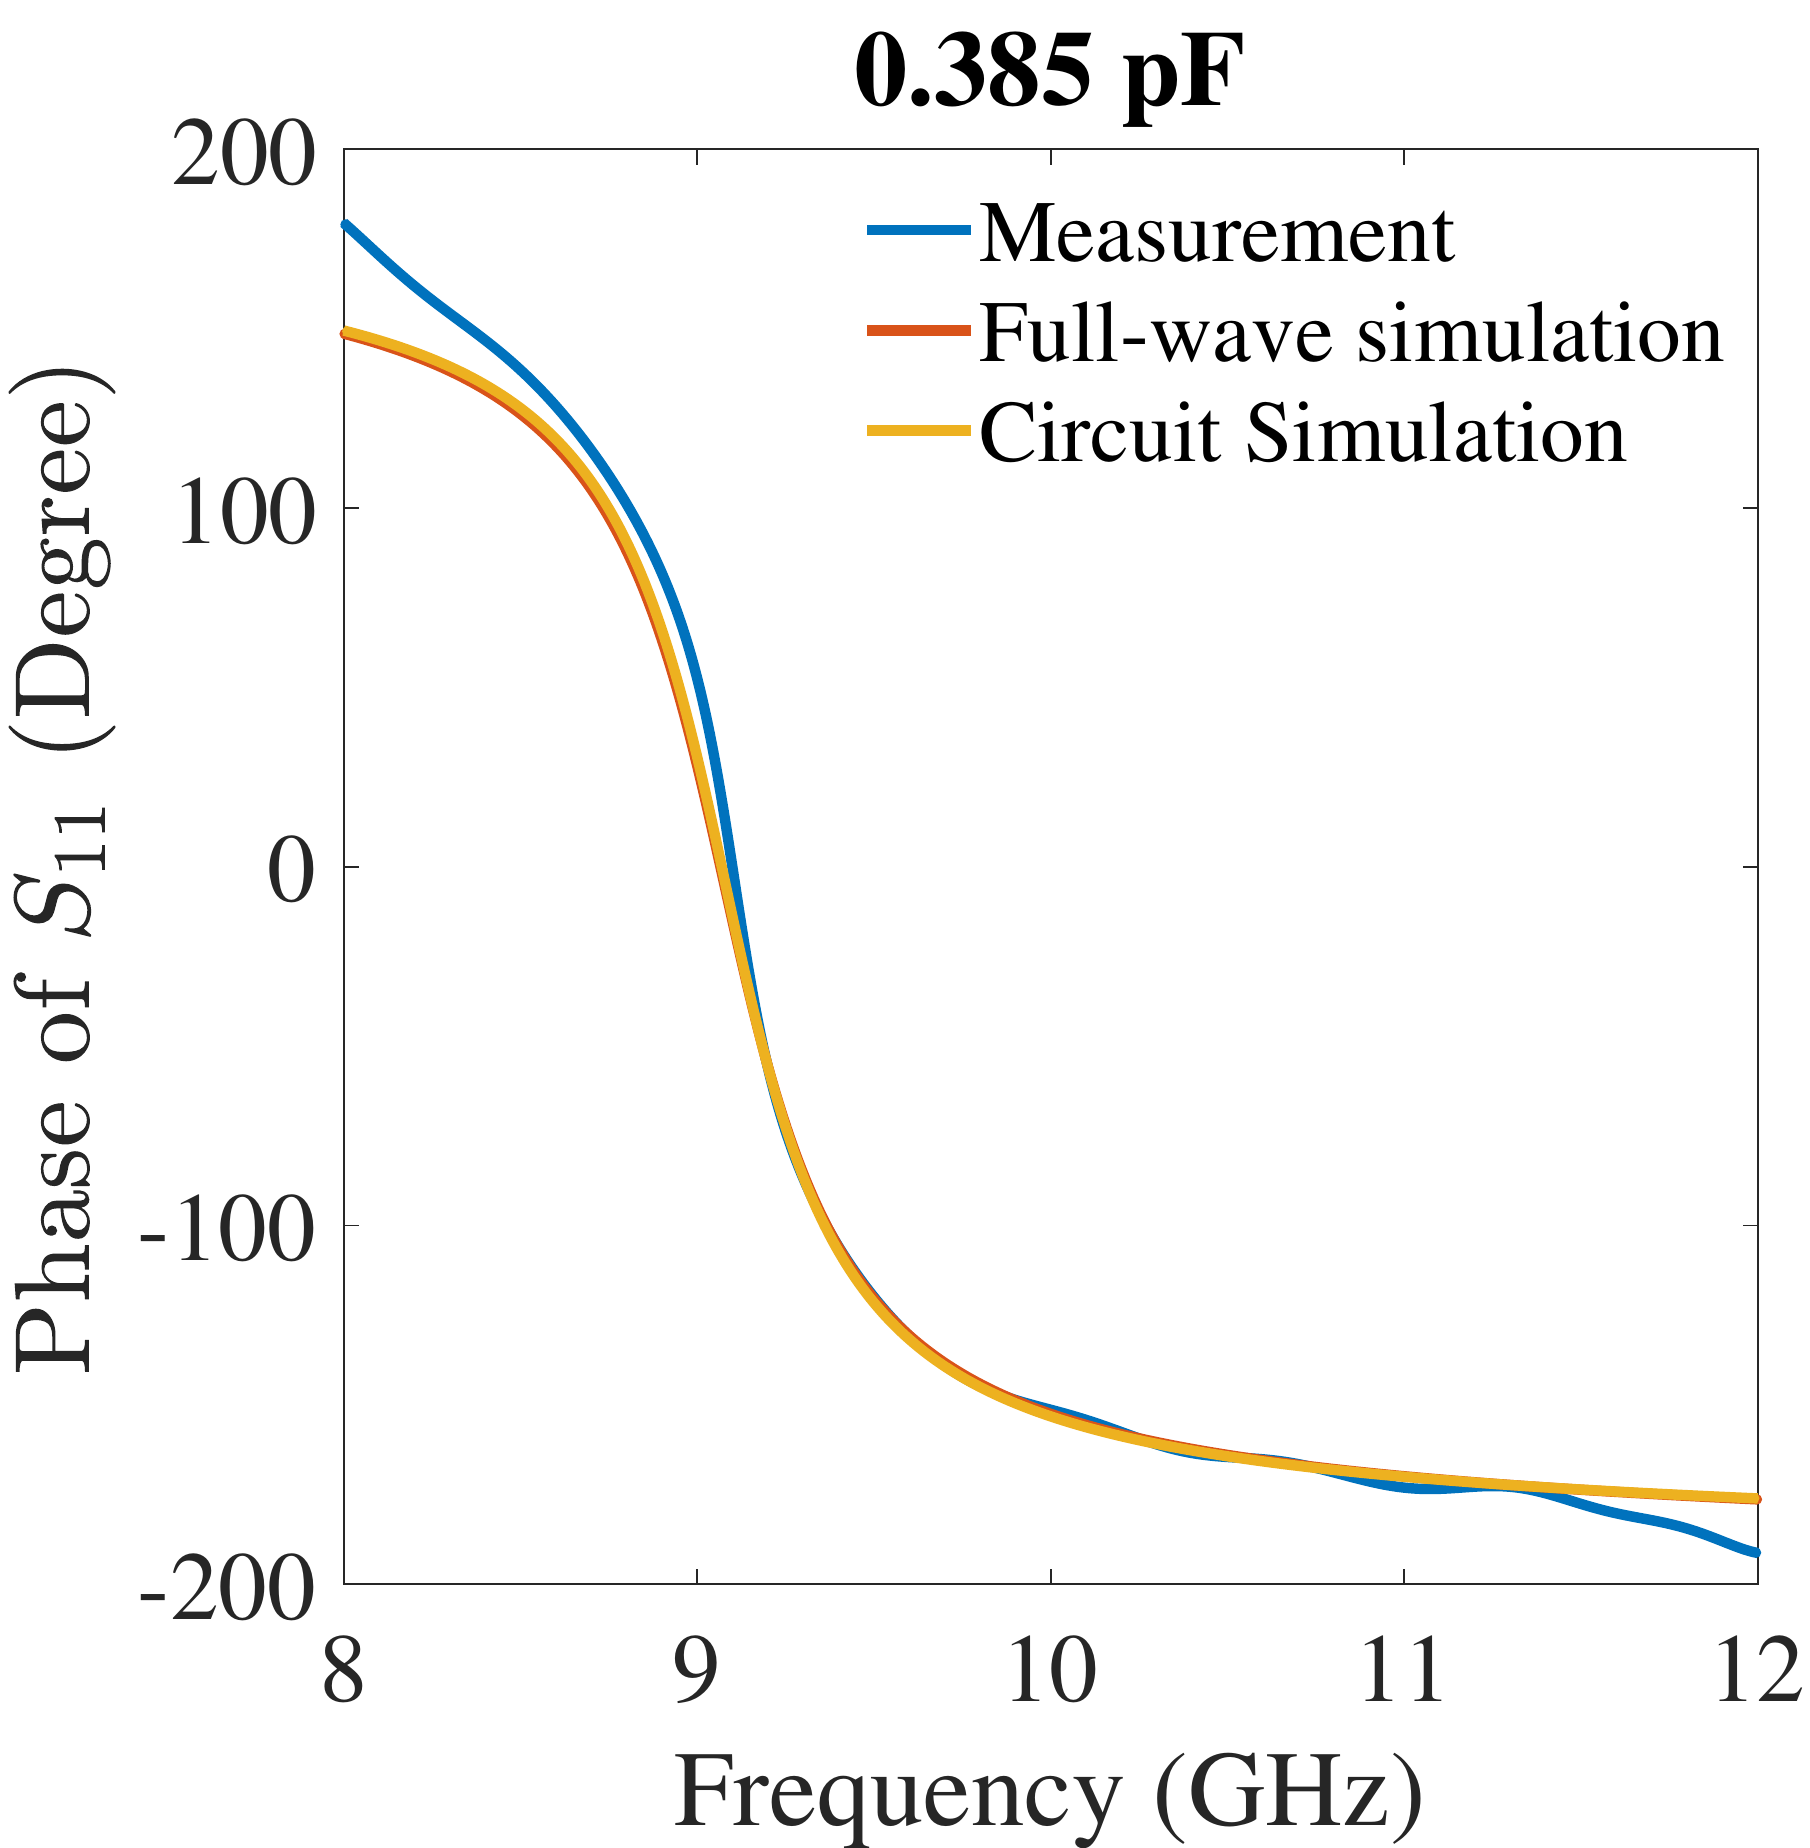}%
}\hfill
\subfloat[\label{sfig:DC5_P_TE}]{%
  \includegraphics[clip,width=0.165\columnwidth]{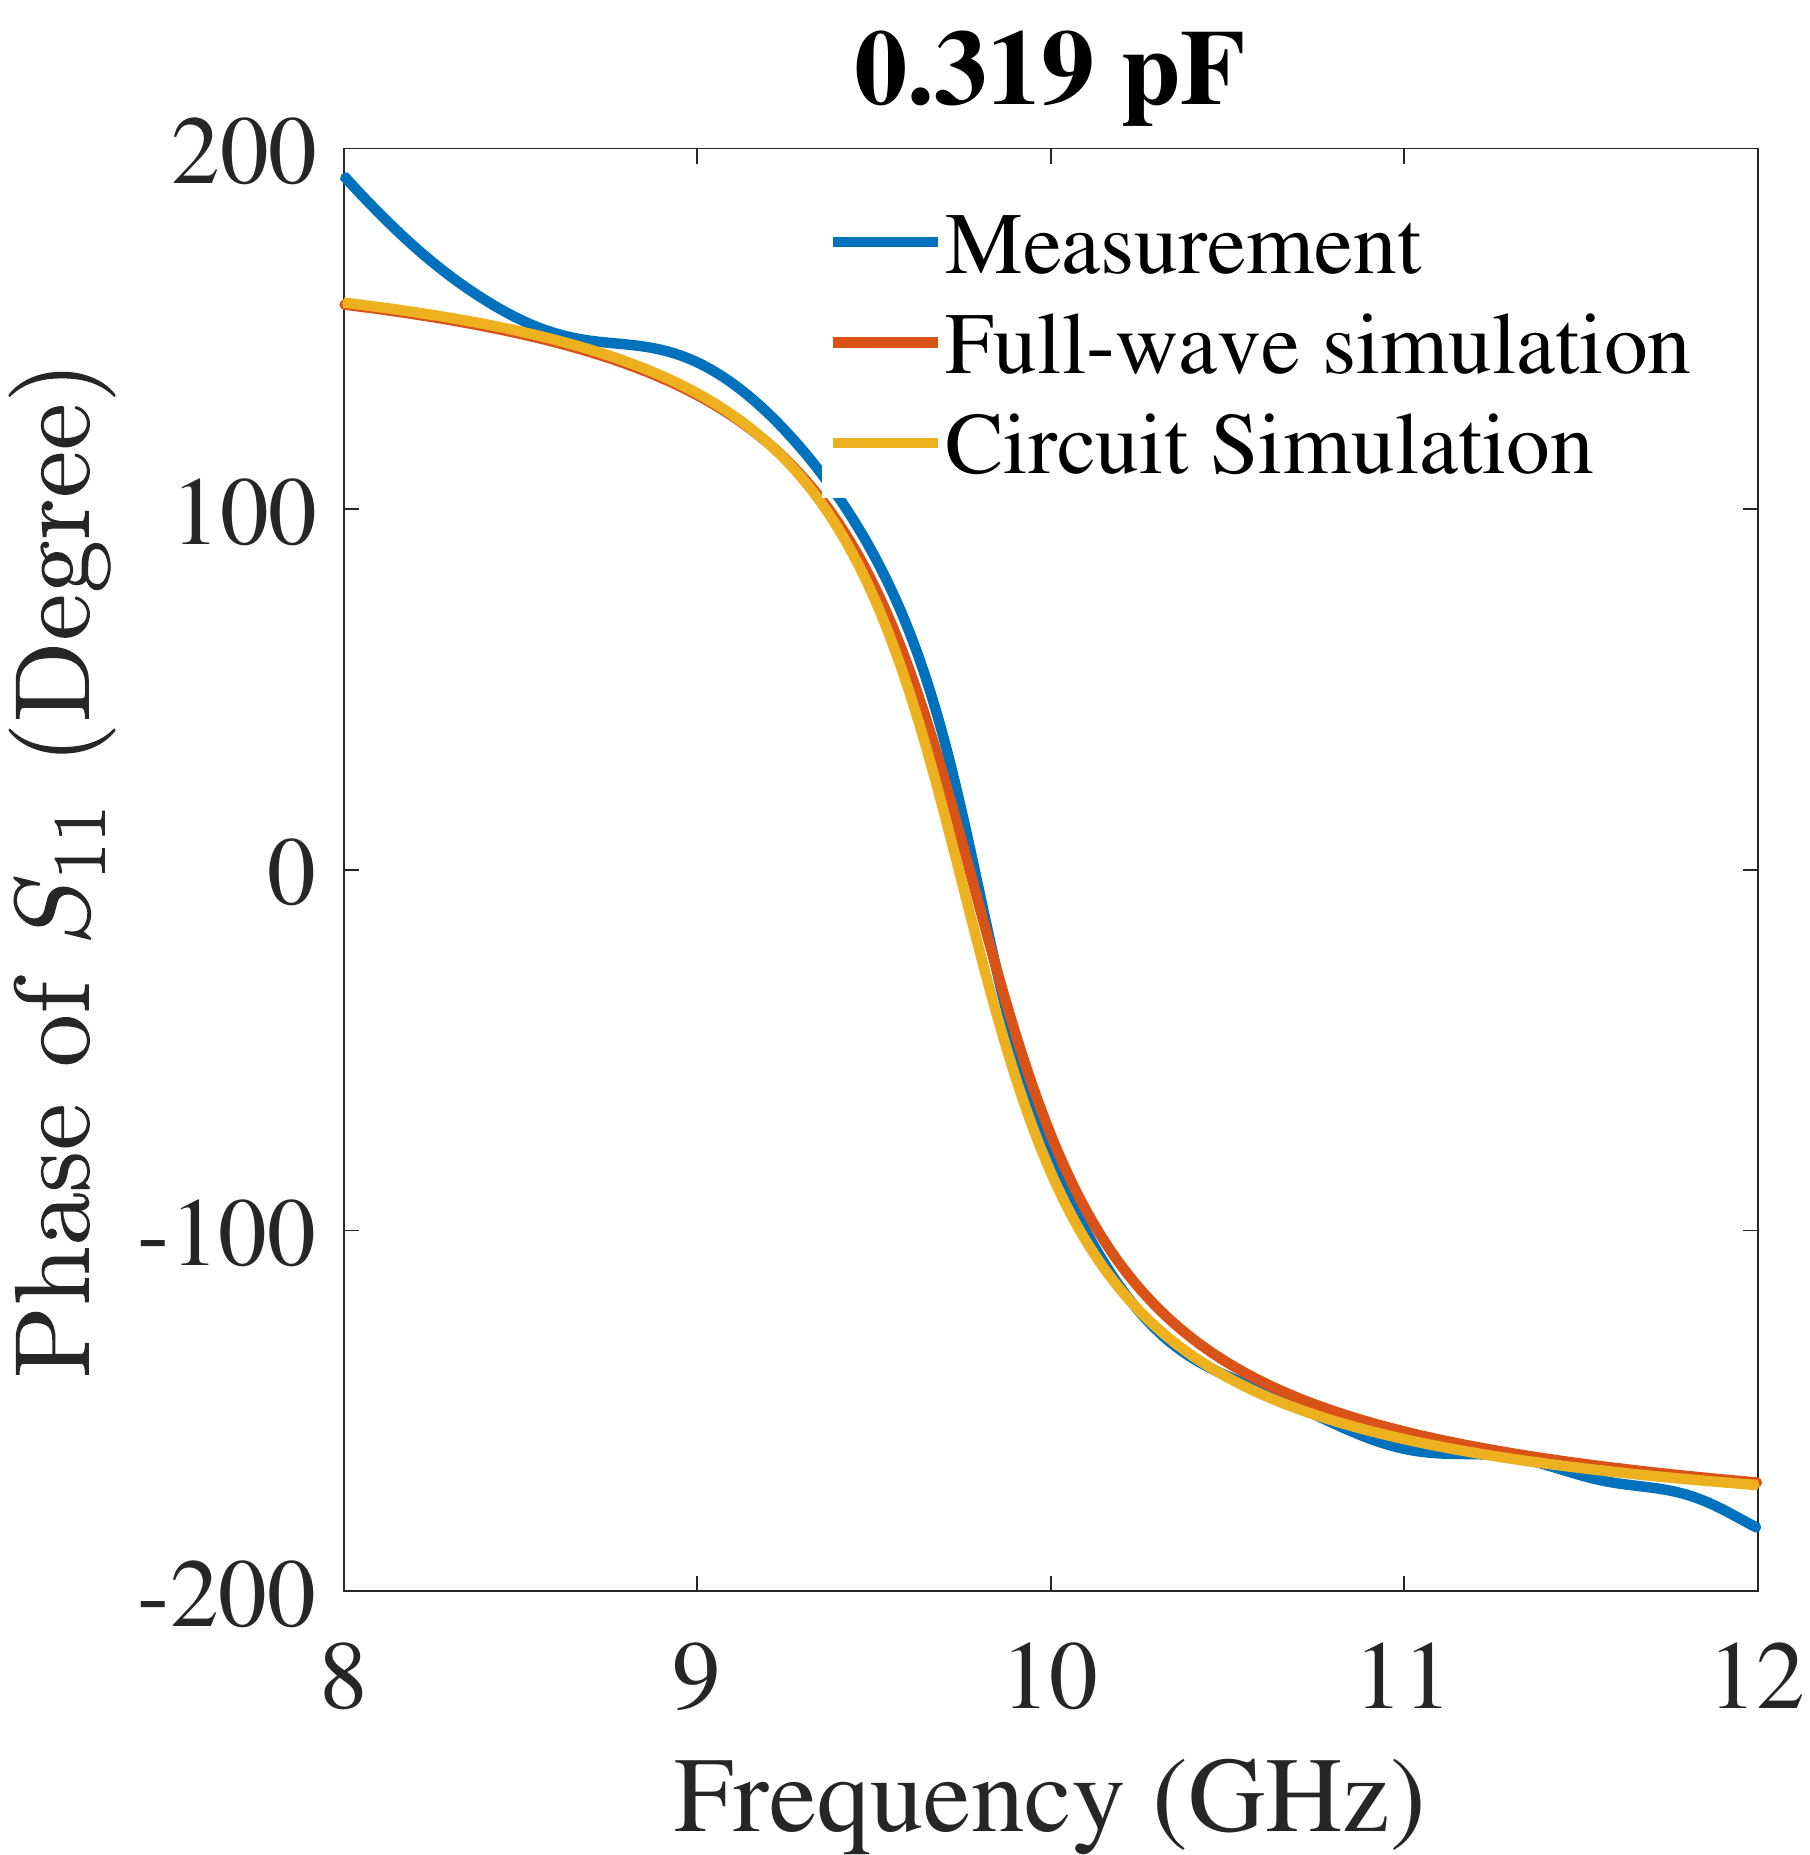}%
}\hfill
\subfloat[\label{sfig:DC6_P_TE}]{%
  \includegraphics[clip,width=0.165\columnwidth]{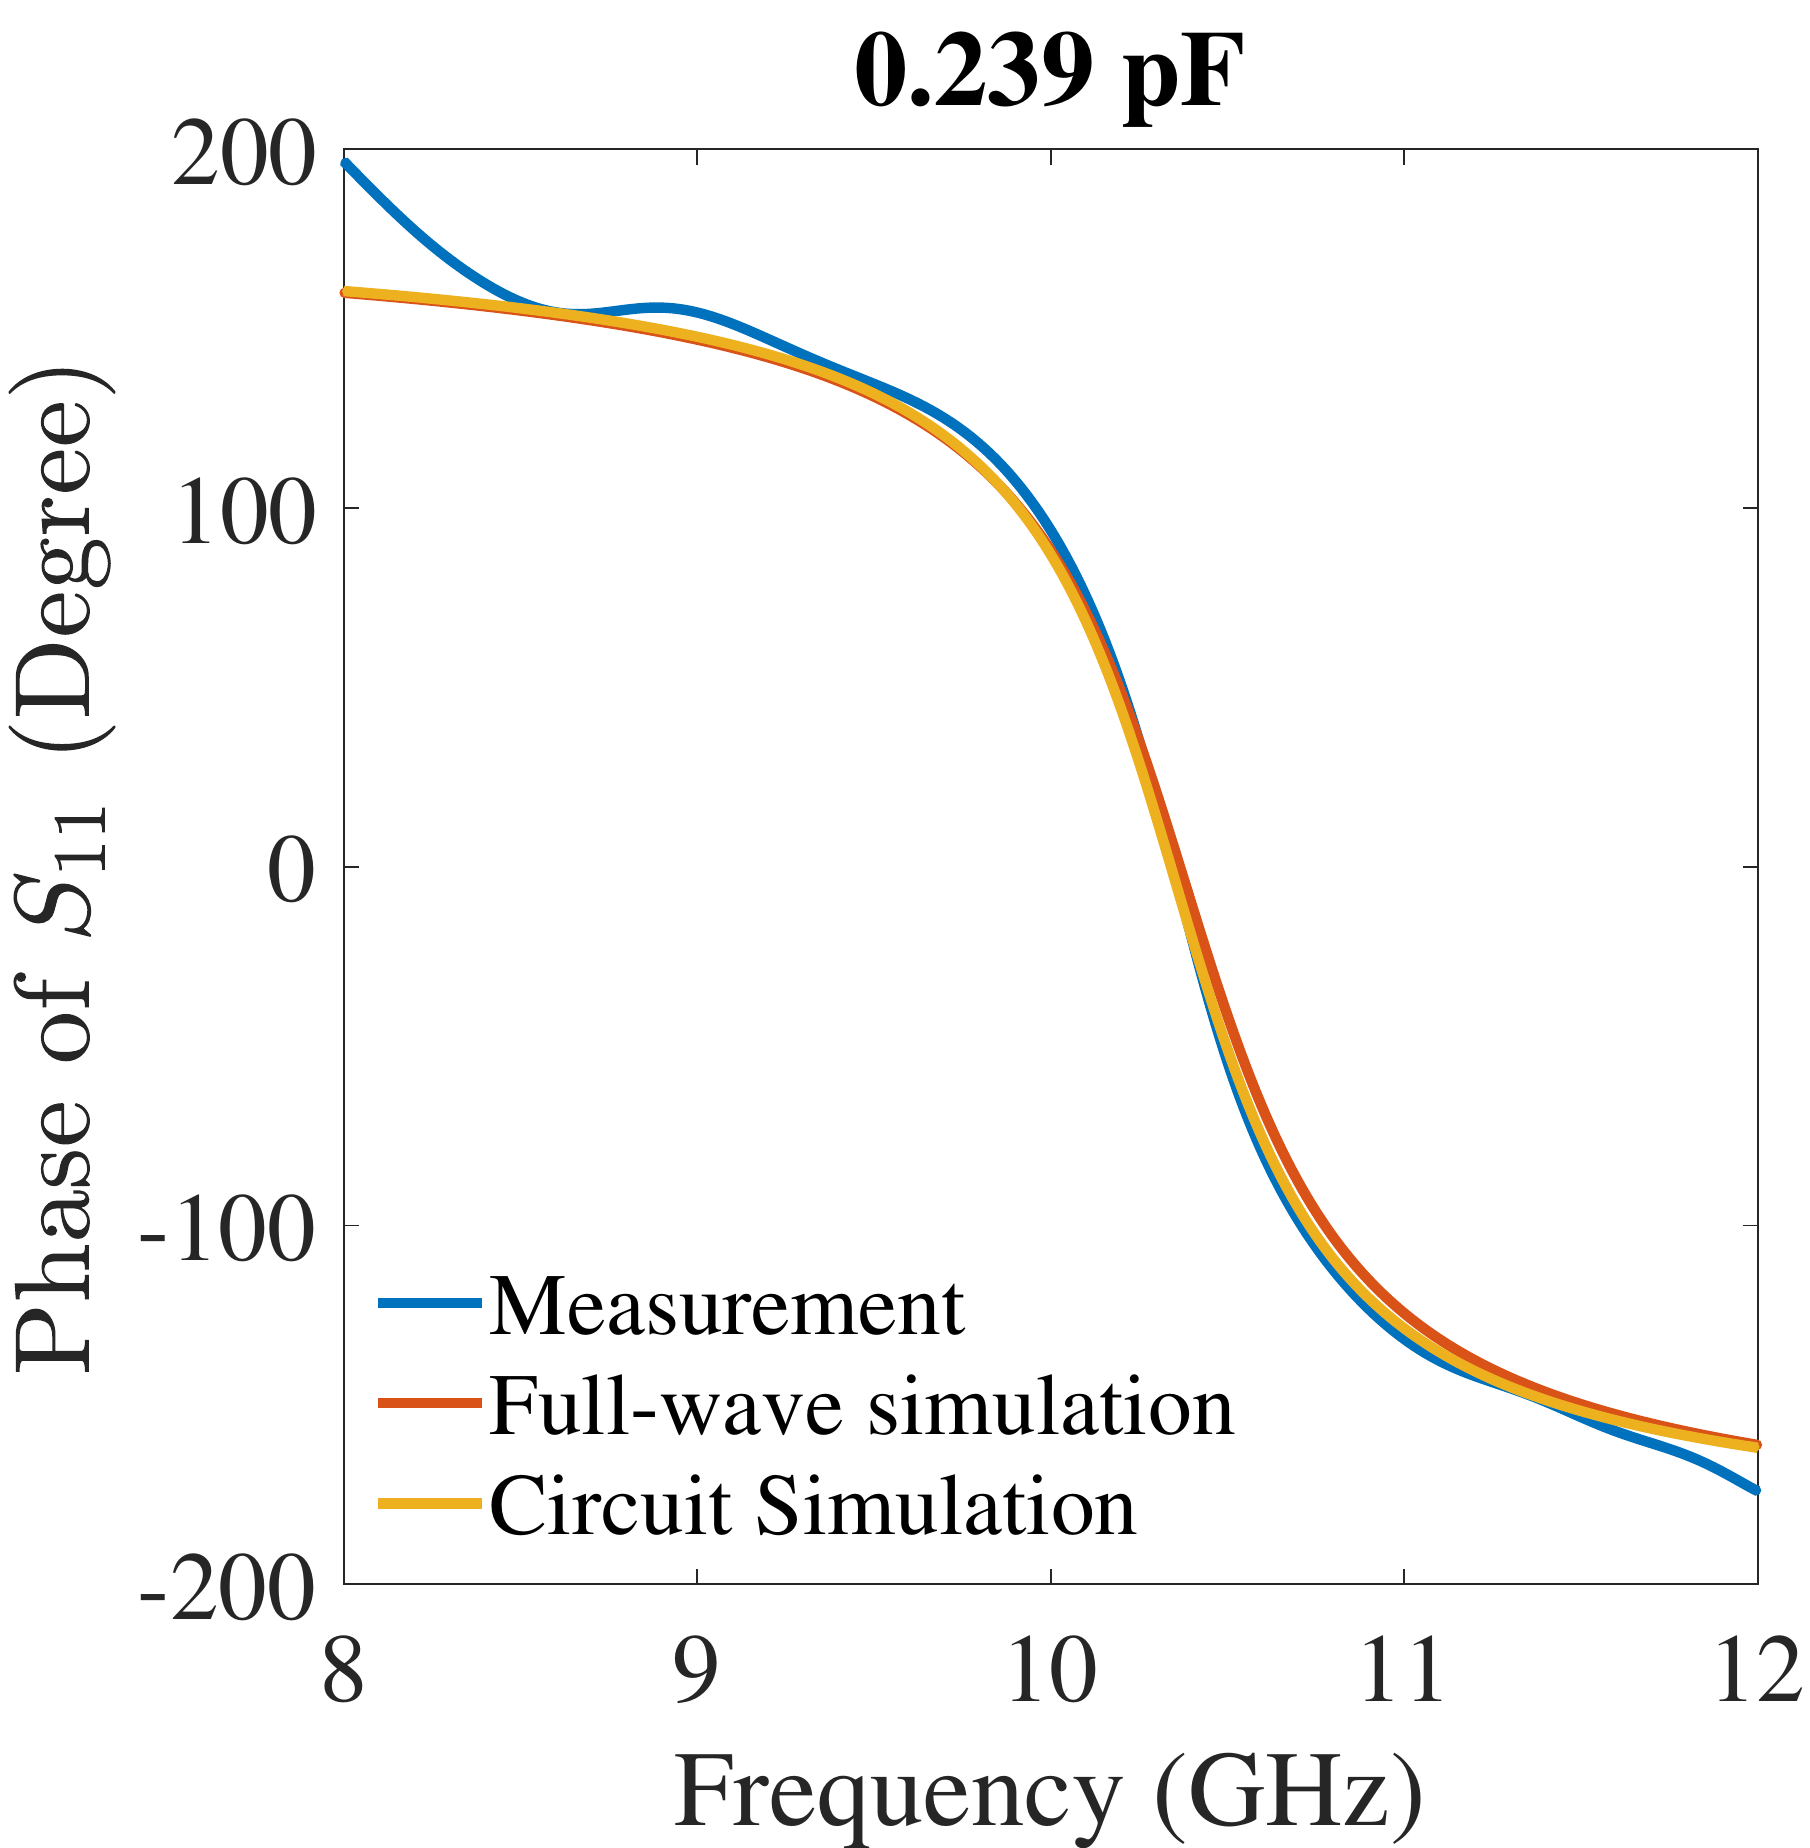}%
}\hfill
\subfloat[\label{sfig:DC7_P_TE}]{%
  \includegraphics[clip,width=0.165\columnwidth]{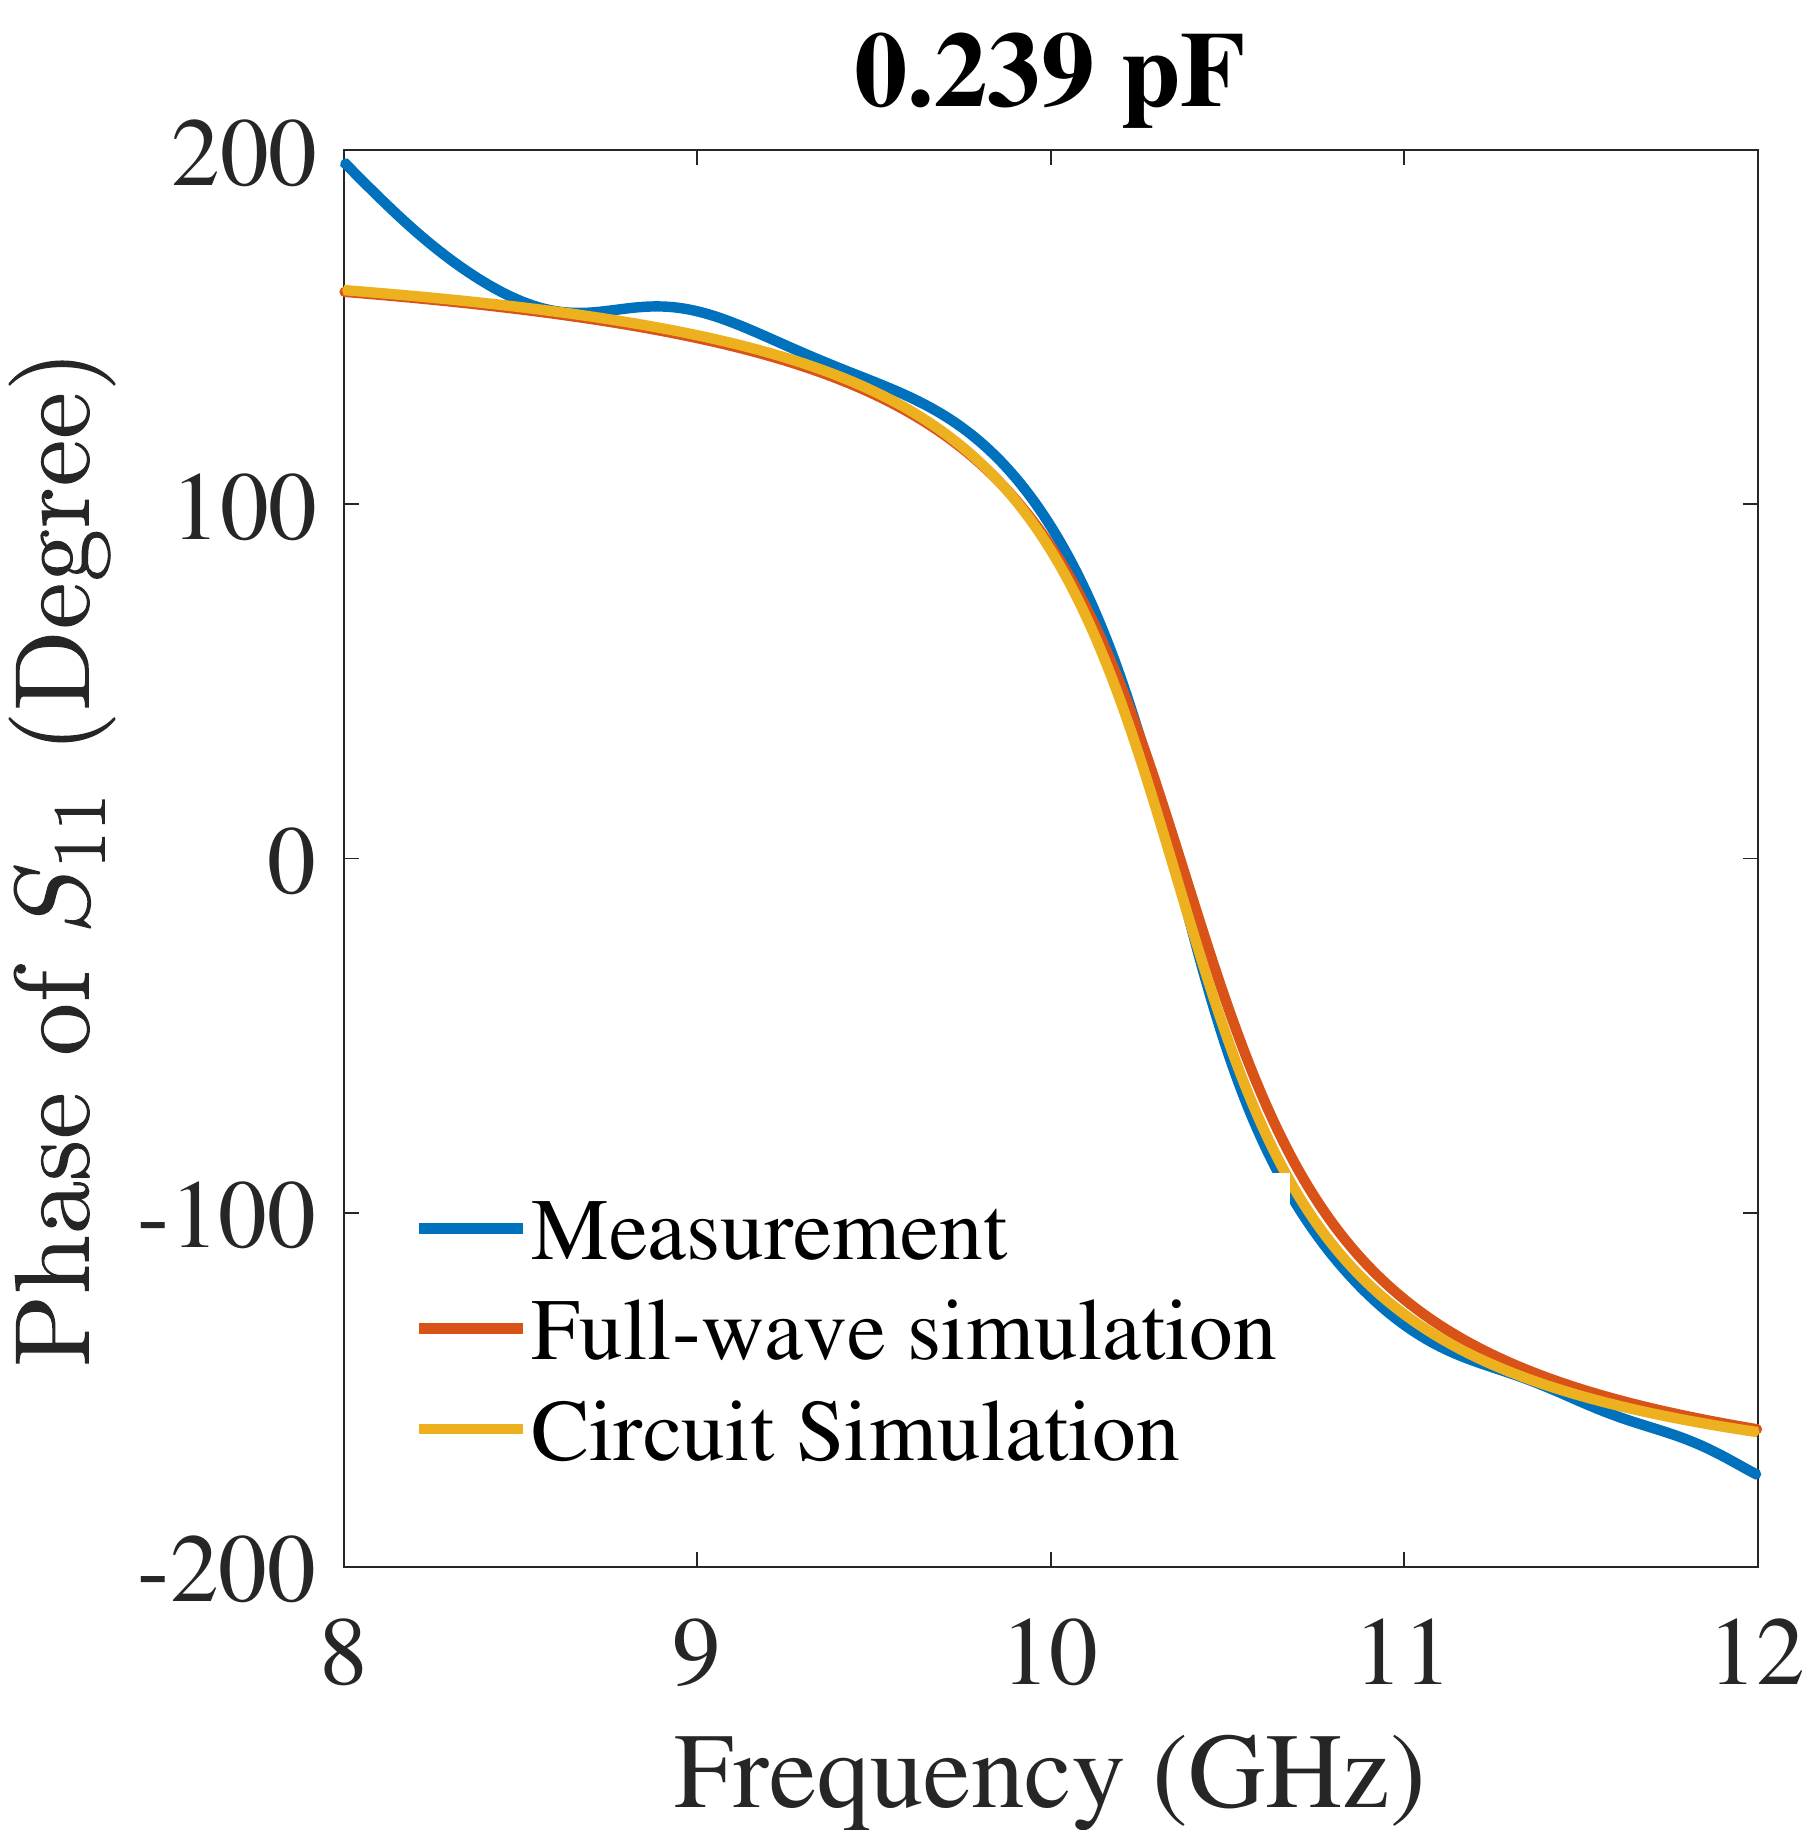}%
}\hfill
\subfloat[\label{sfig:DC8_P_TE}]{%
  \includegraphics[clip,width=0.165\columnwidth]{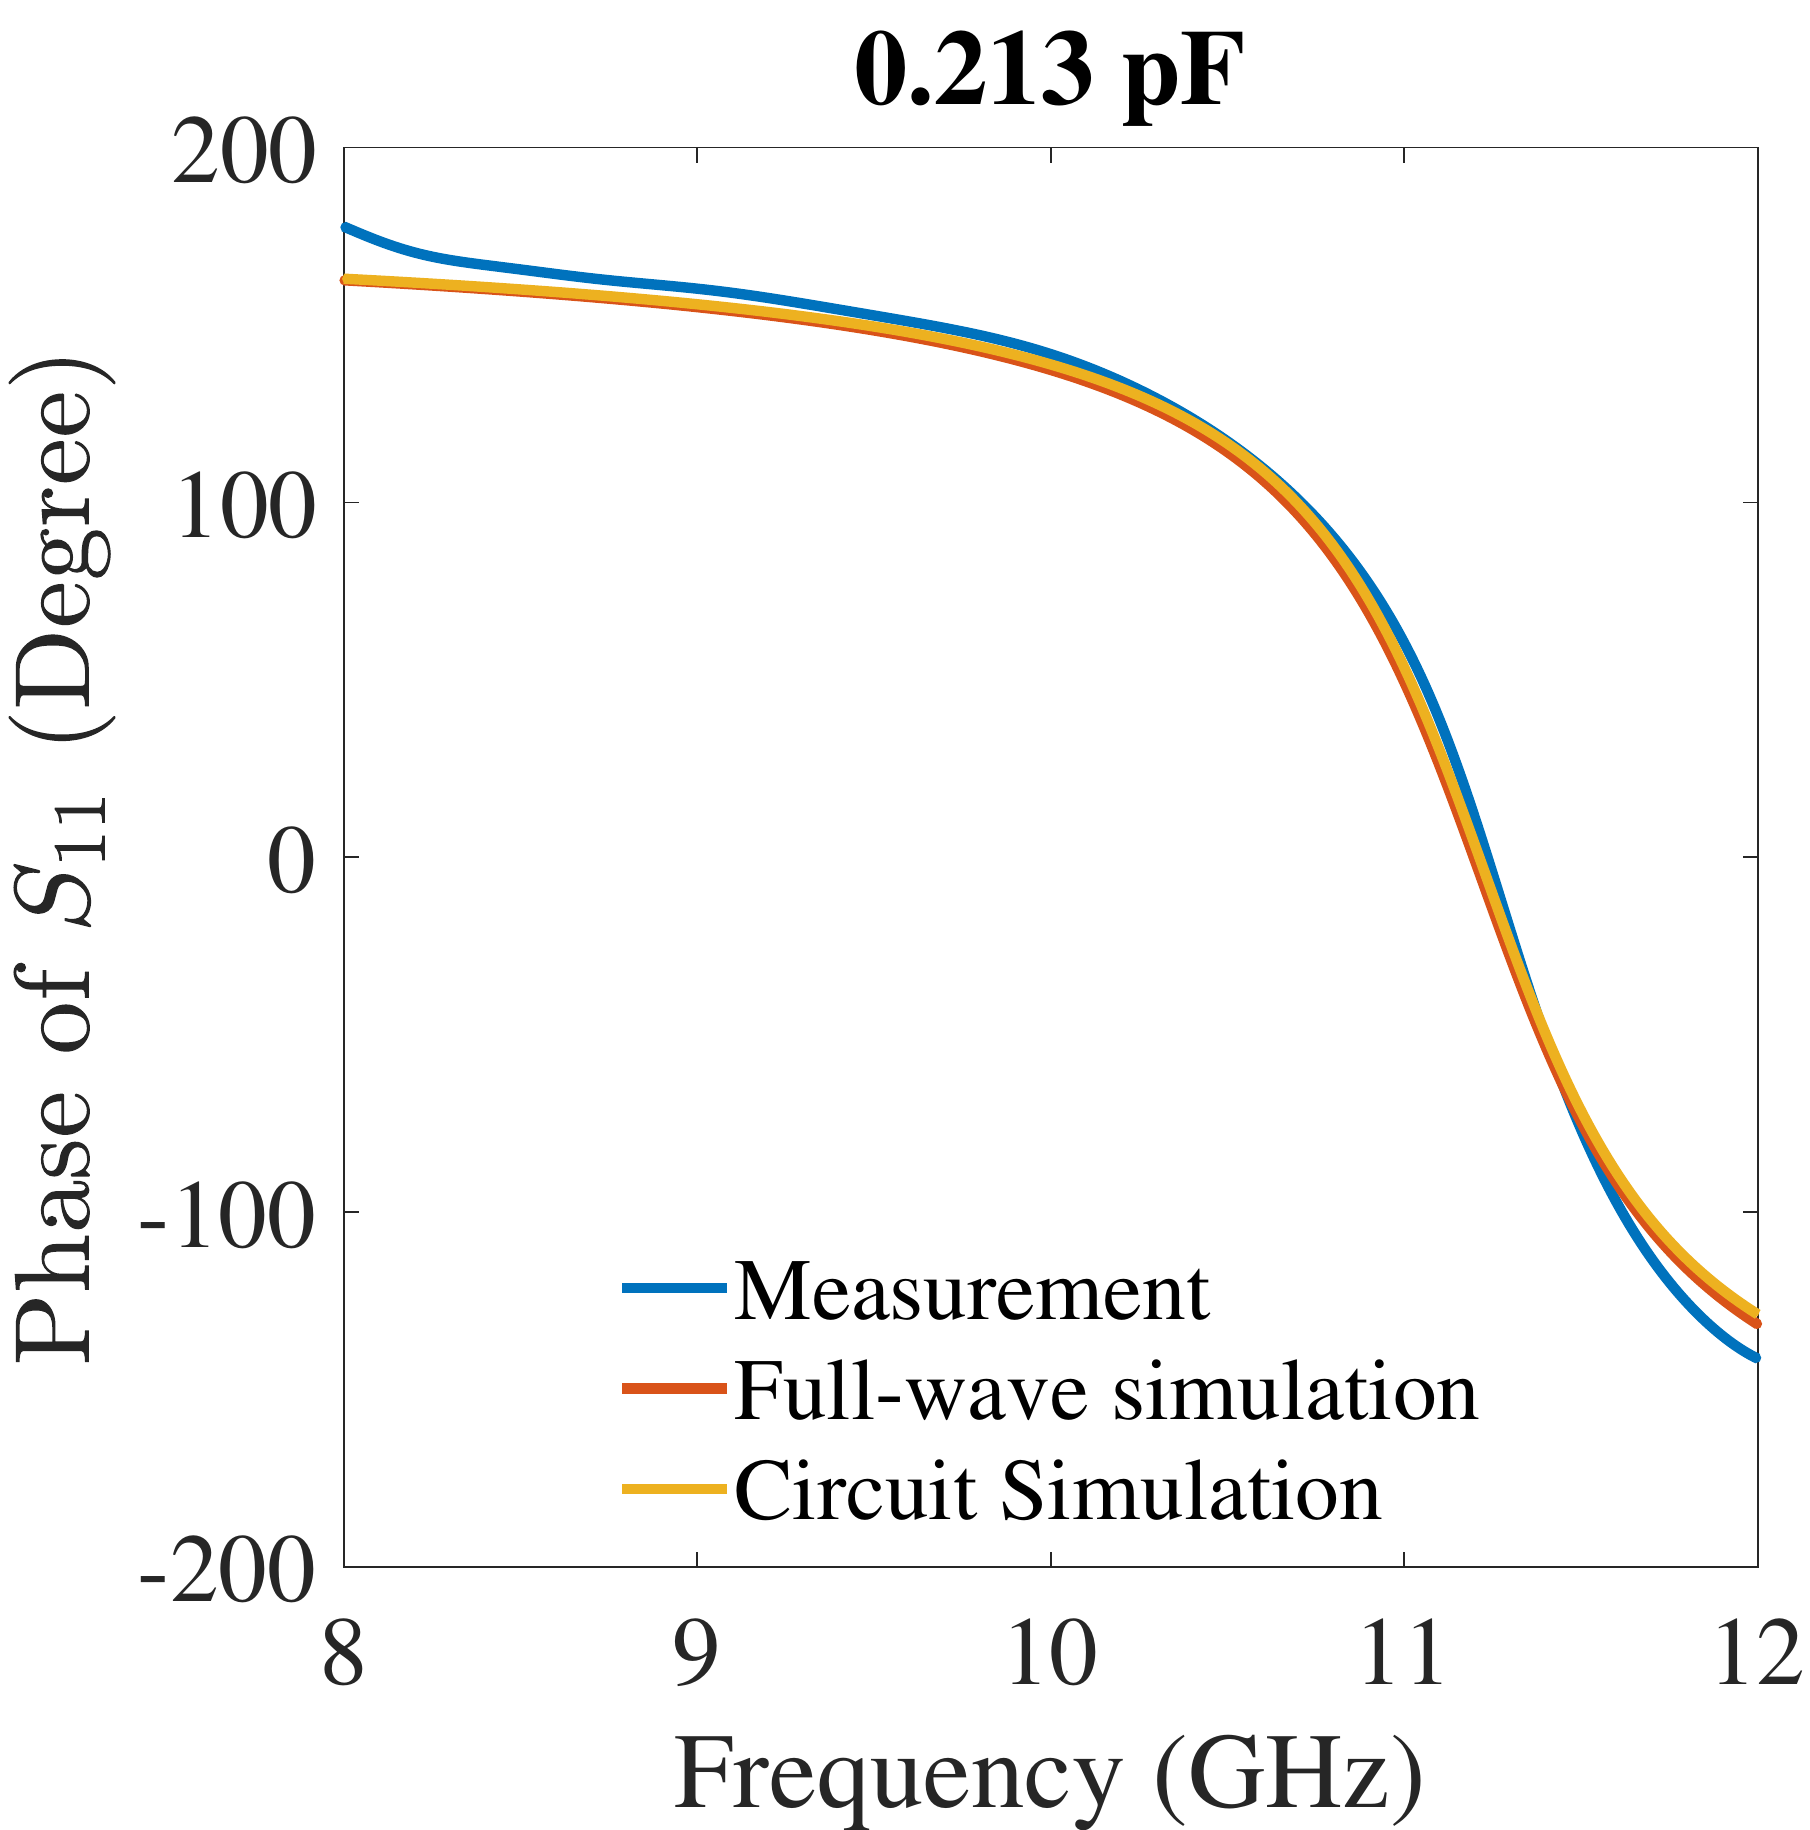}%
}\hfill
\subfloat[\label{sfig:DC9_P_TE}]{%
  \includegraphics[clip,width=0.165\columnwidth]{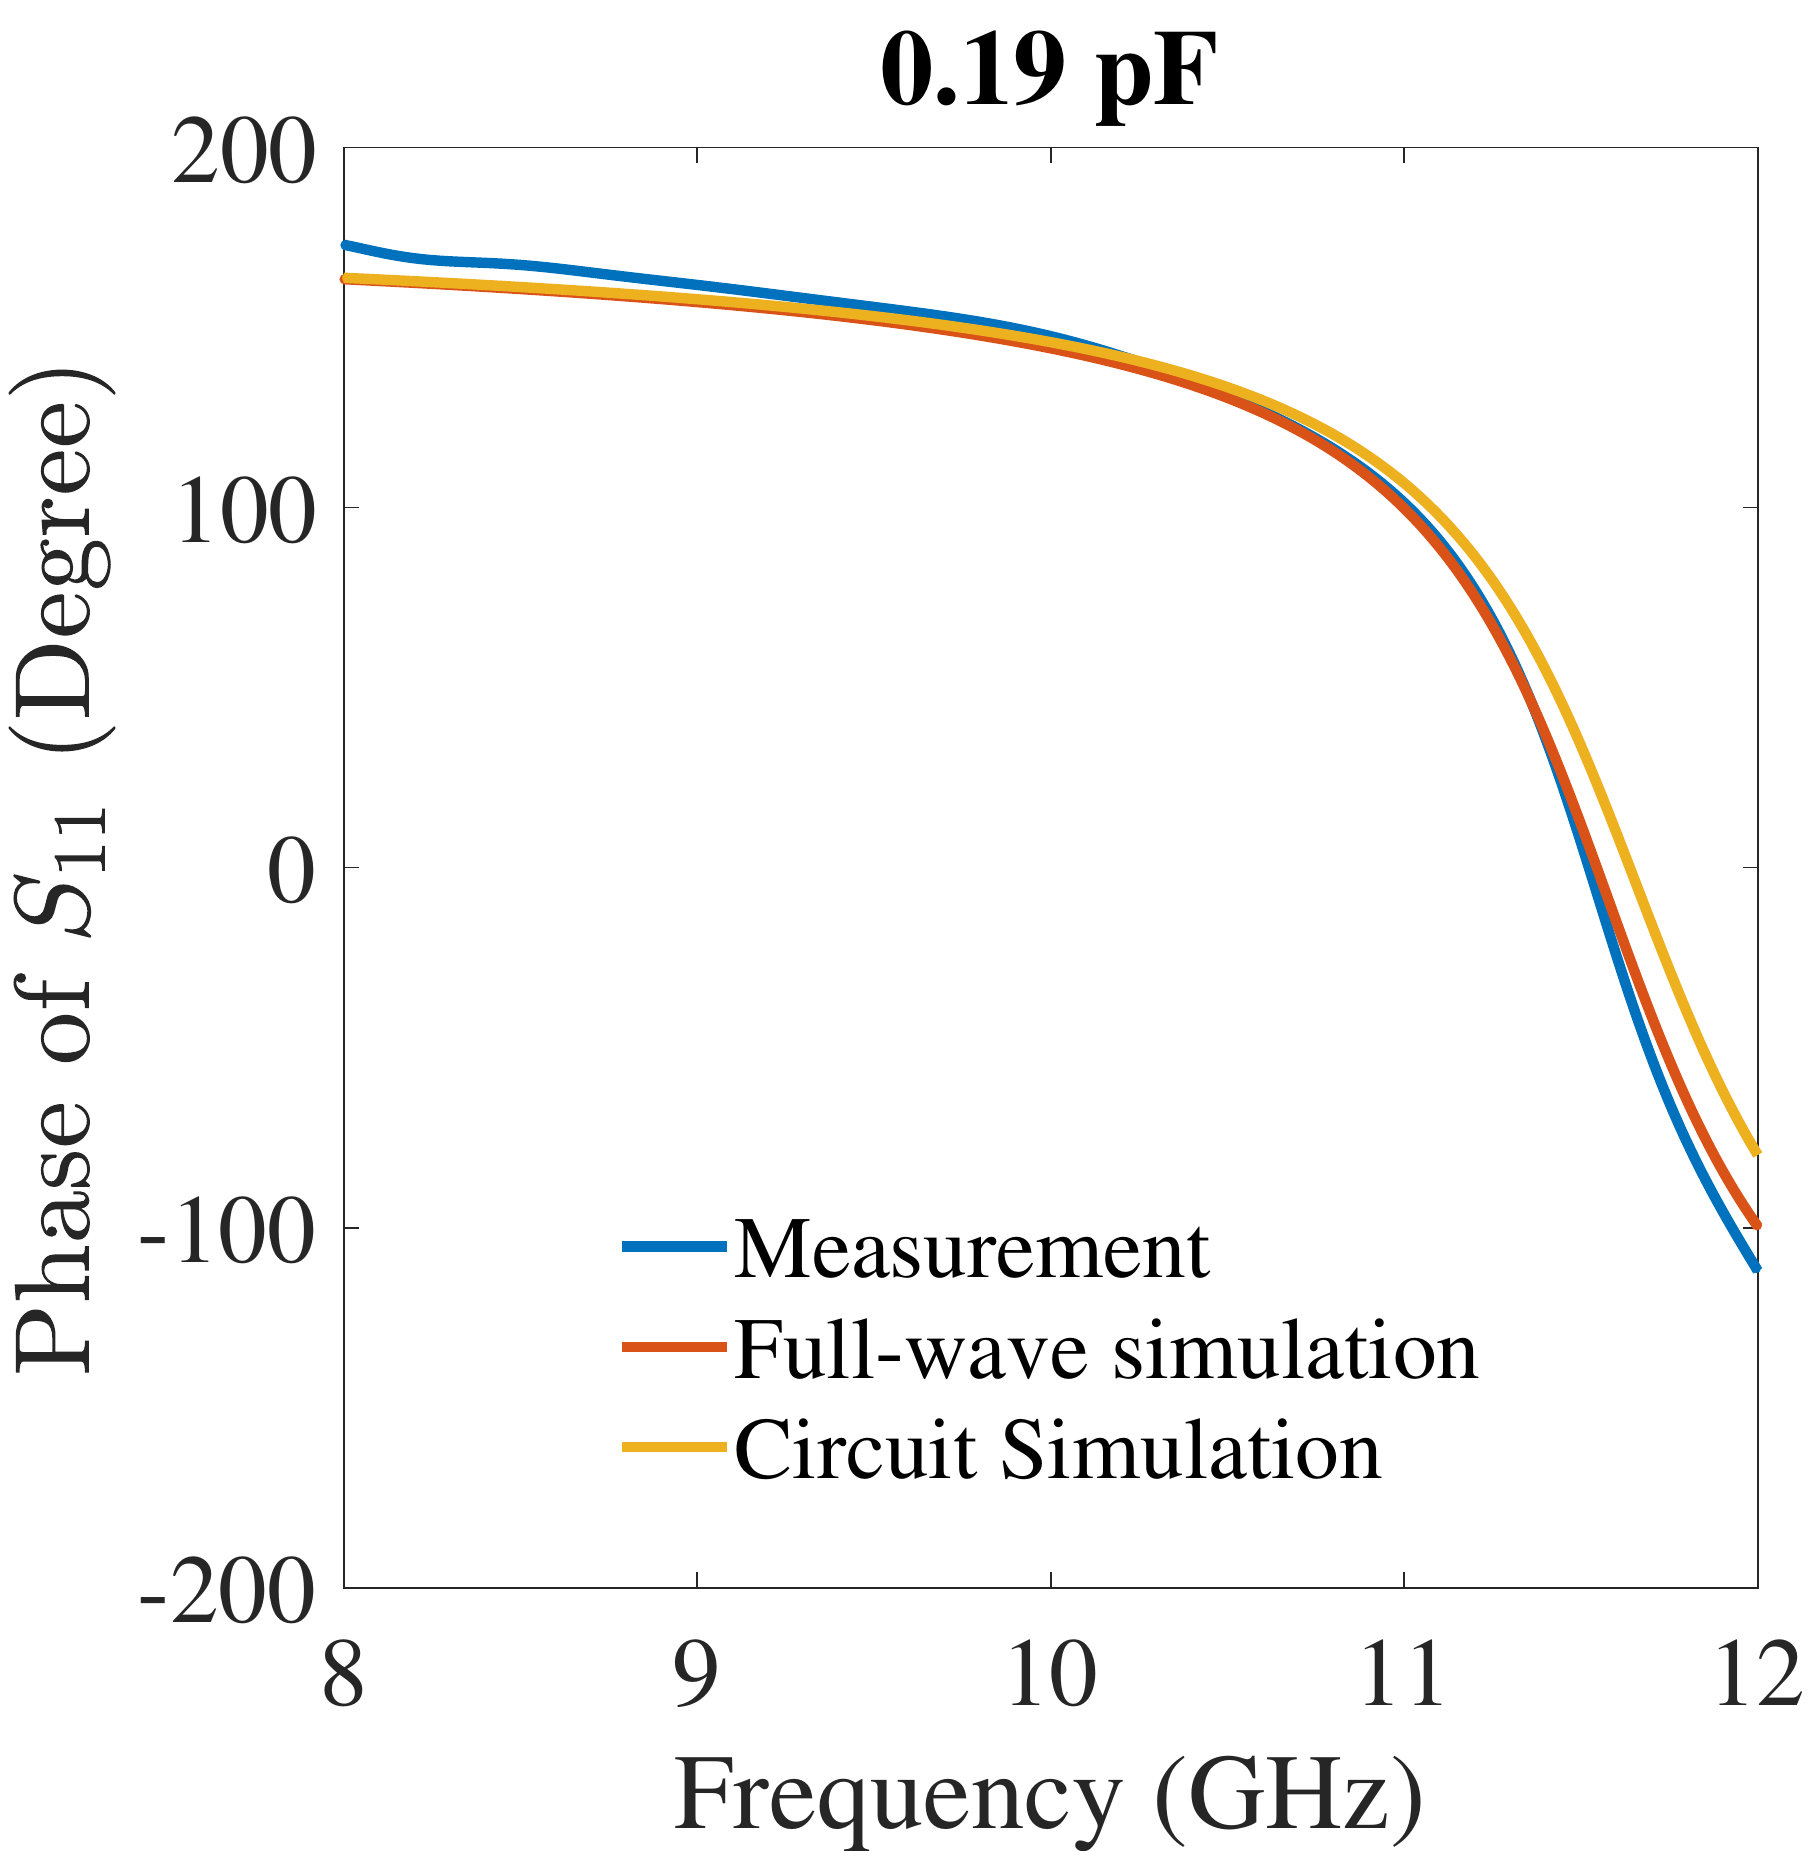}%
}\quad
\caption{Reflection phase and magnitude versus varactor capacitance for the realized metasurface from full-wave simulation, circuit model simulation and measurement under an oblique incident angle of $25^\circ$. Results are shown for a TM polarization.}
\label{fig:DCPerformance_TM}
\end{figure}

In order to conduct harmonic balance simulation (see Section \ref{sec:HarmonicBalance}) to predict the reflection spectrum of the metasurface when modulated, a circuit representation of the fabricated metasurface was extracted for each polarization. The circuit models are extracted from the full-wave scattering simulations, with an added voltage-dependent resistance $R^{TX}$ to account for the additional loss observed in measurement. The dependence of $R^{TX}$ is obtained by aligning the measured and simulated reflection amplitudes. The extracted circuit models are shown in Fig. \ref{fig:ExtractCircuit}. The values of the extracted circuit parameters are shown in Table \ref{tab:CircuitParam}. The varactor diode $C_d$ is modeled using the SPICE model for MAVR-000120-1411 varactors. For each varactor capacitance, the corresponding bias voltages used in circuit simulation (given by the SPICE model) and measurement, as well as the additional resistances $R^{TX}$ are given in Table \ref{tab:DiodeTE} and \ref{tab:DiodeTM} for the TE and TM polarizations. The varactor characteristics and additional losses $R^{TX}$ are slightly different for the two polarizations. This is likely due to tolerances in the varactor capacitance and resistance values.

The extracted circuits shown in Fig. \ref{fig:ExtractCircuit} are simulated with the commercial circuit solver Keysight Advanced Design System (ADS). Comparisons between full-wave simulation,  measurement, and circuit simulation are shown in \ref{fig:DCPerformance_TE} and \ref{fig:DCPerformance_TM} for various capacitance values.  The reverse bias voltage values used in circuit simulation are given in Table \ref{tab:DiodeTE} and \ref{tab:DiodeTM}. The circuit simulations agree closely with full-wave simulations and measurements of the metasurface, confirming the accuracy of the circuit model shown in Fig. \ref{fig:ExtractCircuit}.  

%\FloatBarrier

%\begin{table}[t]
%\caption{\label{tab:DiodeSPICE}%
%Varactor (MAVR-000120-1411) capacitance and resistance verses reverse bias voltage, extracted from the SPICE model.} 
%\begin{tabular}{>{\centering\arraybackslash}p{0.26\columnwidth} >{\centering\arraybackslash}p{0.22\columnwidth}>{\centering\arraybackslash}p{0.4\columnwidth}}
% \toprule
% Varactor capacitance (pF) &Varactor resistance ($\Omega$)&Reverse bias voltage used in circuit simulation (V)\\
 % \hline
%0.18&0.045&14.6\\
%0.2&0.081&11.56\\
%0.22 & 0.119&9.66\\
%0.24&0.153&8.36\\
%0.28&0.222&6.56\\
%0.32&0.28&5.42\\
%0.4 &0.373&3.94\\
%0.5&0.459&2.8\\
%.2&0.689&0.06\\
%  \bottomrule
%\end{tabular}
%\end{table}



%%%%%%%%%%%%%%%%%%%%%%%%%%%%%%%%%%%%%%%%%%%%%%%%%%
%%%%%%%%%%%%%%%%%%%%%%%%%%%%%%%%%%%%%%%%%%%%%%%%%%
%%%%%%%%%% Section 7
%%%%%%%%%%%%%%%%%%%%%%%%%%%%%%%%%%%%%%%%%%%%%%%%%%
%%%%%%%%%%%%%%%%%%%%%%%%%%%%%%%%%%%%%%%%%%%%%%%%%%

\section{Calculating the optimized bias waveform}

In order to achieve serrodyne frequency translation, a bias waveform is needed that generates a sawtooth reflection phase, which varies over $2\pi$ radians within each modulation period. To obtain the bias waveform, the following procedure was followed. Using the extracted circuit models shown in Fig. \ref{fig:ExtractCircuit}, the reflection amplitude and phase were obtained versus bias voltage at 10 GHz, as shown in Fig. \ref{fig:CircuitRef}. The plots show that the bias voltage versus reflection phase curves follow a tangent function. Since the targeted sawtooth reflection phase is linear with respect to time over each modulation period, the bias waveform was assumed to be of the following form,  
\begin{equation}\label{BiasModel}
    V_{bias}^{TX}(t)=
        \begin{cases}
      A\tan (B (\omega_p t +C))+D, & \text{for} \  0<V_{bias}^{TX}<14\\
      0, & \text{for} \  V_{bias}^{TX}<0\\
      14, &\text{for} \  V_{bias}^{TX}>14
    \end{cases}.
\end{equation}
over each 40 usec modulation period ($-T_p/2<t<T_p/2$). The parameters A, B, C, and D were then numerically optimized to provide optimal serrodyne frequency translation: the highest frequency conversion and lowest sidebands. The optimized values for TE polarization are $A=0.51$ V, $B=0.522$, $C=0.266$ rad, $D=5.597$ V. The optimized values for TM polarization are $A=0.8$ V, $B=0.535$, $C=0.339$ rad, $D=5.9$ V.

%relations ($|S_{11}|(V_{bias}^{TX})$, $\angle S_{11}(V_{bias}^{TX})$) are extracted at the operating frequency of 10 GHz, as shown in Fig. \ref{fig:CircuitRef}. The bias voltage is curve fitted to a tangent function of the reflection phase, motivated by Eq. (\ref{RefPhase}). This allowed the bias waveform $V_{bias}^{TX}(t)$ to be found that linearize the phase in time. However, since the varactor resistance and metal loss are included in the circuit models, the reflection amplitude is not unity. To account for this, we model the bias waveform as the following function, over a 40 usec modulation period ($-T_p/2<t<T_p/2$).
%\begin{equation}\label{BiasModel}
%    V_{bias}^{TX}(t)=
%        \begin{cases}
%      A\tan (B (\omega_p t +C))+D, & \text{for} %\  0<V_{bias}^{TX}<15\\
%      0, & \text{for} \  V_{bias}^{TX}<0\\
%      15, &\text{for} \  V_{bias}^{TX}>15
%    \end{cases}.
%\end{equation}
%The parameters A, B, C, and D are fitting parameters and are numerically optimized to provide the highest frequency conversion and lowest sidebands. The optimized waveform used in simulation is shown in Fig. \ref{sfig:Waveform_TE} and \ref{sfig:Waveform_TM} respectively. 

\begin{figure}[b!]
\centering
\subfloat[\label{sfig:CircuitTE}]{%
  \includegraphics[clip,width=0.3\columnwidth]{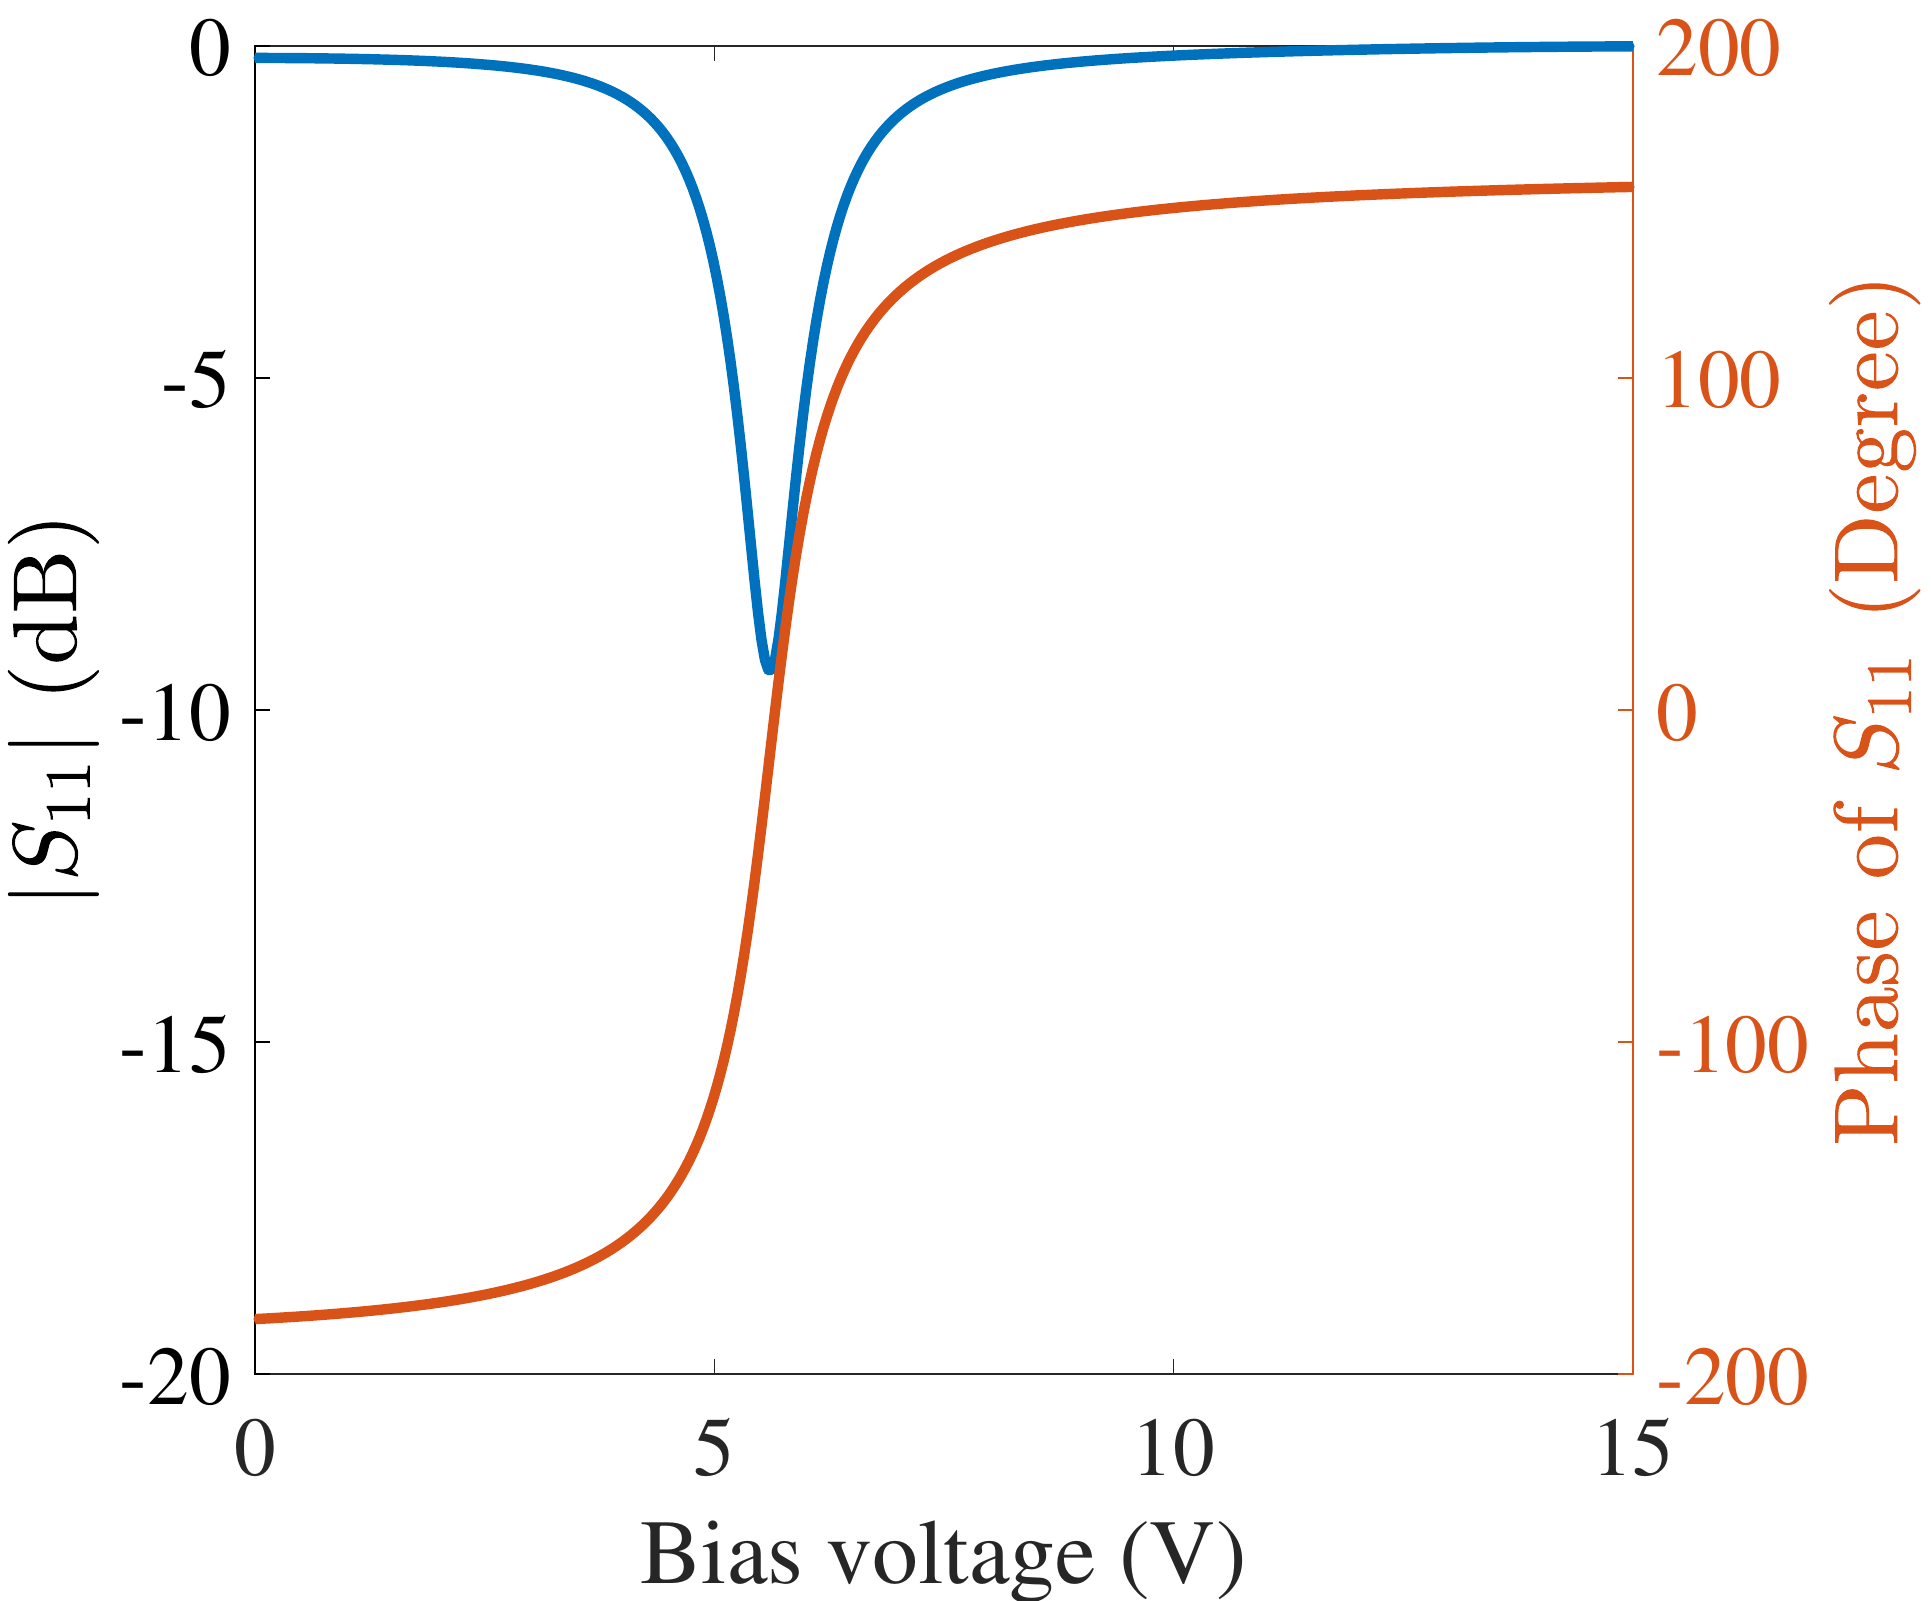}%
}\hspace{4em}
\subfloat[\label{sfig:CircuitTM}]{%
  \includegraphics[clip,width=0.3\columnwidth]{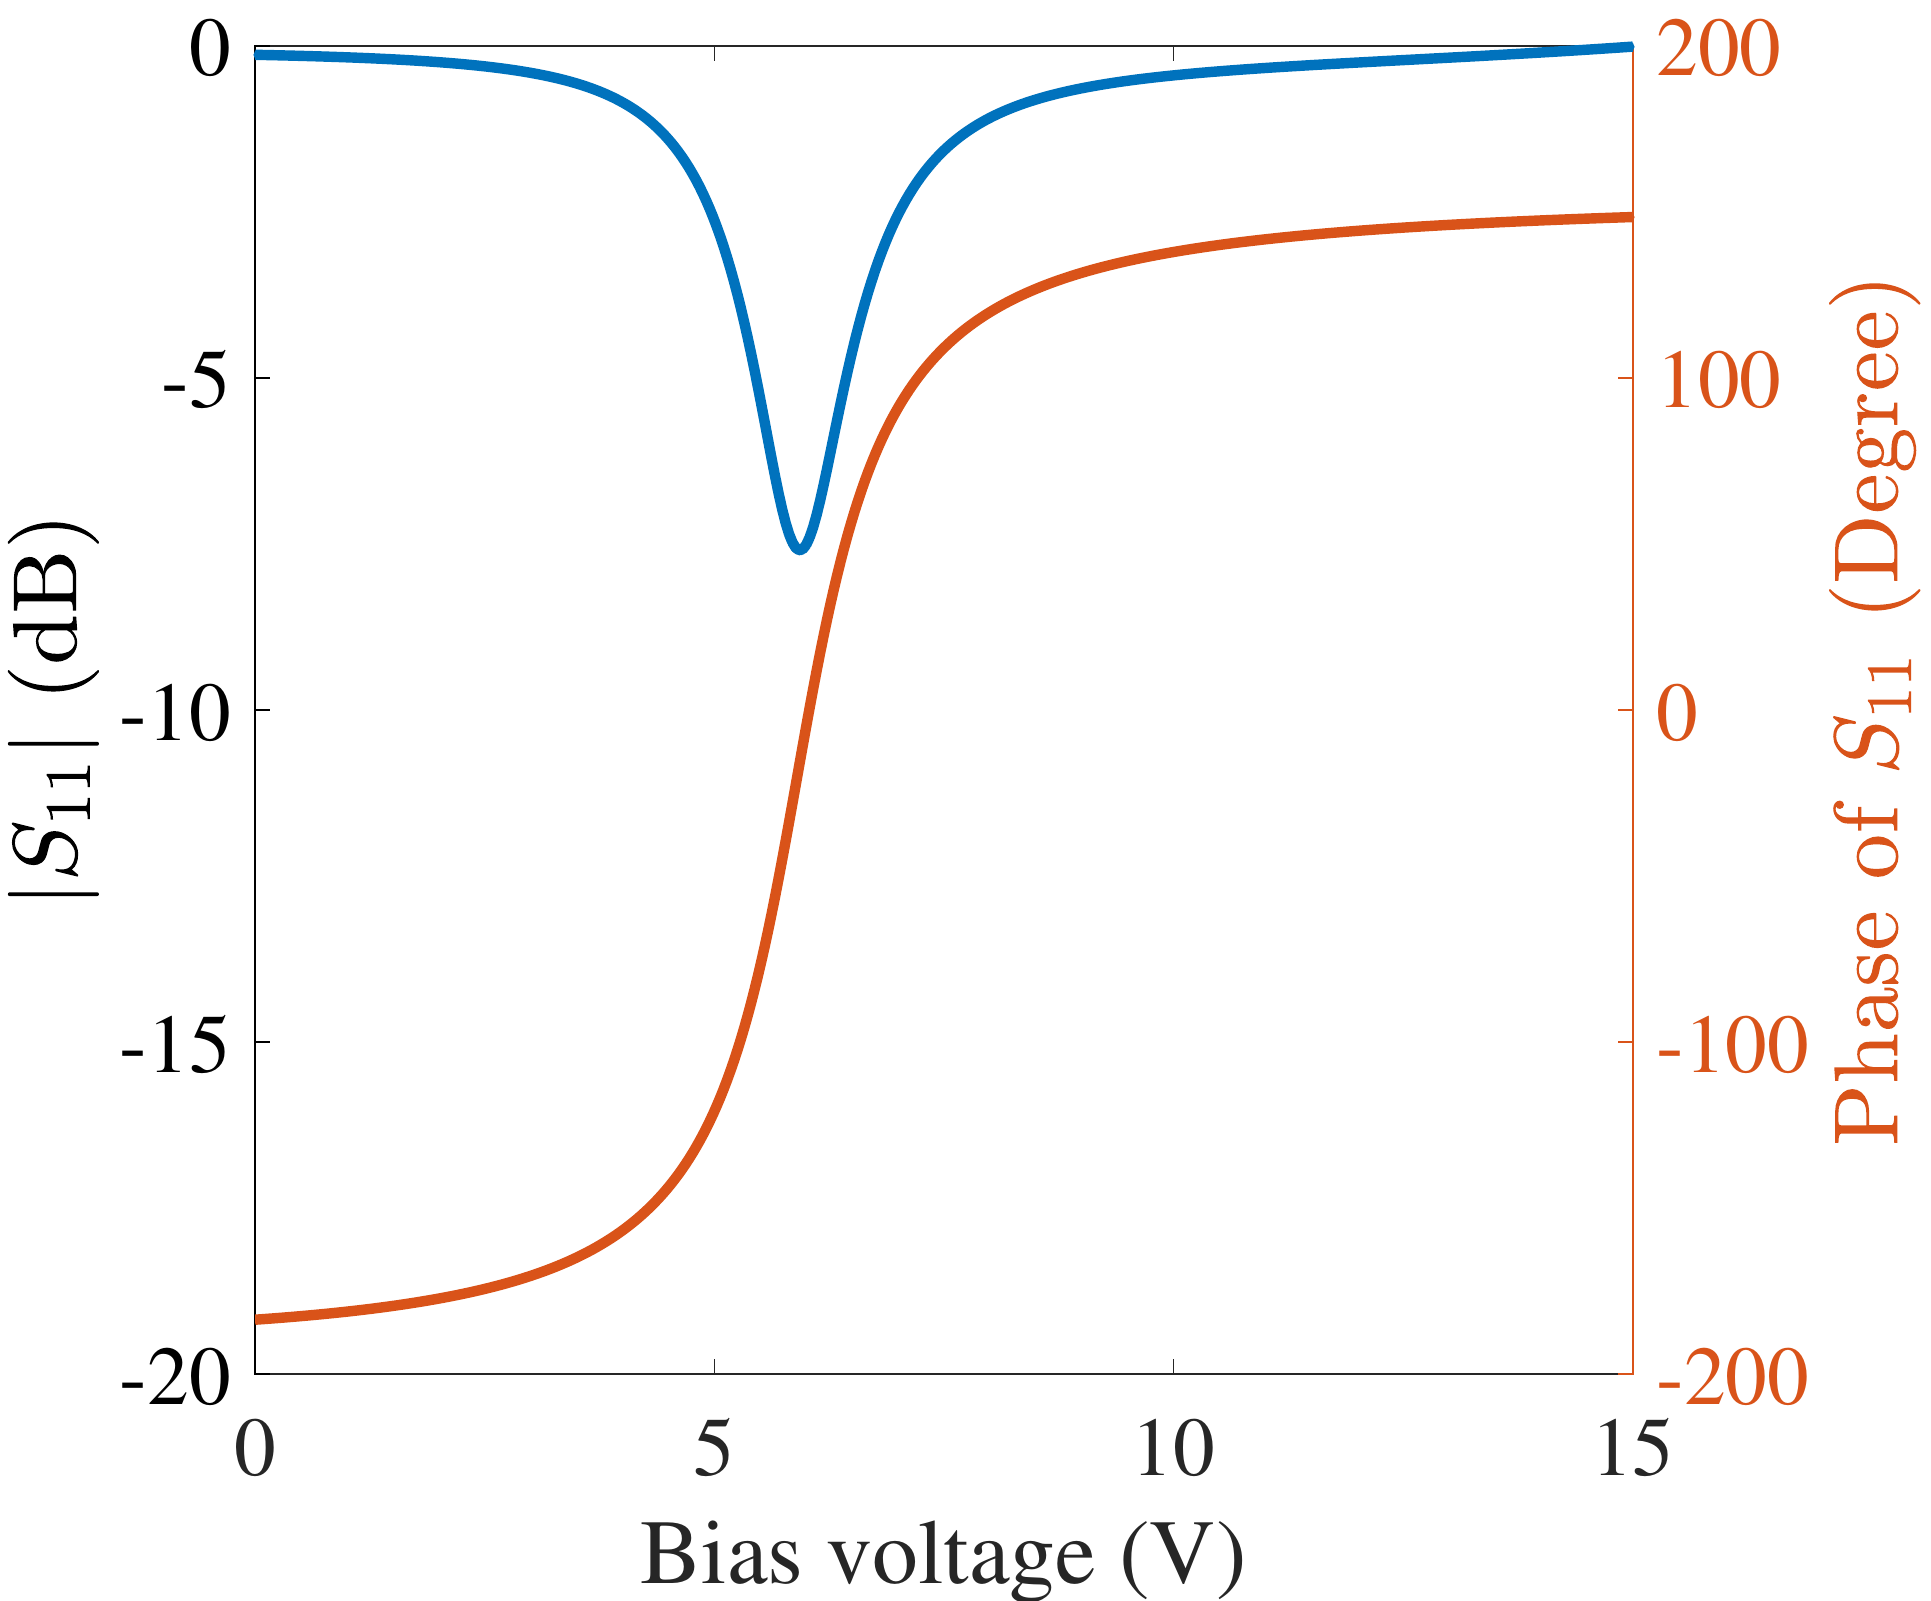}%
}\quad
\caption{Reflection coefficient magnitude and phase of the extracted circuit model for the metasurface as a function of reverse bias voltage. (a)TE polarization. (b) TM polarization.}
\label{fig:CircuitRef}
\end{figure} 

Similarly, in order to generate a sinusoidal reflection phase with respect to time, the bias waveform was assumed to be of the following form,
\begin{equation}\label{BiasModel_Sin}
    V_{bias}^{TX}(t)=
        \begin{cases}
      A\tan (B (A_0 \sin (\omega_p t) +C))+D, & \text{for} \  0<V_{bias}^{TX}<14\\
      0, & \text{for} \  V_{bias}^{TX}<0\\
      14, &\text{for} \  V_{bias}^{TX}>14
    \end{cases}.
\end{equation}
where $A_0=138^\circ$, as explained in the paper. The fitting parameters A, B, C, and D were again numerically optimized to suppress the zeroth harmonic in reflection. The optimized waveform used in simulation is shown in Figs. \ref{sfig:Waveform_TE_Sin} and \ref{sfig:Waveform_TM_Sin}. The optimized values for TE polarization are $A=0.45$ V, $B=0.455$, $C=0.286$ rad, $D=5.53$ V. The optimized values for TM polarization are $A=0.65$ V, $B=0.458$, $C=0.389$ rad, $D=5.8$ V.

A harmonic representation of the optimized bias waveform (referred to as simulated bias waveform) was then used in the harmonic balance simulation, which is detailed in the next section. In addition, a mapping between the bias voltage used in circuit simulation and in measurement for each varactor capacitance value, was obtained from Table \ref{tab:DiodeTE} and \ref{tab:DiodeTM}. The experimental bias waveform was determined by applying this mapping to the optimized bias waveform. A sampled version (20 points per period) of the experimental bias waveform (referred to as measured bias waveform) was applied to the metasurface through the D/A converter in measurement. The optimized and measured bias waveform used in the measurement are shown in Fig. 26a and 26c for serrodyne frequency translation.

%%%%%%%%%%%%%%%%%%%%%%%%%%%%%%%%%%%%%%%%%%%%%%%%%%
%%%%%%%%%%%%%%%%%%%%%%%%%%%%%%%%%%%%%%%%%%%%%%%%%%
%%%%%%%%%% Section 8
%%%%%%%%%%%%%%%%%%%%%%%%%%%%%%%%%%%%%%%%%%%%%%%%%%
%%%%%%%%%%%%%%%%%%%%%%%%%%%%%%%%%%%%%%%%%%%%%%%%%%

\section{Harmonic balance simulation of the extracted circuit model} \label{sec:HarmonicBalance}

If all the columns of the metasurface are biased with the same waveform, the metasurface's response can be predicted by performing a harmonic balance simulation of a single unit cell's extracted circuit model. Harmonic balance simulations of the circuit model shown in Fig. \ref{fig:ExtractCircuit} were performed using Keysight ADS. The incident signal was set to an amplitude of $-20$ dBm at frequency $f_0=10$ GHz. The optimized waveforms $V_{bias}^y$ and $V_{bias}^x$ were calculated as described in the previous section. 

\begin{figure}[b!]
\centering
\subfloat[\label{sfig:Waveform_TE}]{%
  \includegraphics[clip,width=0.25\columnwidth]{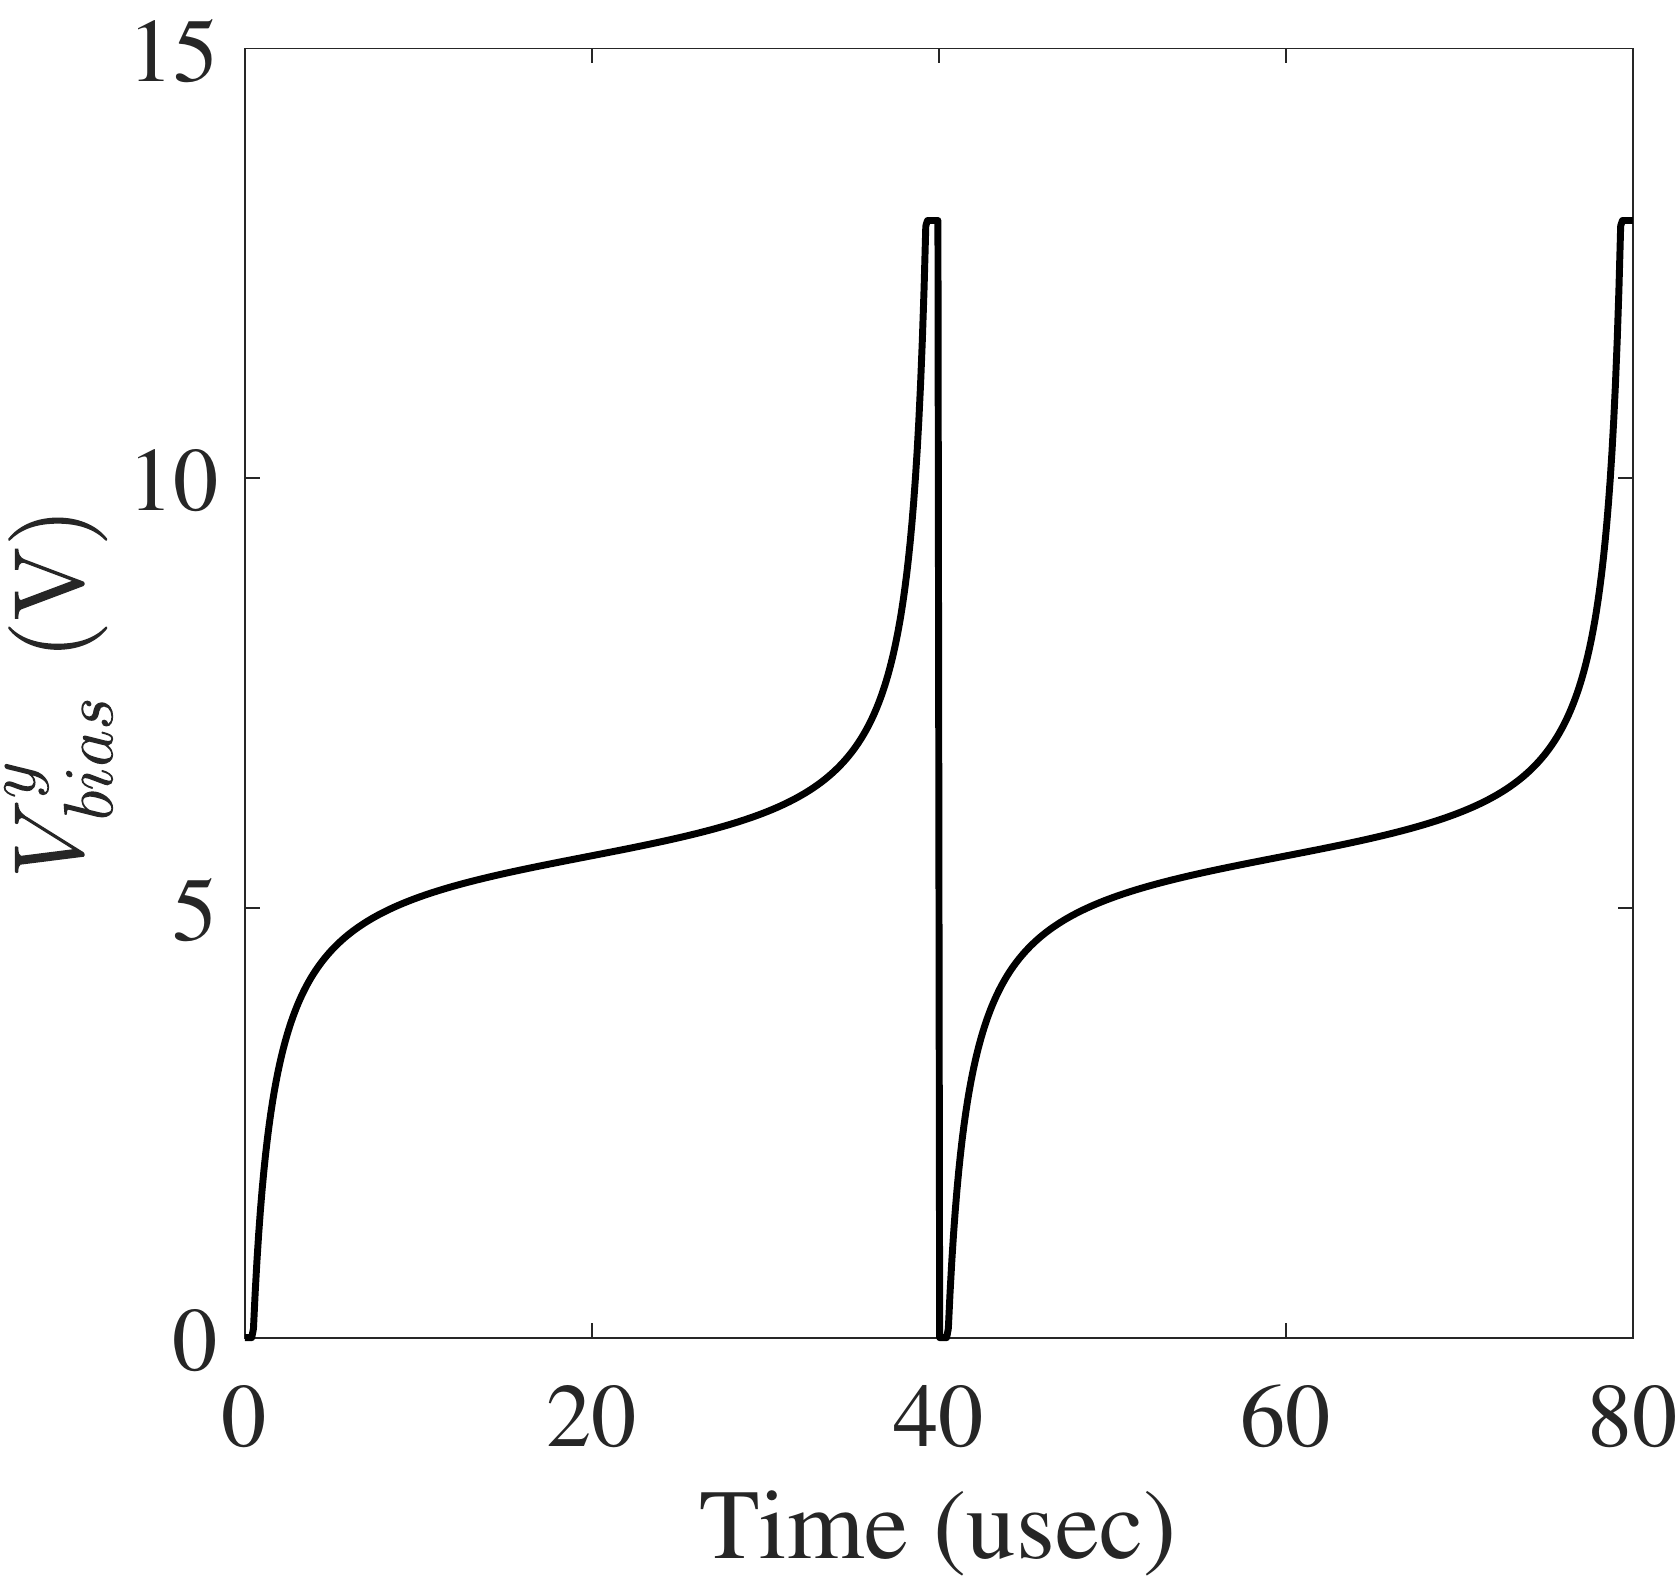}%
}\hfill
\subfloat[\label{sfig:TE1path_Sim}]{%
  \includegraphics[clip,width=0.25\columnwidth]{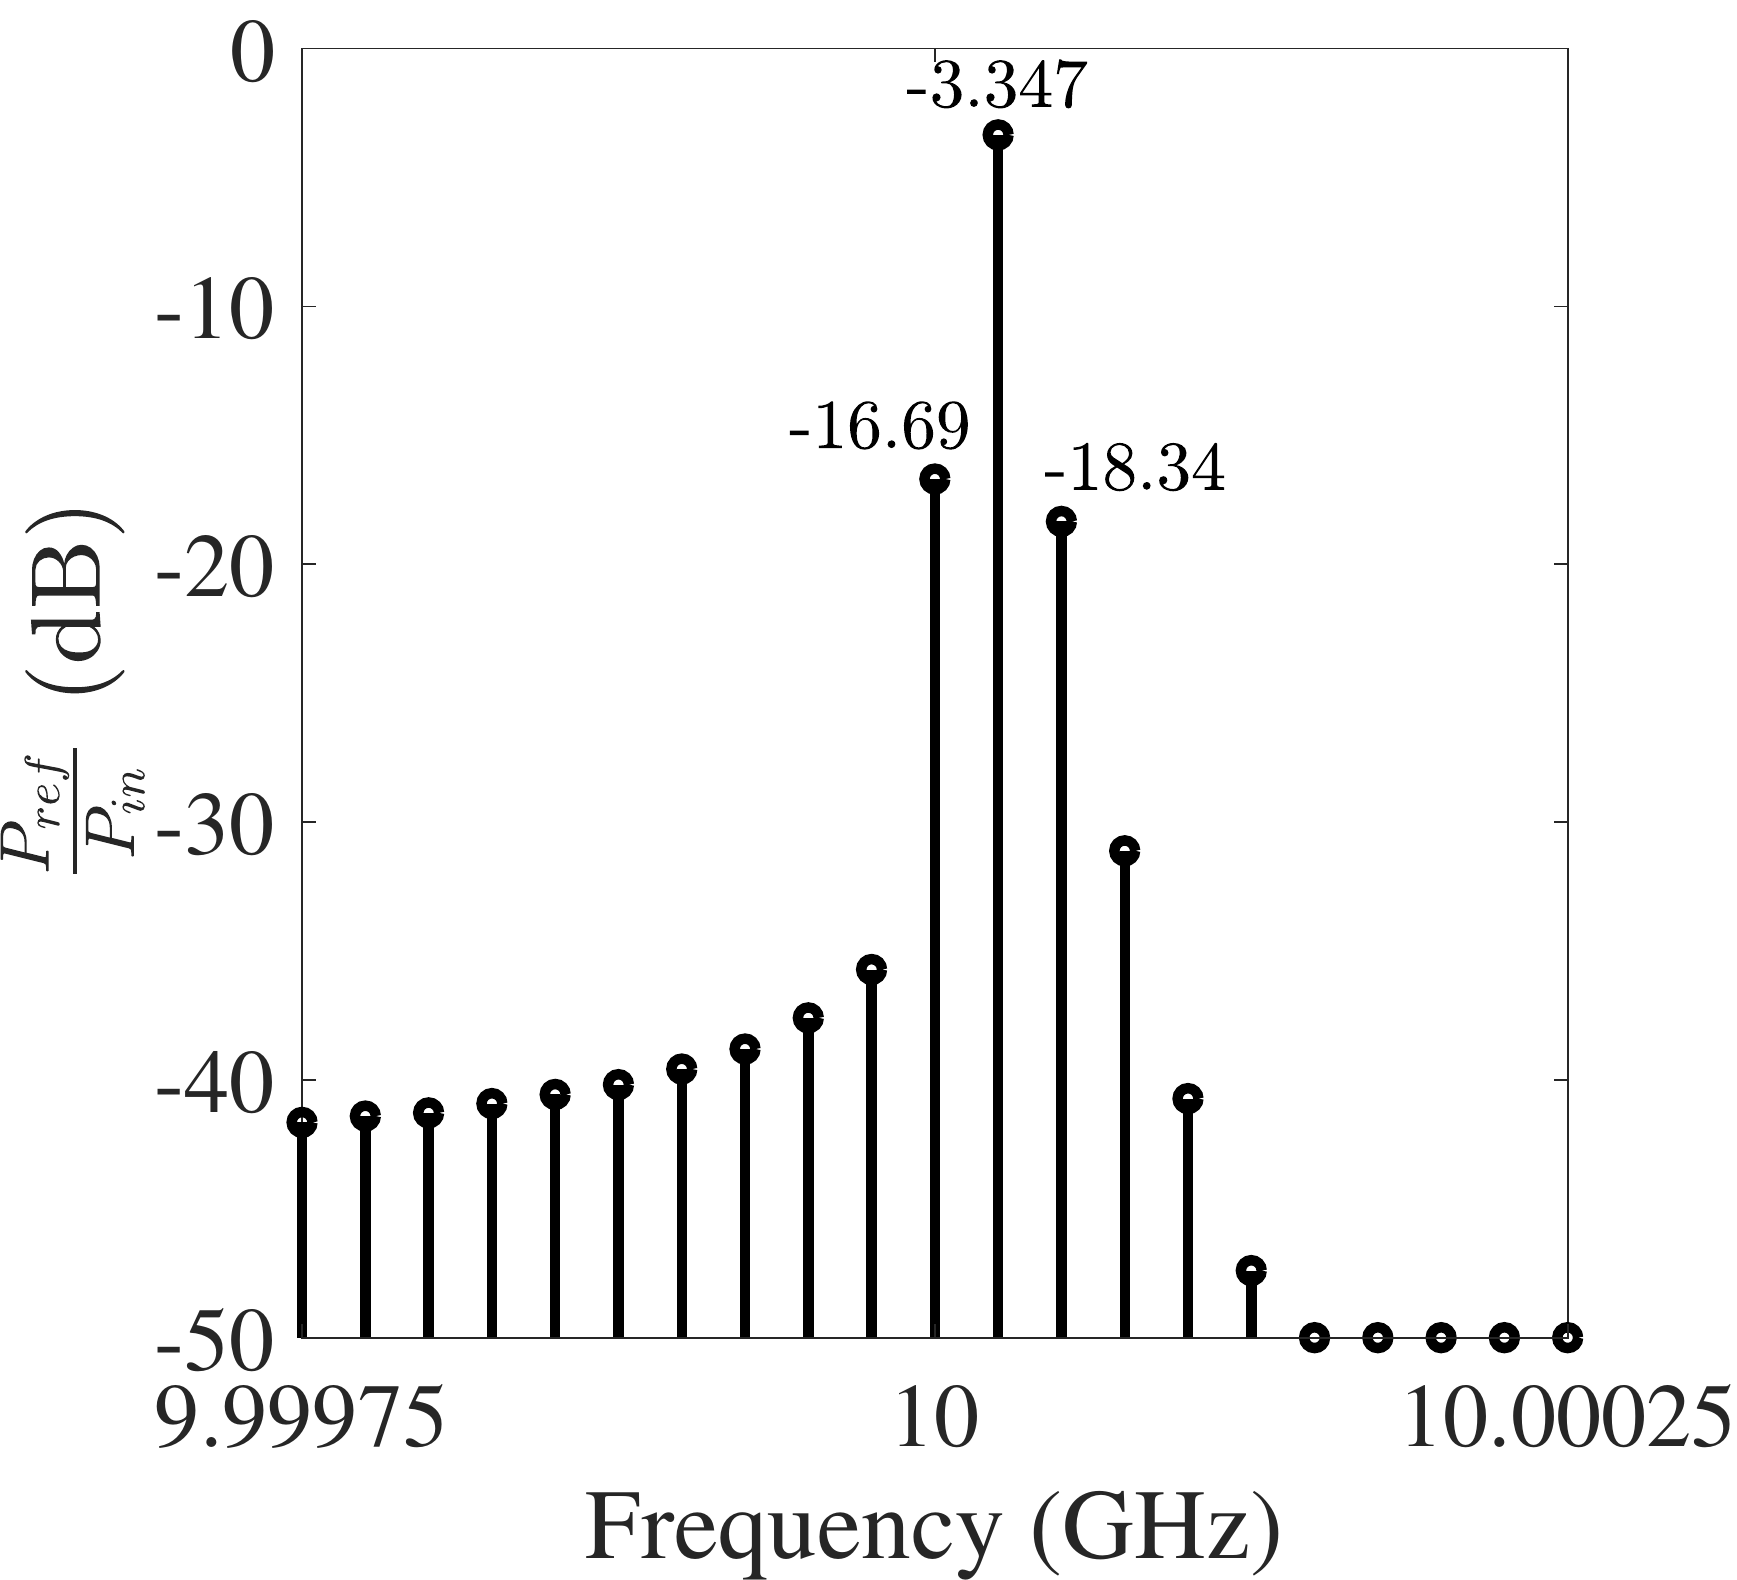}%
}\hfill
\subfloat[\label{sfig:Waveform_TM}]{%
  \includegraphics[clip,width=0.25\columnwidth]{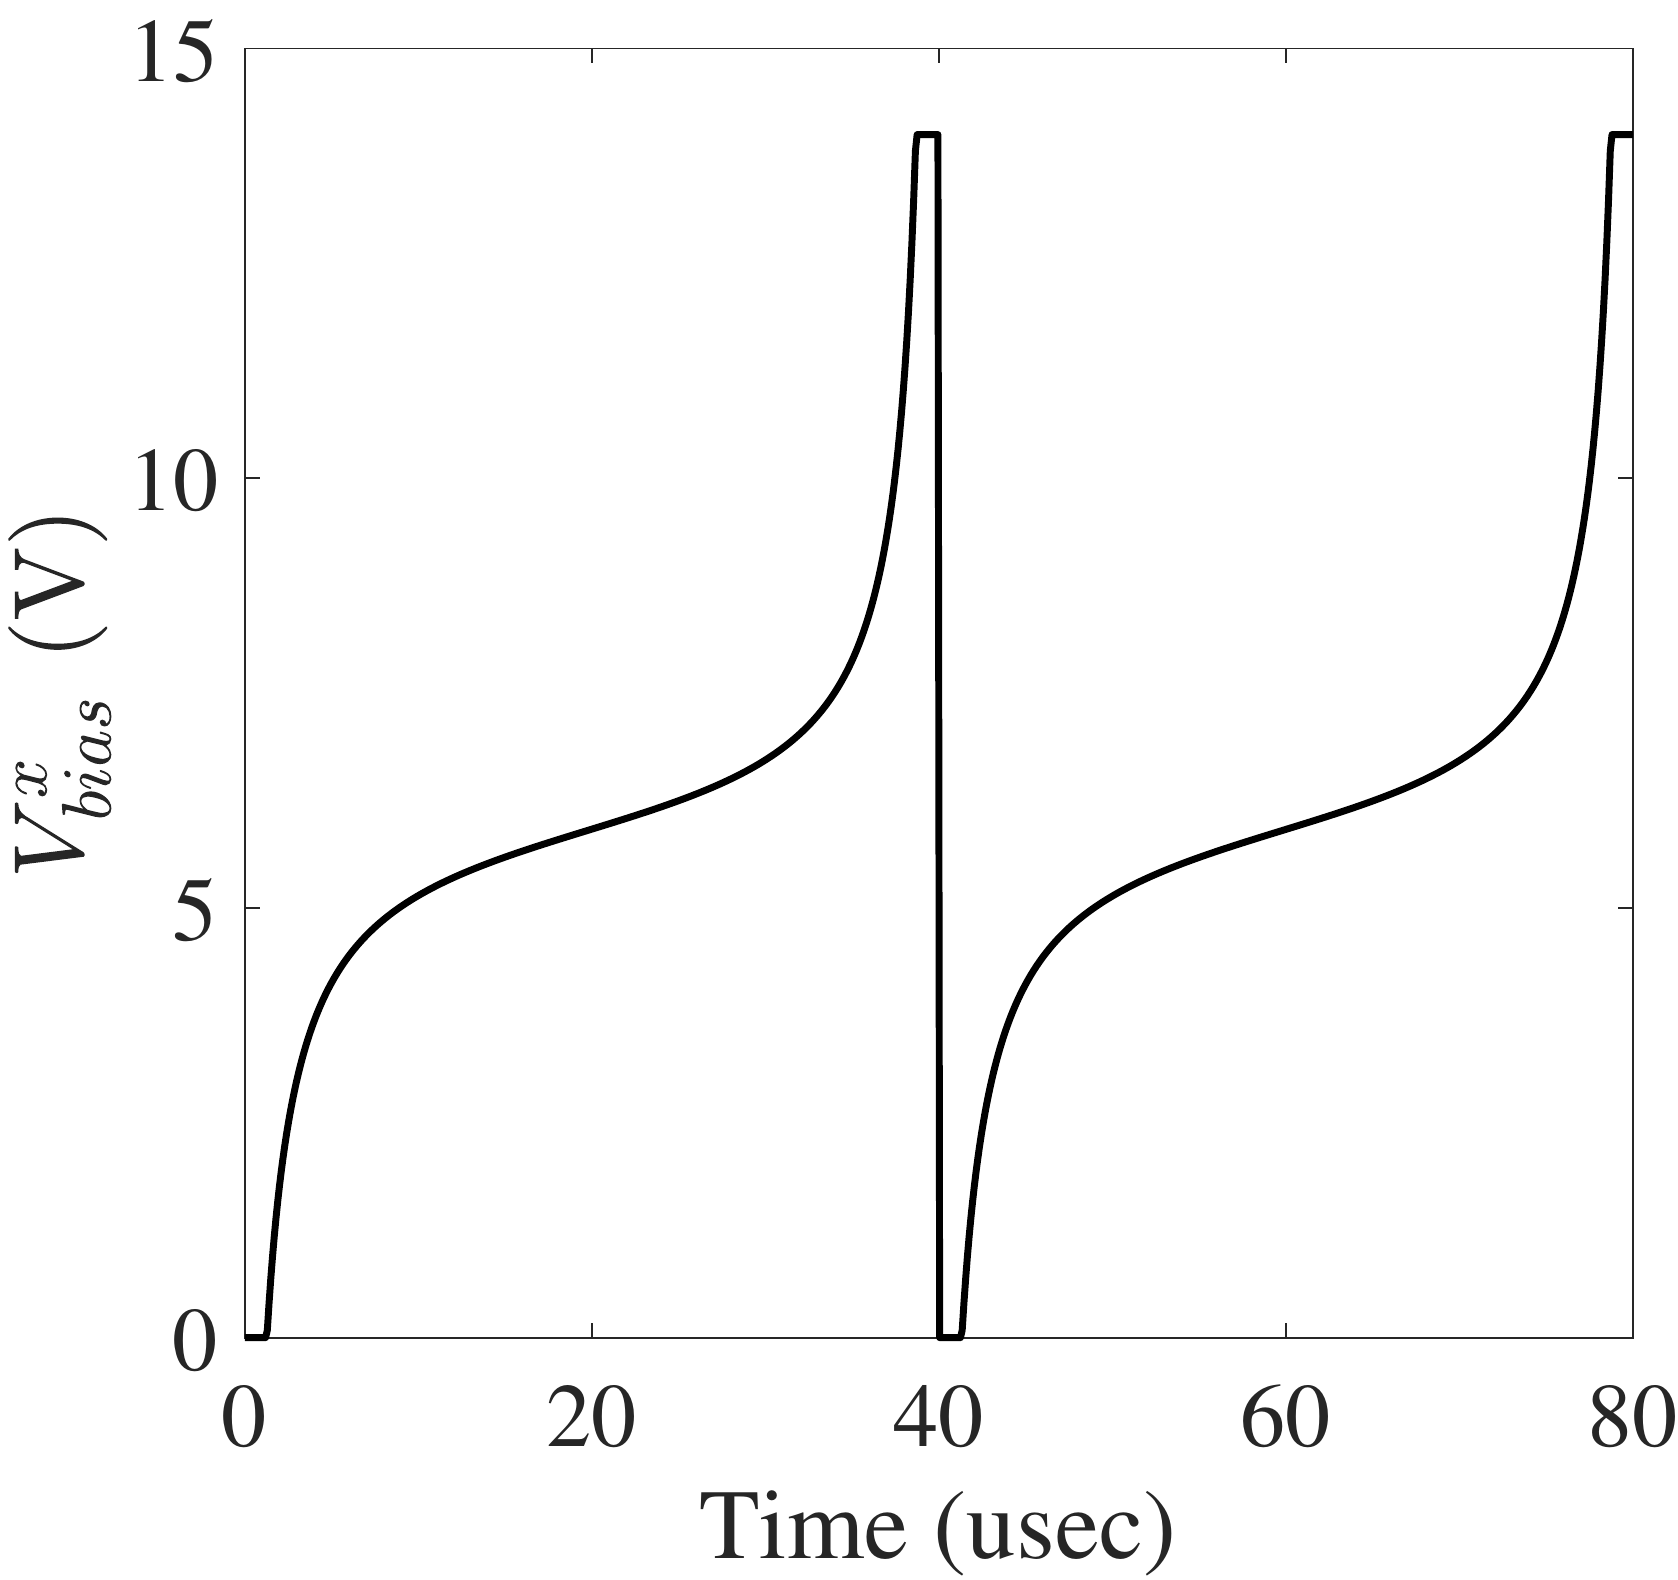}%
}\hfill
\subfloat[\label{sfig:TM1path_Sim}]{%
  \includegraphics[clip,width=0.25\columnwidth]{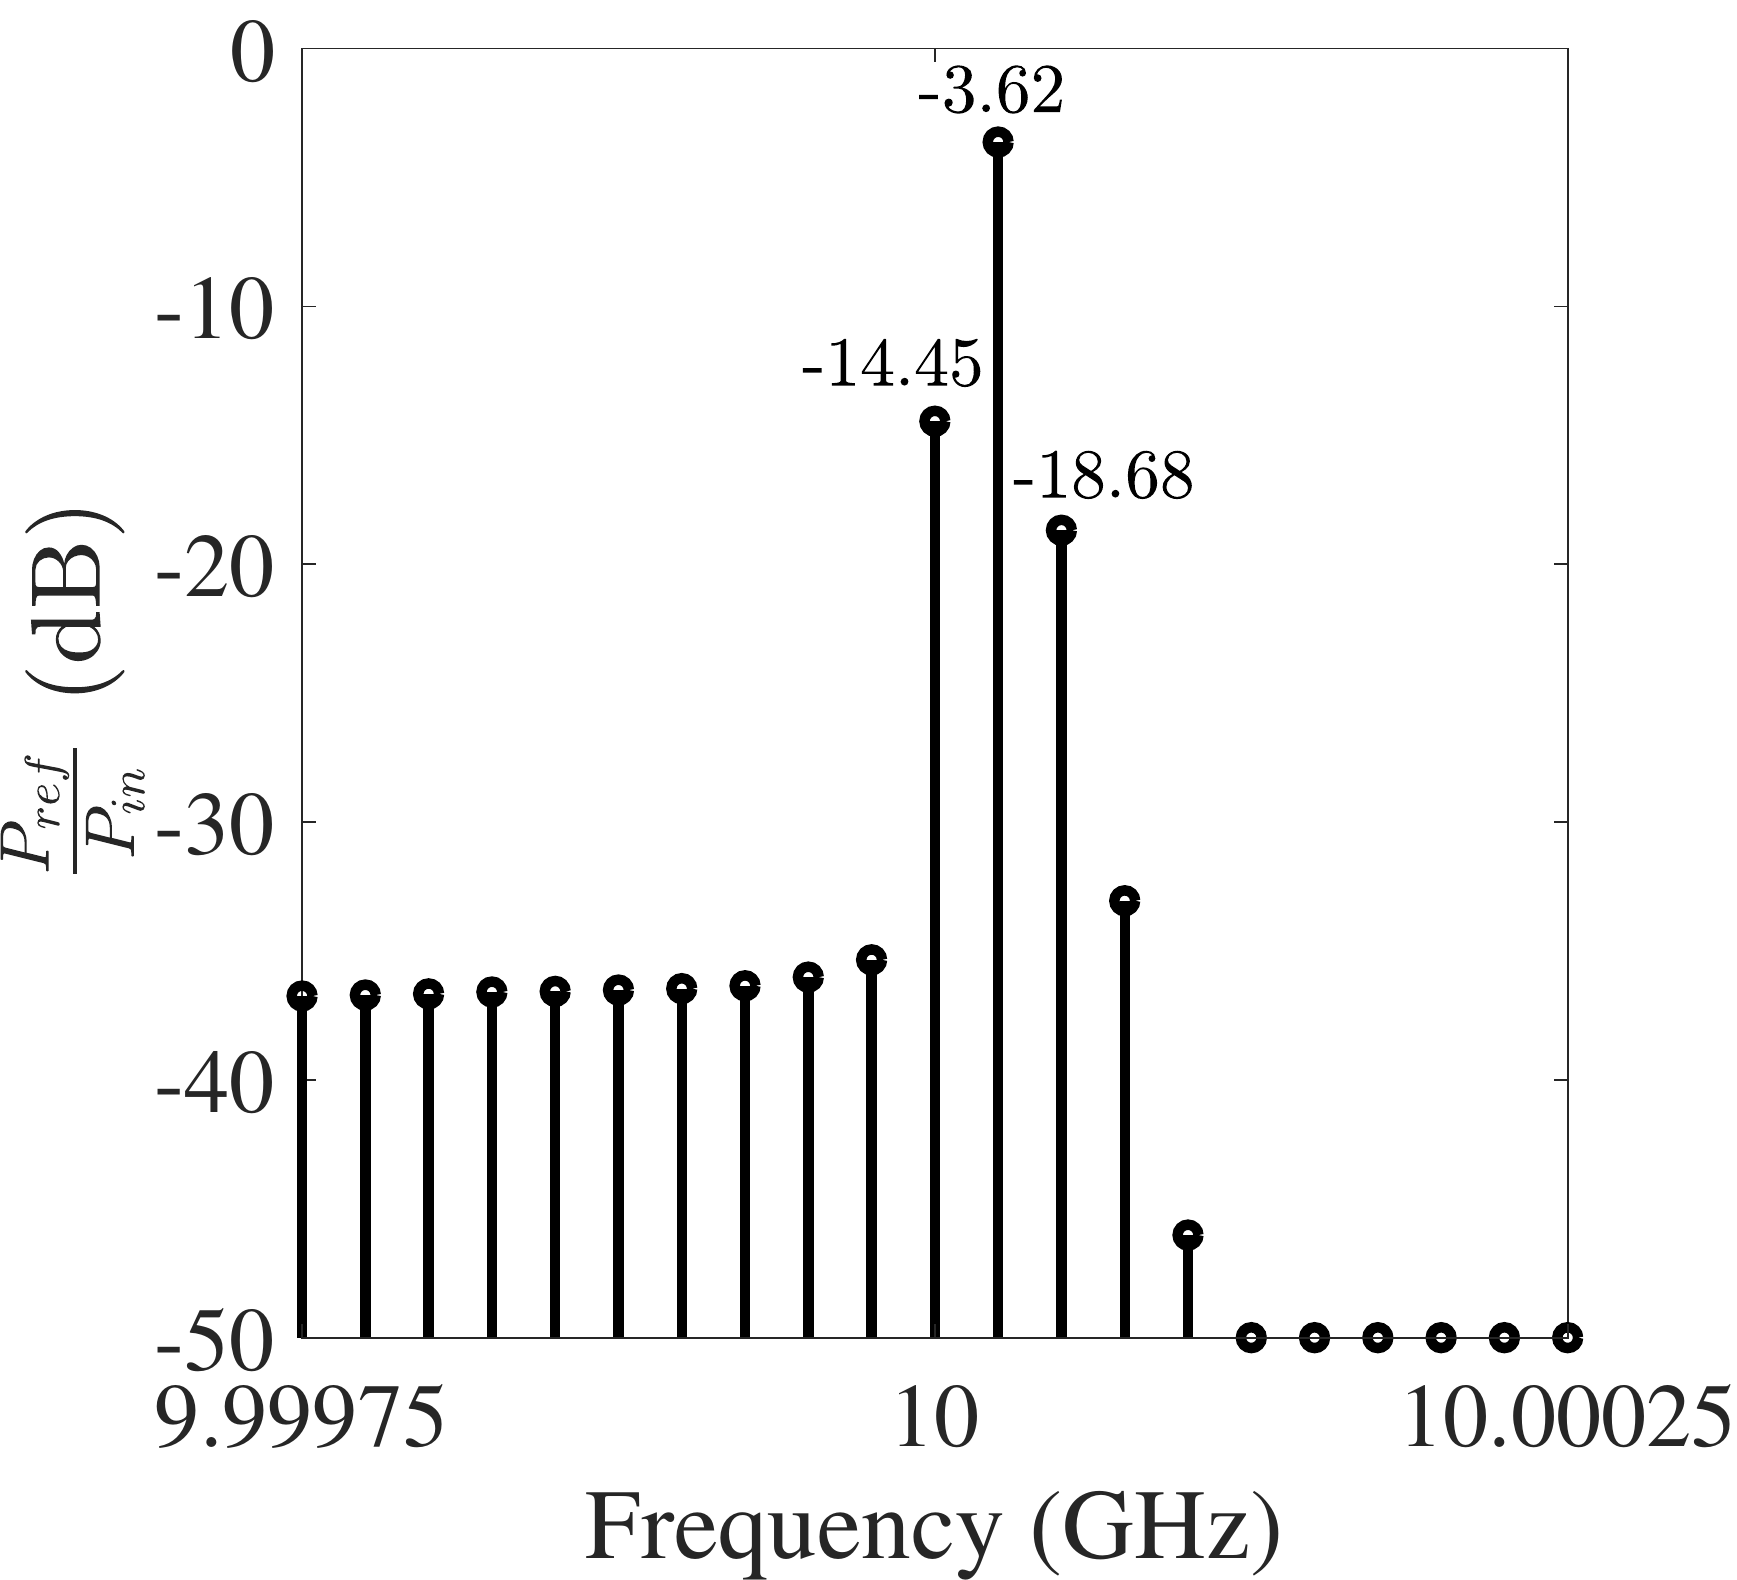}%
}\quad
\caption{(a) Optimized bias waveform for a TE polarization. (b) Reflection spectrum from harmonic balance simulation of the extracted circuit shown in Fig. \ref{sfig:CircuitTE}. The bias waveform is given in Fig. \ref{sfig:Waveform_TE}. (c) Optimized bias waveform for TM polarization. (d) Reflection spectrum from harmonic balance simulation of the extracted circuit shown in Fig. \ref{sfig:CircuitTM}. The bias waveform is given in Fig. \ref{sfig:Waveform_TM}.}
\label{fig:1pathSim}
\end{figure} 

\begin{figure}[t!]
\centering
\subfloat[\label{sfig:Waveform_TE_Sin}]{%
  \includegraphics[clip,width=0.25\columnwidth]{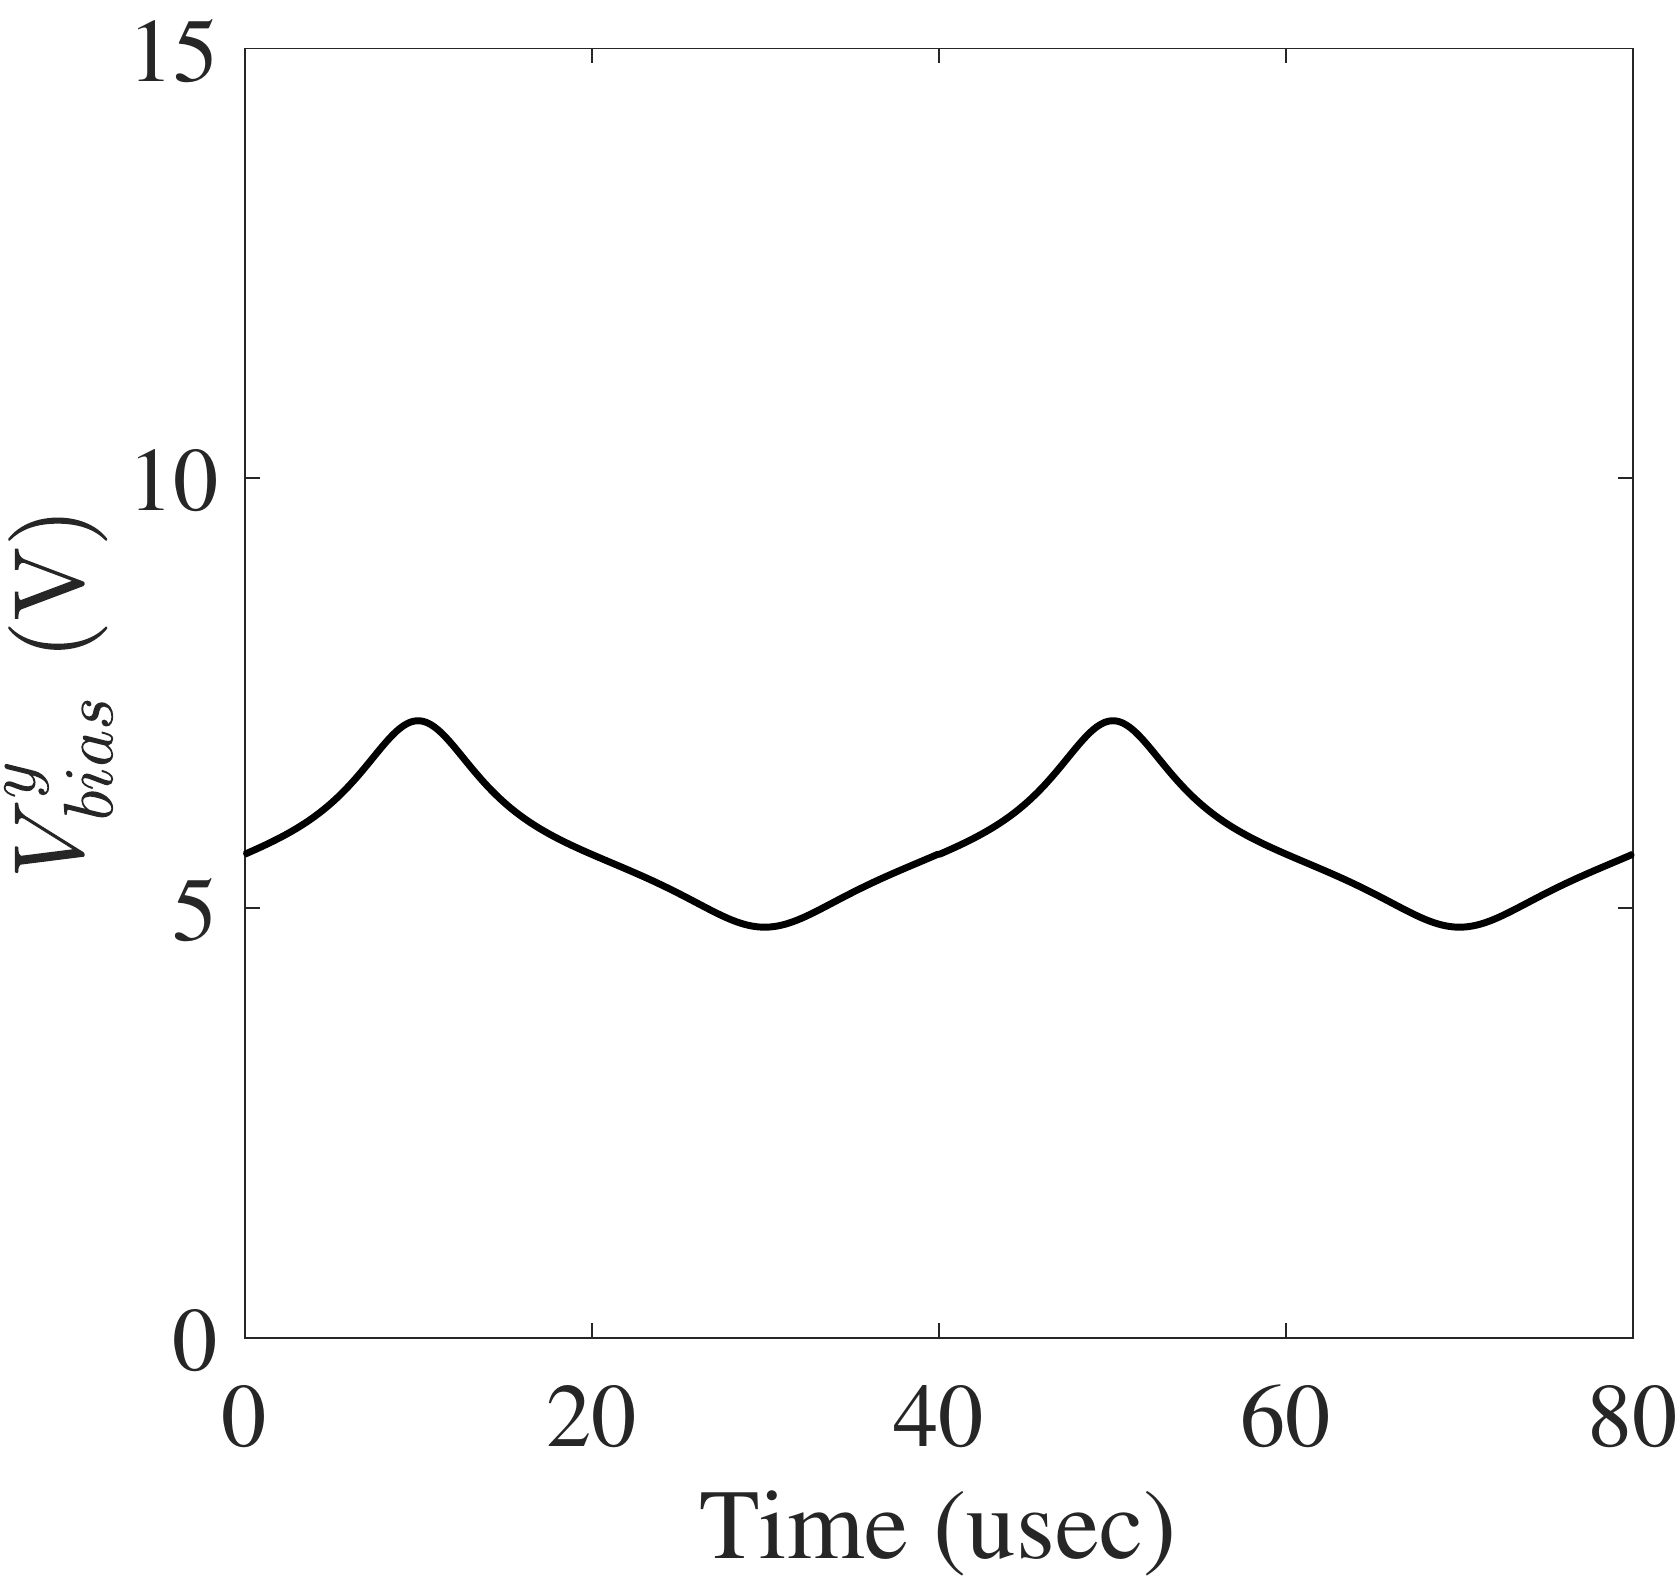}%
}\hfill
\subfloat[\label{sfig:TE1path_Sim_Sin}]{%
  \includegraphics[clip,width=0.25\columnwidth]{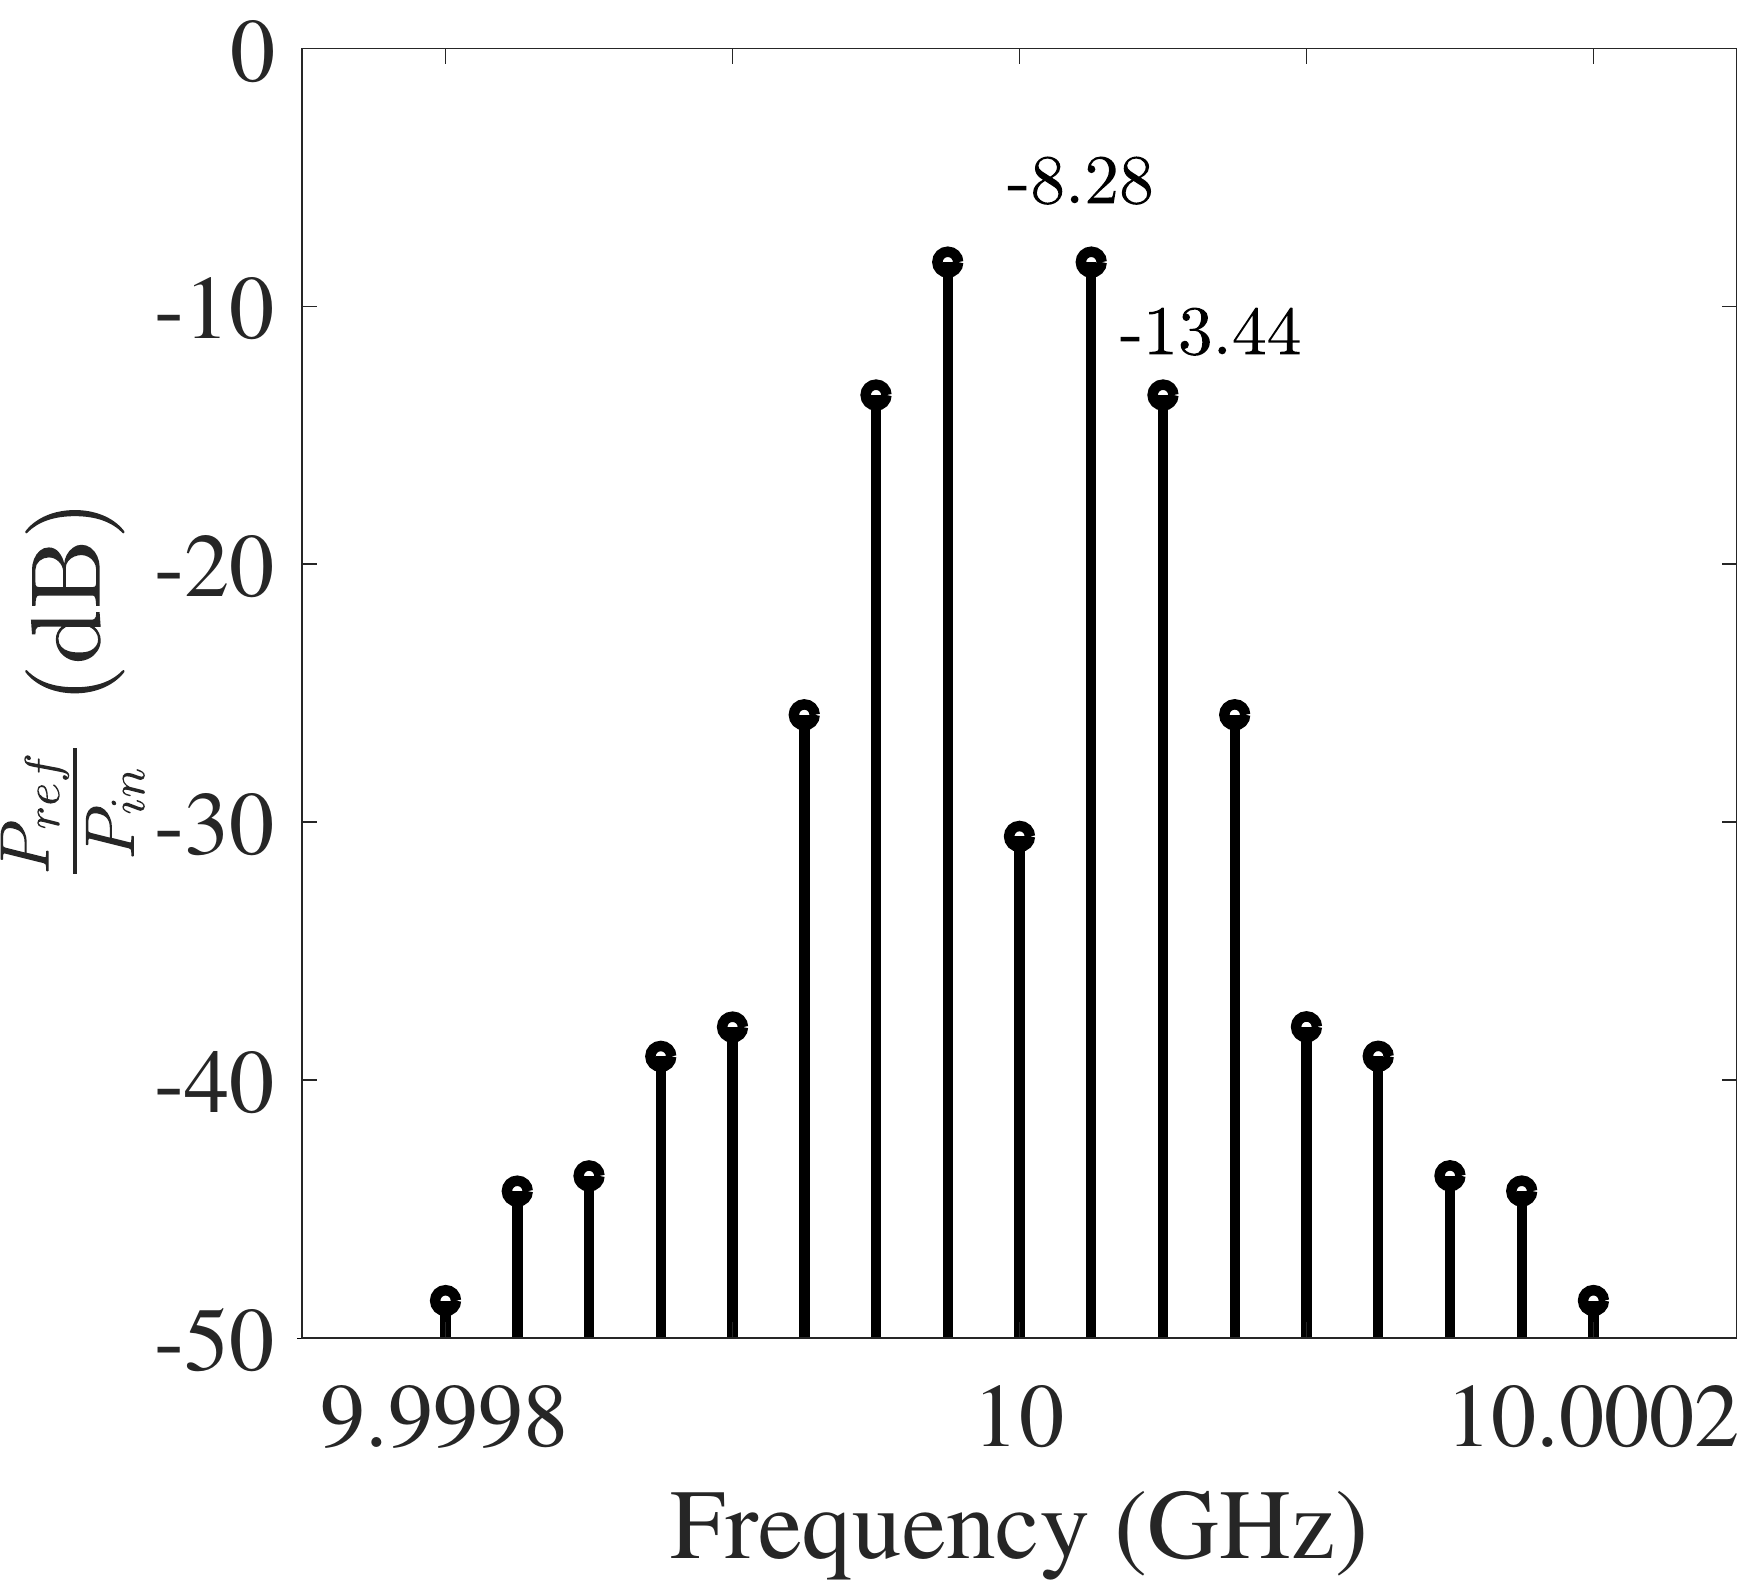}%
}\hfill
\subfloat[\label{sfig:Waveform_TM_Sin}]{%
  \includegraphics[clip,width=0.25\columnwidth]{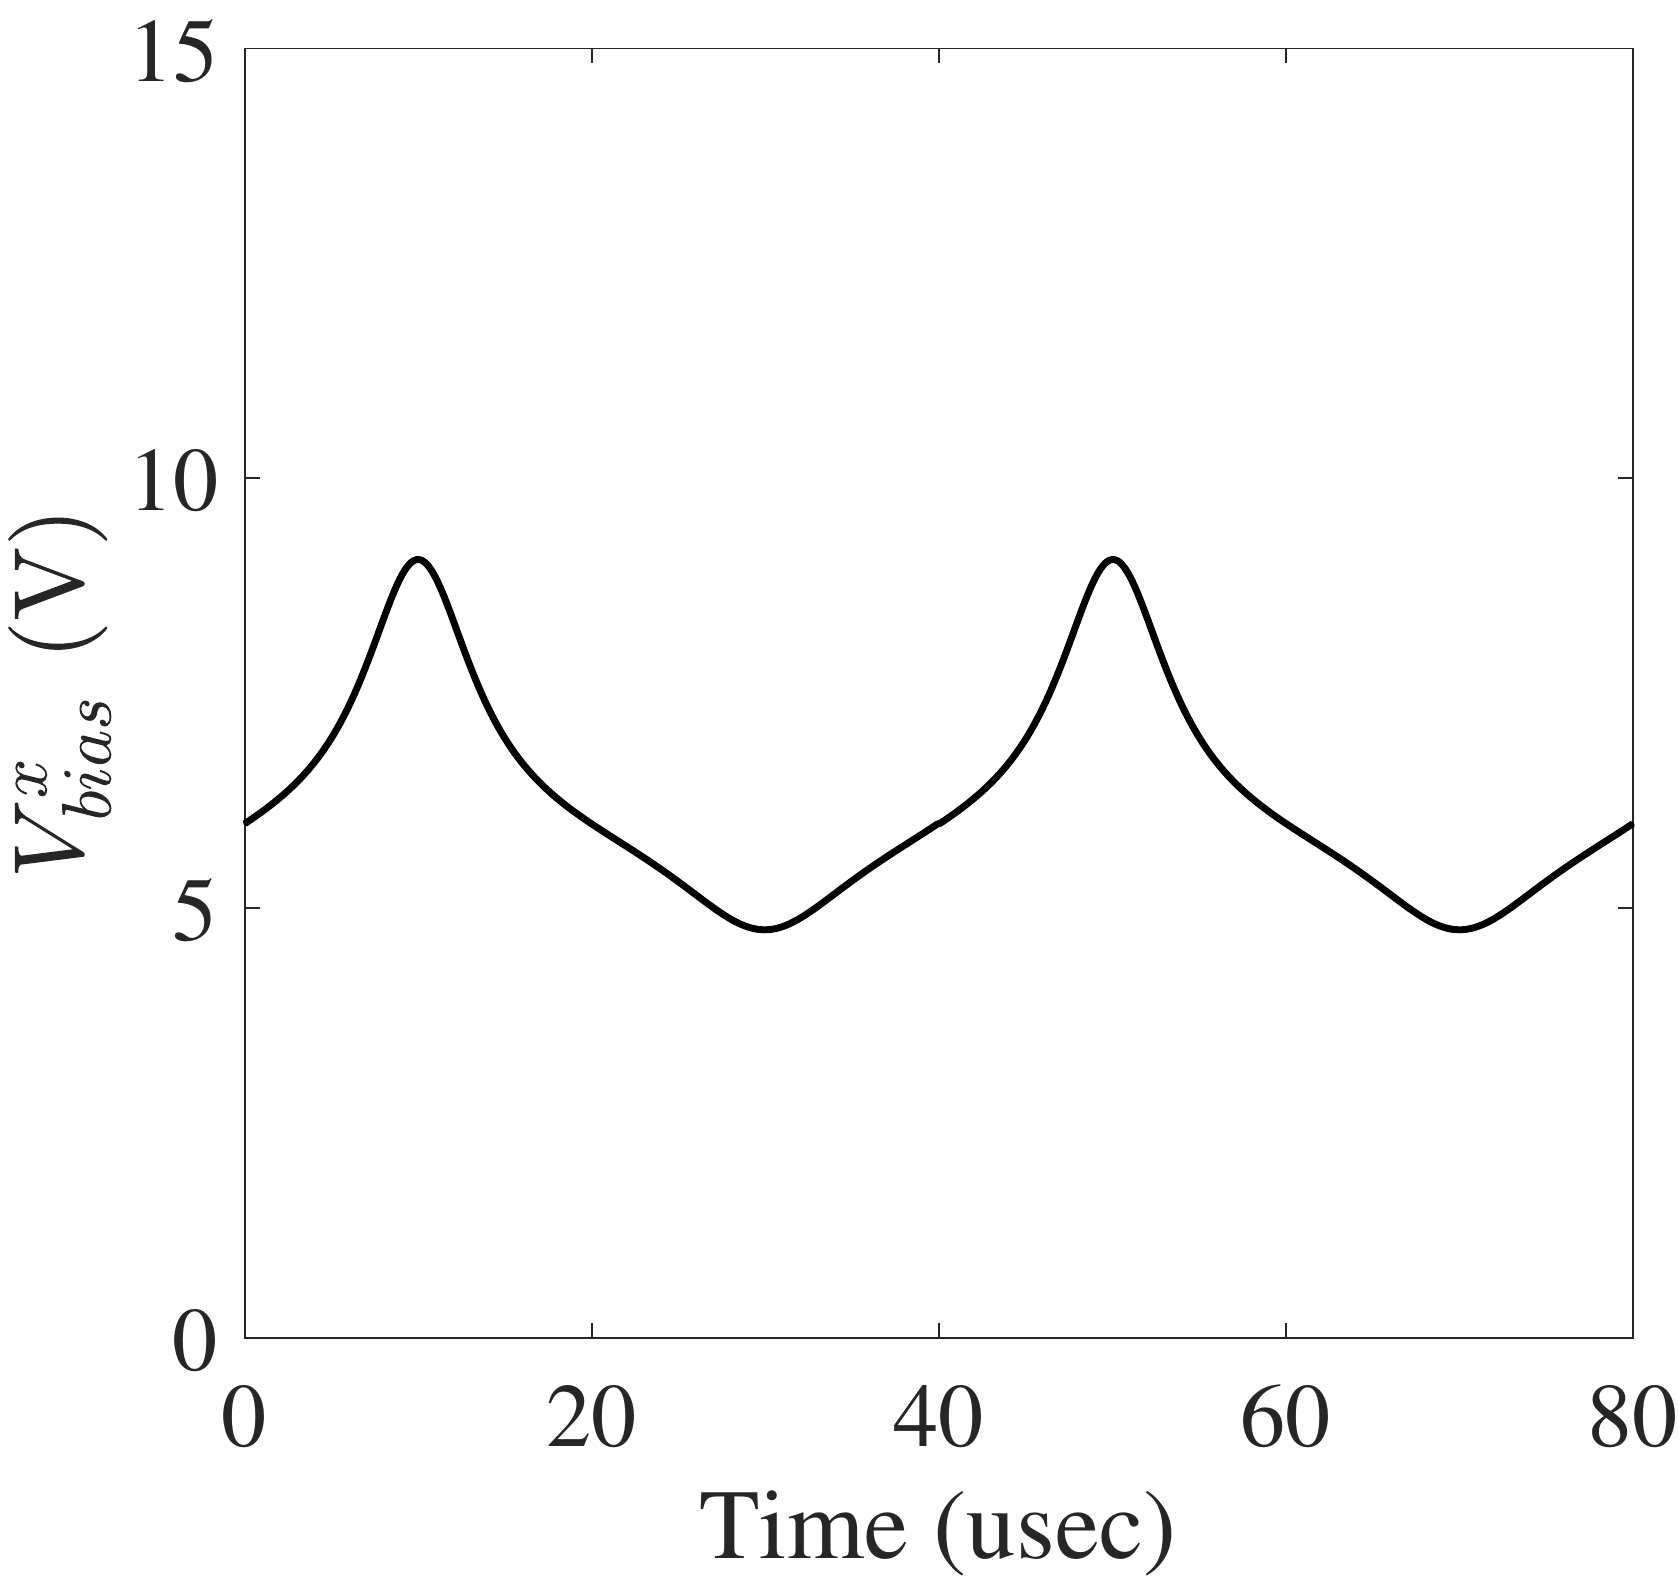}%
}\hfill
\subfloat[\label{sfig:TM1path_Sim_Sin}]{%
  \includegraphics[clip,width=0.25\columnwidth]{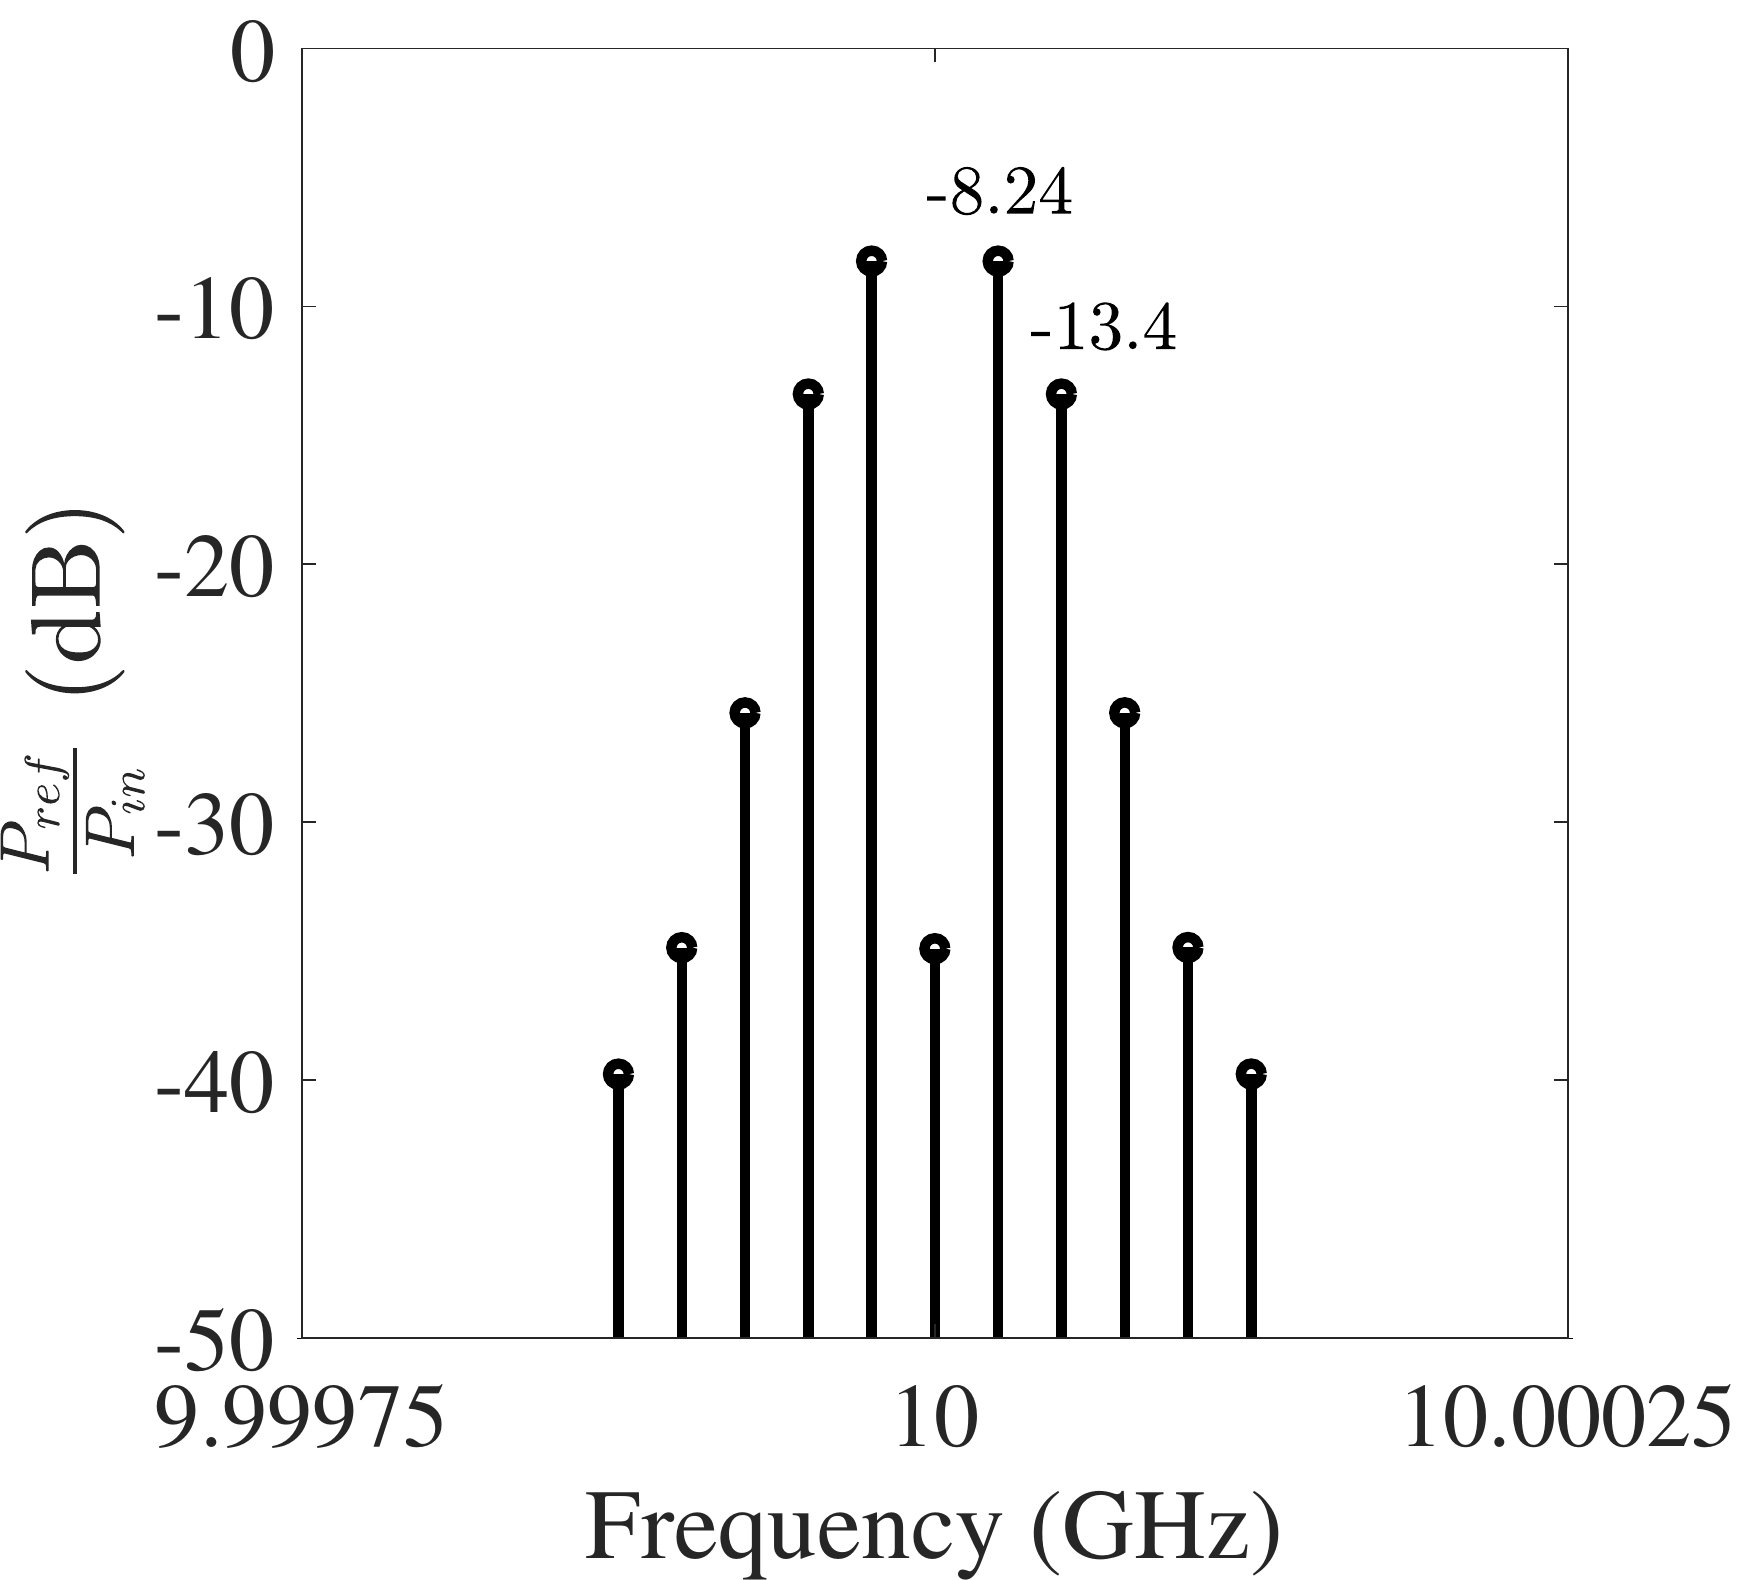}%
}\quad
\caption{(a) Optimized bias waveform for a TE polarization. (b) Reflection spectrum from harmonic balance simulation of the extracted circuit shown in Fig. \ref{sfig:CircuitTE}. The bias waveform is given in Fig. \ref{sfig:Waveform_TE_Sin}. (c) Optimized bias waveform for TM polarization. (d) Reflection spectrum from harmonic balance simulation of the extracted circuit shown in Fig. \ref{sfig:CircuitTM}. The bias waveform is given in Fig. \ref{sfig:Waveform_TM_Sin}}
\label{fig:1pathSim_Sin}
\end{figure} 

When the reflection phase is a sawtooth function in time, the simulated reflection spectra are given in Fig. \ref{sfig:TE1path_Sim} and \ref{sfig:TM1path_Sim}. The simulation results agree with the measurement results shown in Fig. 26. However, the measured results shows higher conversion loss and lower sideband suppression. This can be attributed to the fact that the measured bias waveform is a coarsely sampled version of the optimized waveform. The sampling rate of the D/A converter used in experiment is $0.5$ MHz. Therefore, only 20 samples per period could be taken of the $25$ KHz modulation waveform. 
For a reflection phase that is a sinusoidal function of time, the simulated reflection spectra are given in Fig. \ref{sfig:TE1path_Sim_Sin} and \ref{sfig:TM1path_Sim_Sin}. 

\begin{figure}[t!]
\centering
\subfloat[\label{sfig:TE2path_Sim}]{%
  \includegraphics[clip,width=0.25\columnwidth]{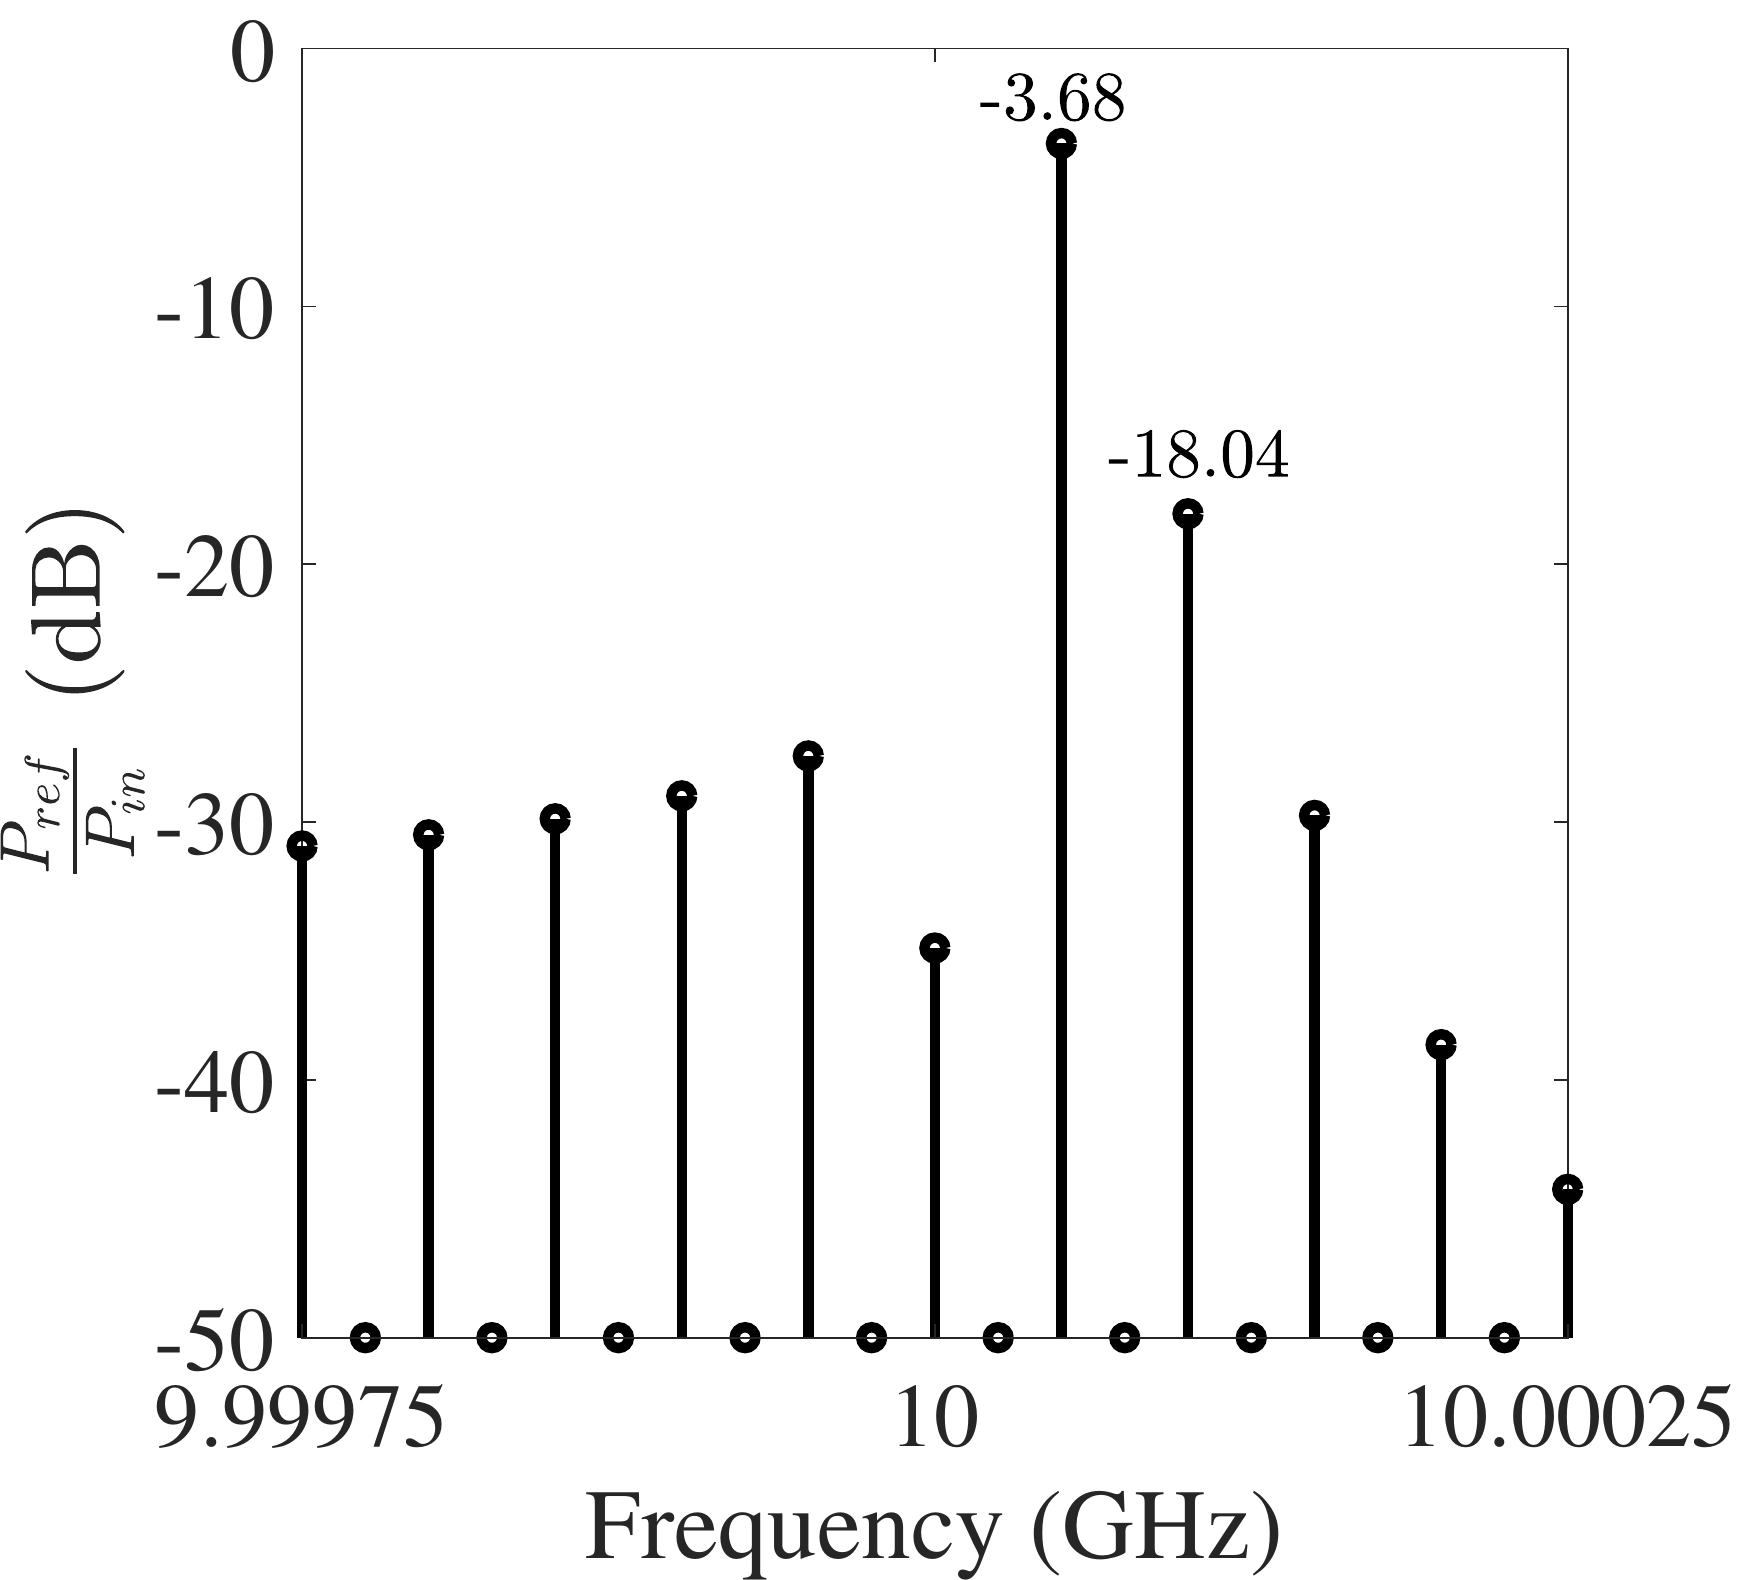}%
}\hfill
\subfloat[\label{sfig:TE3path_Sim}]{%
  \includegraphics[clip,width=0.25\columnwidth]{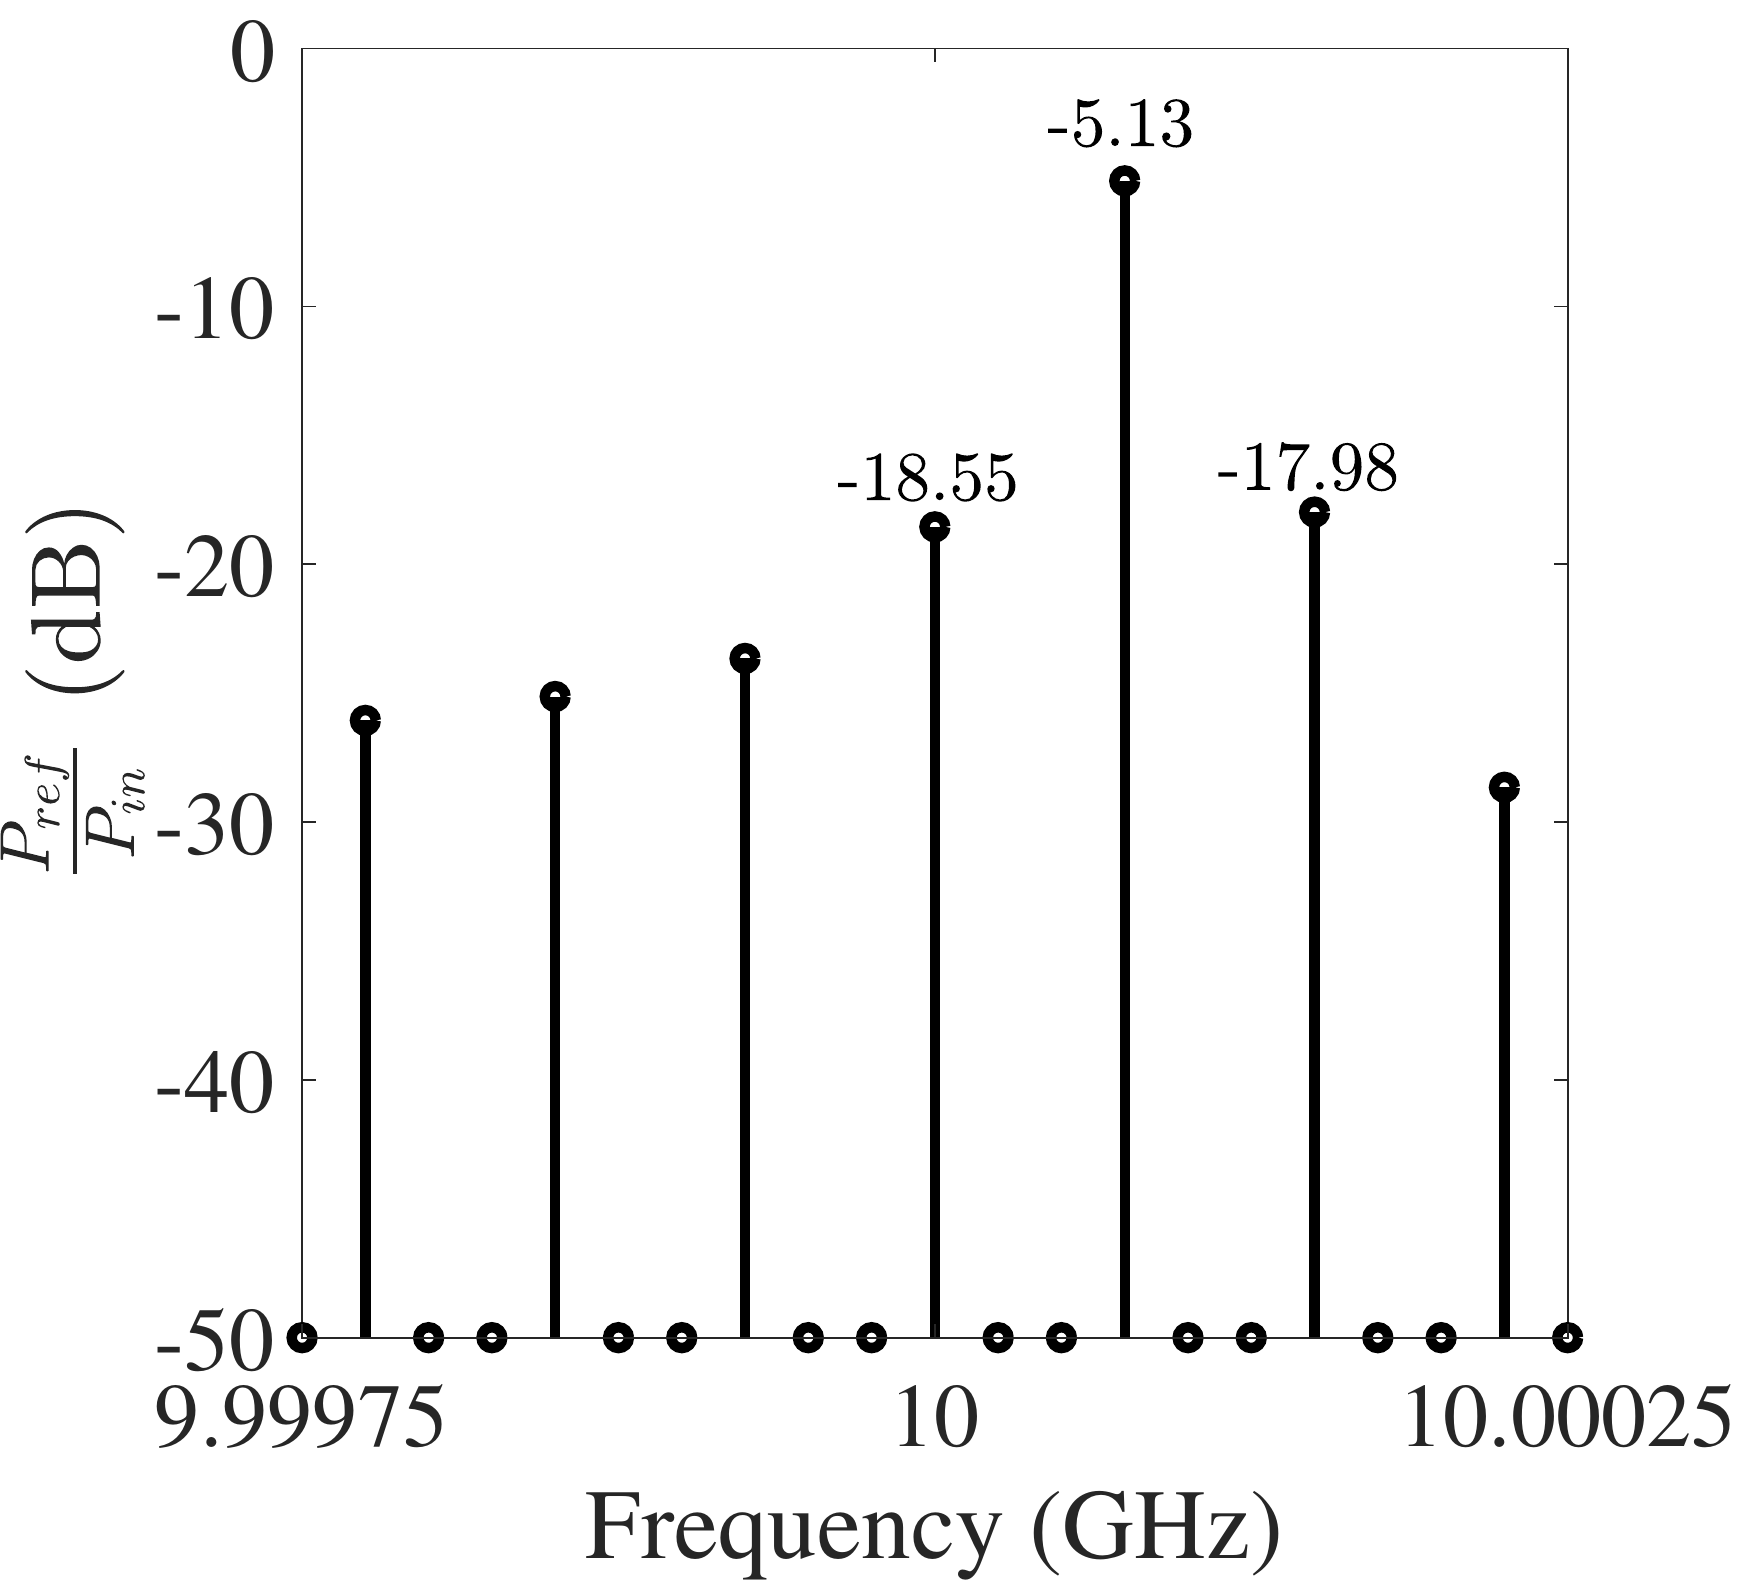}%
}\hfill
\subfloat[\label{sfig:TM2path_Sim}]{%
  \includegraphics[clip,width=0.25\columnwidth]{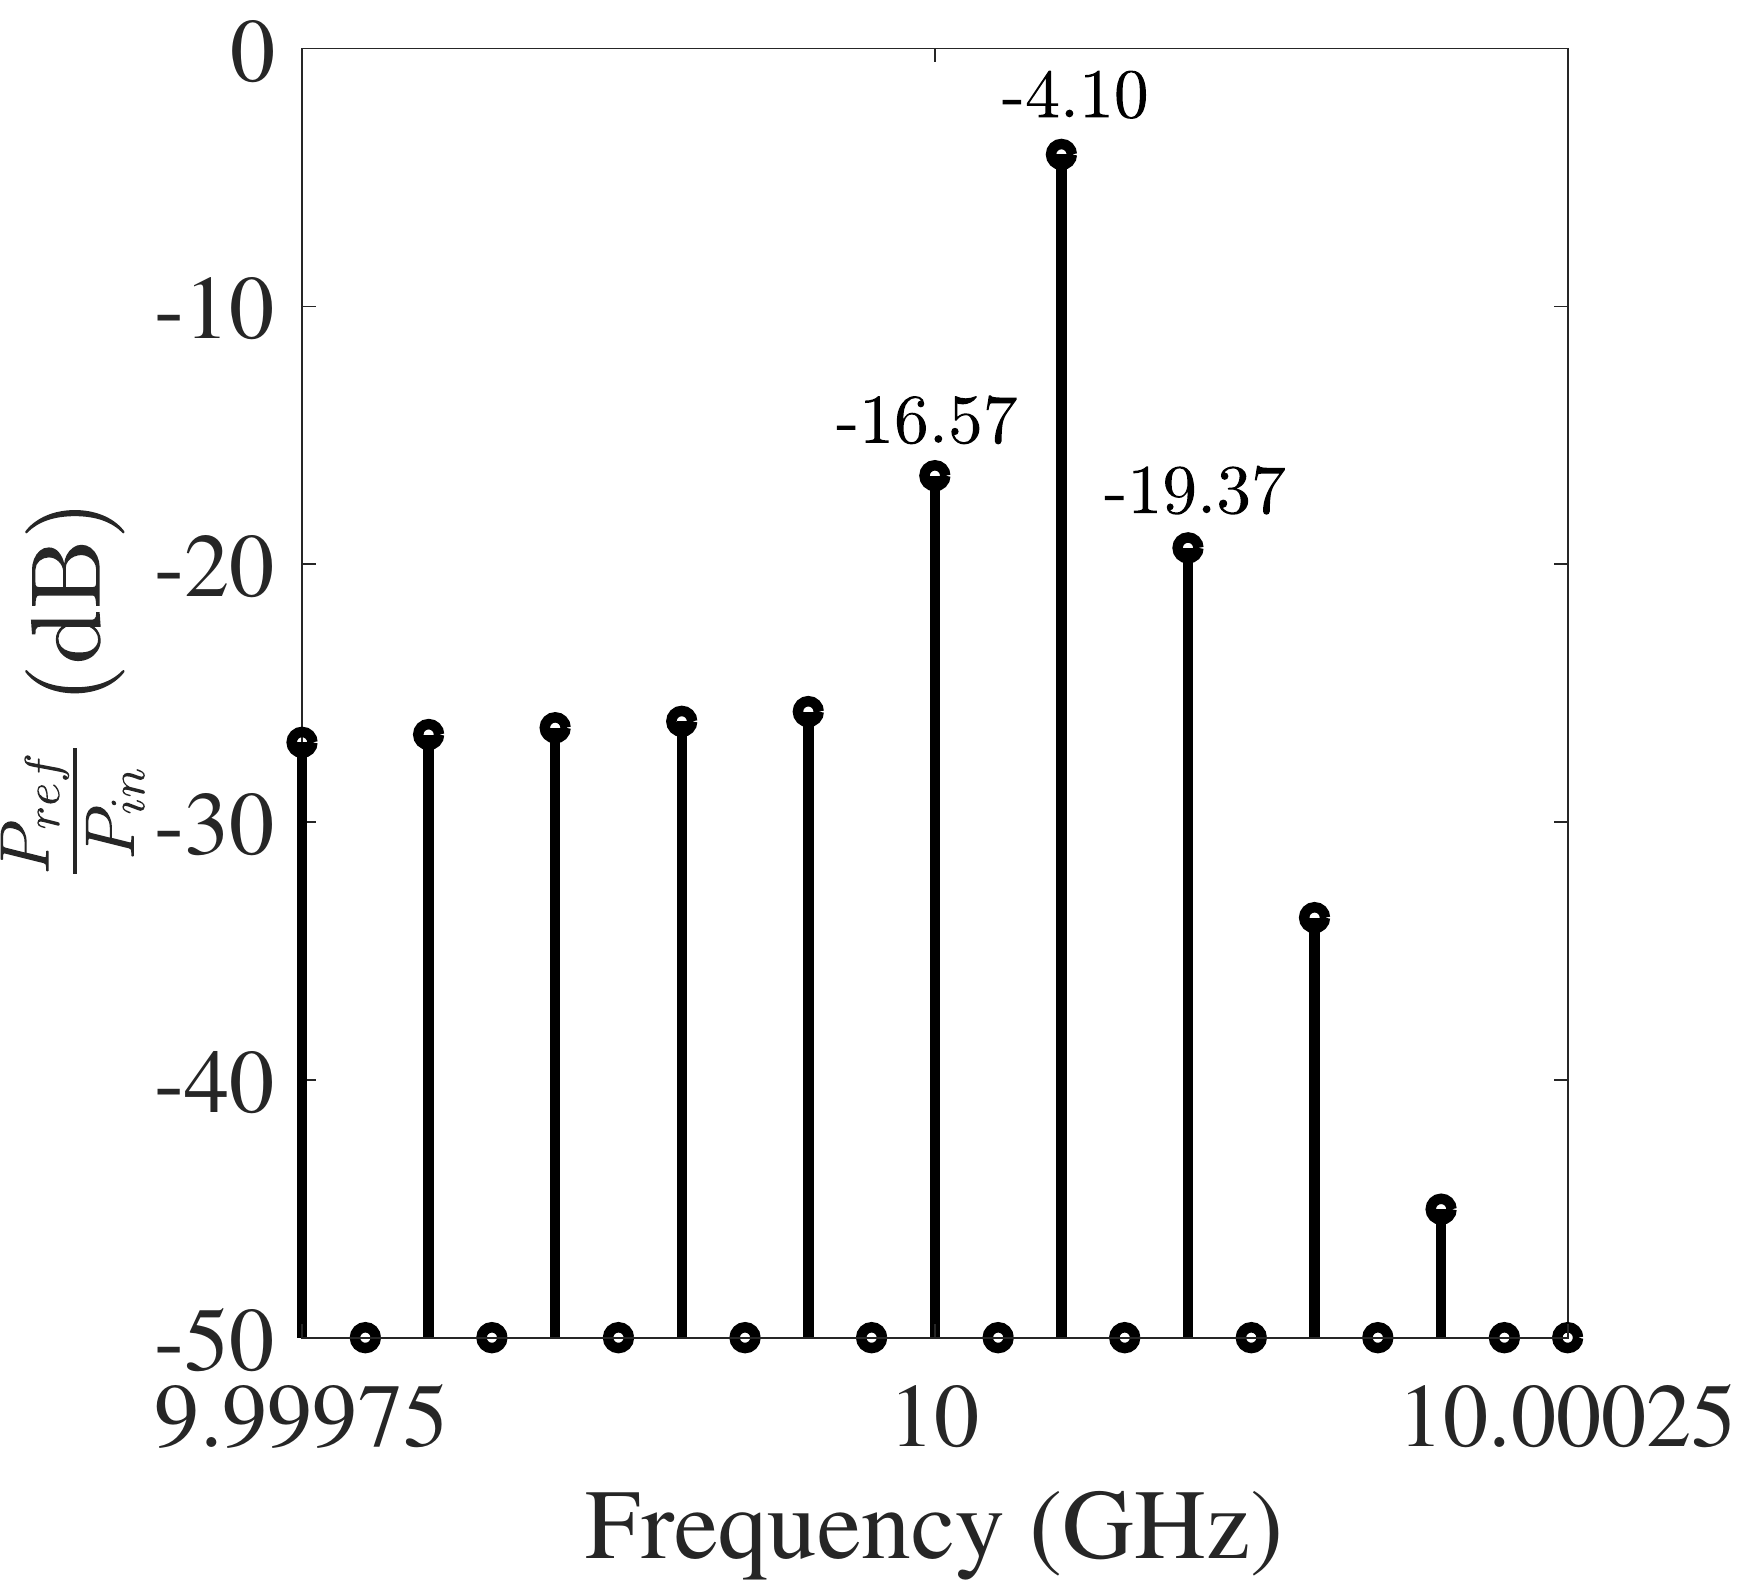}%
}\hfill
\subfloat[\label{sfig:TM3path_Sim}]{%
  \includegraphics[clip,width=0.25\columnwidth]{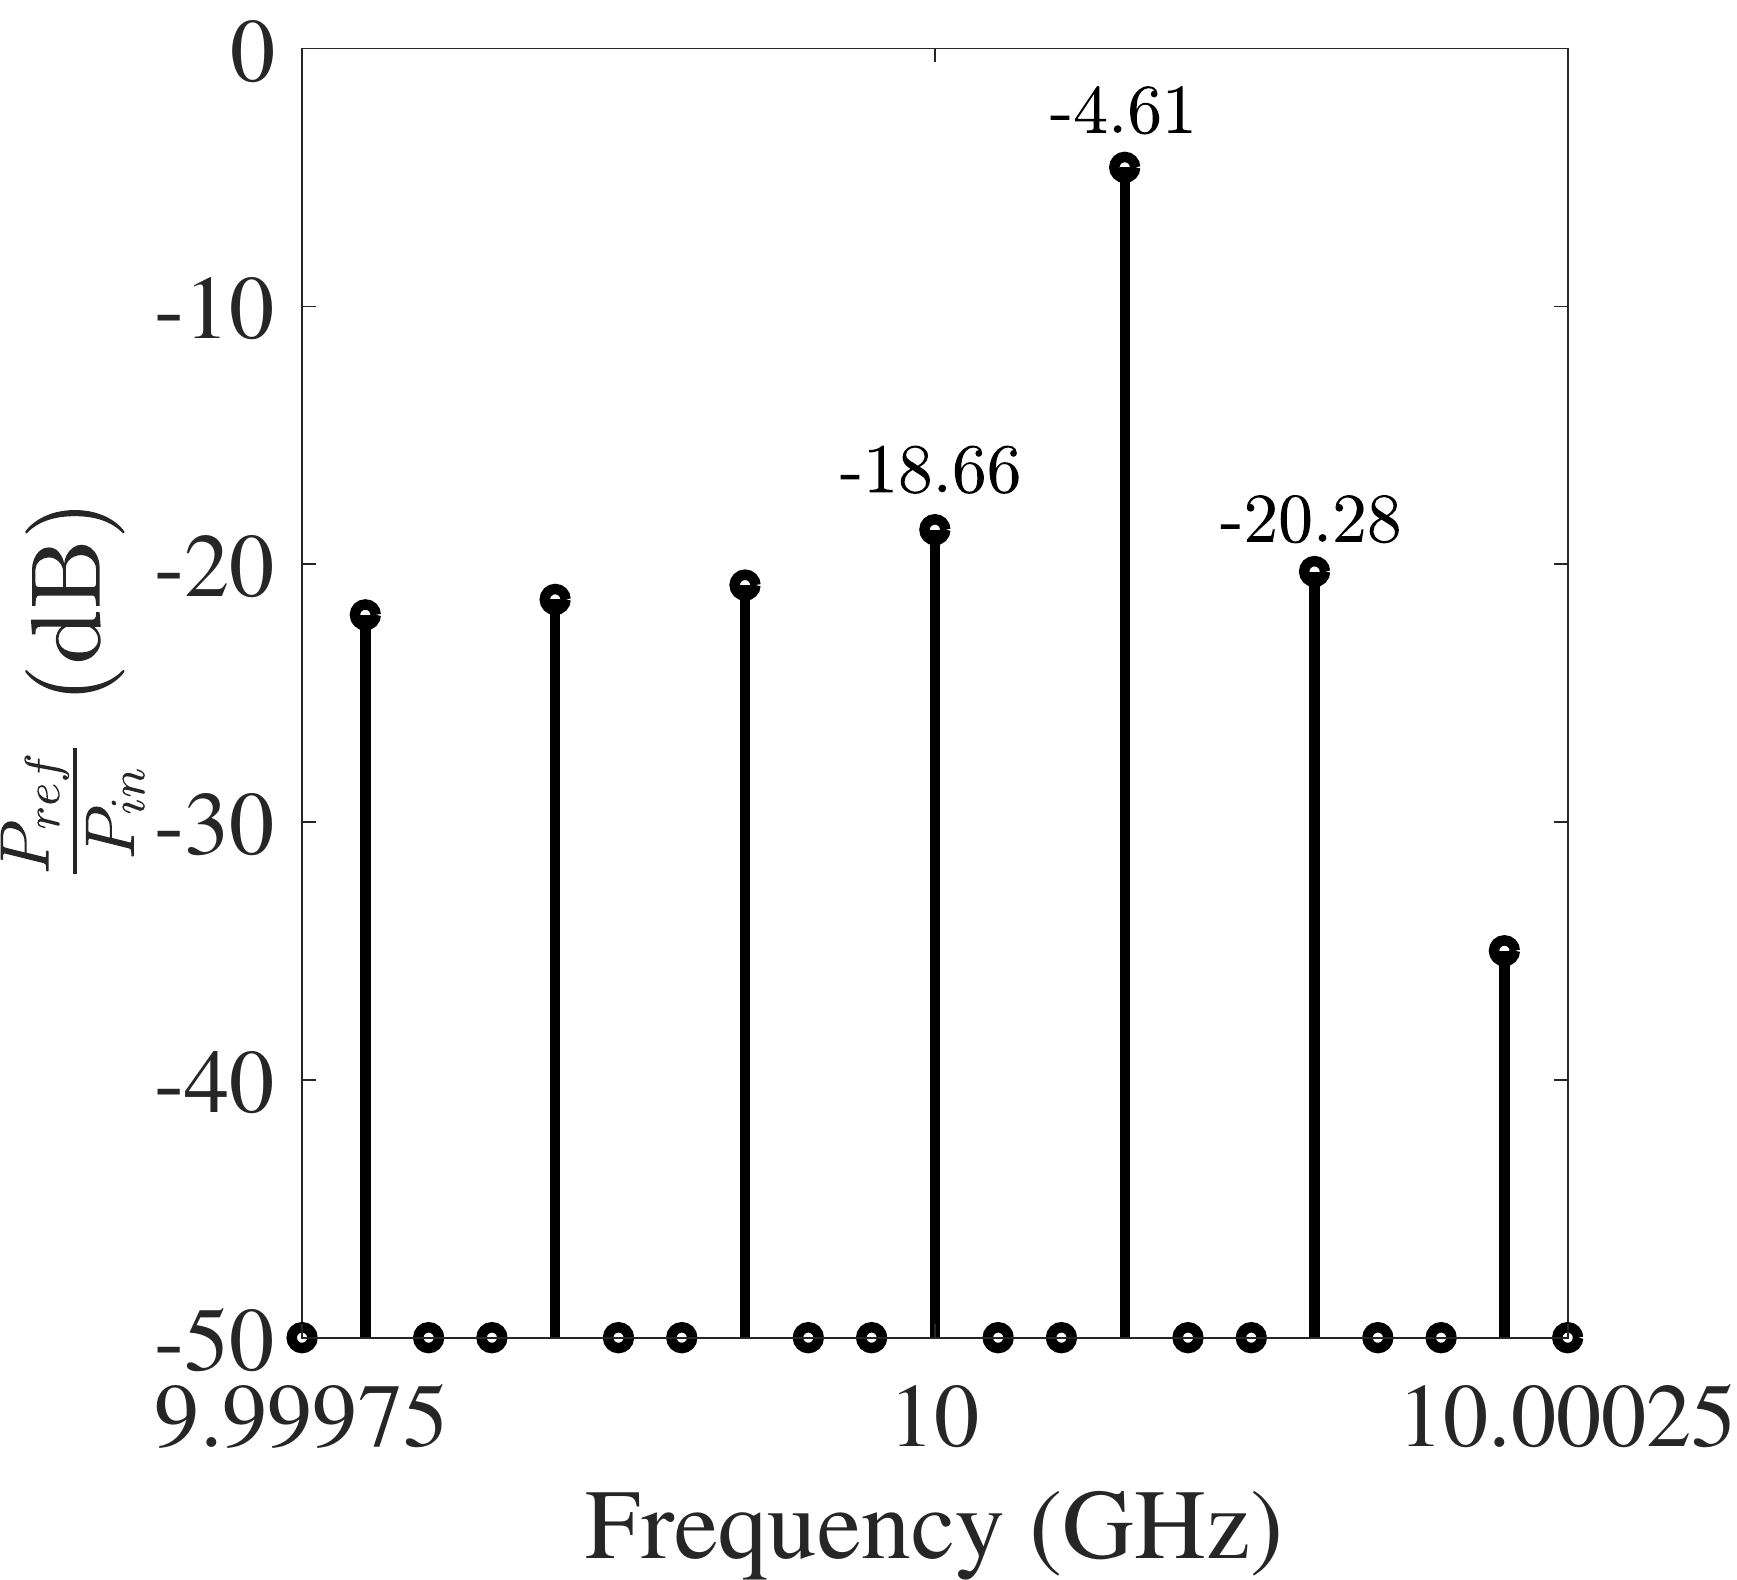}%
}\quad
\caption{Reflection spectrum from harmonic balance simulation of the N-path circuit model depicted in Fig. 9. Each path is represented by the extracted circuit models shown in Fig. \ref{fig:ExtractCircuit}. (a) 2-path ($N=2$) modulation for TE polarization. (b) 3-path ($N=3$) modulation for TE polarization.  (c) 2-path ($N=2$) modulation for TM polarization. (d) 3-path ($N=3$) modulation for TM polarization. }
\label{fig:123path_Sim}
\end{figure} 

%\clearpage

As mentioned in the paper, when the spatial modulation period is small, the metasurface can be viewed as an N-path system. Subharmonic frequency translation is supported in this case, and the metasurface exhibits Doppler-like frequency translation to a high-order frequency harmonic. The metasurface can be represented using an N-path circuit model shown in Fig. 8, where there are $N$ branches of time-varying circuits connected to a common port. Each path (column of metasurface) is represented by a circuit model shown in Fig. \ref{fig:ExtractCircuit}. The bias wavefrom of each path is given in Fig. \ref{sfig:Waveform_TE} and \ref{sfig:Waveform_TM}; and is staggered in time by $T_p/N$ with respect to that of its adjacent path. The simulated reflection spectra for 2-path and 3-path configurations are shown in Fig. \ref{fig:123path_Sim}. Note that, as the path number $N$ increases, the conversion loss increases as well. This is because the N-path metasurface upconverts the frequency to the first propagating harmonic pair. The higher the upconverted frequency, the more loss there is in the frequency conversion process. The simulated results agree with the measurement results shown in Fig. 27. However, the conversion loss of the measured results degrade more severely as the path number increases. This is due to the fact that when the metasurface is lossy, the evanescent harmonic pairs on the metasurface consume energy as well. Those harmonic pairs are not represented in the N-path circuit network, where the $N$ branches of time-varying circuits are considered perfectly co-located.

\begin{thebibliography}{9}

\bibitem{Collin}
R. E. Collin , ``Foundations for microwave engineering'', \emph{John Wiley \& Sons}, ch. 11, pp. 799-830, 2007.

\bibitem{cody_meta}
C. Scarborough, and A. Grbic ``Modified Floquet Boundary Condition for Open Boundary Problems with N-Path Symmetry'', \emph{2020 14th International Congress on Artificial Materials for Novel Wave Phenomena (Metamaterials)}, 2020.

%\bibitem{Npath}
%C. Scarborough, and A. Grbic ``Accelerated N-Path Network Analysis Using the Floquet Scattering Matrix Method'', \emph{IEEE Transactions on Microwave Theory and Techniques}, vol. 64, pp. 1248-1259, 2020.

\bibitem{Tsang}
L. Tsang, J. A. Kong, and K. H. Ding ``Scattering of electromagnetic waves: theories and application,'' vol. 27, John Wiley \& Sons, 2004.

\bibitem{Shaltout}
A. M. Shaltout, A. Kildishev, and V. Shalaev ``Time-varying  metasurfaces  and  lorentz  non-reciprocity,'' \emph{Optical  Materials  Express}, vol. 5, pp. 2459–2467, 2015.

\bibitem{MACOM}
MACOM  Technology  Solutions, \emph{Solderable  GaAs  Con-stant Gamma Flip-Chip Varactor Diode, MAVR-000120-1411}, available  athttps://www.macom.com/products/product-detail/MAVR-000120-14110P

\end{thebibliography}

\end{document}
